# Supplementary material for: A Density Functional Tight Binding Layer for Deep Learning of Chemical Hamiltonians
Source: arXiv:1808.04526 source file (2018-08-20)

Figure S1: Spline models for H operator trained on molecules with up to 4 heavy atoms, without regurlarization.
Red: Initial Blue: Epoch 120 Green: Epoch 250 Yellow: Epoch 540

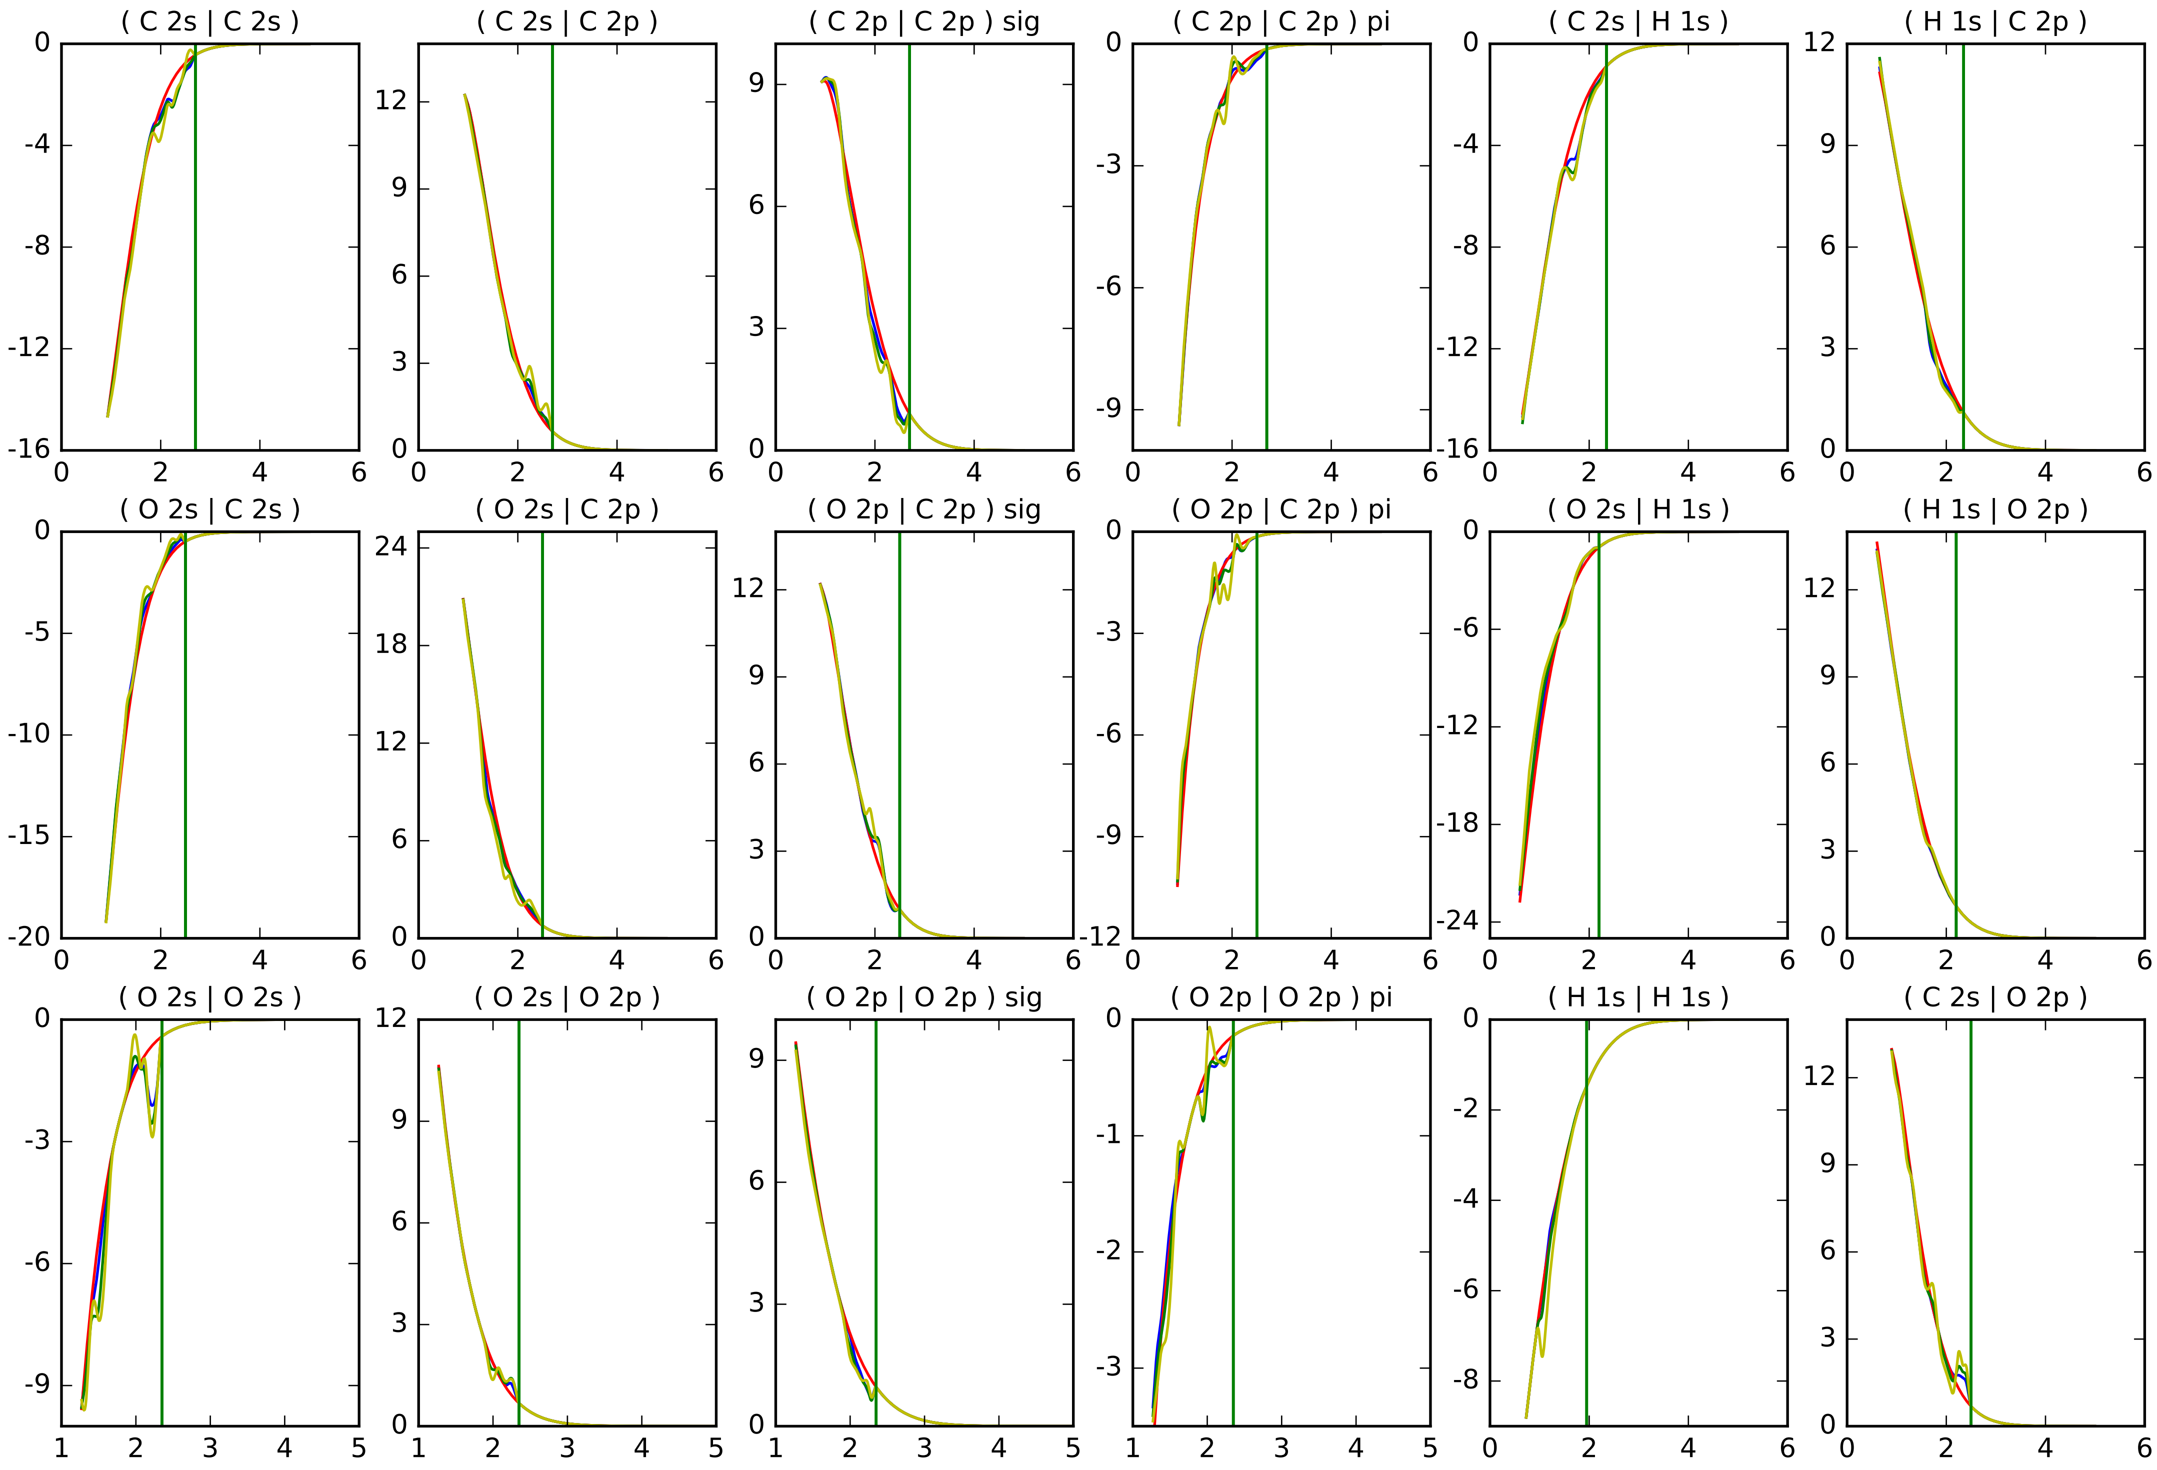

Figure S2: Spline models for G operator trained on molecules with up to 4 heavy atoms, without regurlarization.
Red: Initial Blue: Epoch 120 Green: Epoch 250 Yellow: Epoch 540

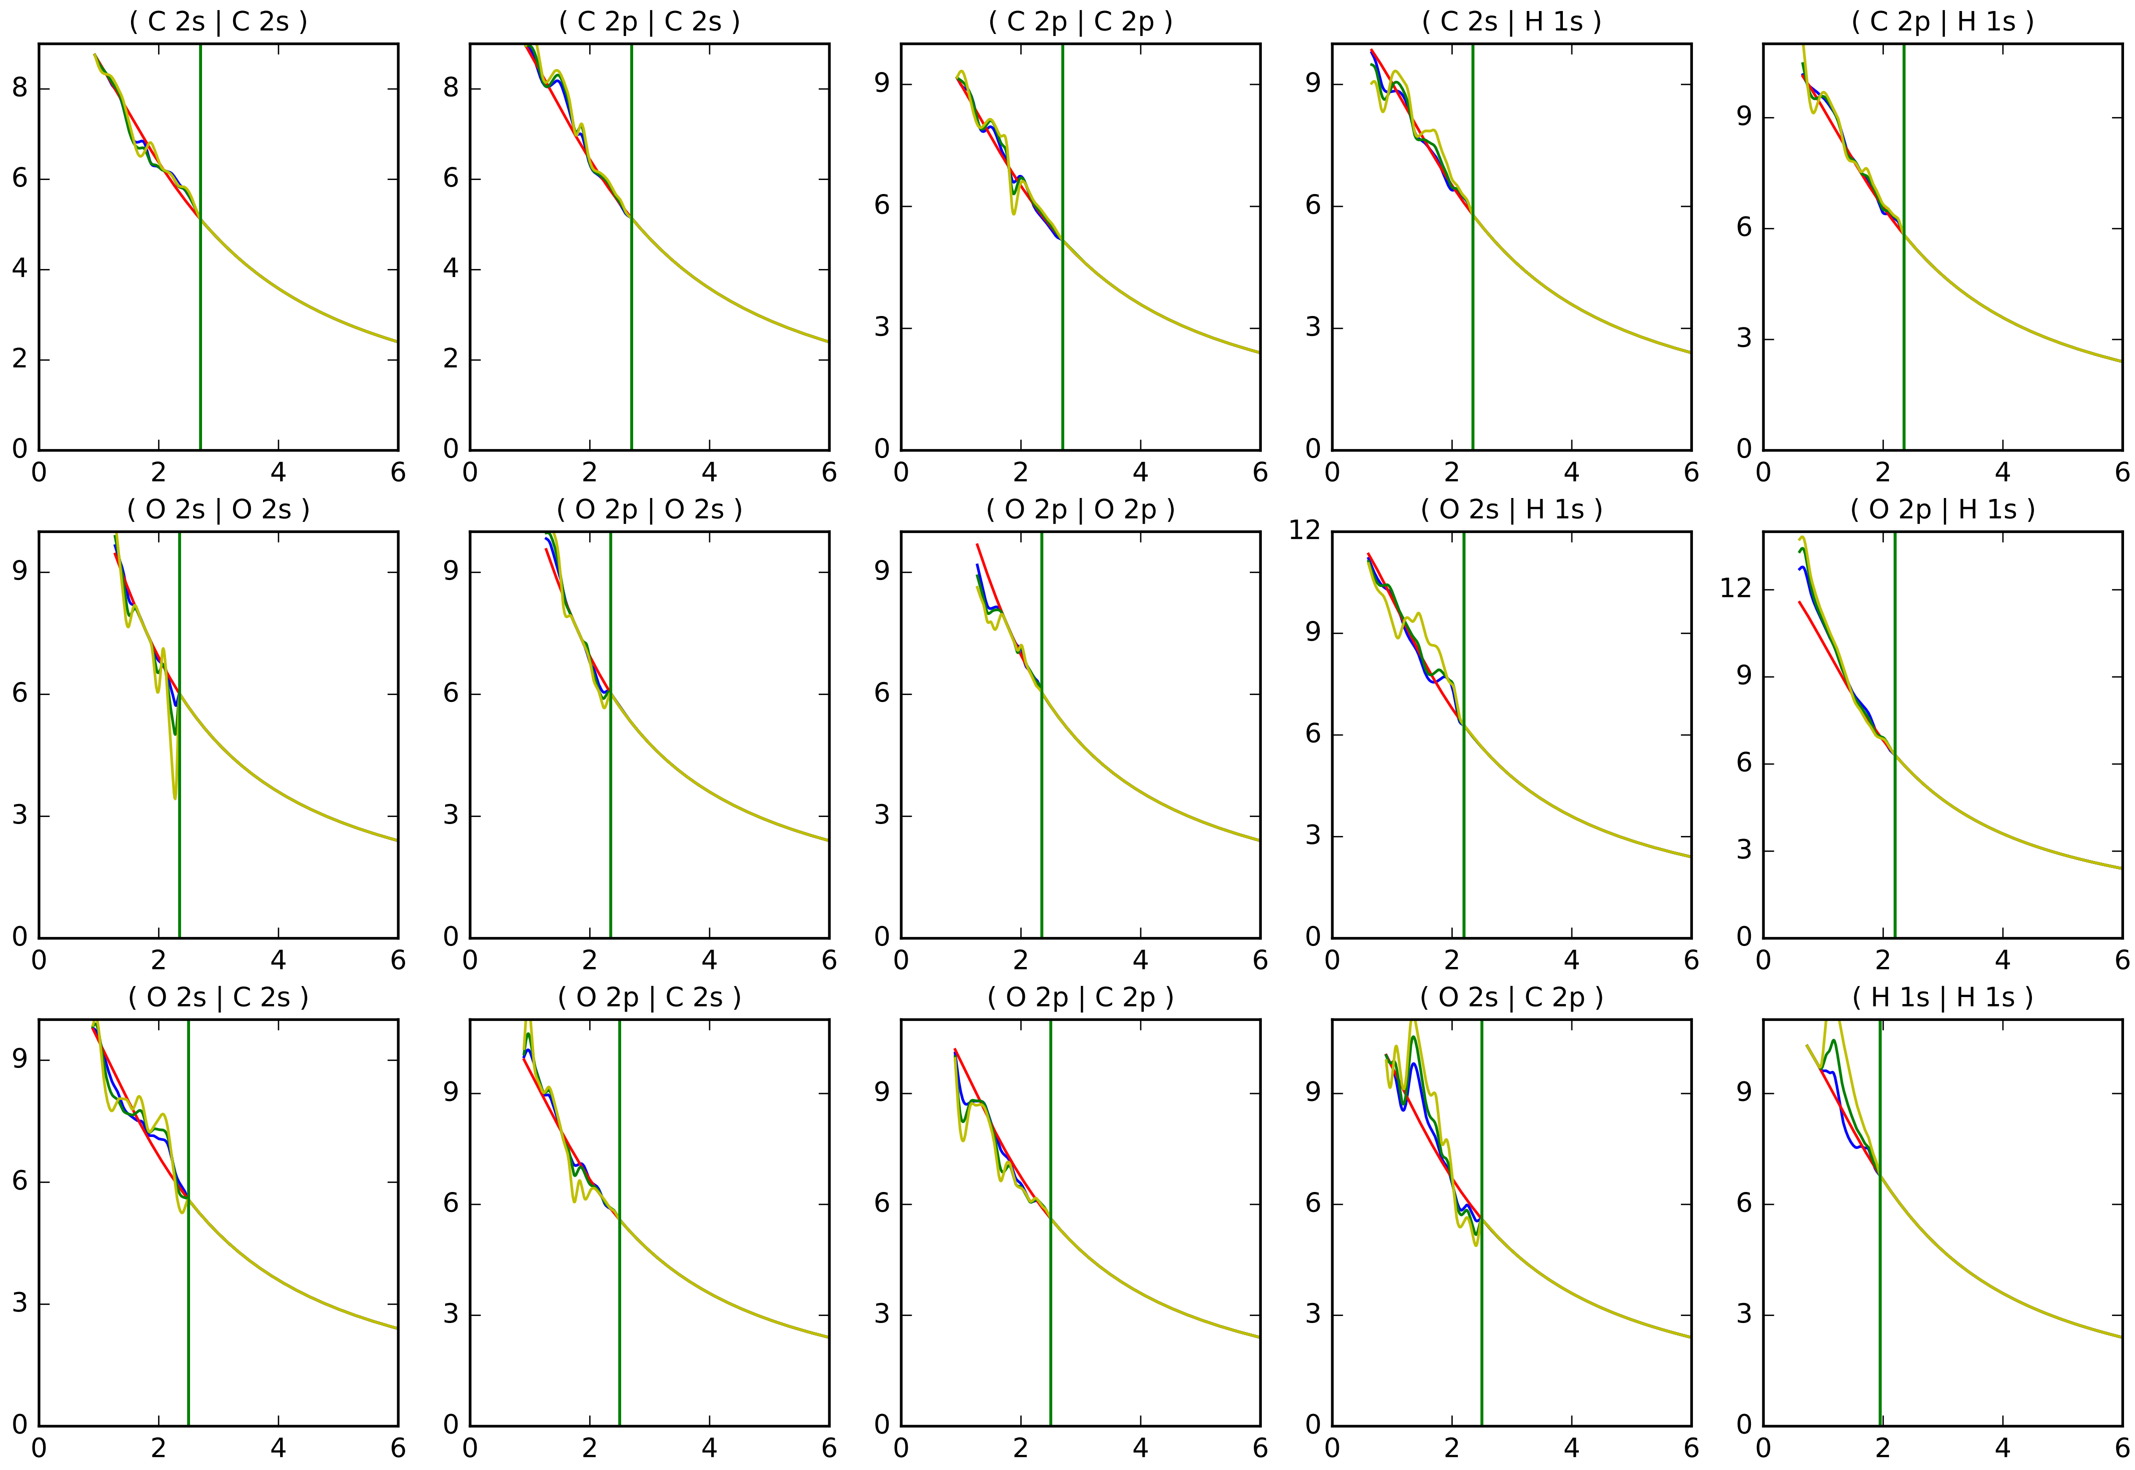

Figure S3: Spline models for R operator trained on molecules with up to 4 heavy atoms, without regurlarization.
Red: Initial Blue: Epoch 120 Green: Epoch 250 Yellow: Epoch 540

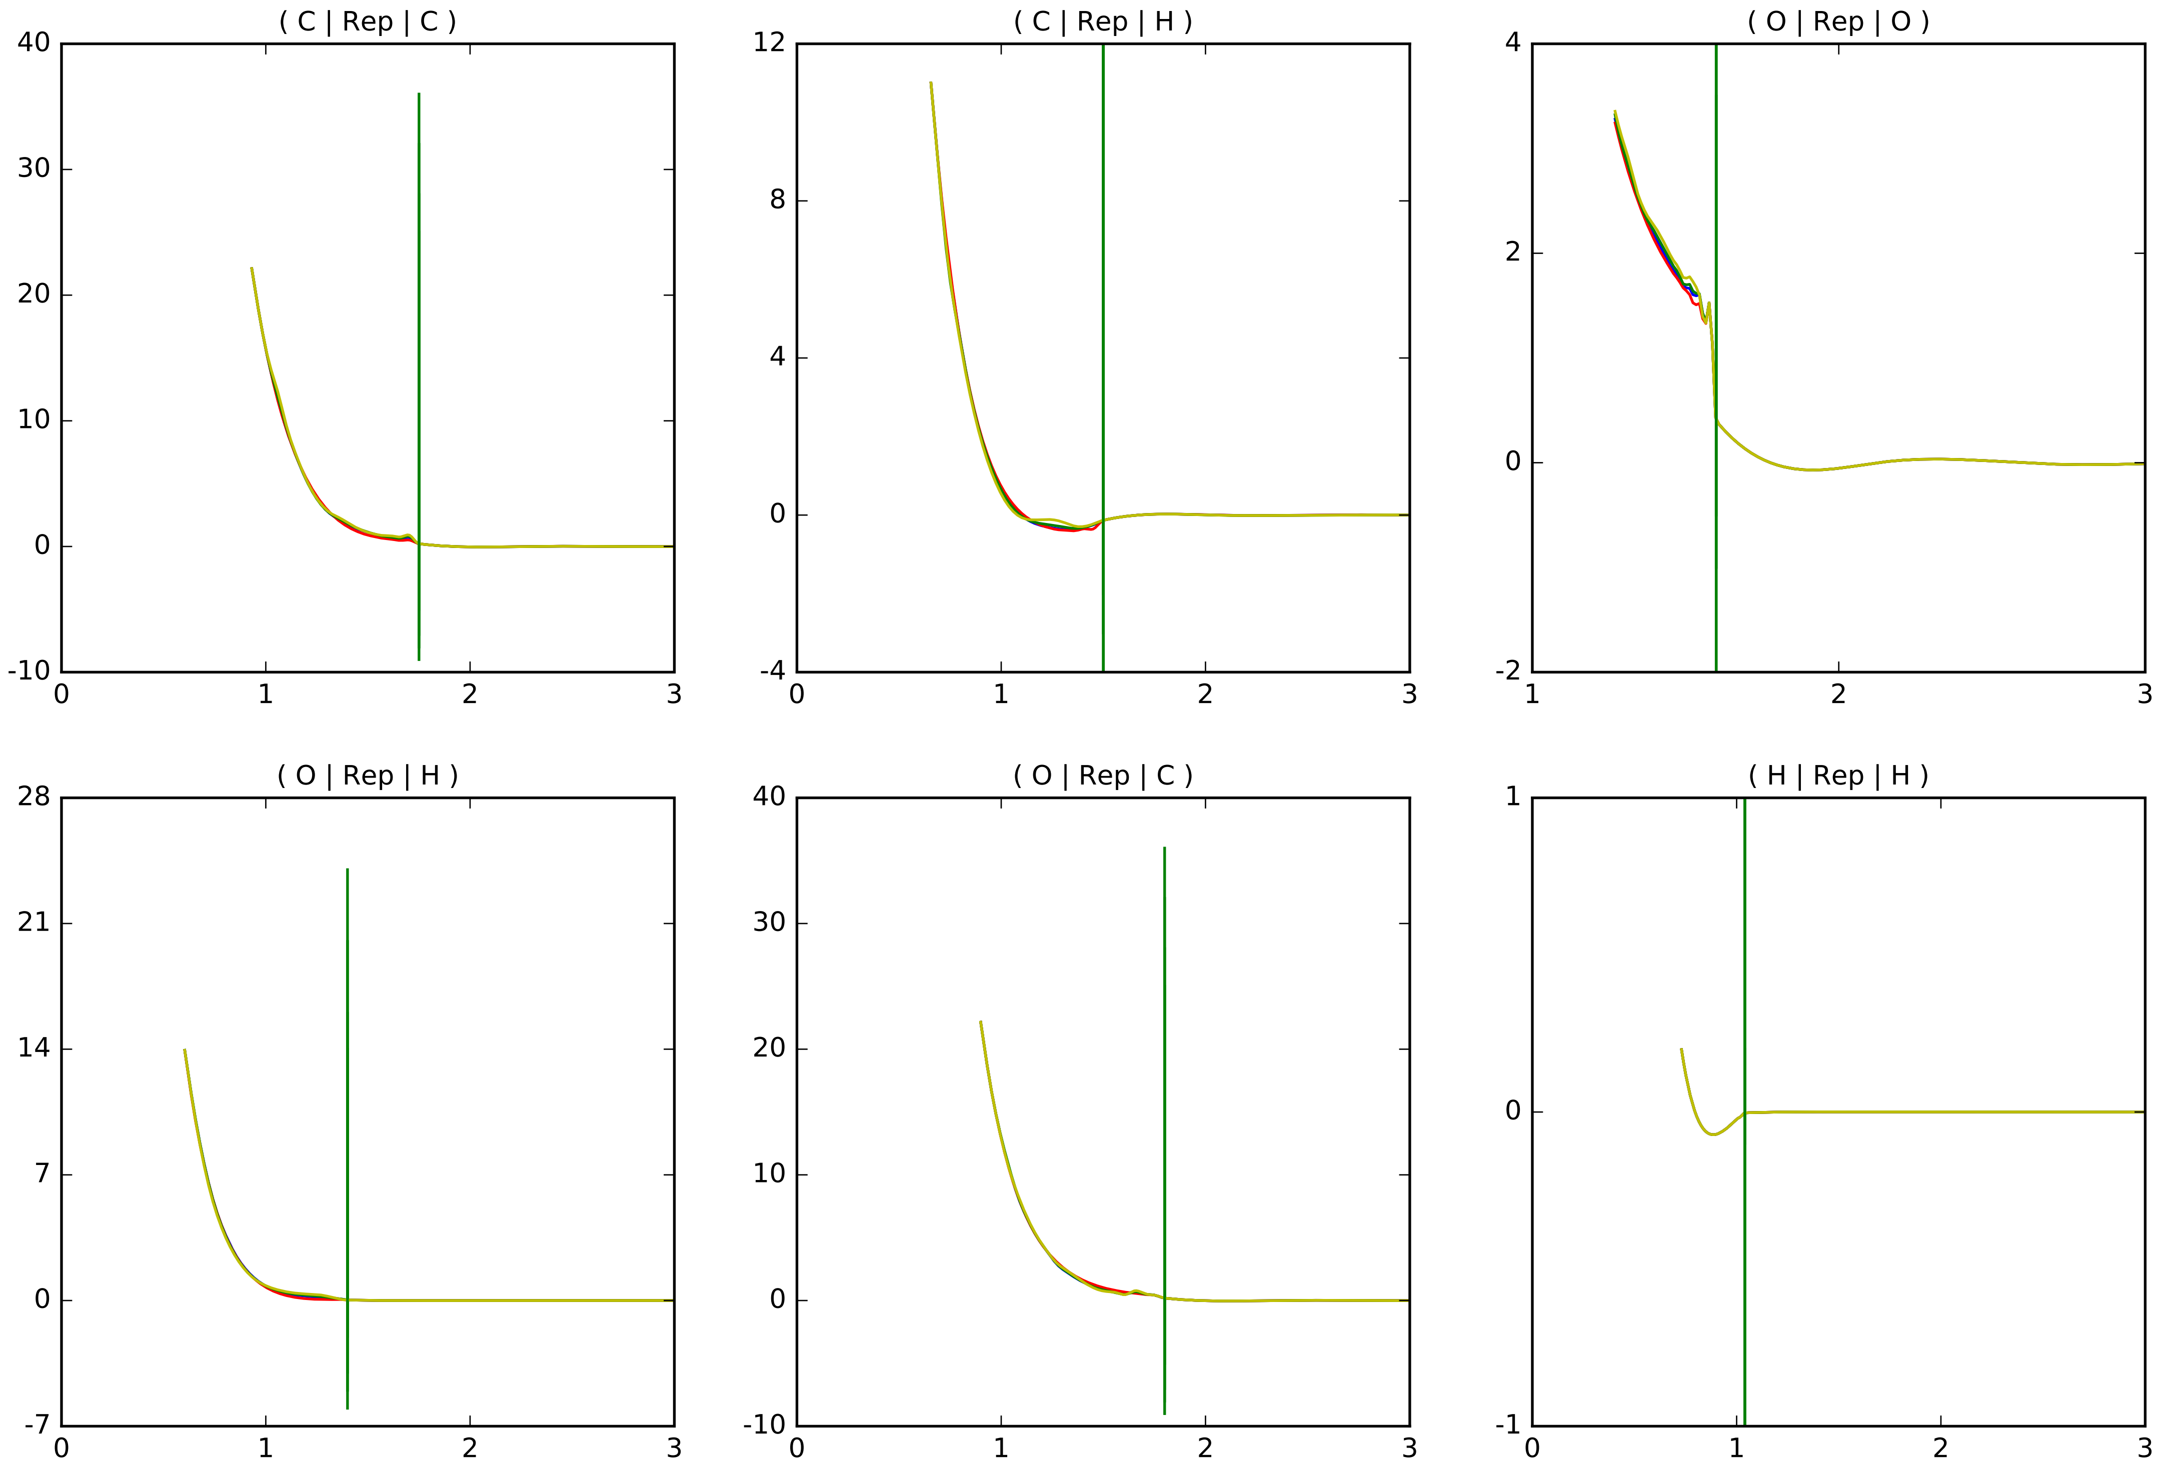

Figure S4: Spline models for H operator trained on molecules with up to 7 heavy atoms, without regurlarization.
Red: Initial Blue: Epoch 120 Green: Epoch 250 Yellow: Epoch 540

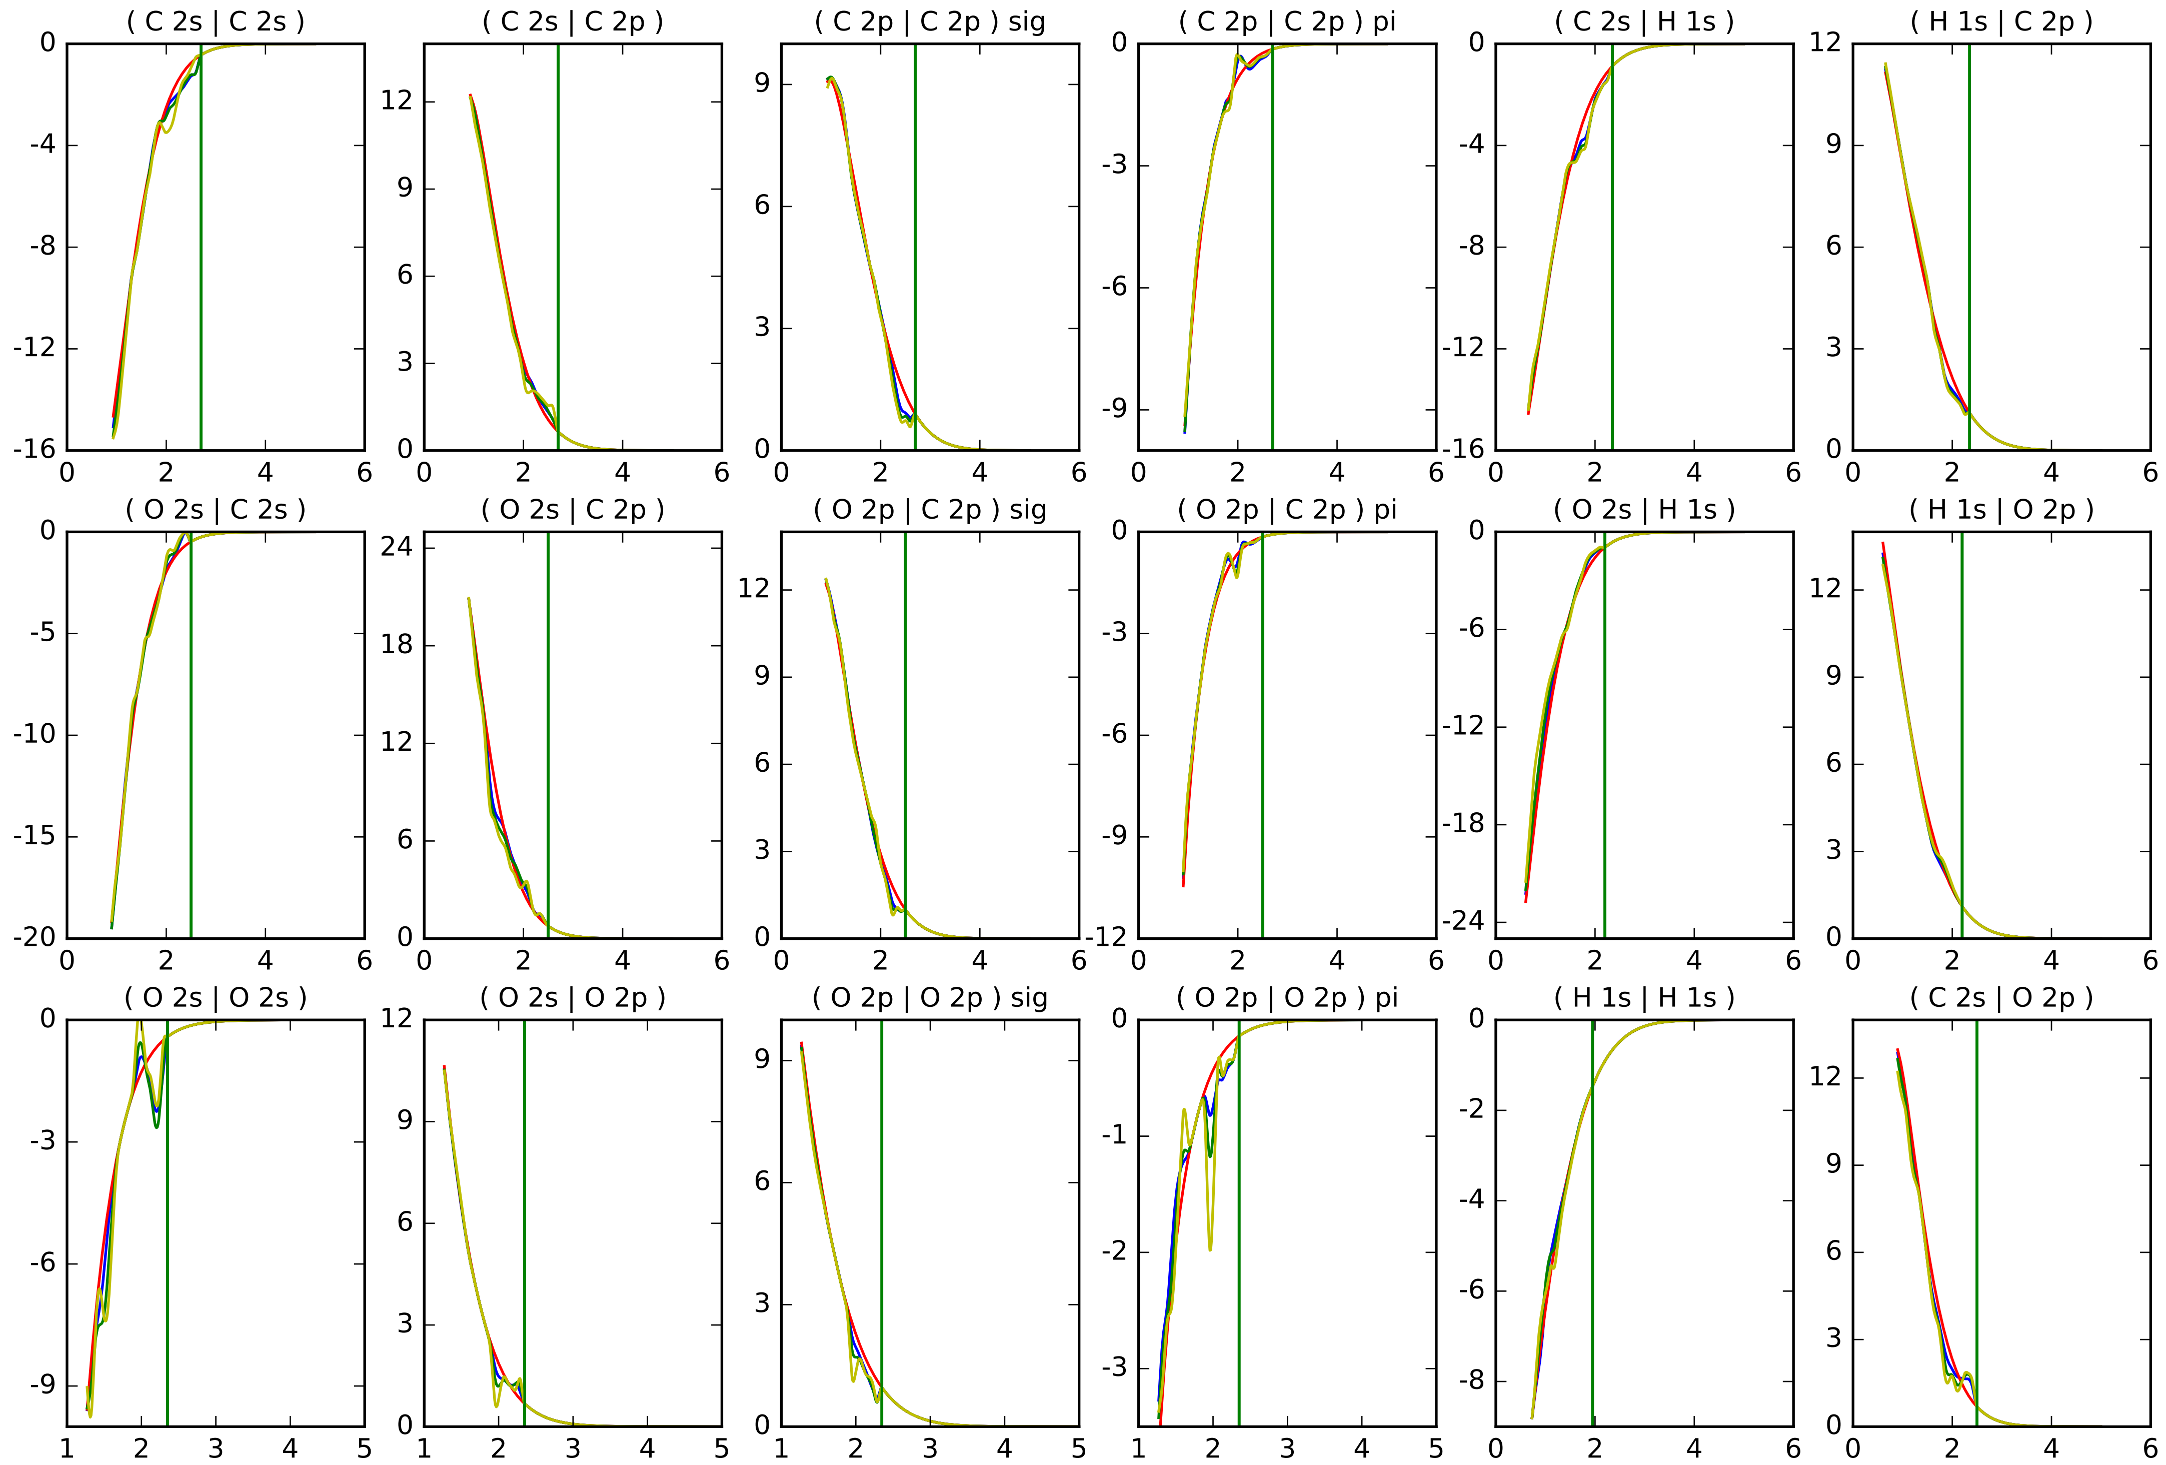

Figure S5: Spline models for G operator trained on molecules with up to 7 heavy atoms, without regurlarization.
Red: Initial Blue: Epoch 120 Green: Epoch 250 Yellow: Epoch 540

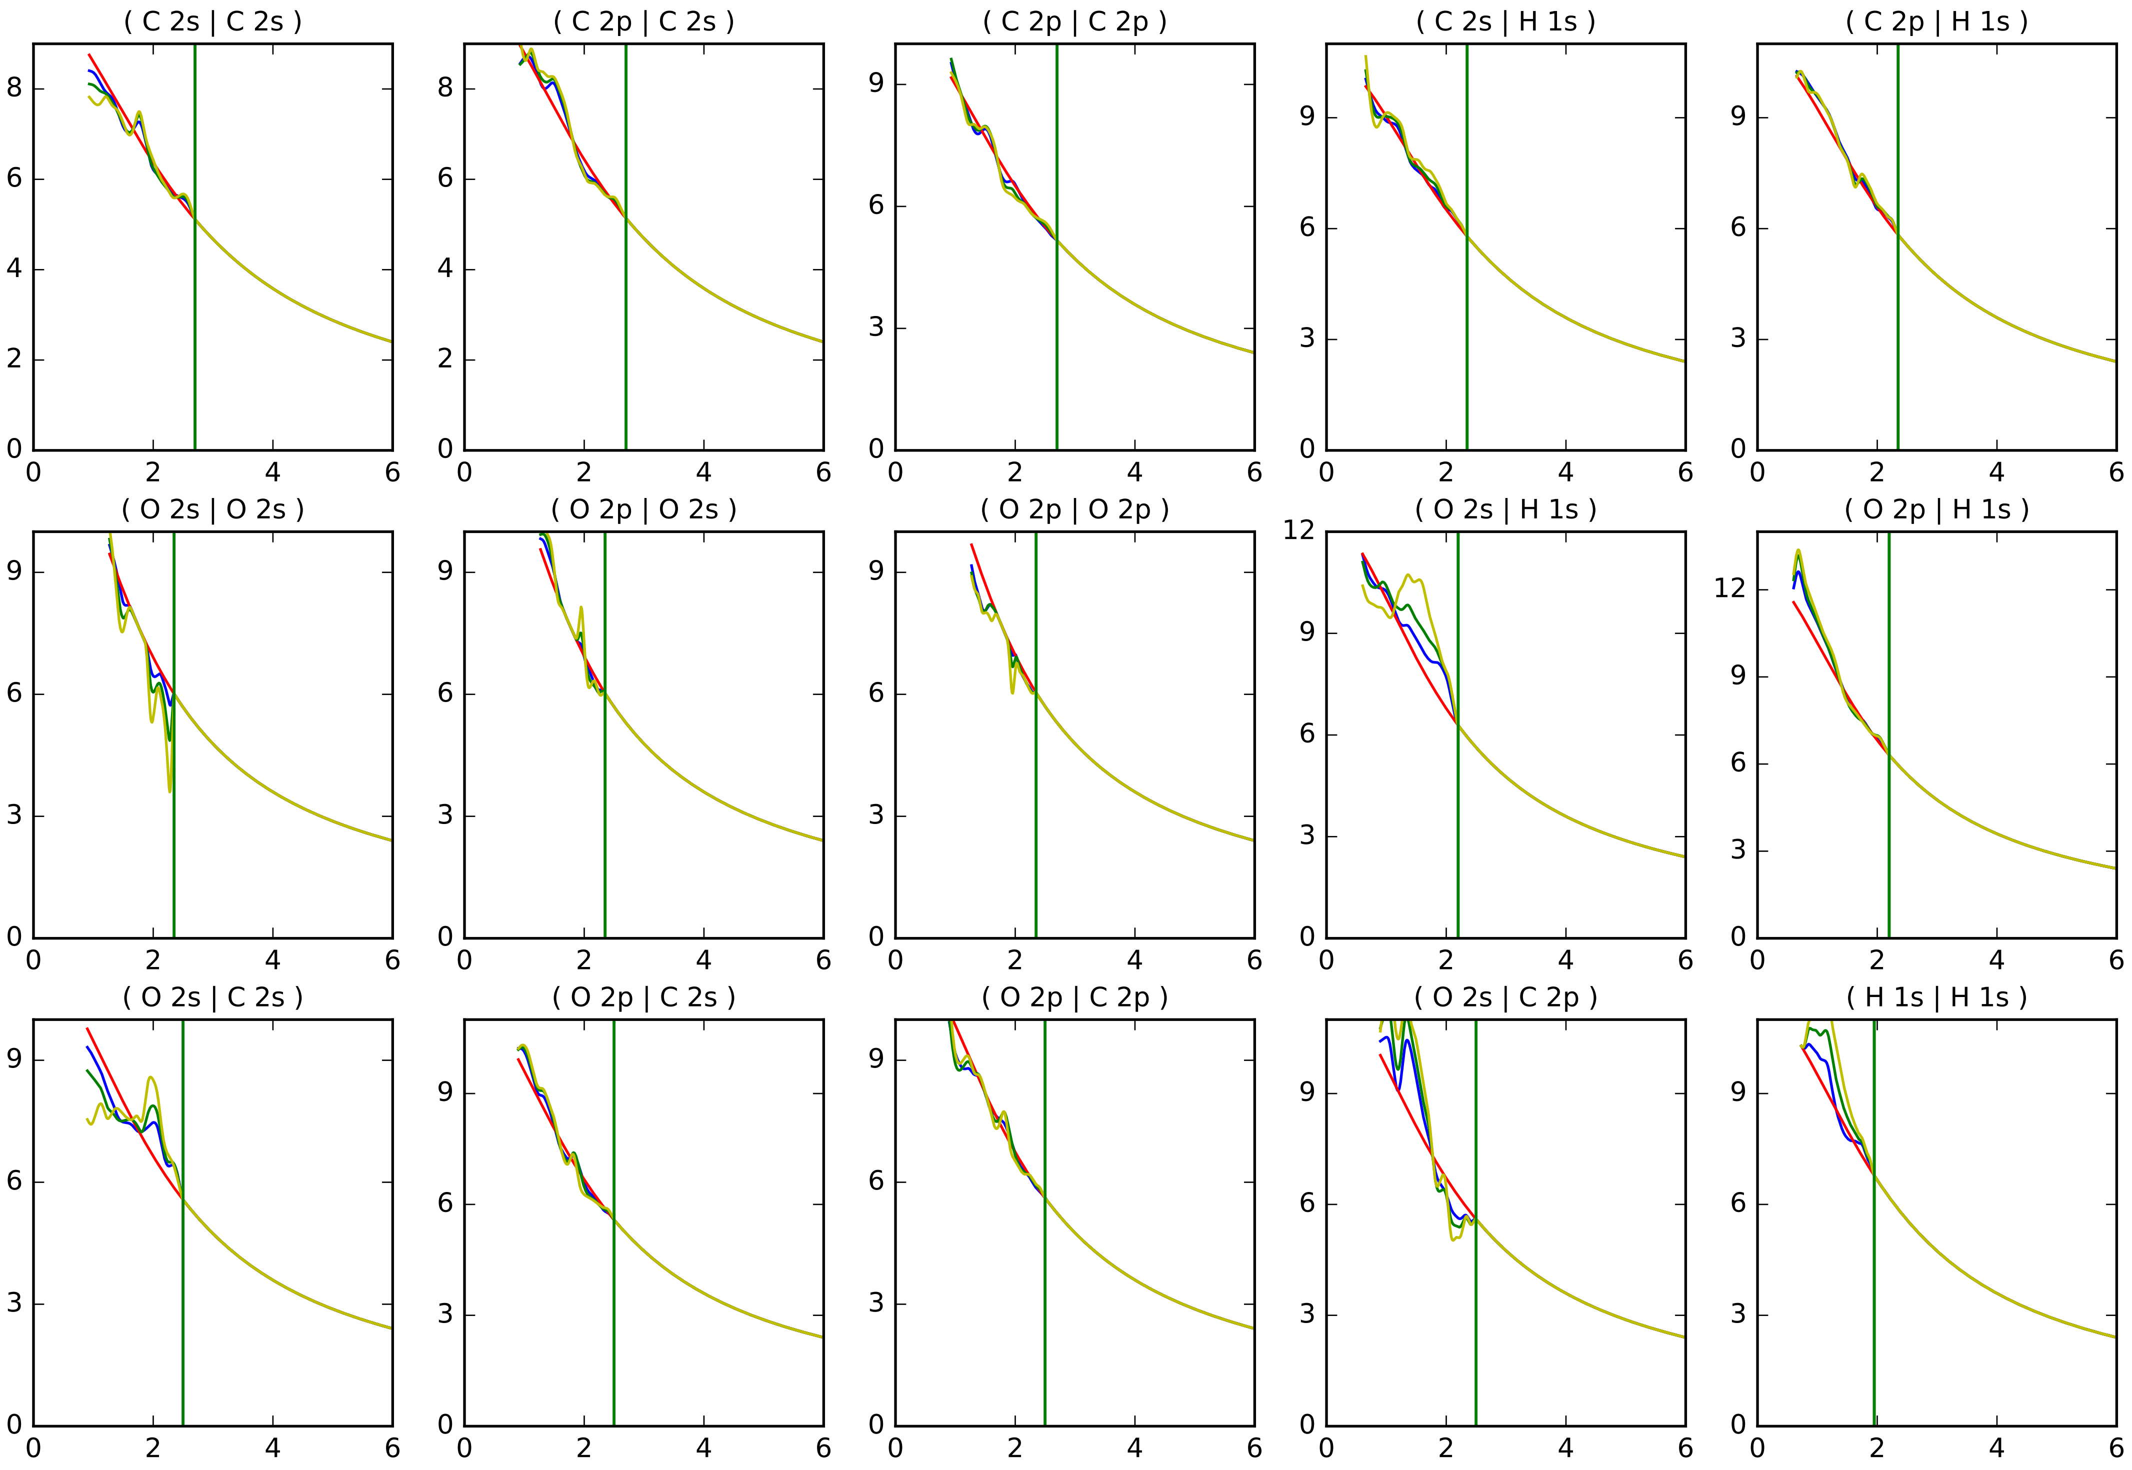

Figure S6: Spline models for R operator trained on molecules with up to 7 heavy atoms, without regurlarization.
Red: Initial Blue: Epoch 120 Green: Epoch 250 Yellow: Epoch 540

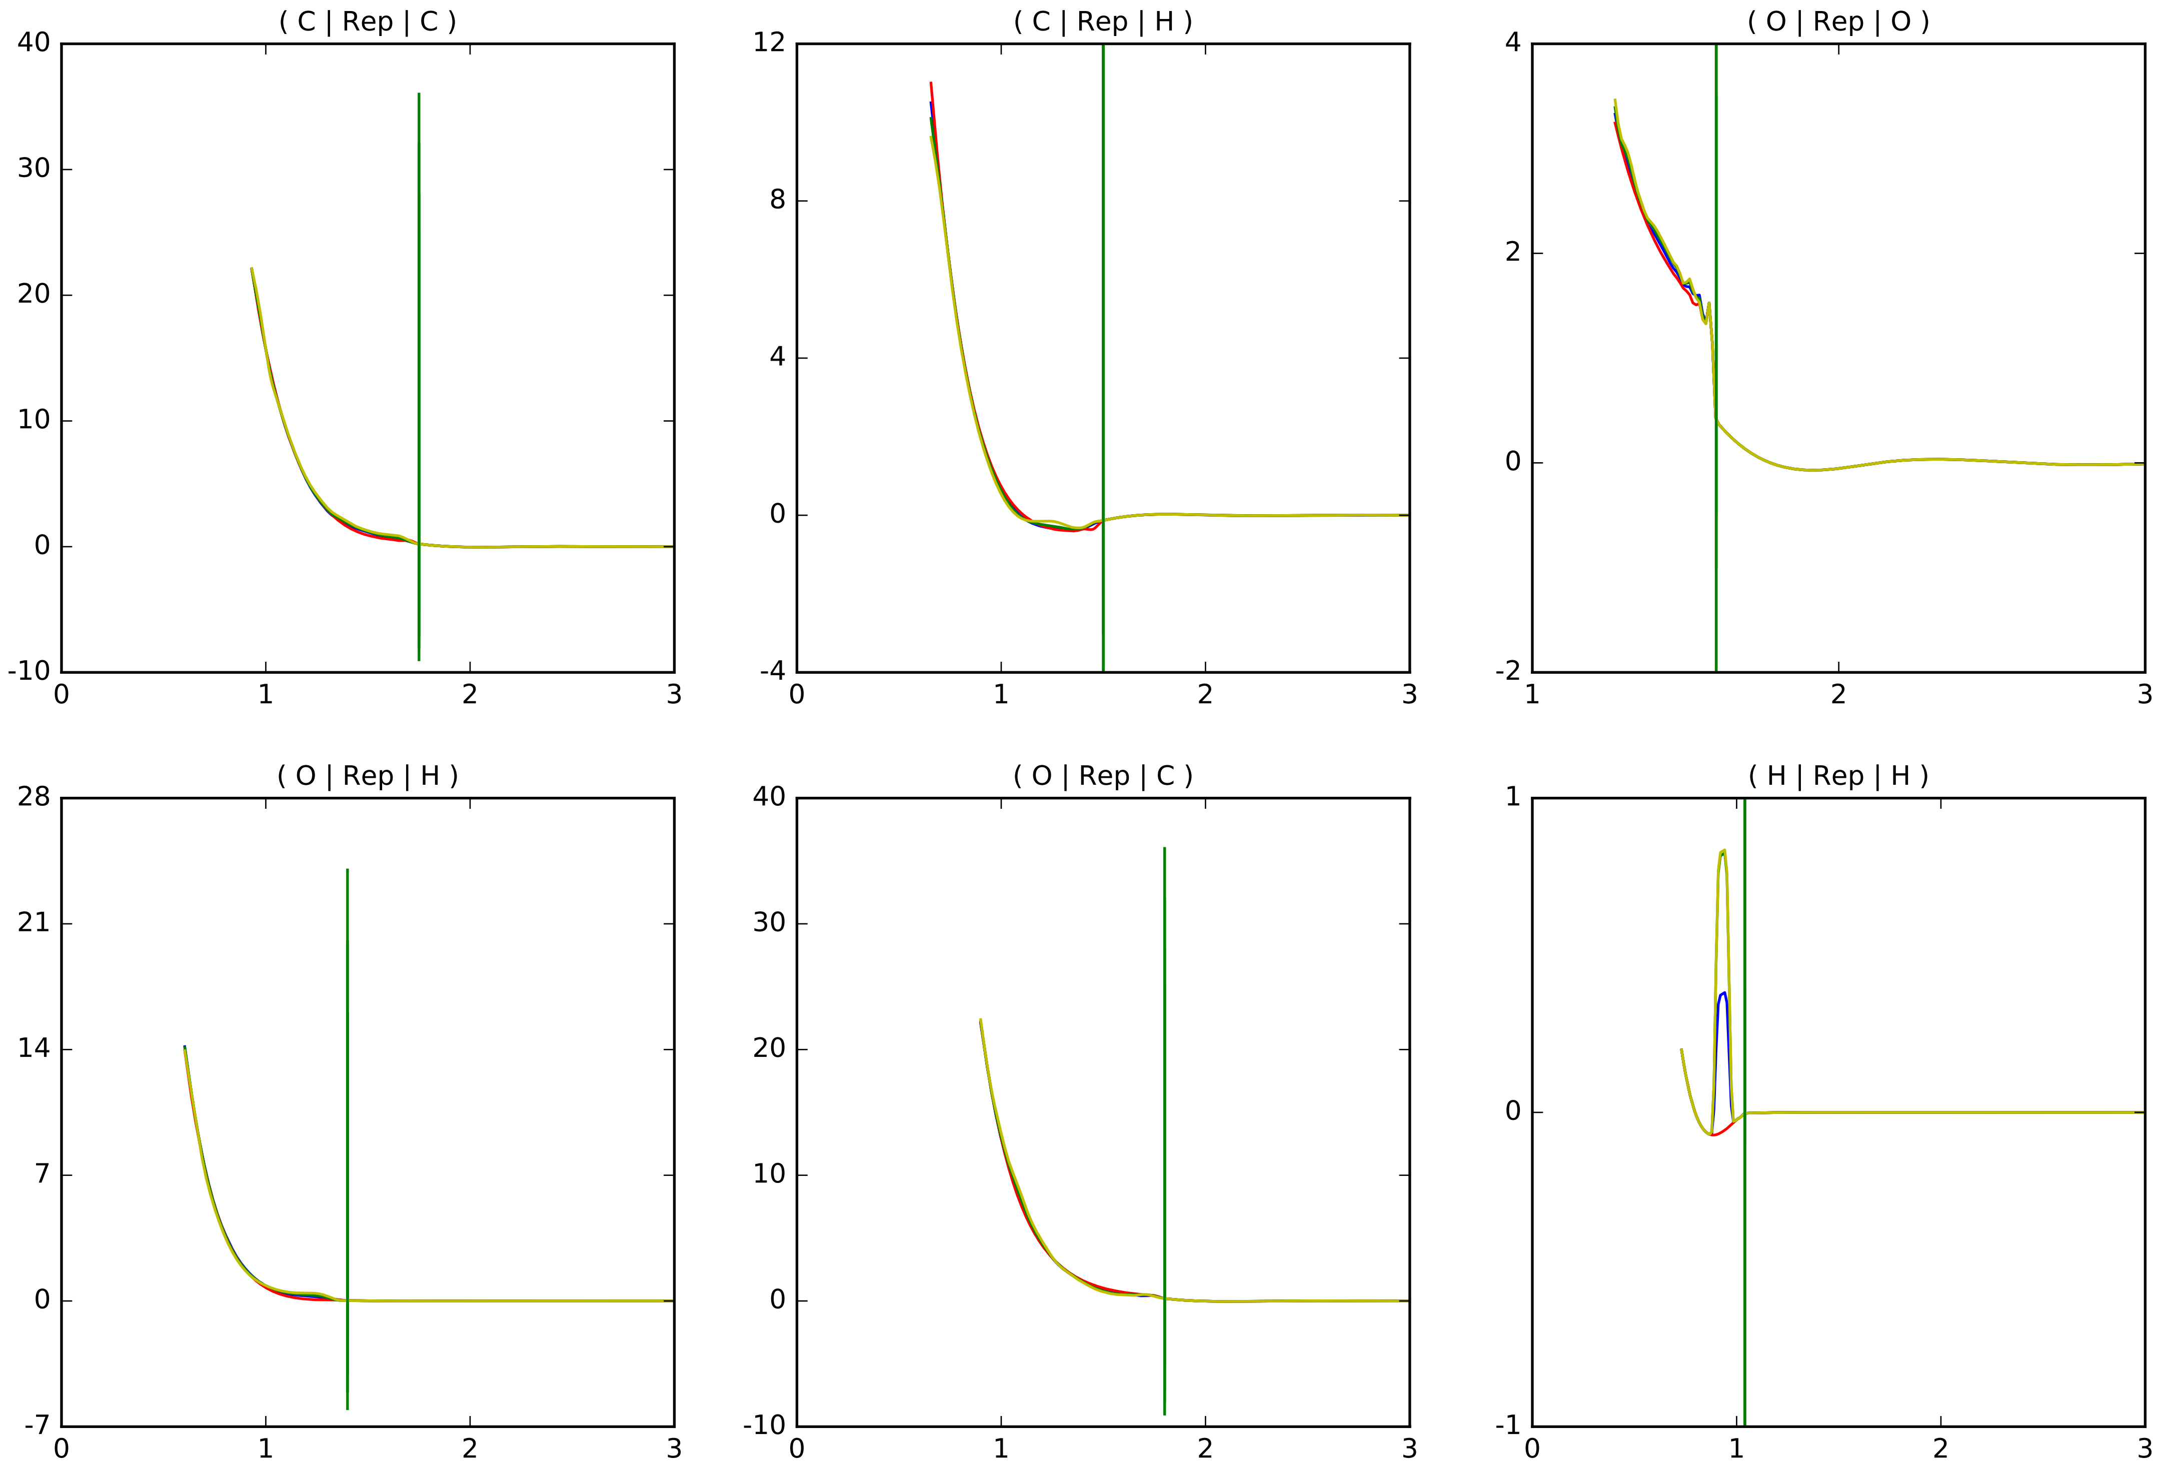

Figure S7: Spline models for H operator trained on molecules with up to 4 heavy atoms, with monotonic regurlarization.
Red: Initial Blue: Epoch 120 Green: Epoch 250 Yellow: Epoch 540

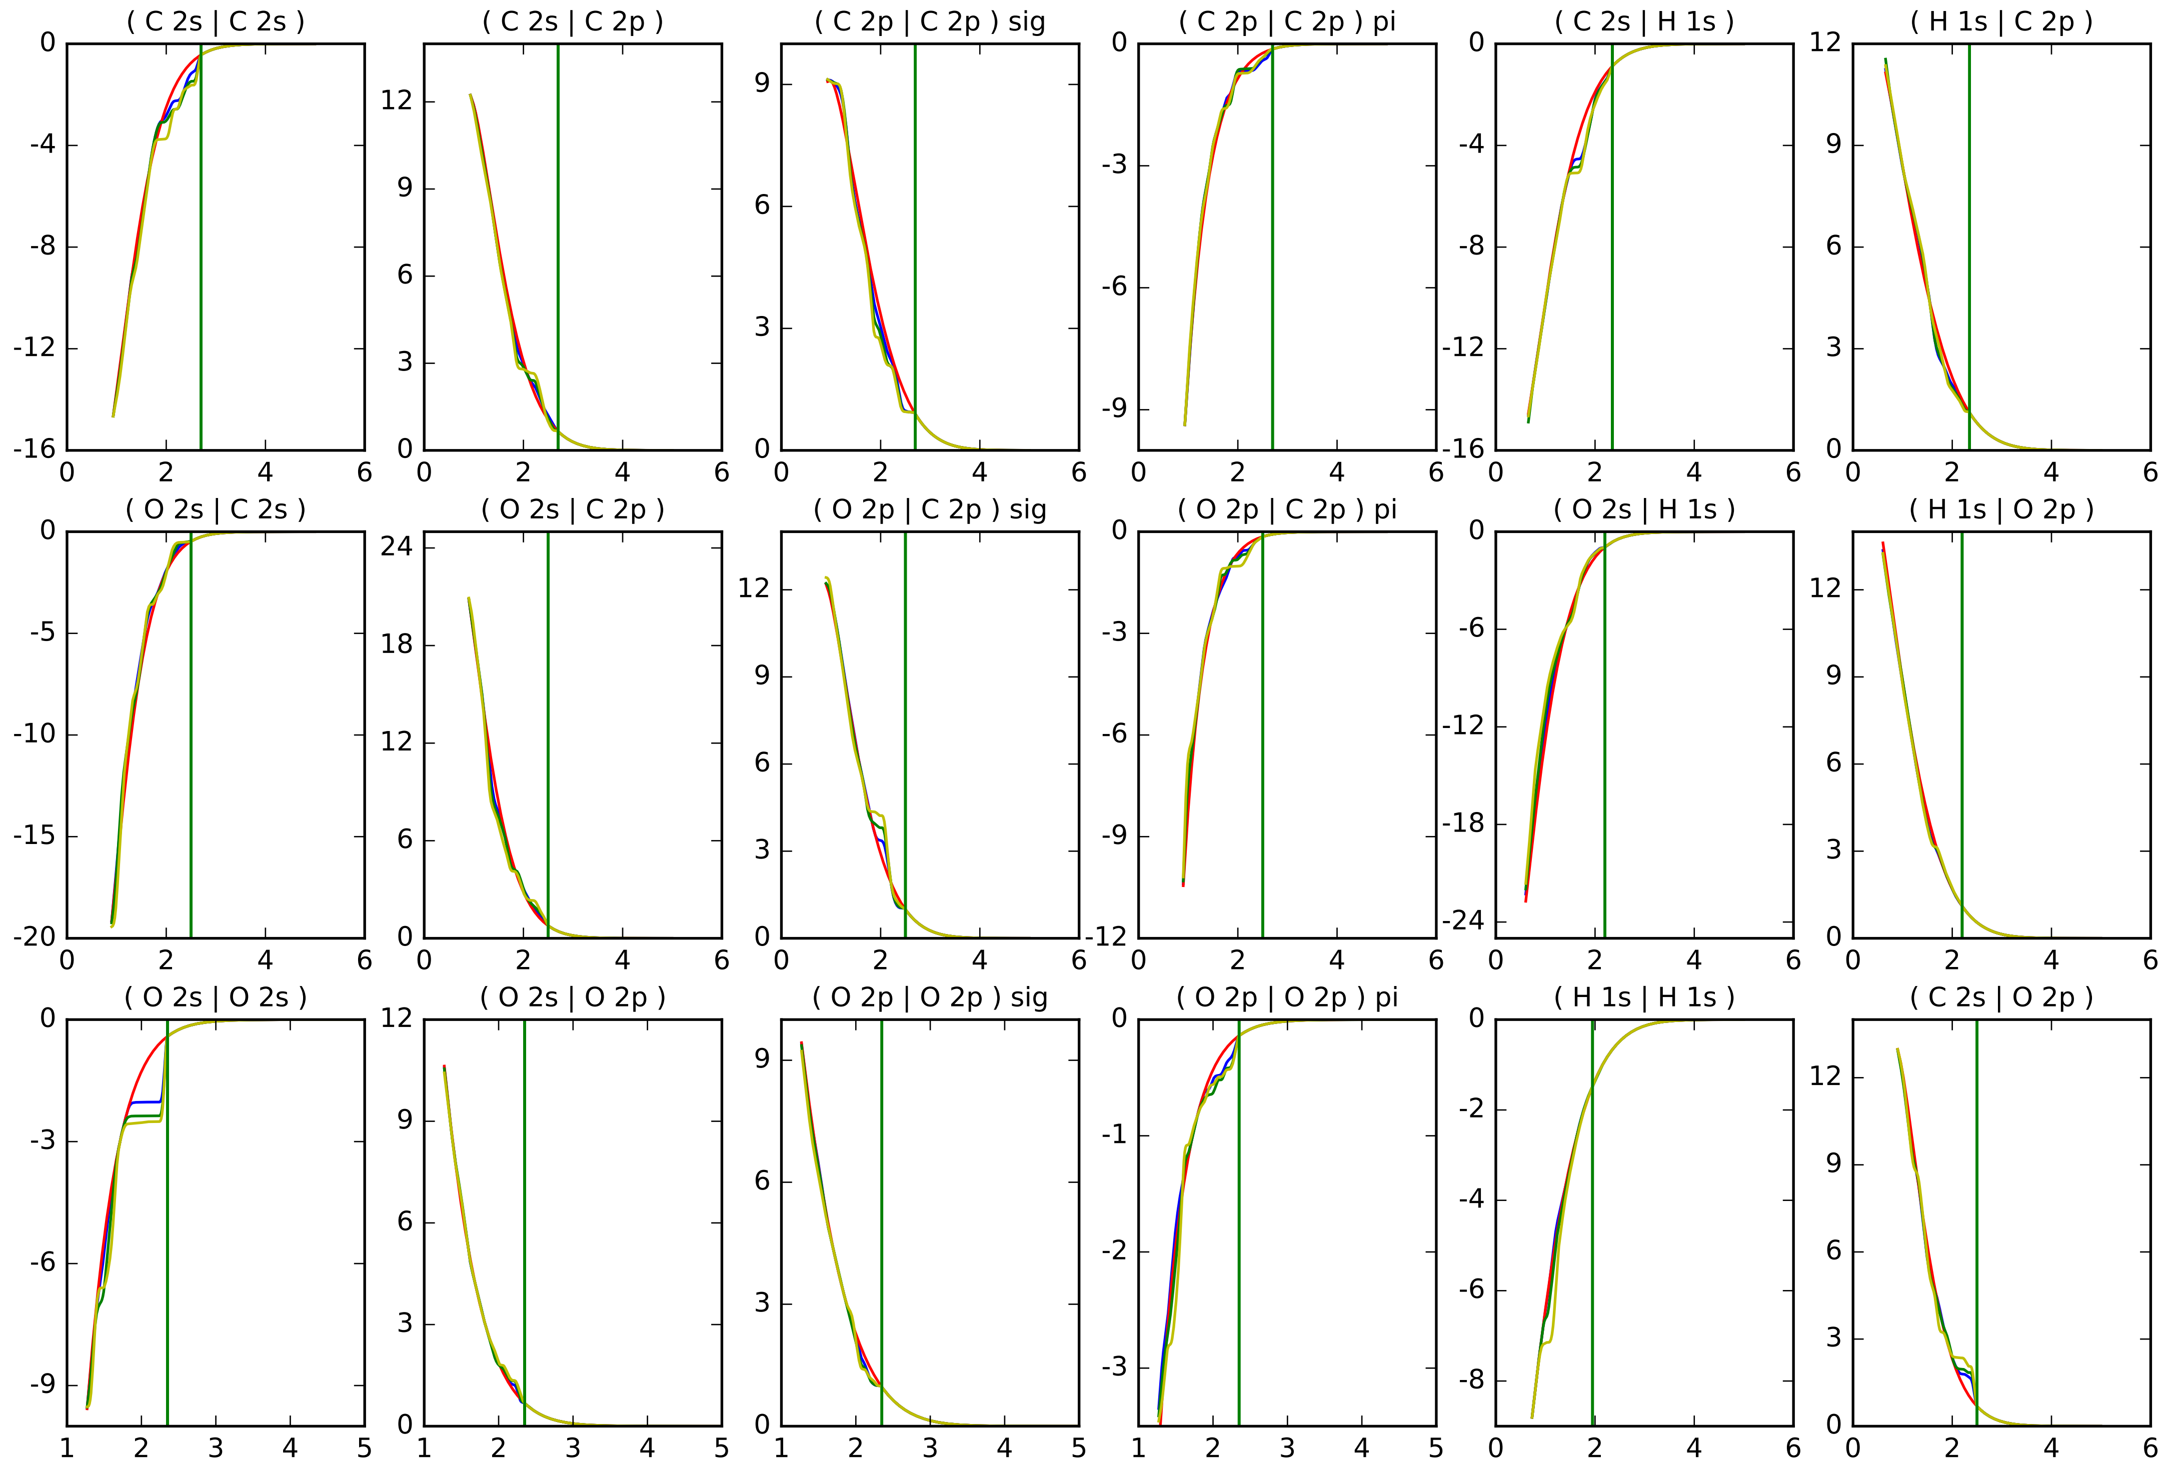

Figure S8: Spline models for G operator trained on molecules with up to 4 heavy atoms, with monotonic regurlarization.
Red: Initial Blue: Epoch 120 Green: Epoch 250 Yellow: Epoch 540

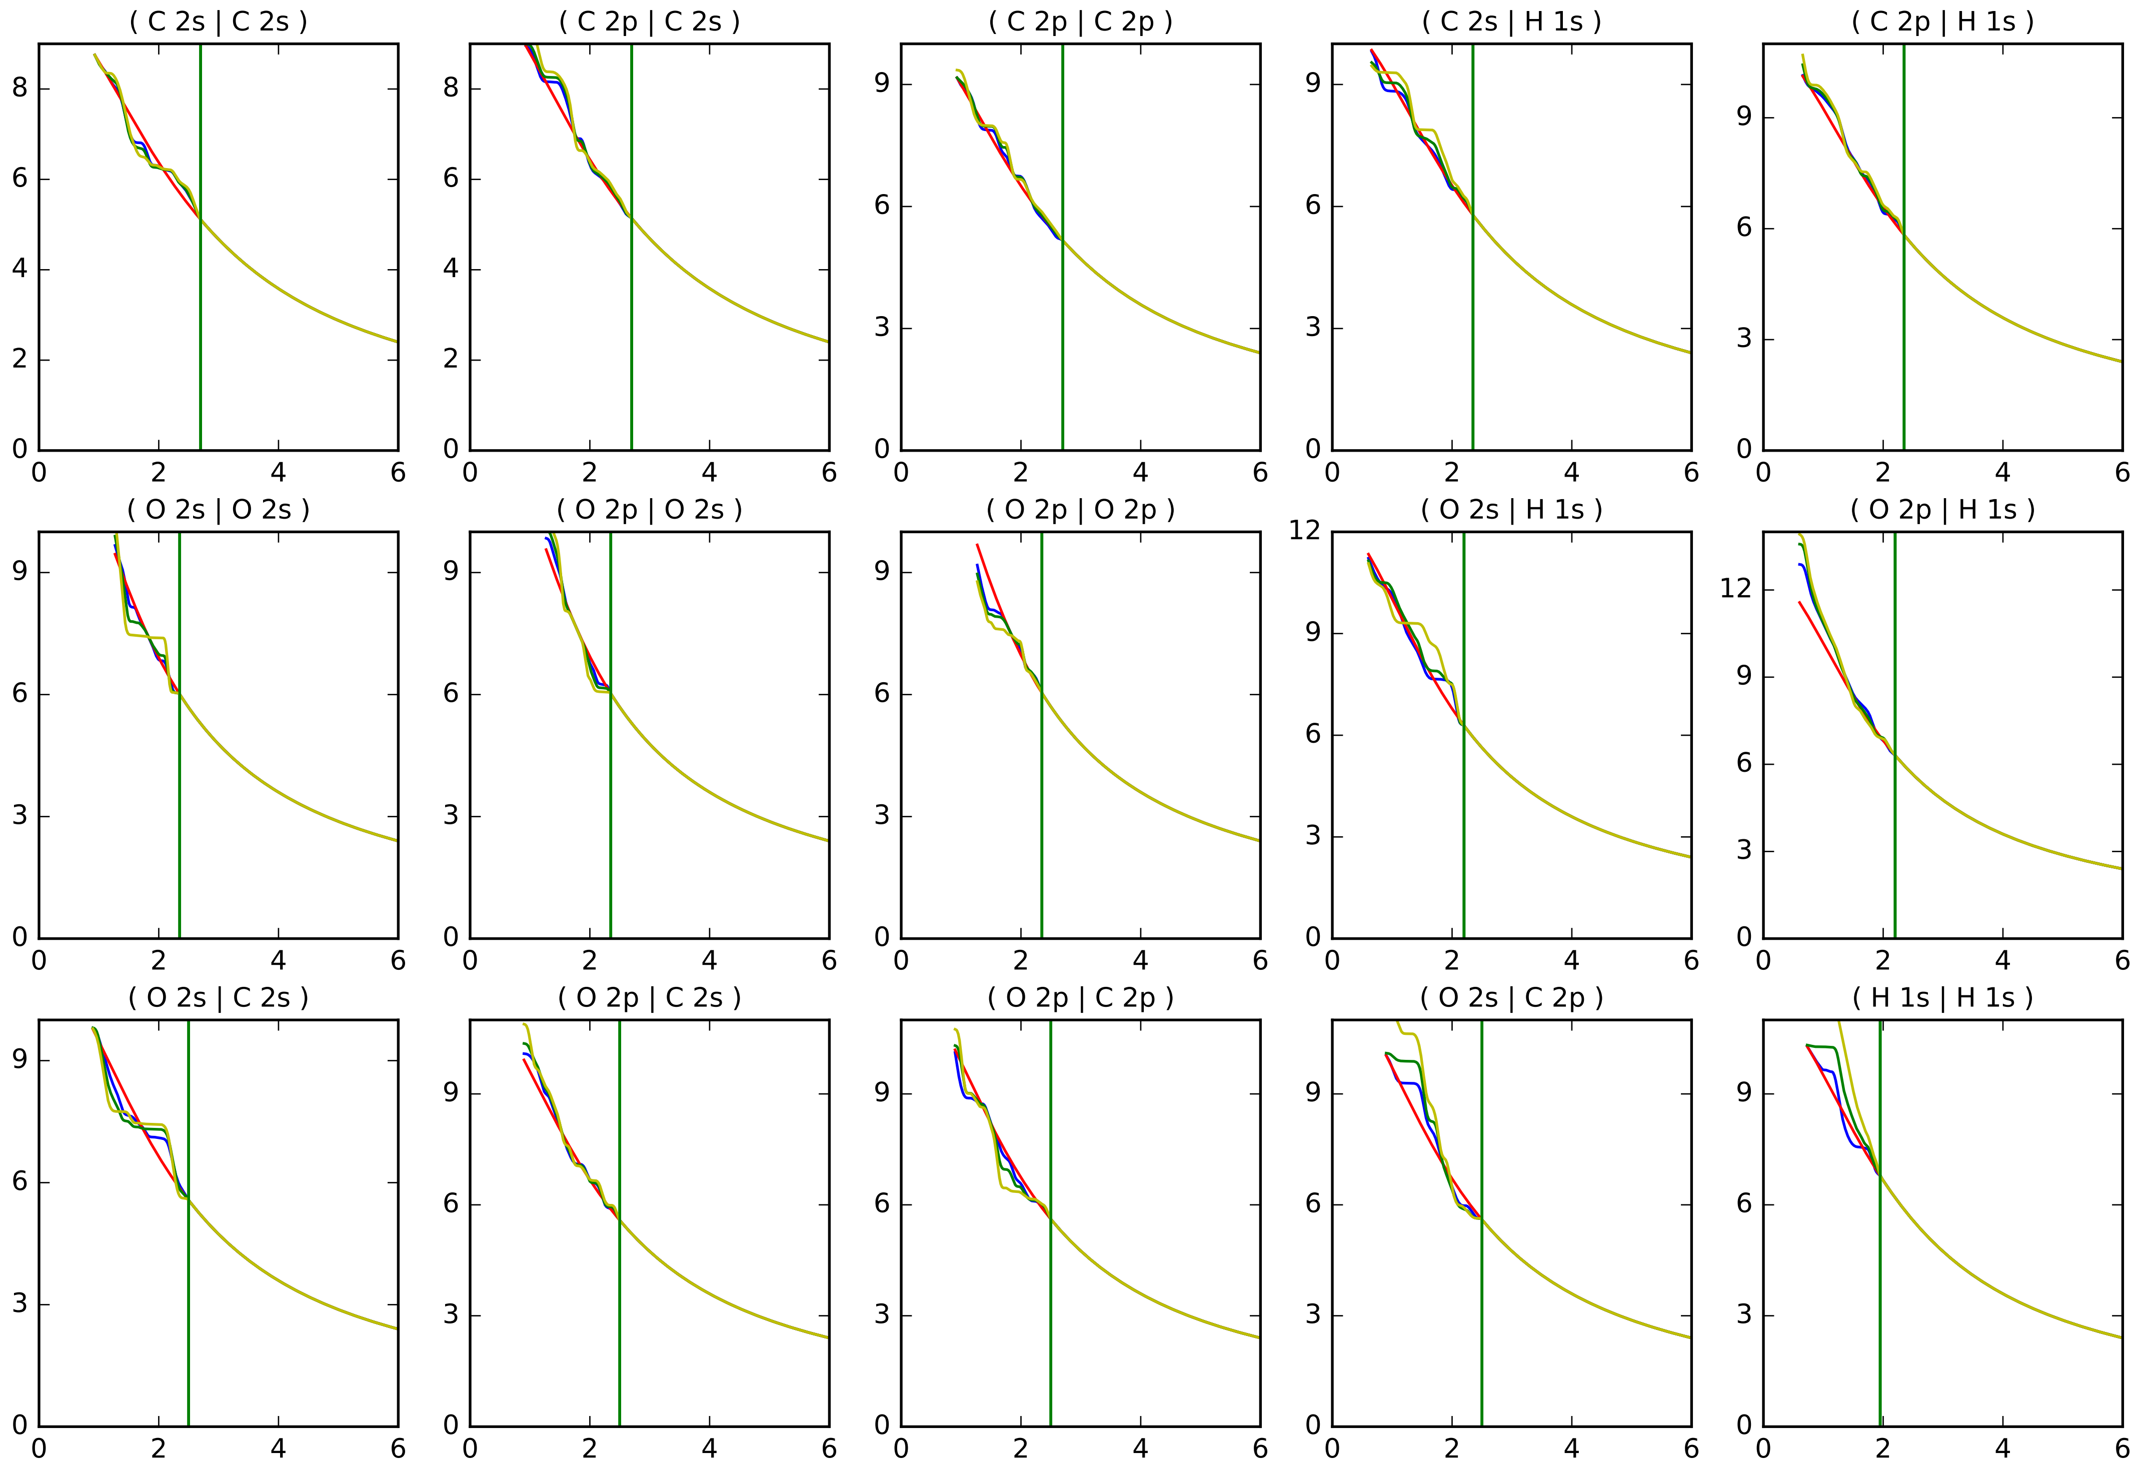

Figure S9: Spline models for R operator trained on molecules with up to 4 heavy atoms, with monotonic regurlarization.
Red: Initial Blue: Epoch 120 Green: Epoch 250 Yellow: Epoch 540

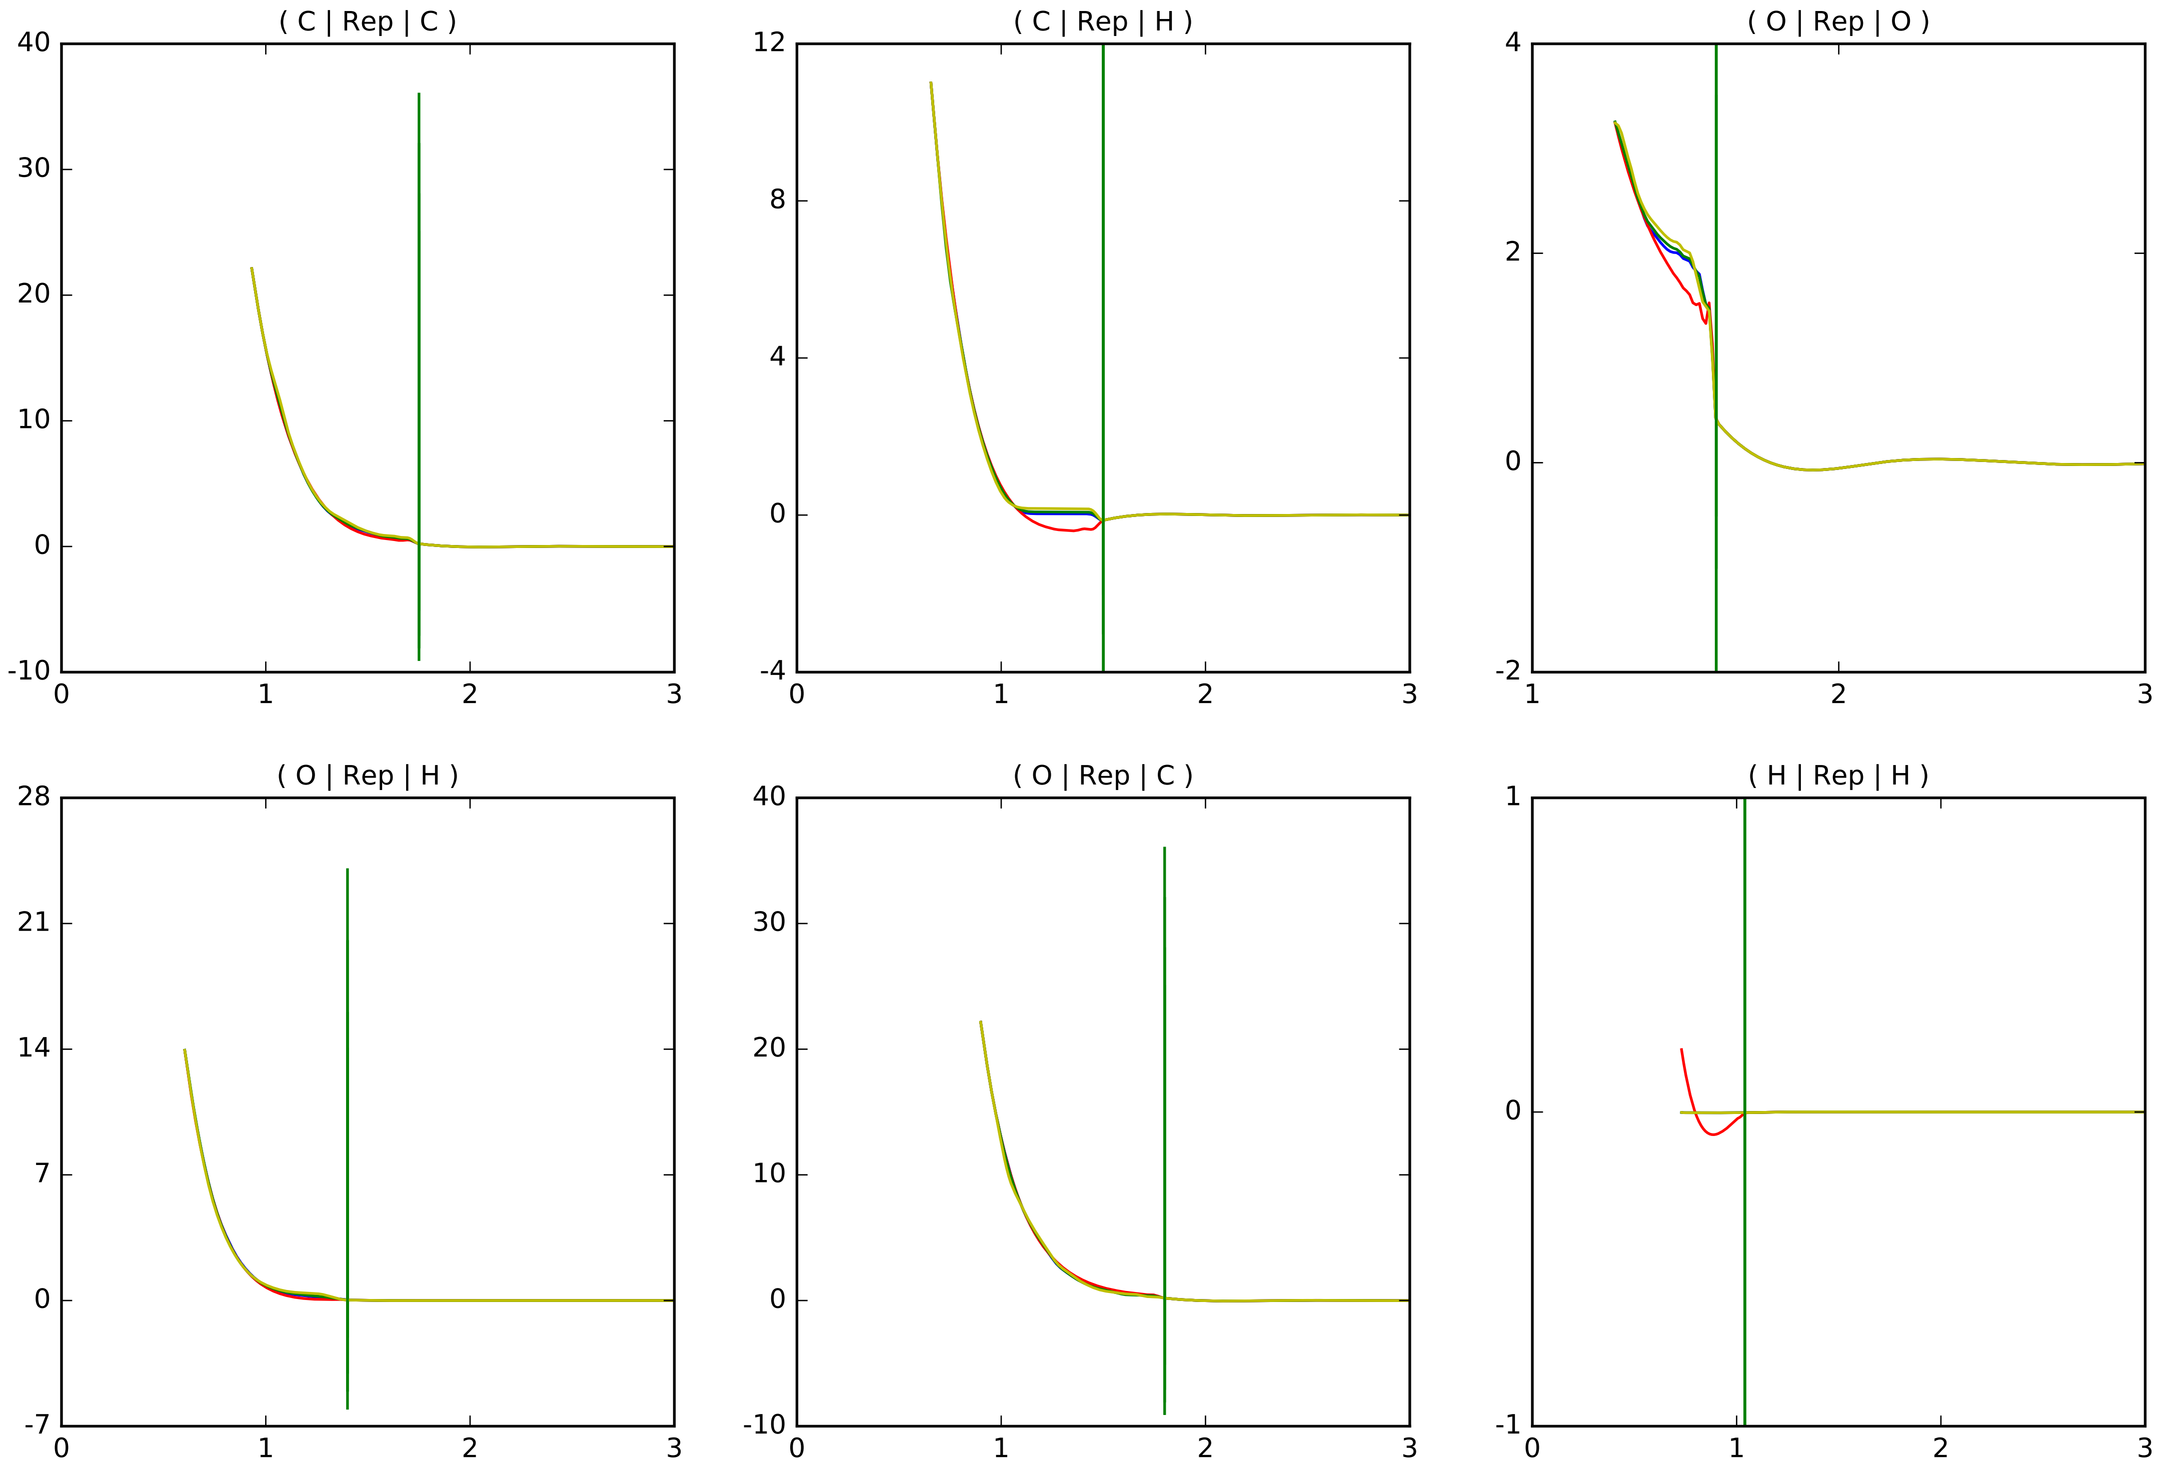

Figure S10: Spline models for H operator trained on molecules with up to 7 heavy atoms, with monotonic regurlarization.
Red: Initial Blue: Epoch 120 Green: Epoch 250 Yellow: Epoch 540

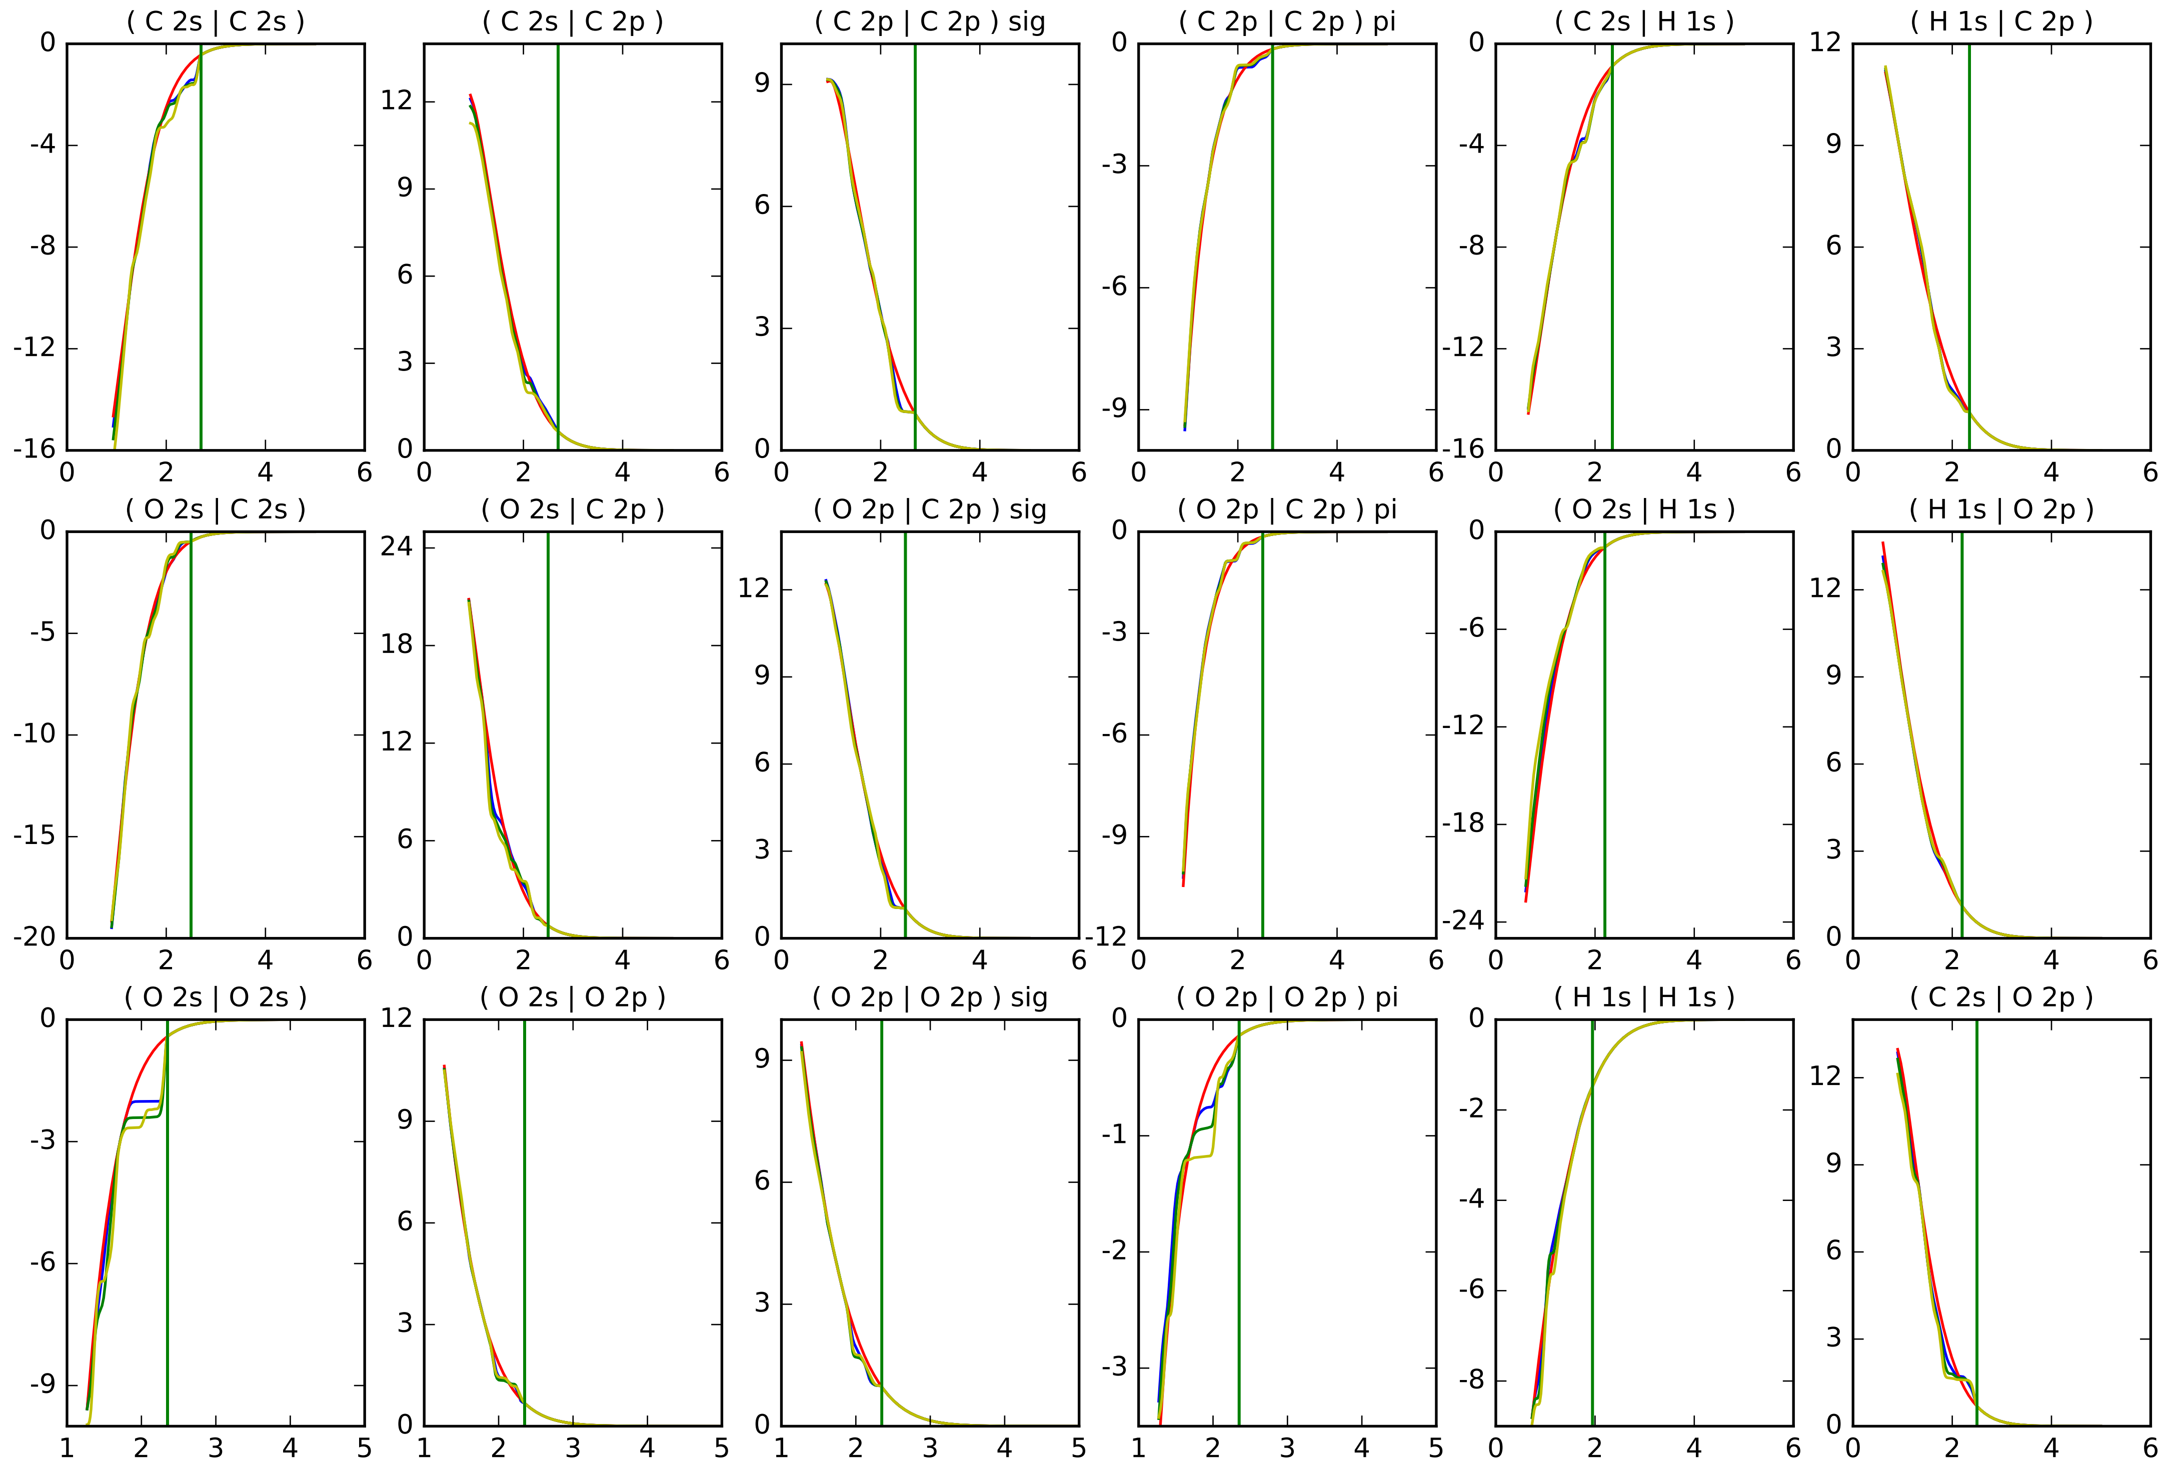

Figure S11: Spline models for G operator trained on molecules with up to 7 heavy atoms, with monotonic regurlarization.
Red: Initial Blue: Epoch 120 Green: Epoch 250 Yellow: Epoch 540

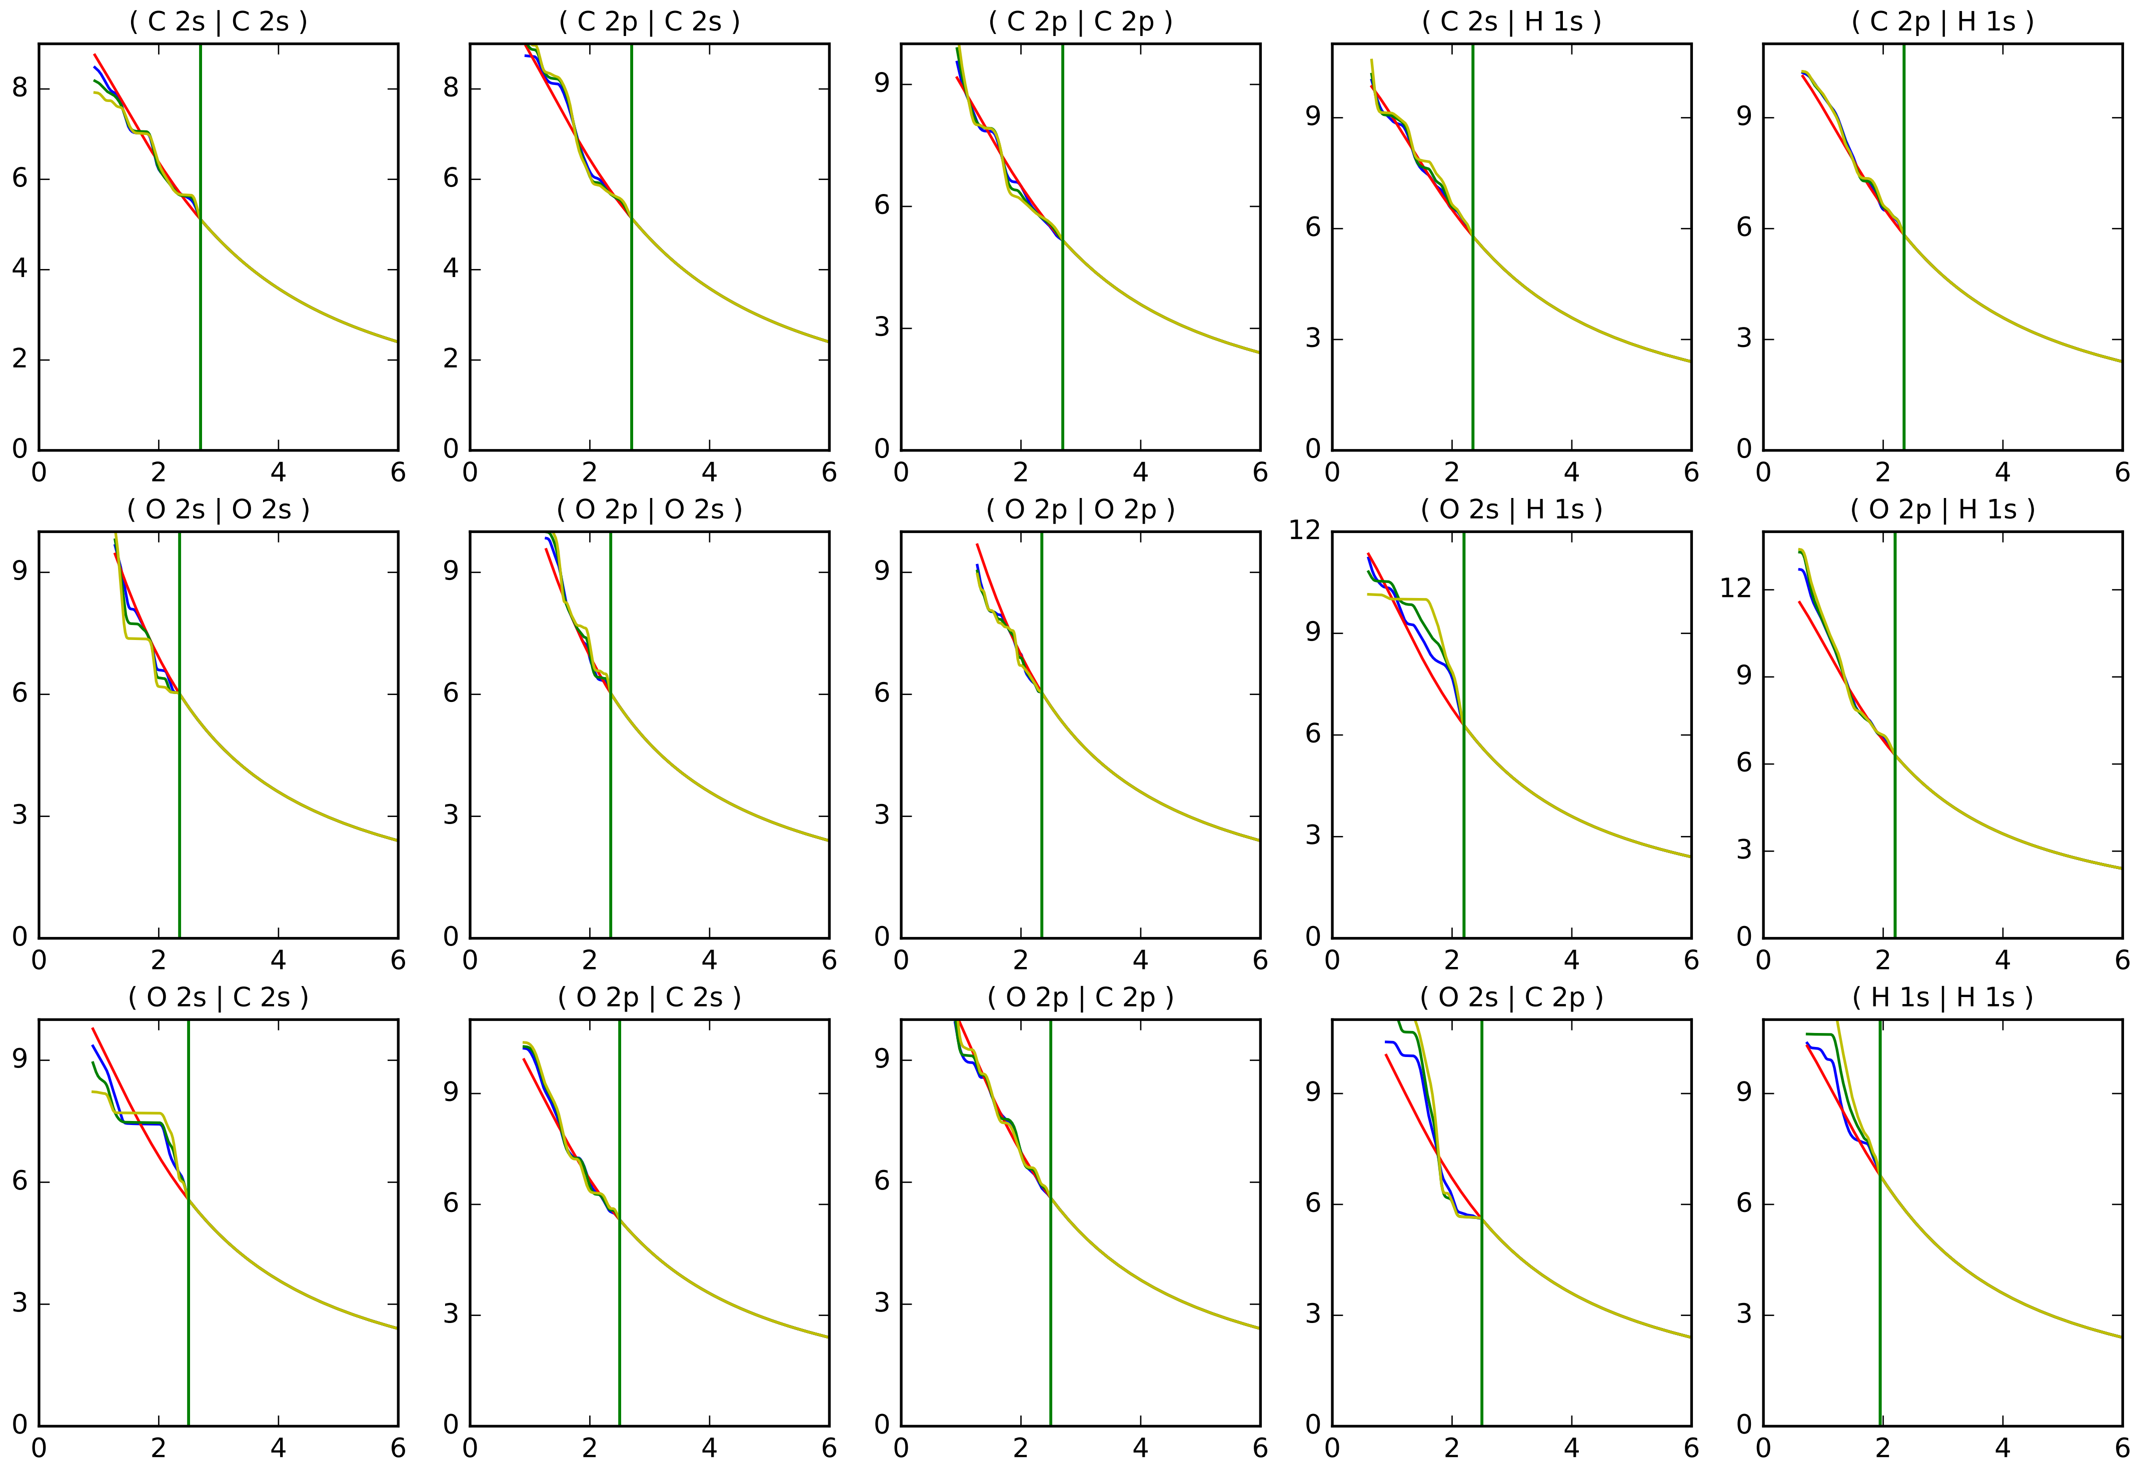

Figure S12: Spline models for R operator trained on molecules with up to 7 heavy atoms, with monotonic regurlarization.
Red: Initial Blue: Epoch 120 Green: Epoch 250 Yellow: Epoch 540

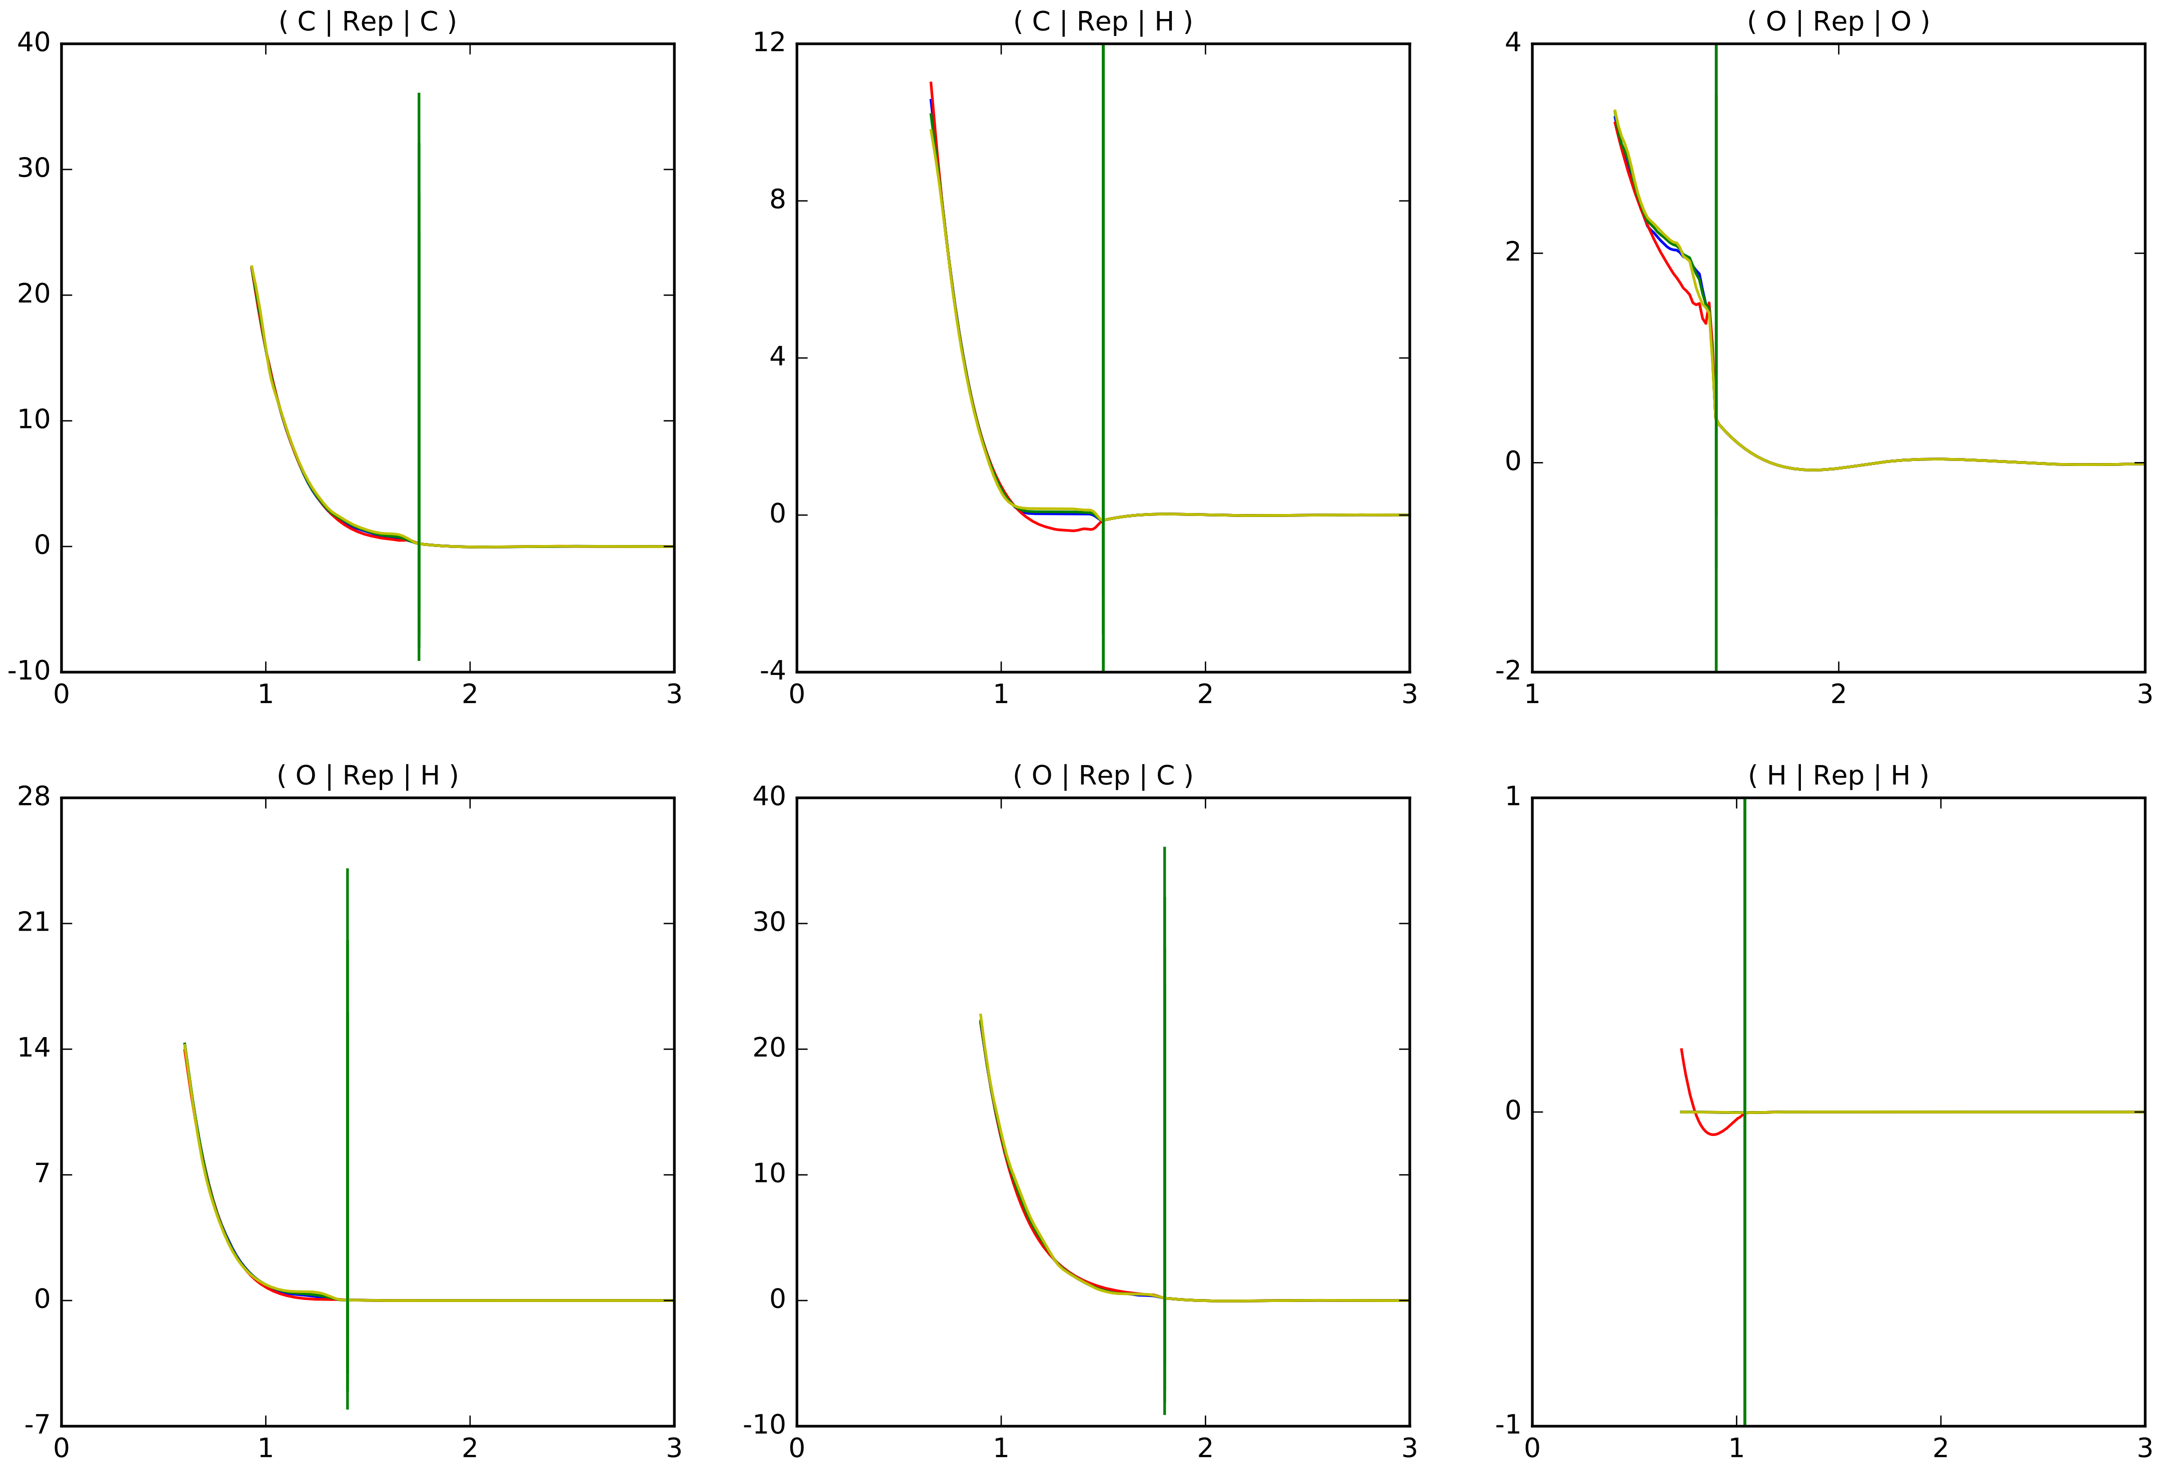

Figure S13: Spline models for H operator trained on molecules with up to 4 heavy atoms, with monotonic and DFTB regurlarization.
Red: Initial Blue: Epoch 290 Green: Epoch 410 Yellow: Epoch 540

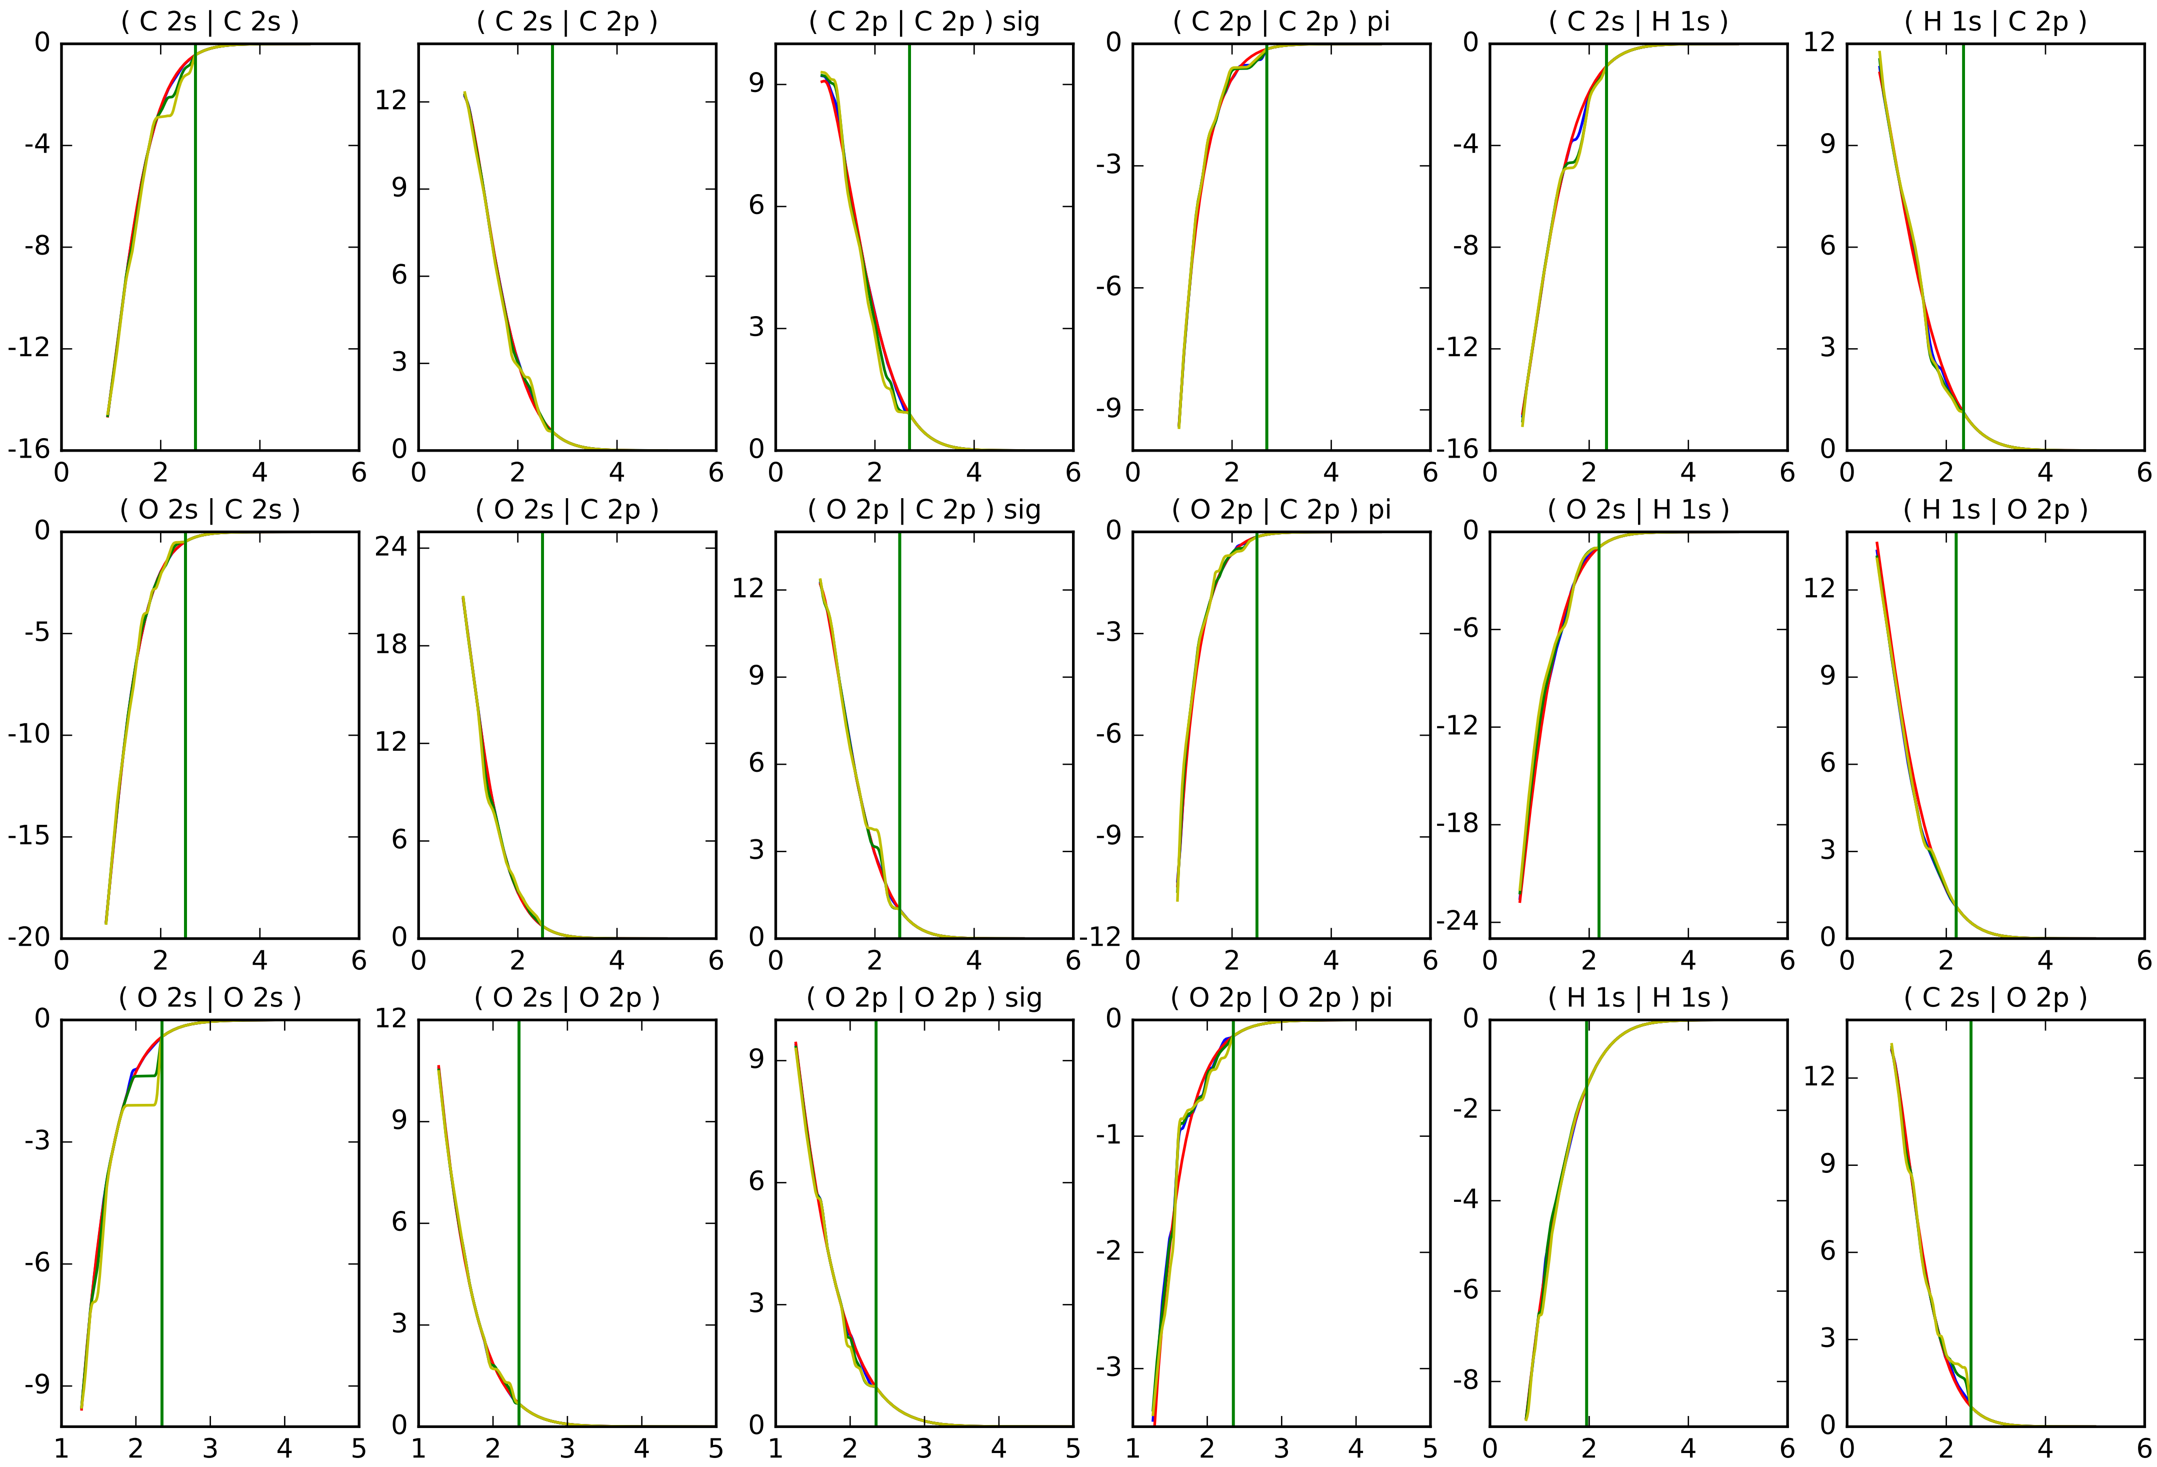

Figure S14: Spline models for G operator trained on molecules with up to 4 heavy atoms, with monotonic and DFTB regurlarization.
Red: Initial Blue: Epoch 290 Green: Epoch 410 Yellow: Epoch 540

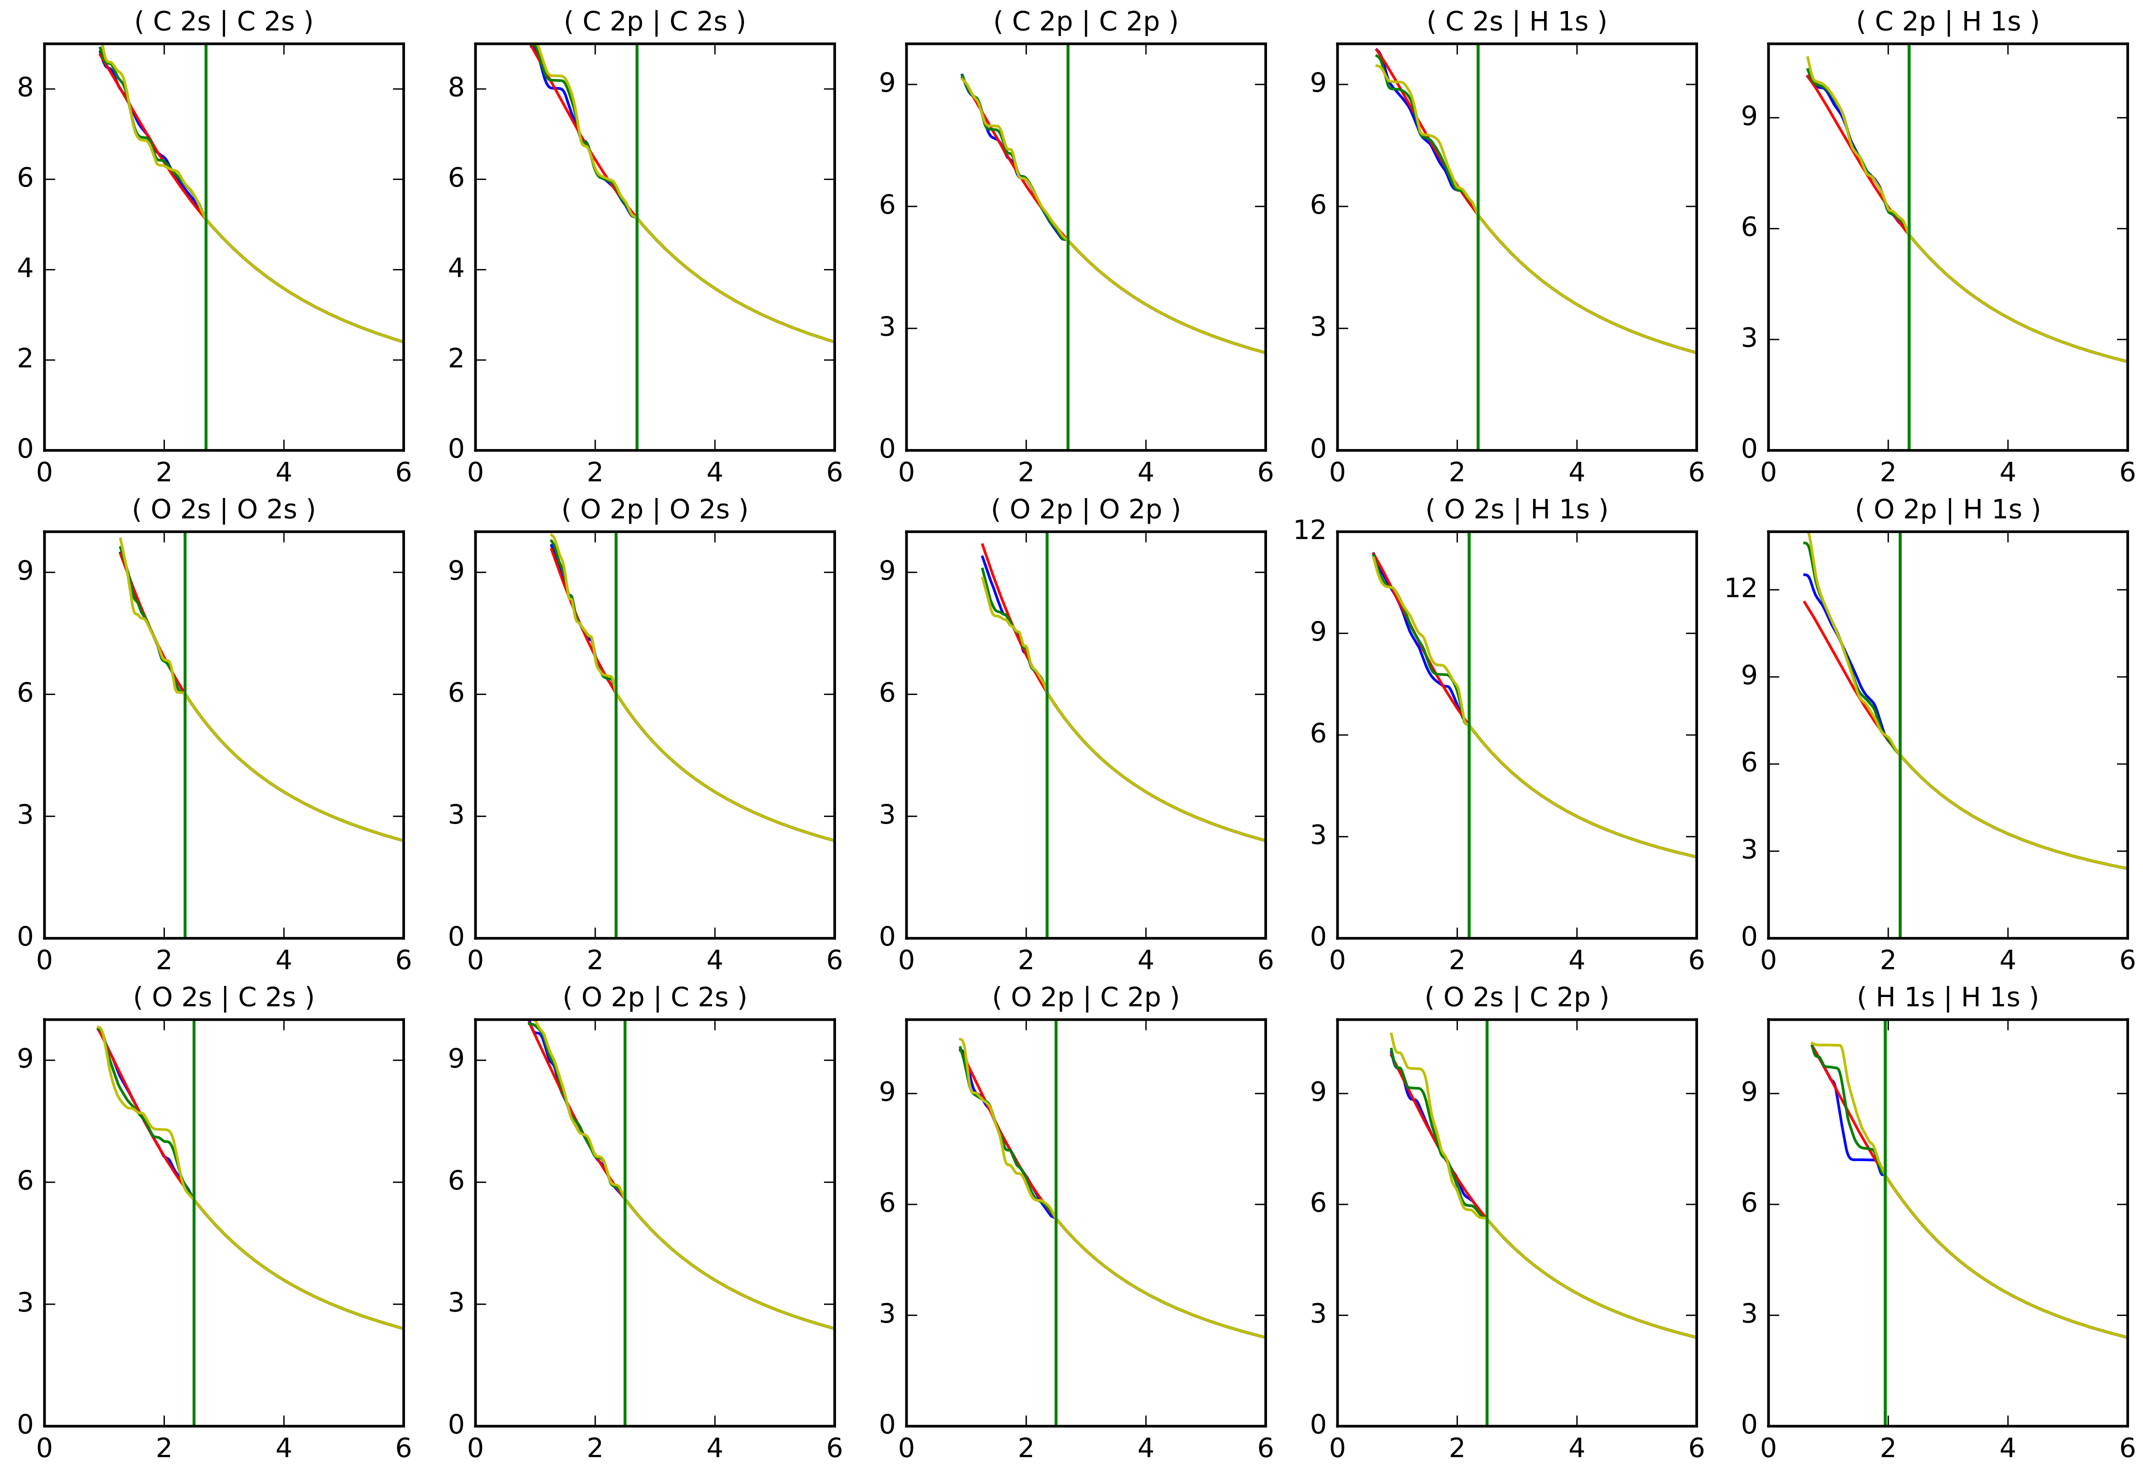

Figure S15: Spline models for R operator trained on molecules with up to 4 heavy atoms, with monotonic and DFTB regurlarization.
Red: Initial Blue: Epoch 290 Green: Epoch 410 Yellow: Epoch 540

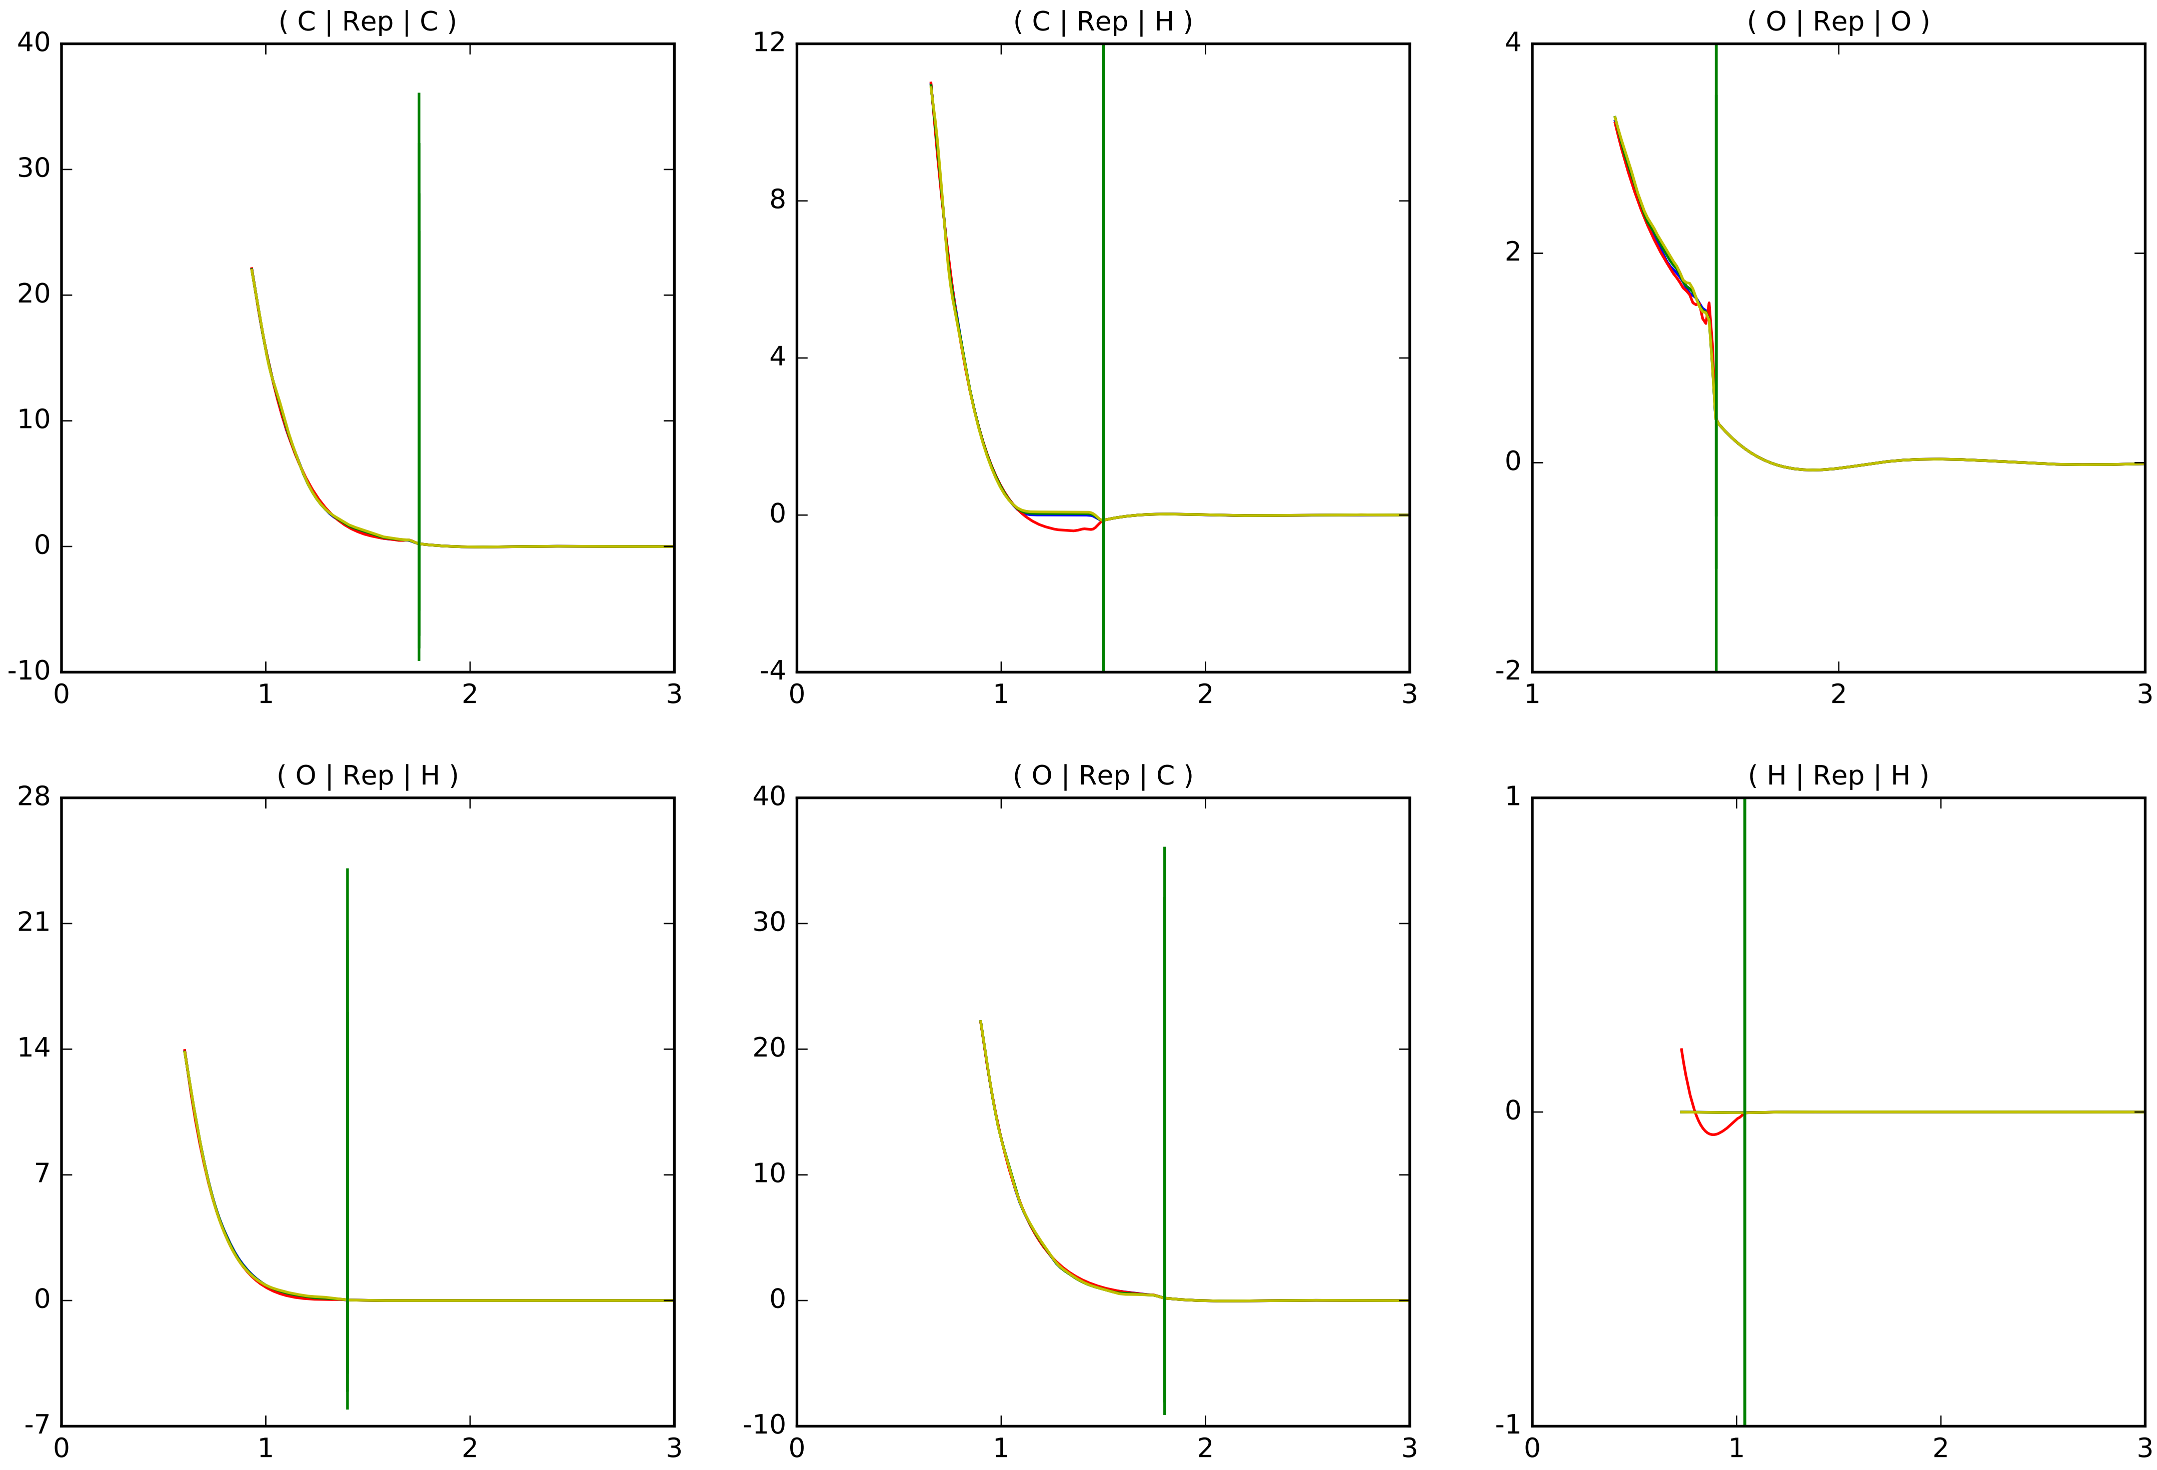

Figure S16: Spline models for H operator trained on molecules with up to 7 heavy atoms, with monotonic and DFTB regurlarization.
Red: Initial Blue: Epoch 290 Green: Epoch 410 Yellow: Epoch 540

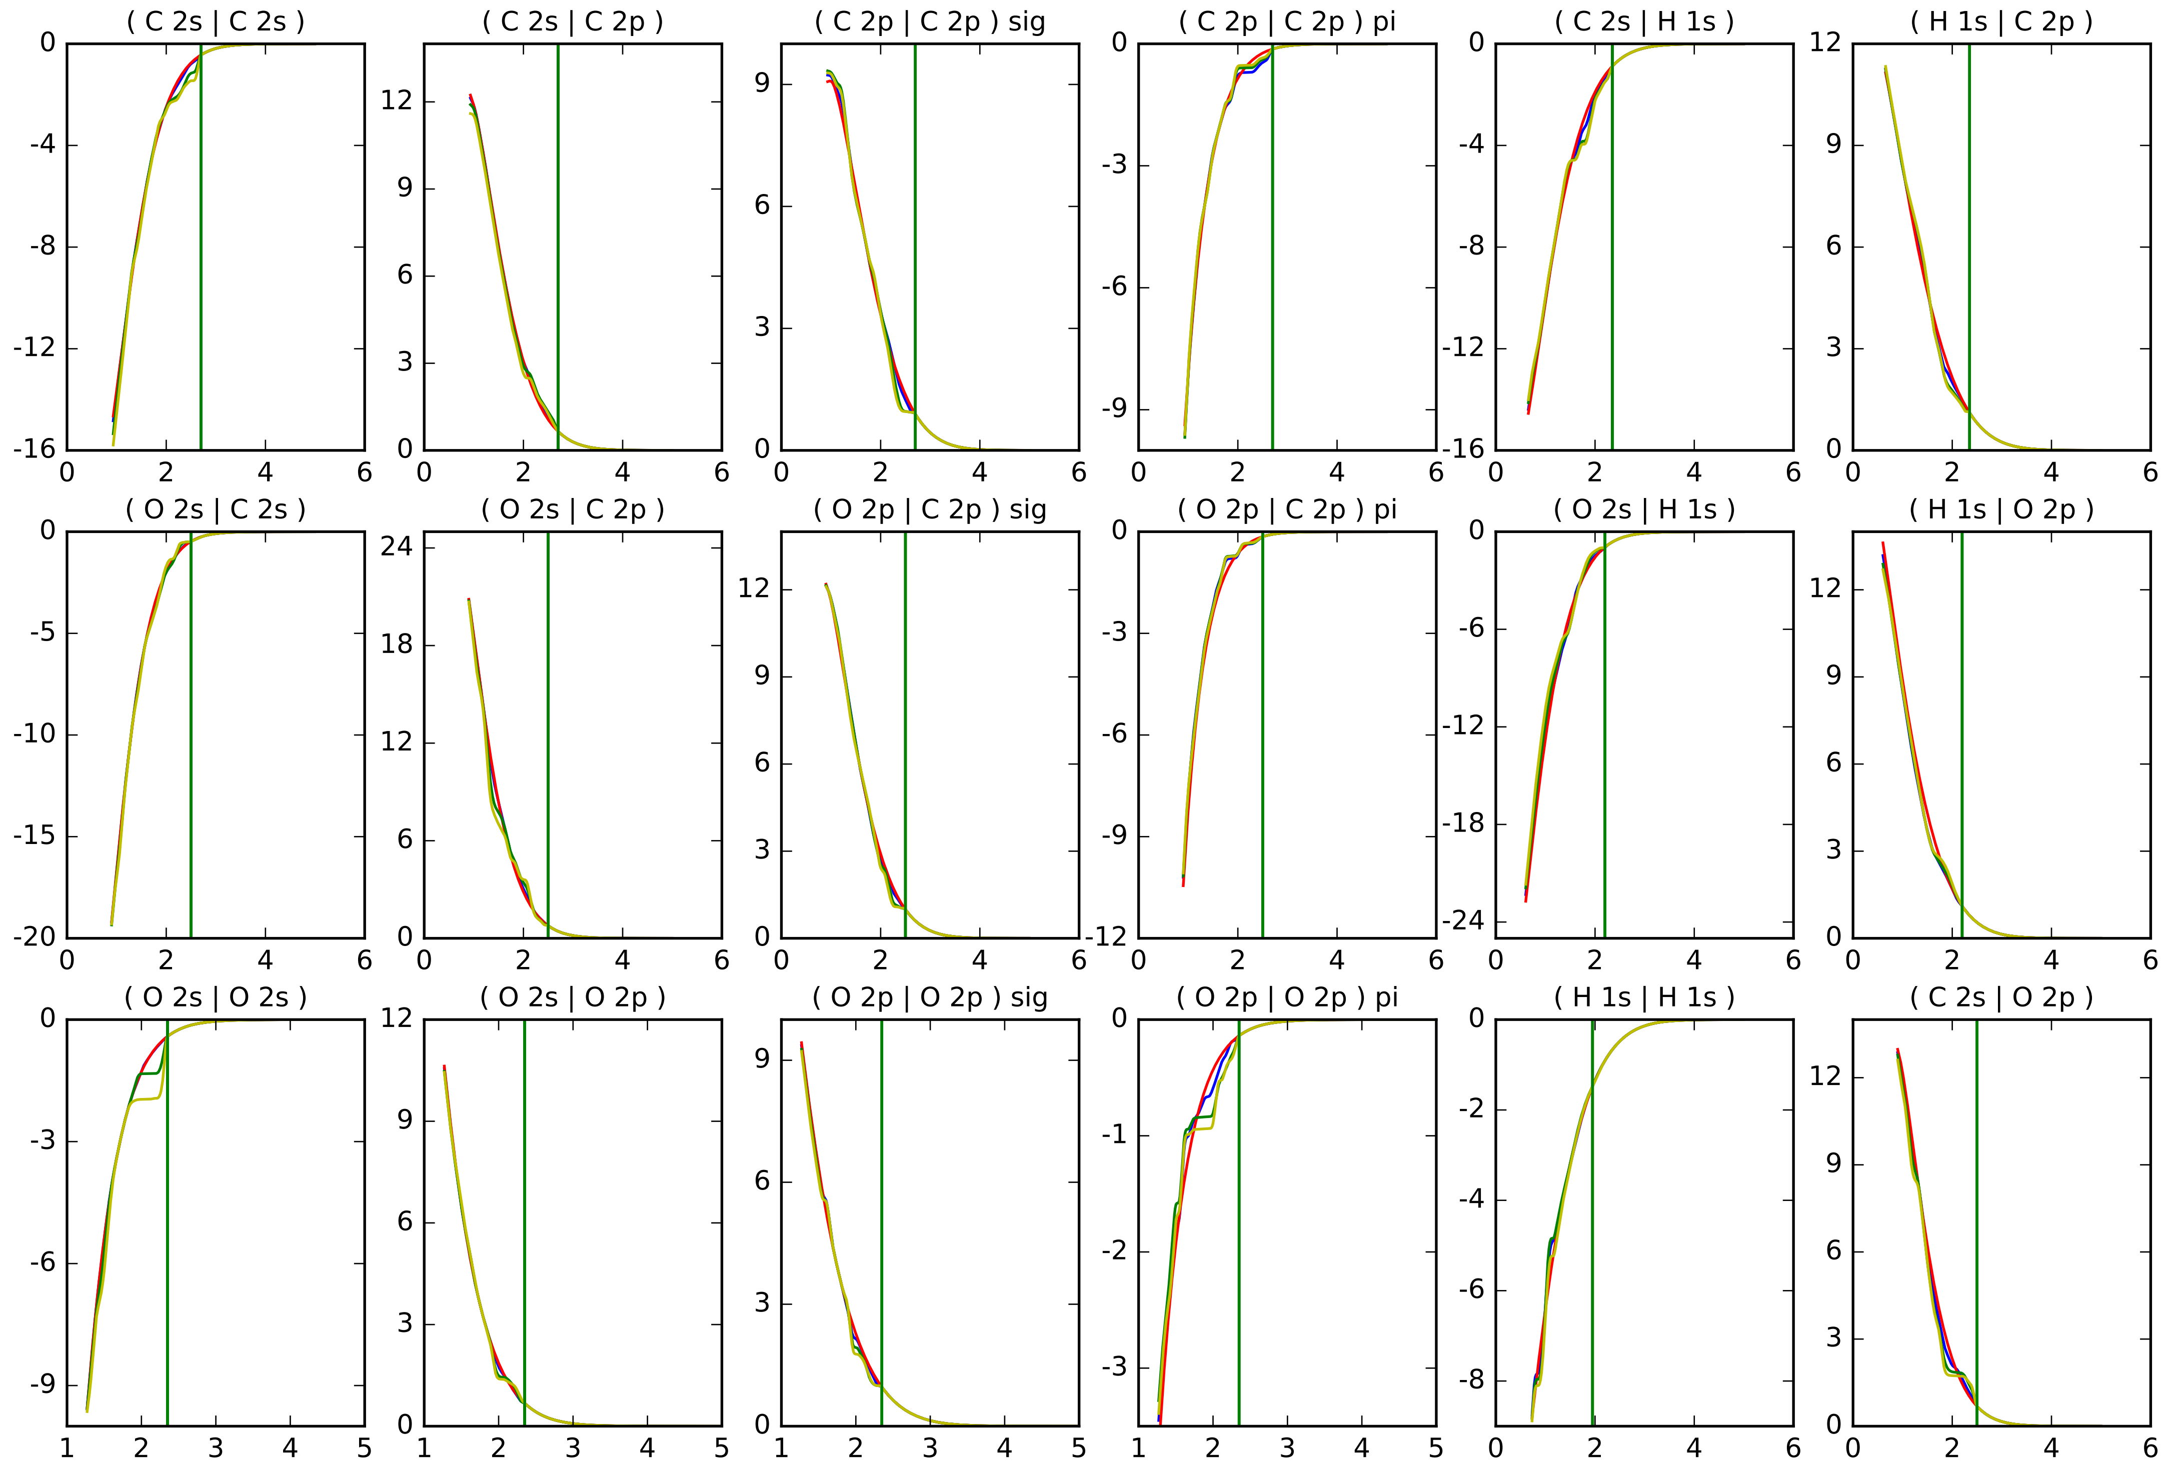

Figure S17: Spline models for G operator trained on molecules with up to 7 heavy atoms, with monotonic and DFTB regurlarization.
Red: Initial Blue: Epoch 290 Green: Epoch 410 Yellow: Epoch 540

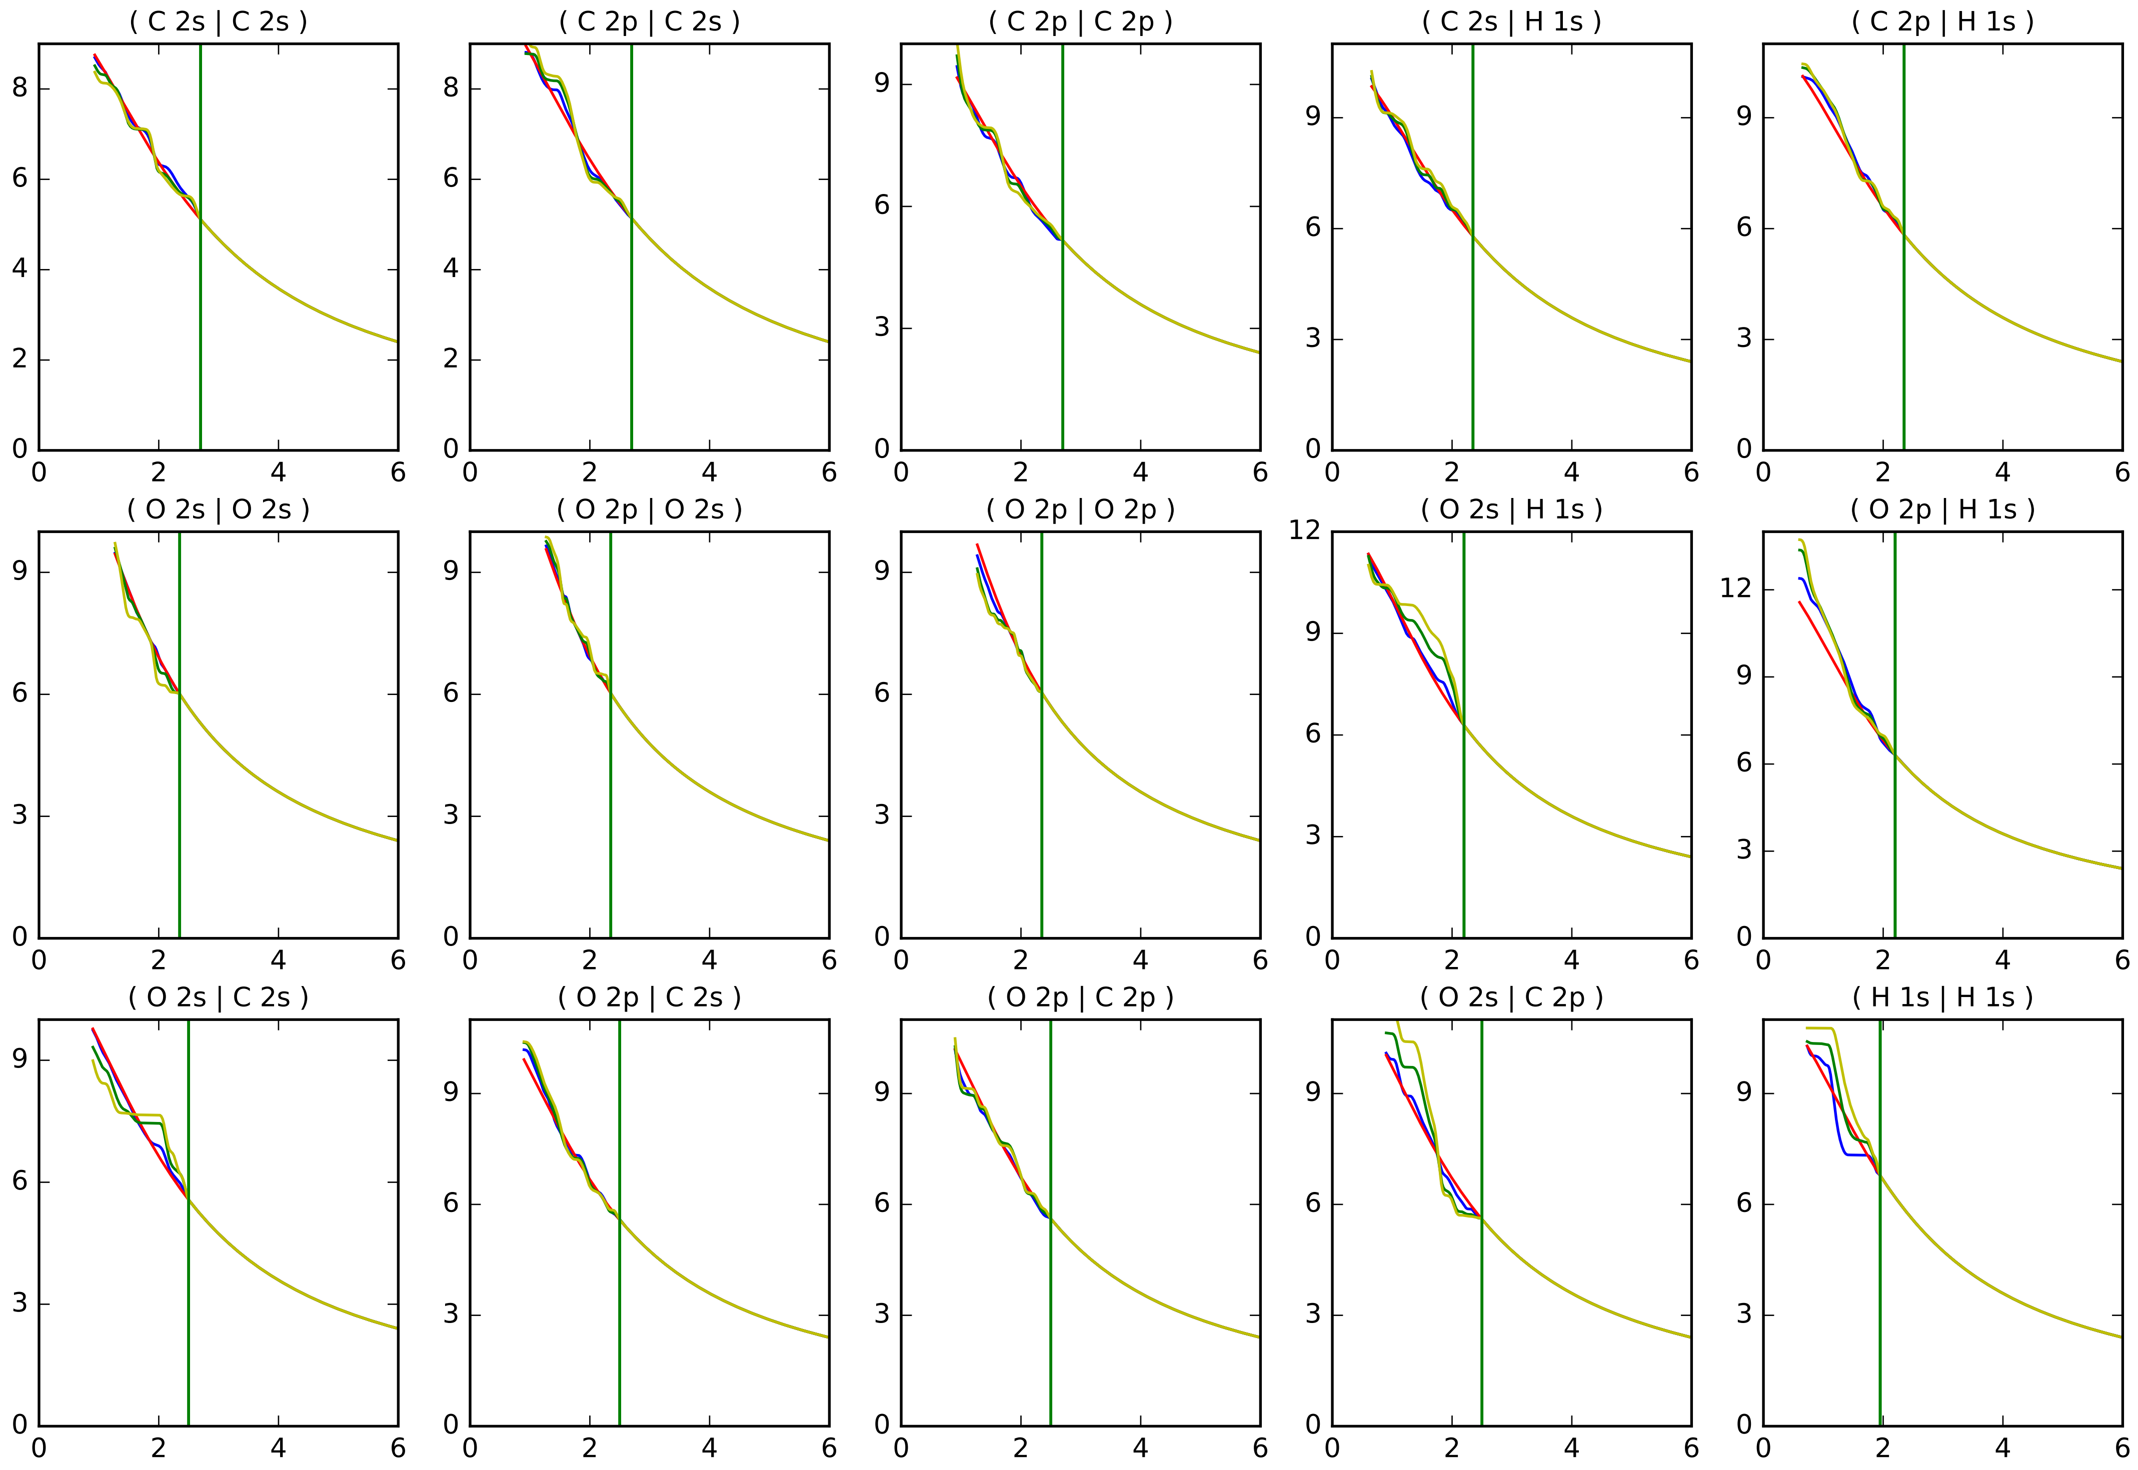

Figure S18: Spline models for R operator trained on molecules with up to 7 heavy atoms, with monotonic and DFTB regurlarization.
Red: Initial Blue: Epoch 290 Green: Epoch 410 Yellow: Epoch 540

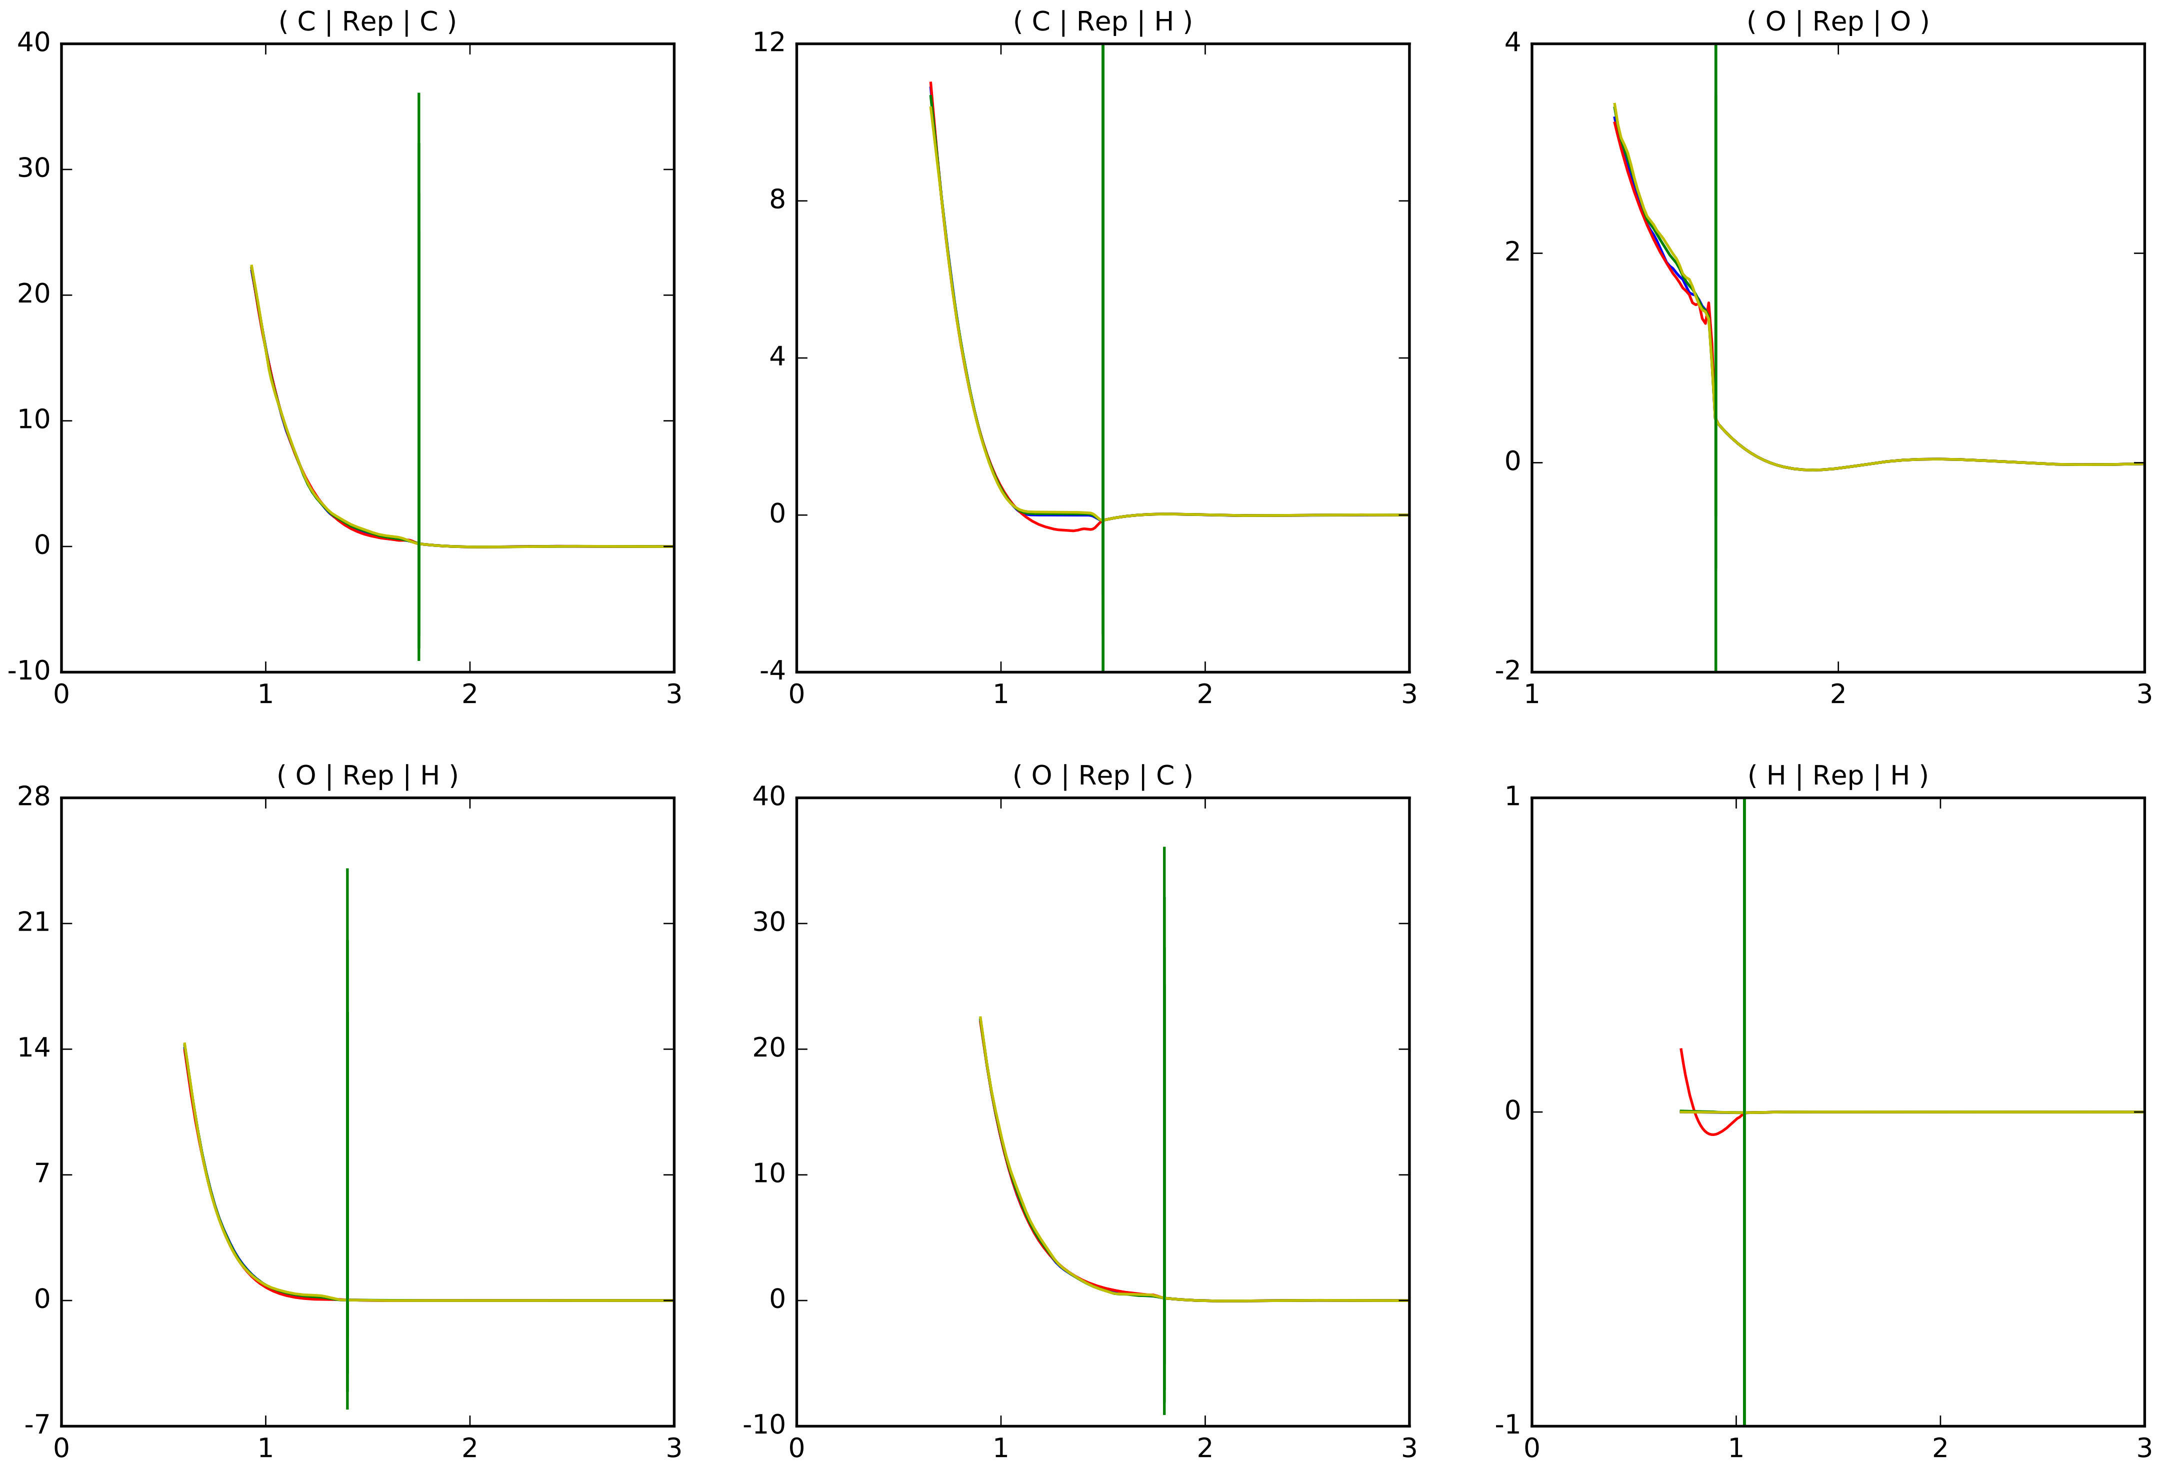

Supplement: Supplementary file 1 [file models_SI.pdf]
