# Supplementary material for: A Density Functional Tight Binding Layer for Deep Learning of Chemical Hamiltonians
Source: arXiv:1808.04526 source file (2018-08-20)

Figure S19 H Diag: Single Variable H Off Diag: Spline
G Diag: Single Variable G Off Diag: Spline Repulsive: Spline

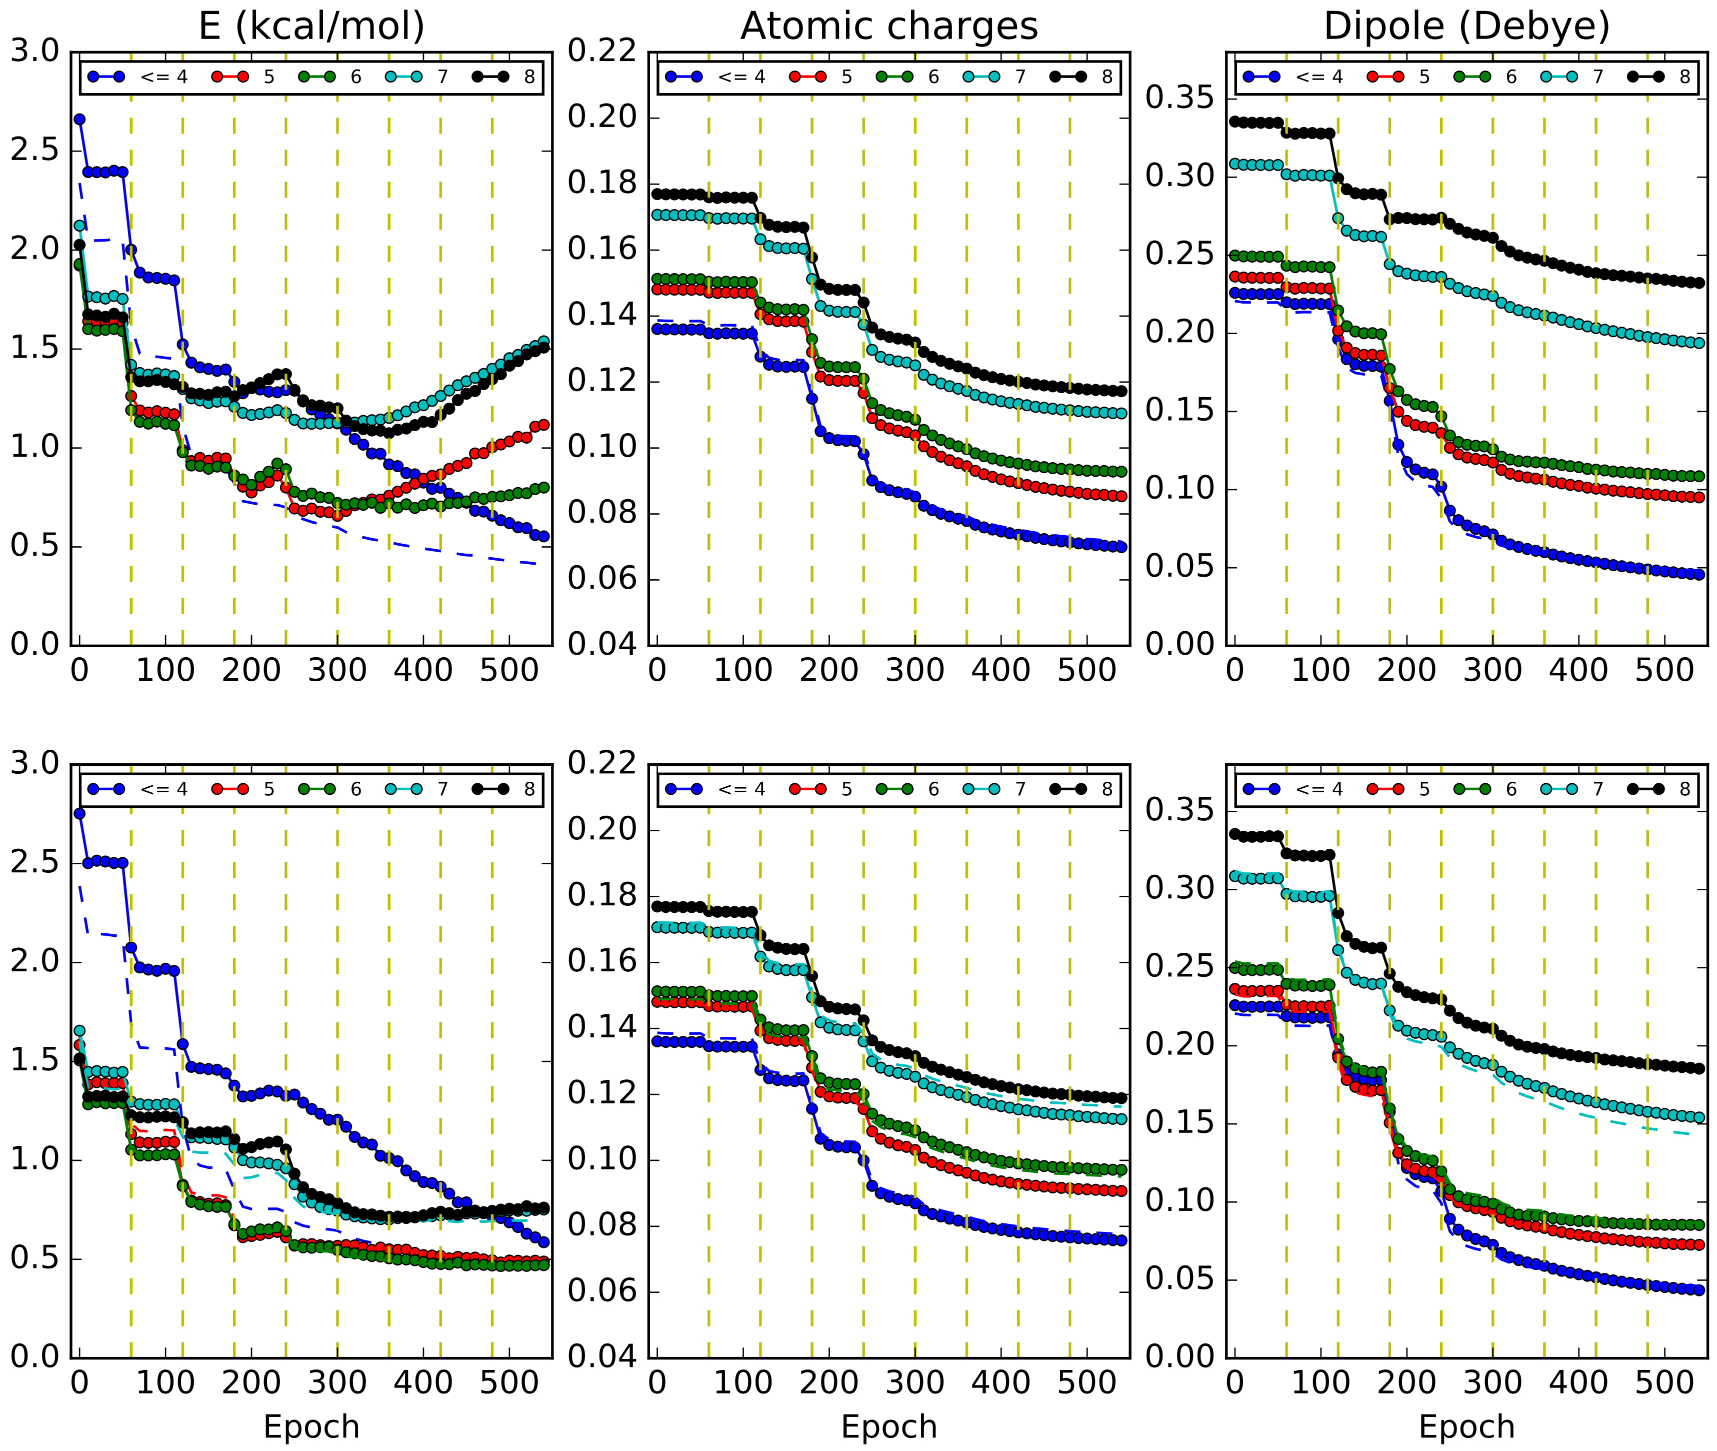

Figure S20 H Diag: Single Variable H Off Diag: DFTB MIO
G Diag: Single Variable G Off Diag: DFTB MIO Repulsive: Spline

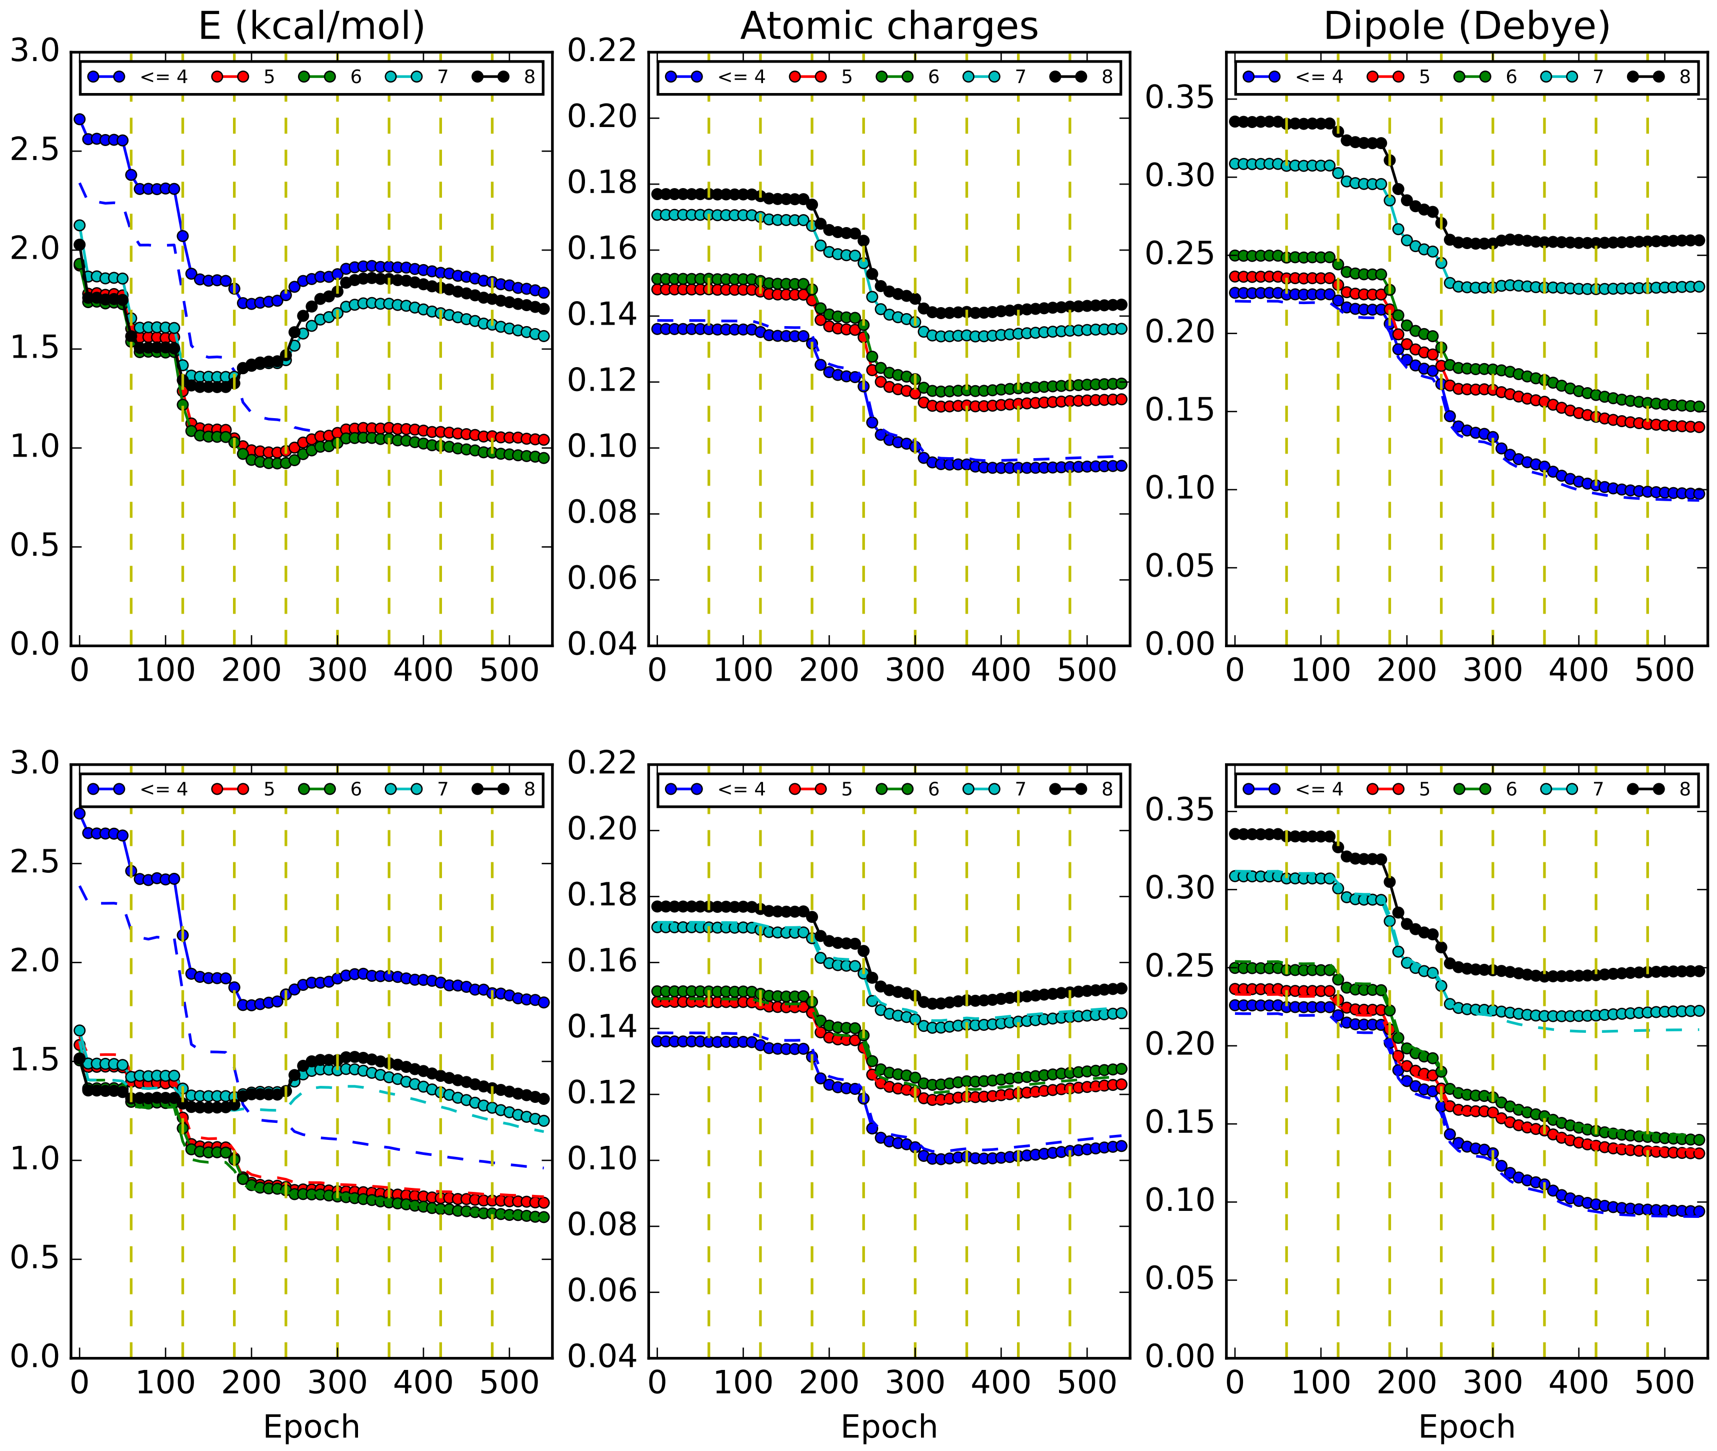

Figure S21 H Diag: DFTB MIO H Off Diag: Spline
G Diag: DFTB MIO G Off Diag: Spline Repulsive: Spline

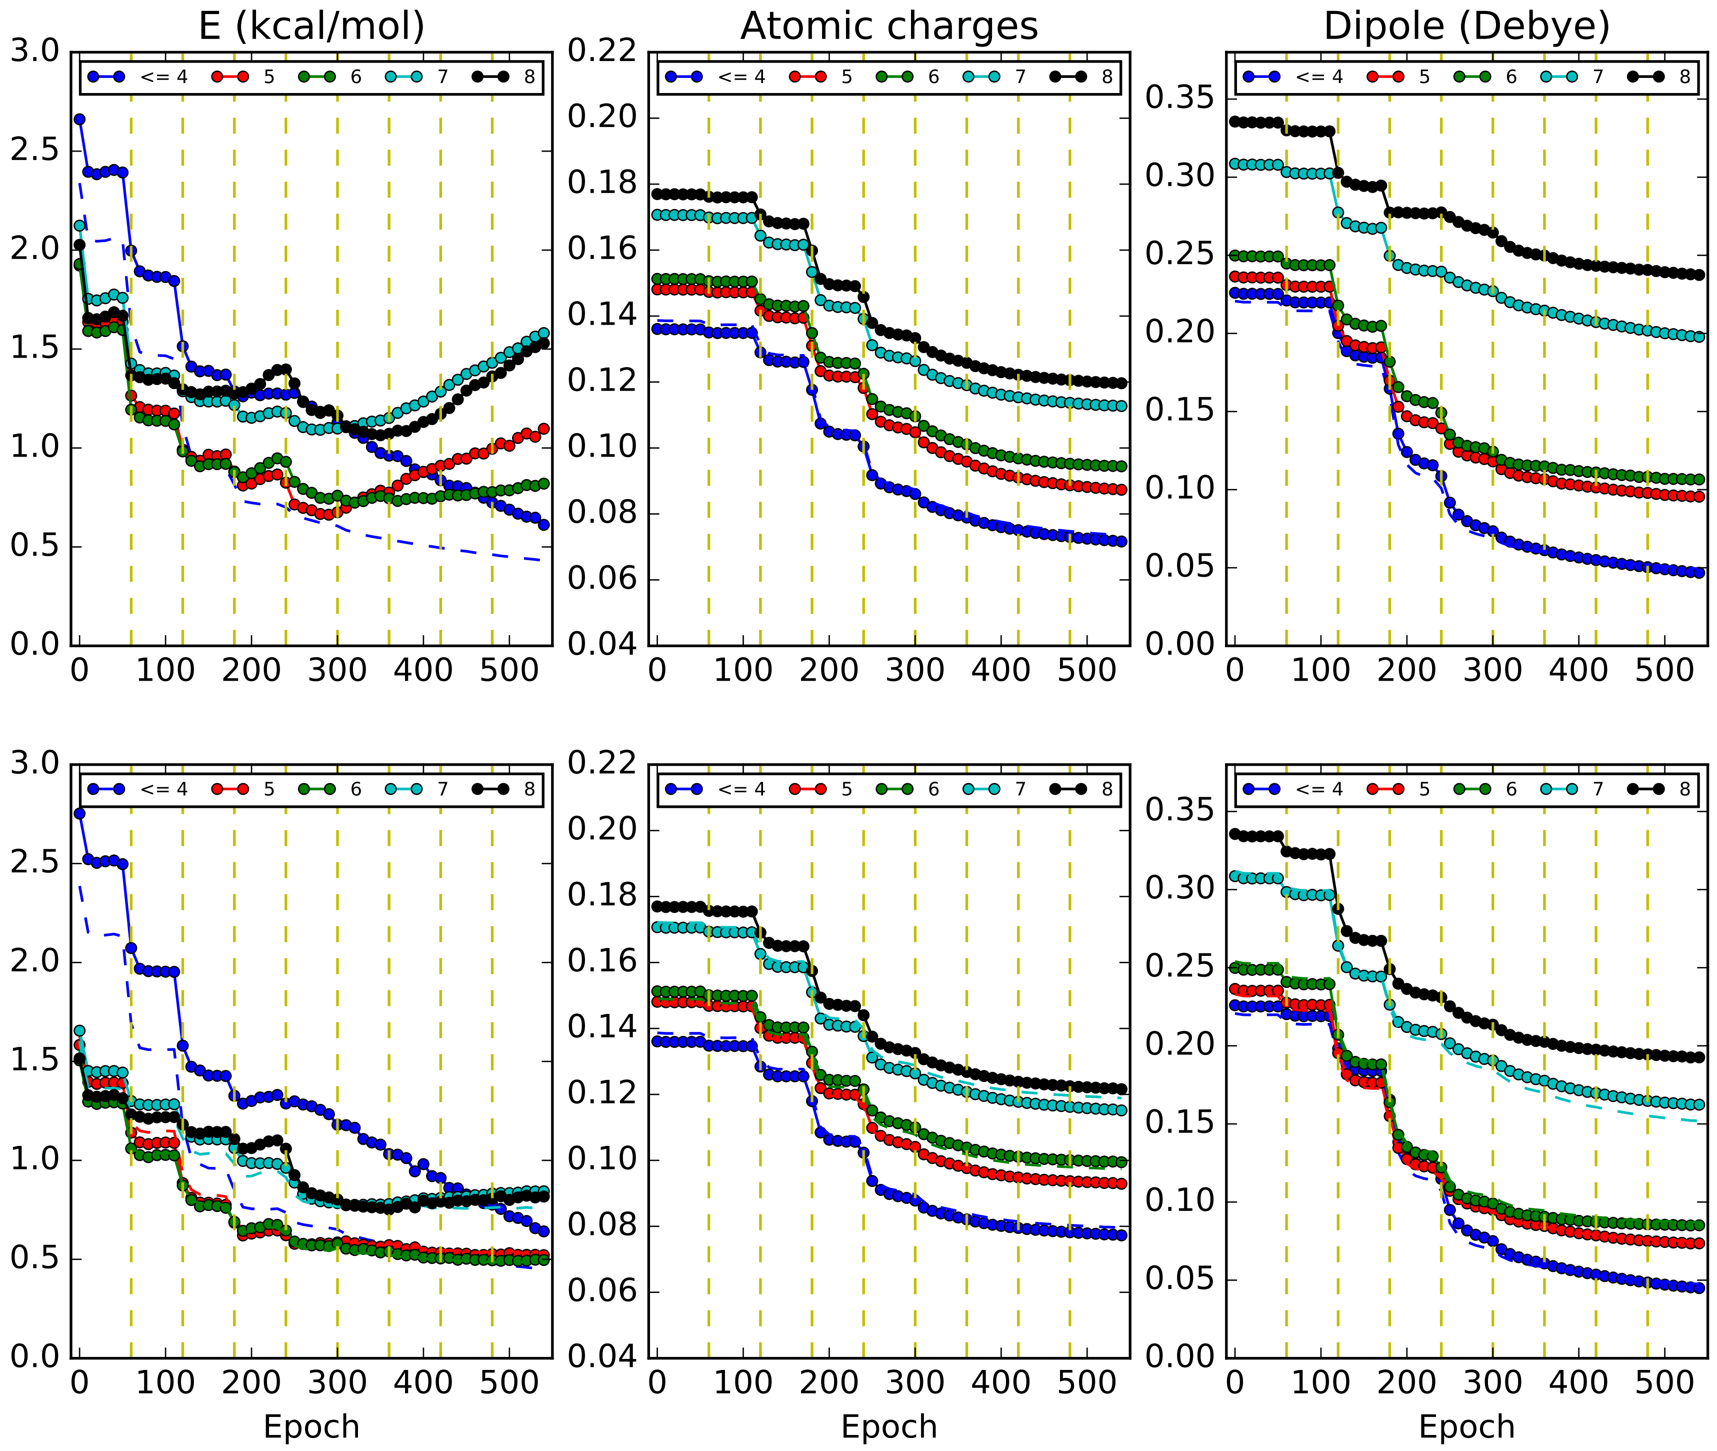

Figure S22 H Diag: DFTB MIO H Off Diag: Spline
G Diag: Single Variable G Off Diag: Spline Repulsive: Spline

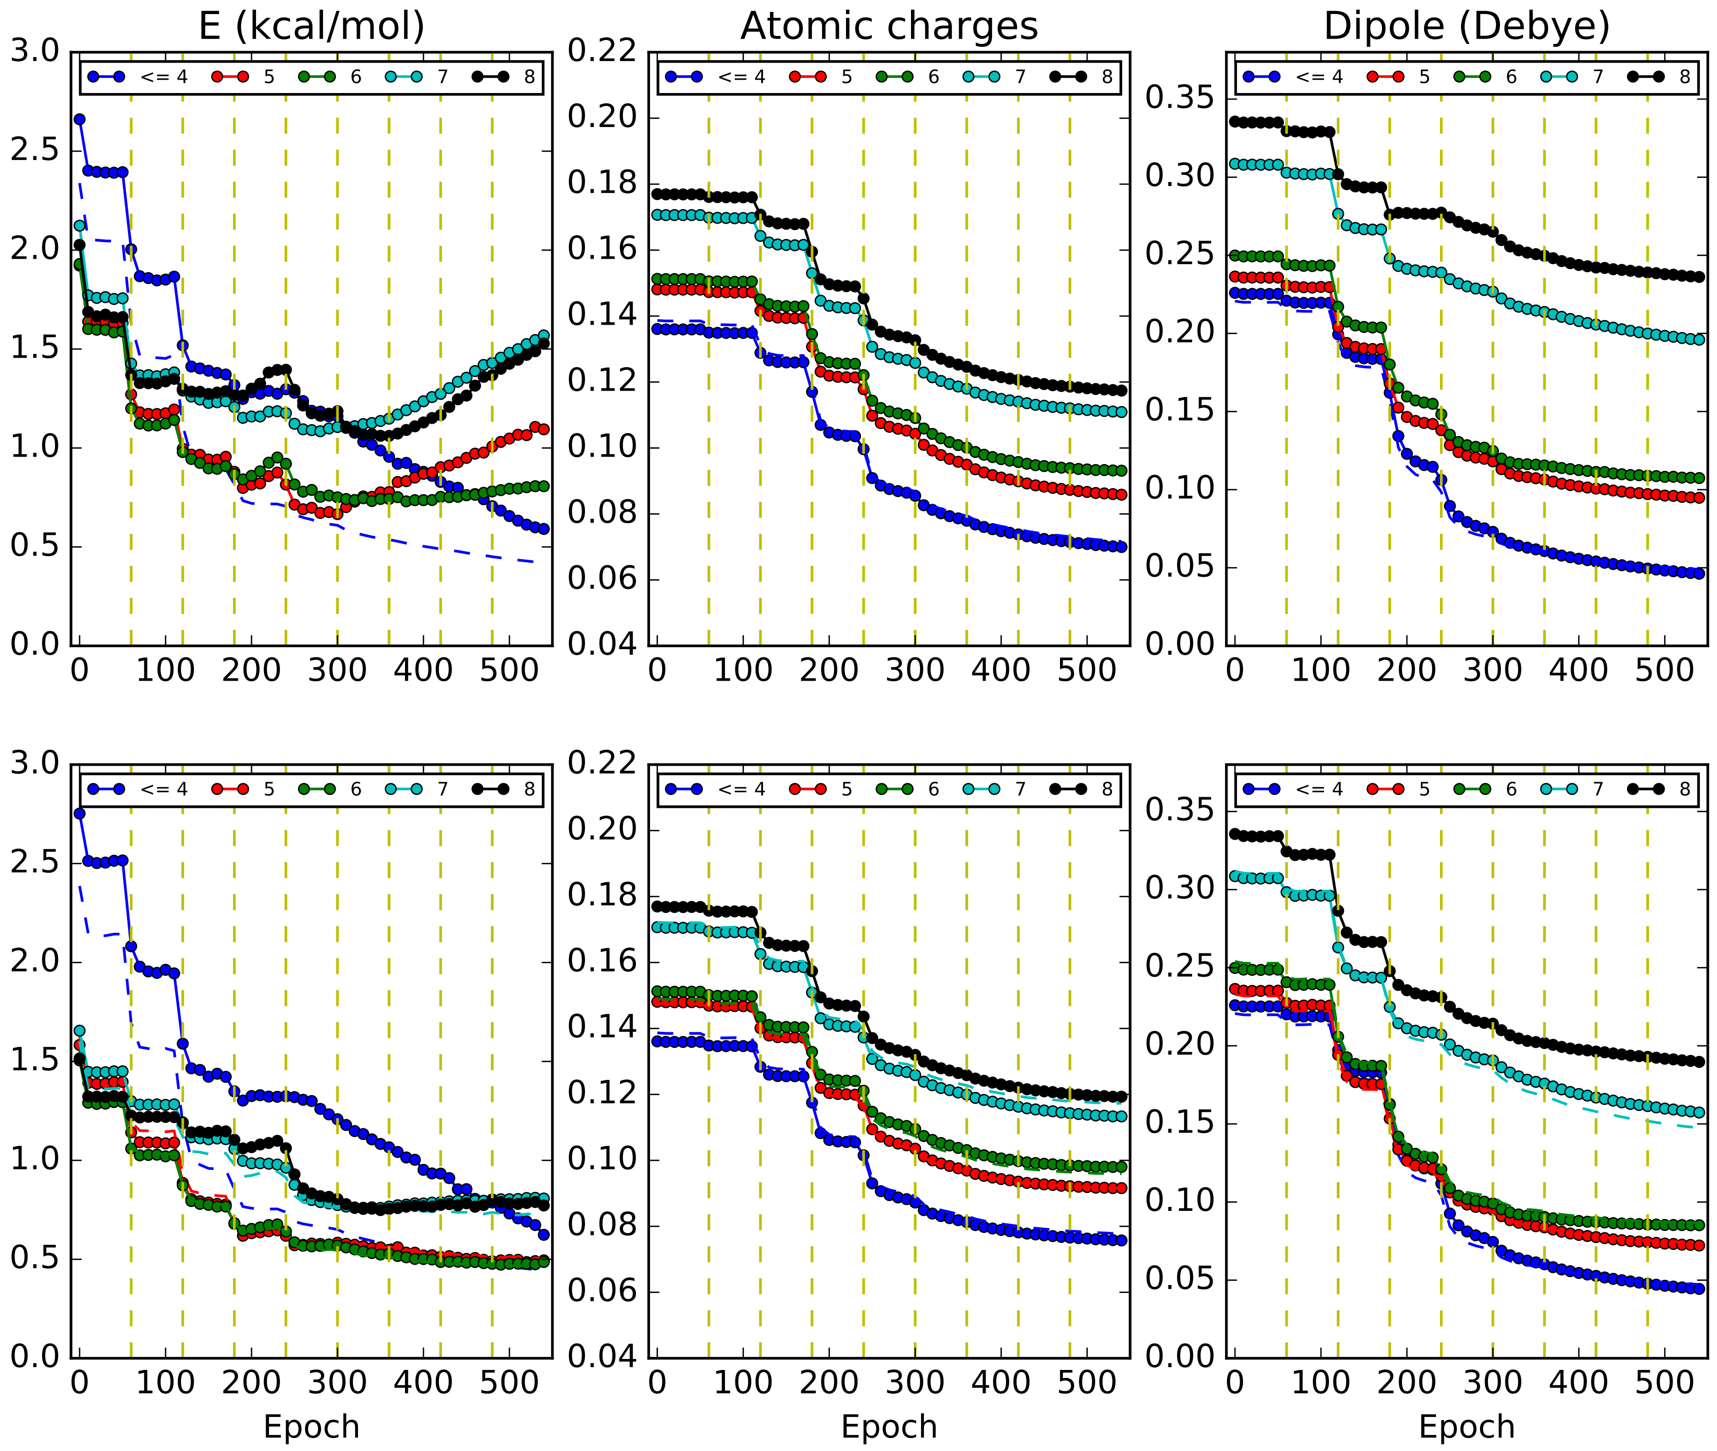

Figure S23 H Diag: Single Variable H Off Diag: DFTB MIO
G Diag: Single Variable G Off Diag: Spline Repulsive: Spline

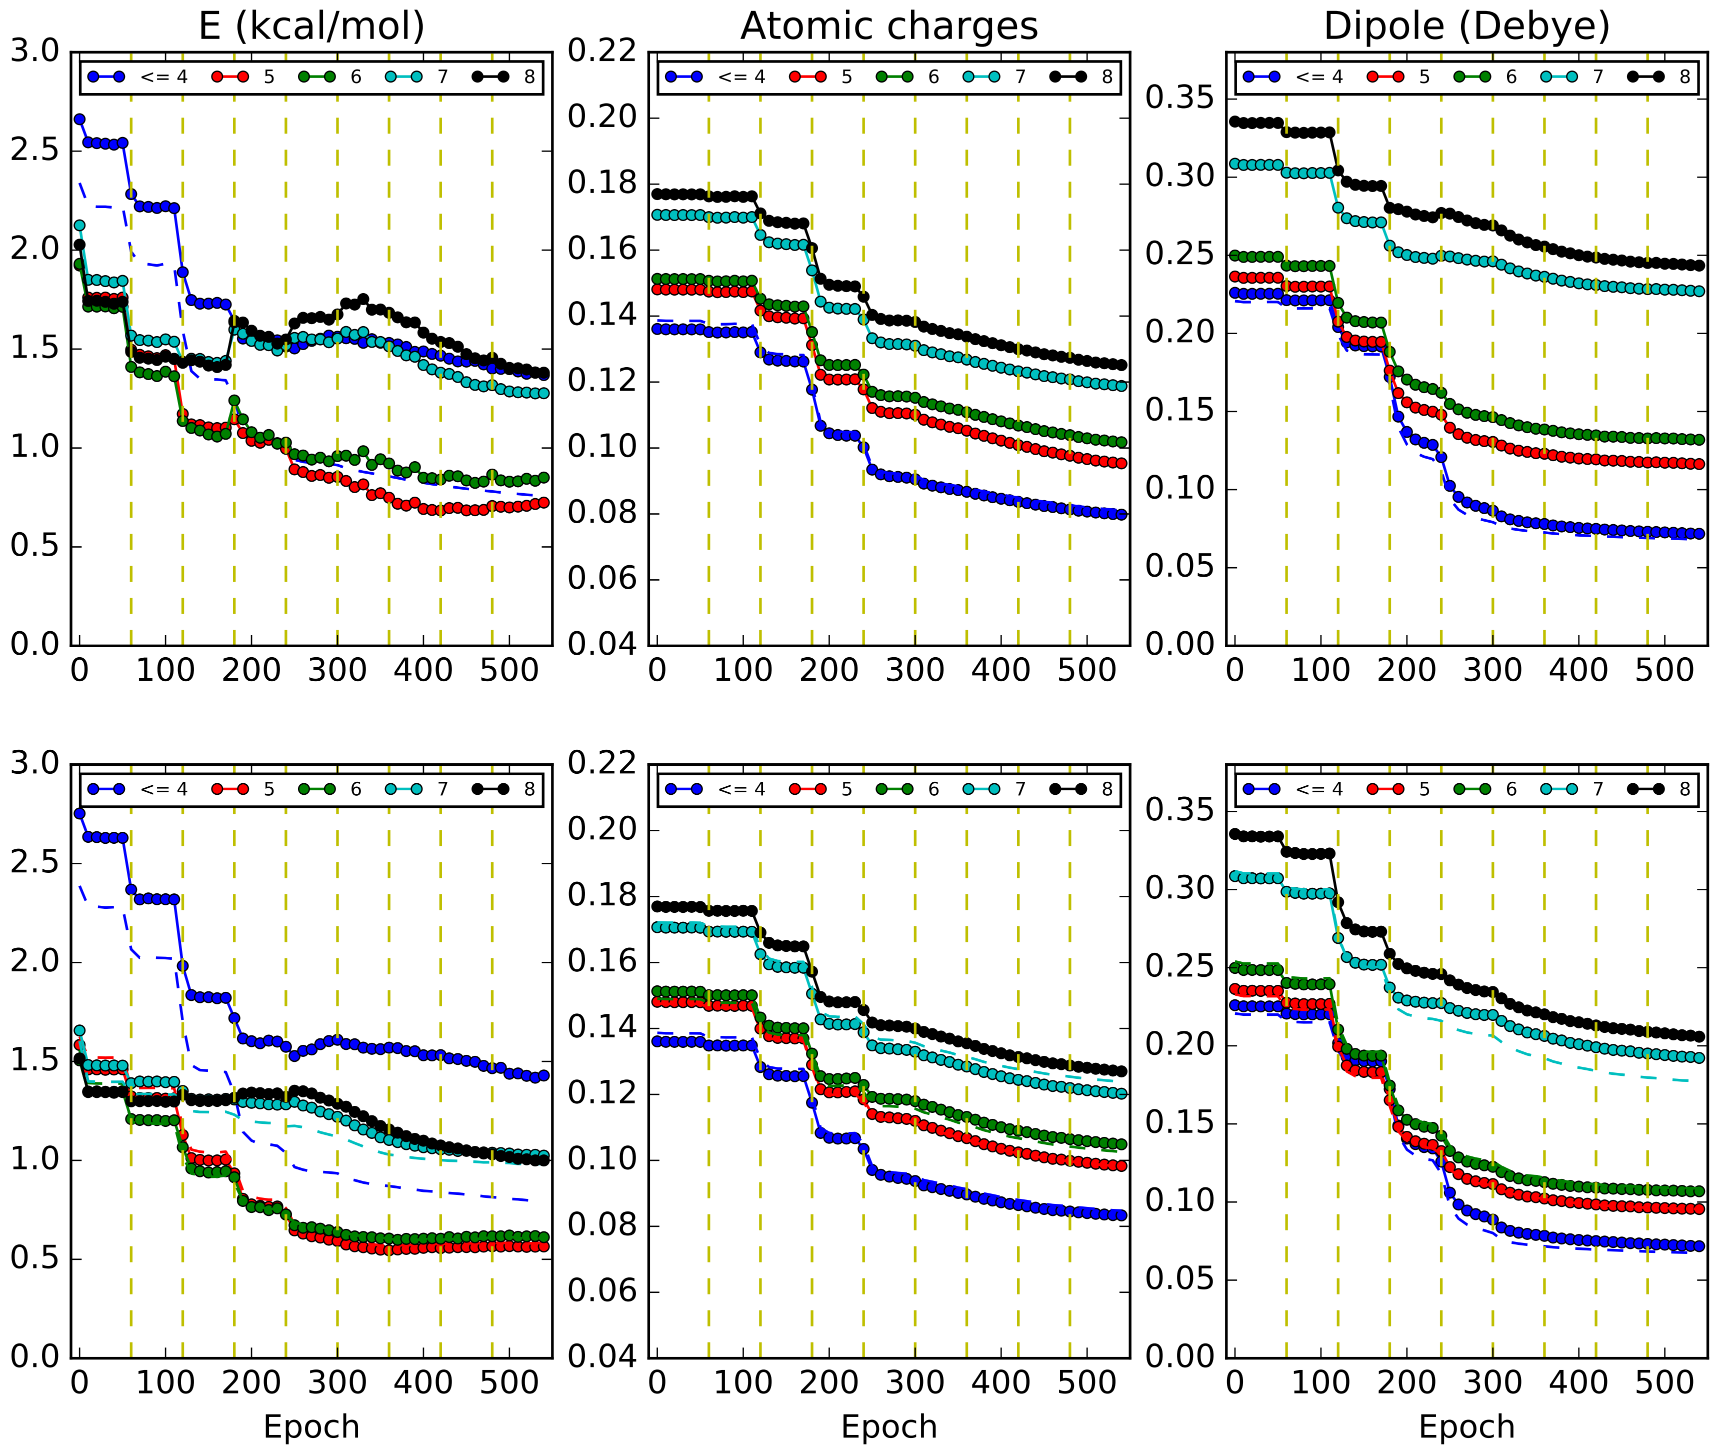

Figure S24 H Diag: Single Variable H Off Diag: Spline
G Diag: DFTB MIO G Off Diag: Spline Repulsive: Spline

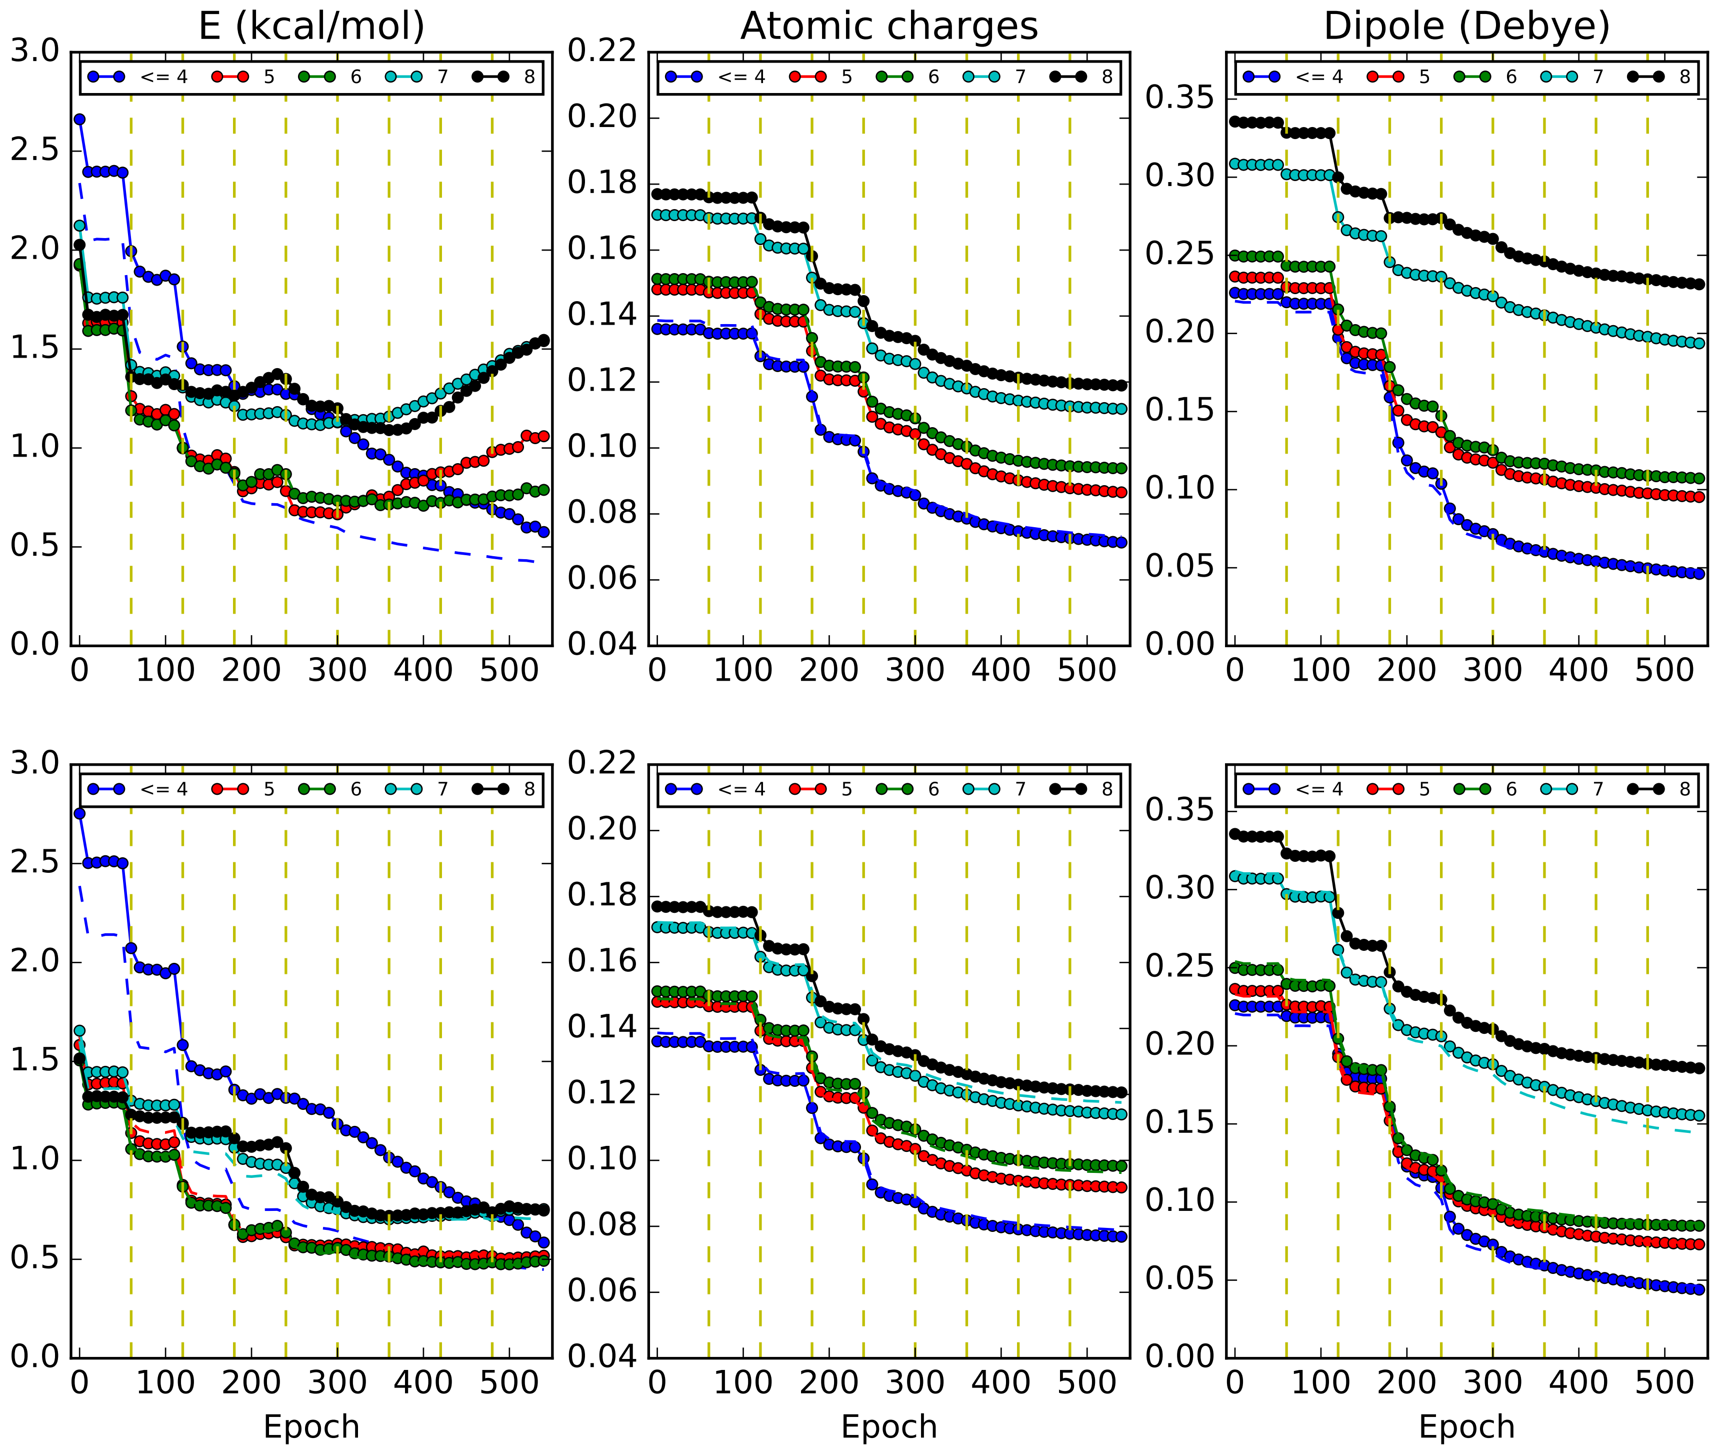

Figure S25 H Diag: Single Variable H Off Diag: Spline
G Diag: Single Variable G Off Diag: DFTB MIO Repulsive: Spline

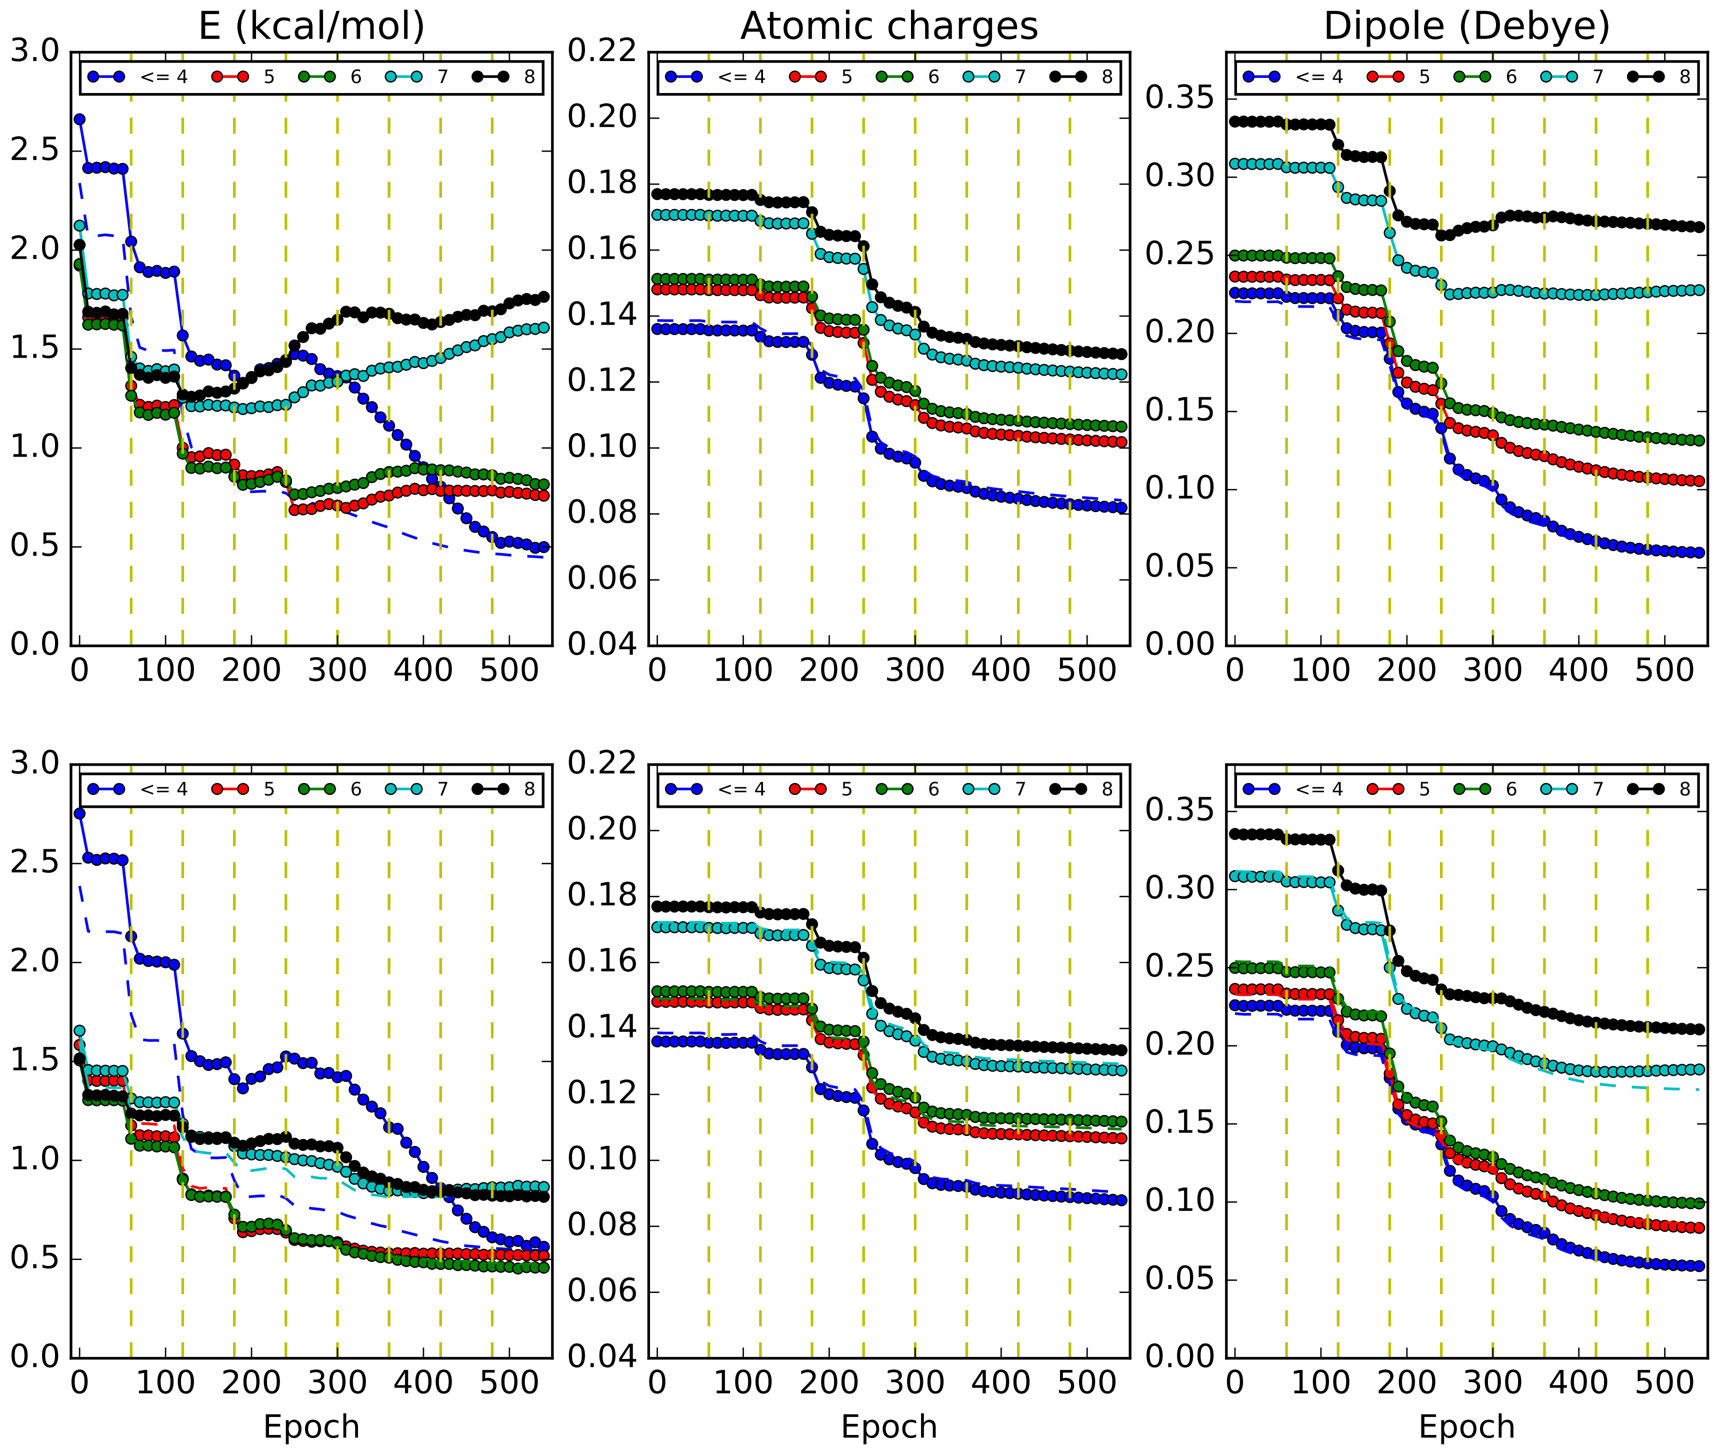

Figure S26 H Diag: Single Variable H Off Diag: Spline
G Diag: Single Variable G Off Diag: Spline Repulsive: DFTB MIO

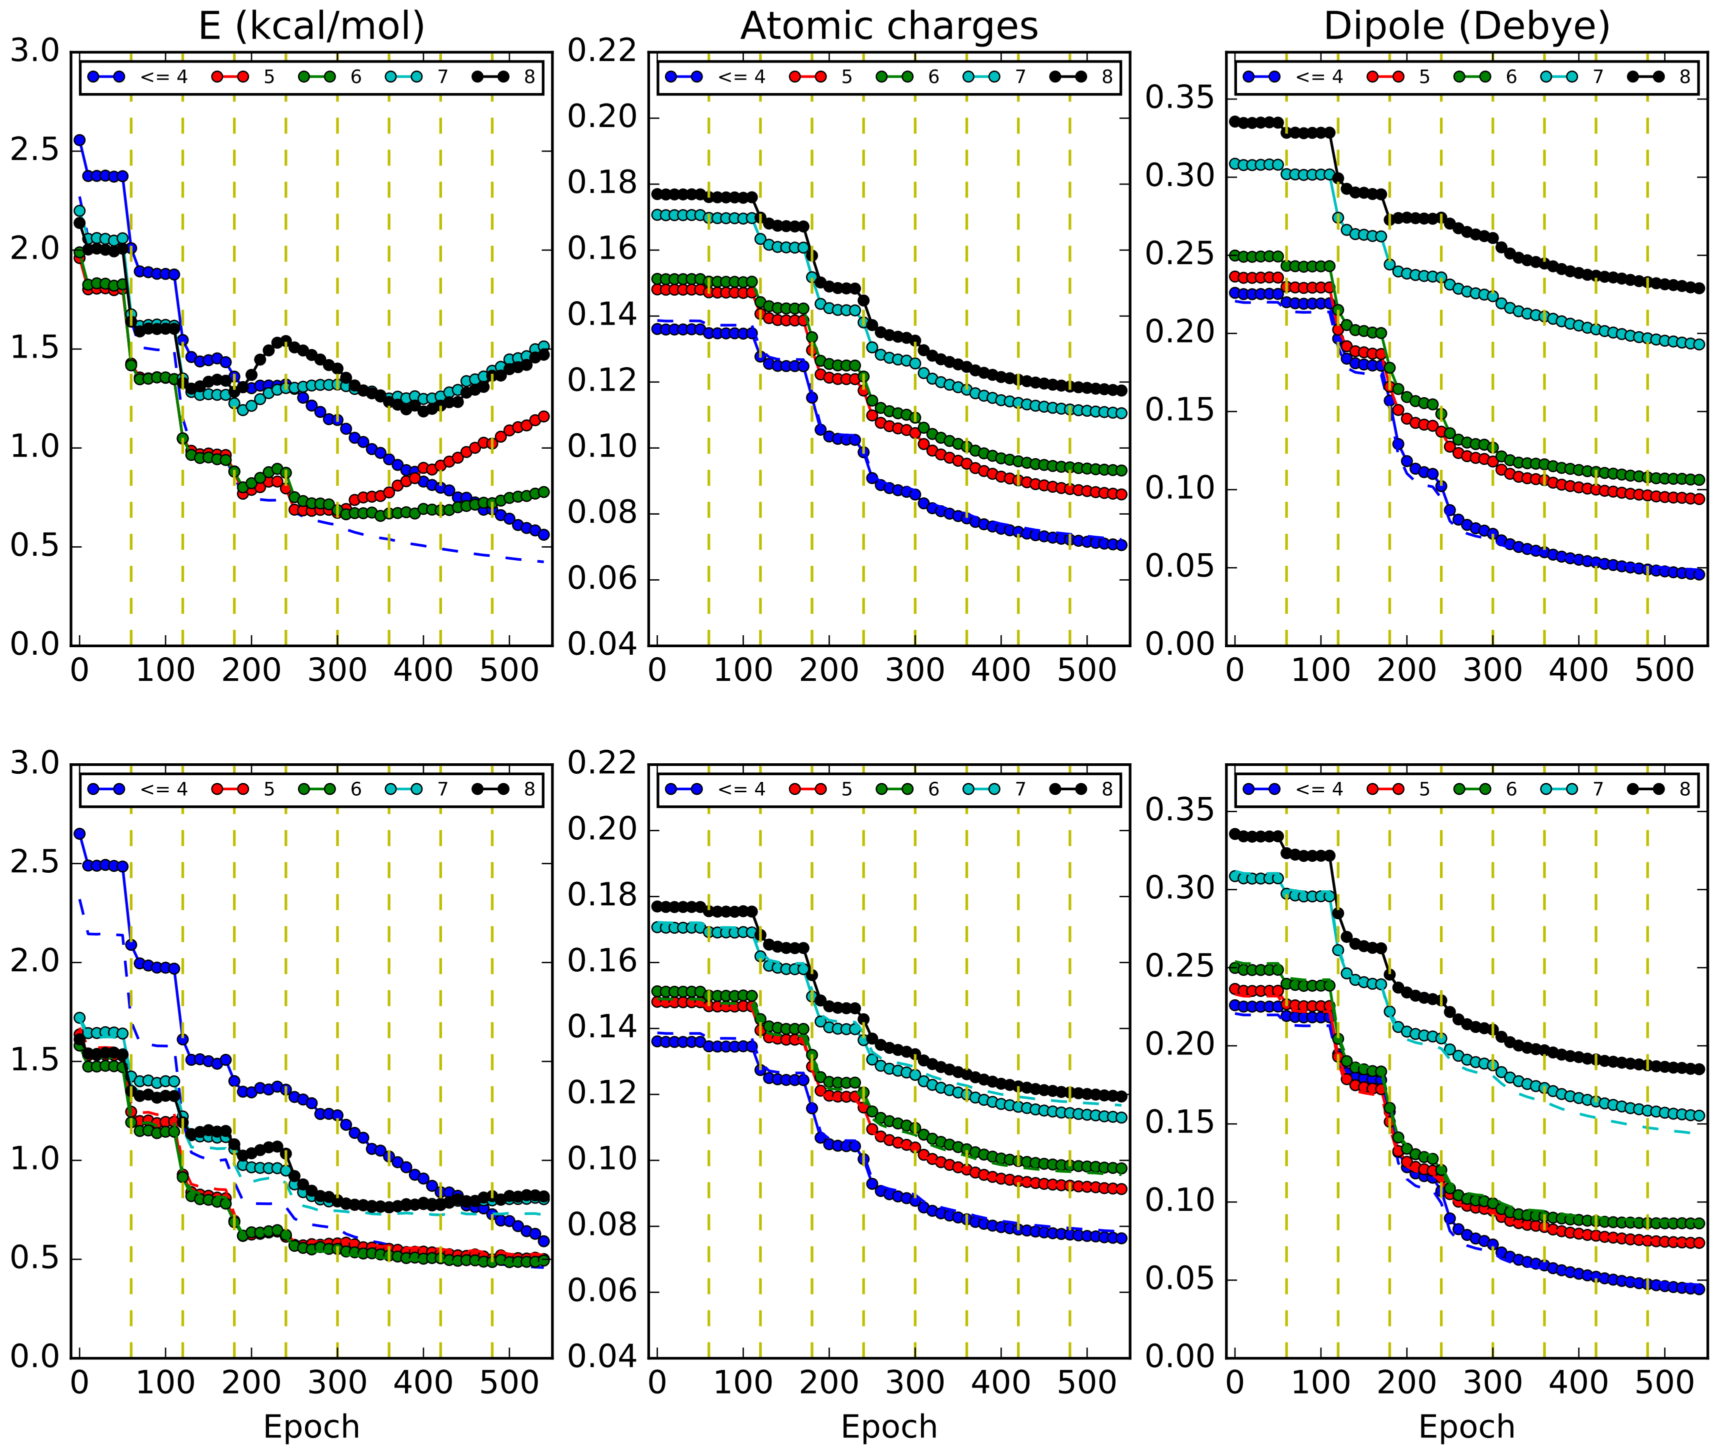

Figure S27 H Diag: Single Variable H Off Diag: DFTB MIO
G Diag: DFTB MIO G Off Diag: DFTB MIO Repulsive: DFTB MIO

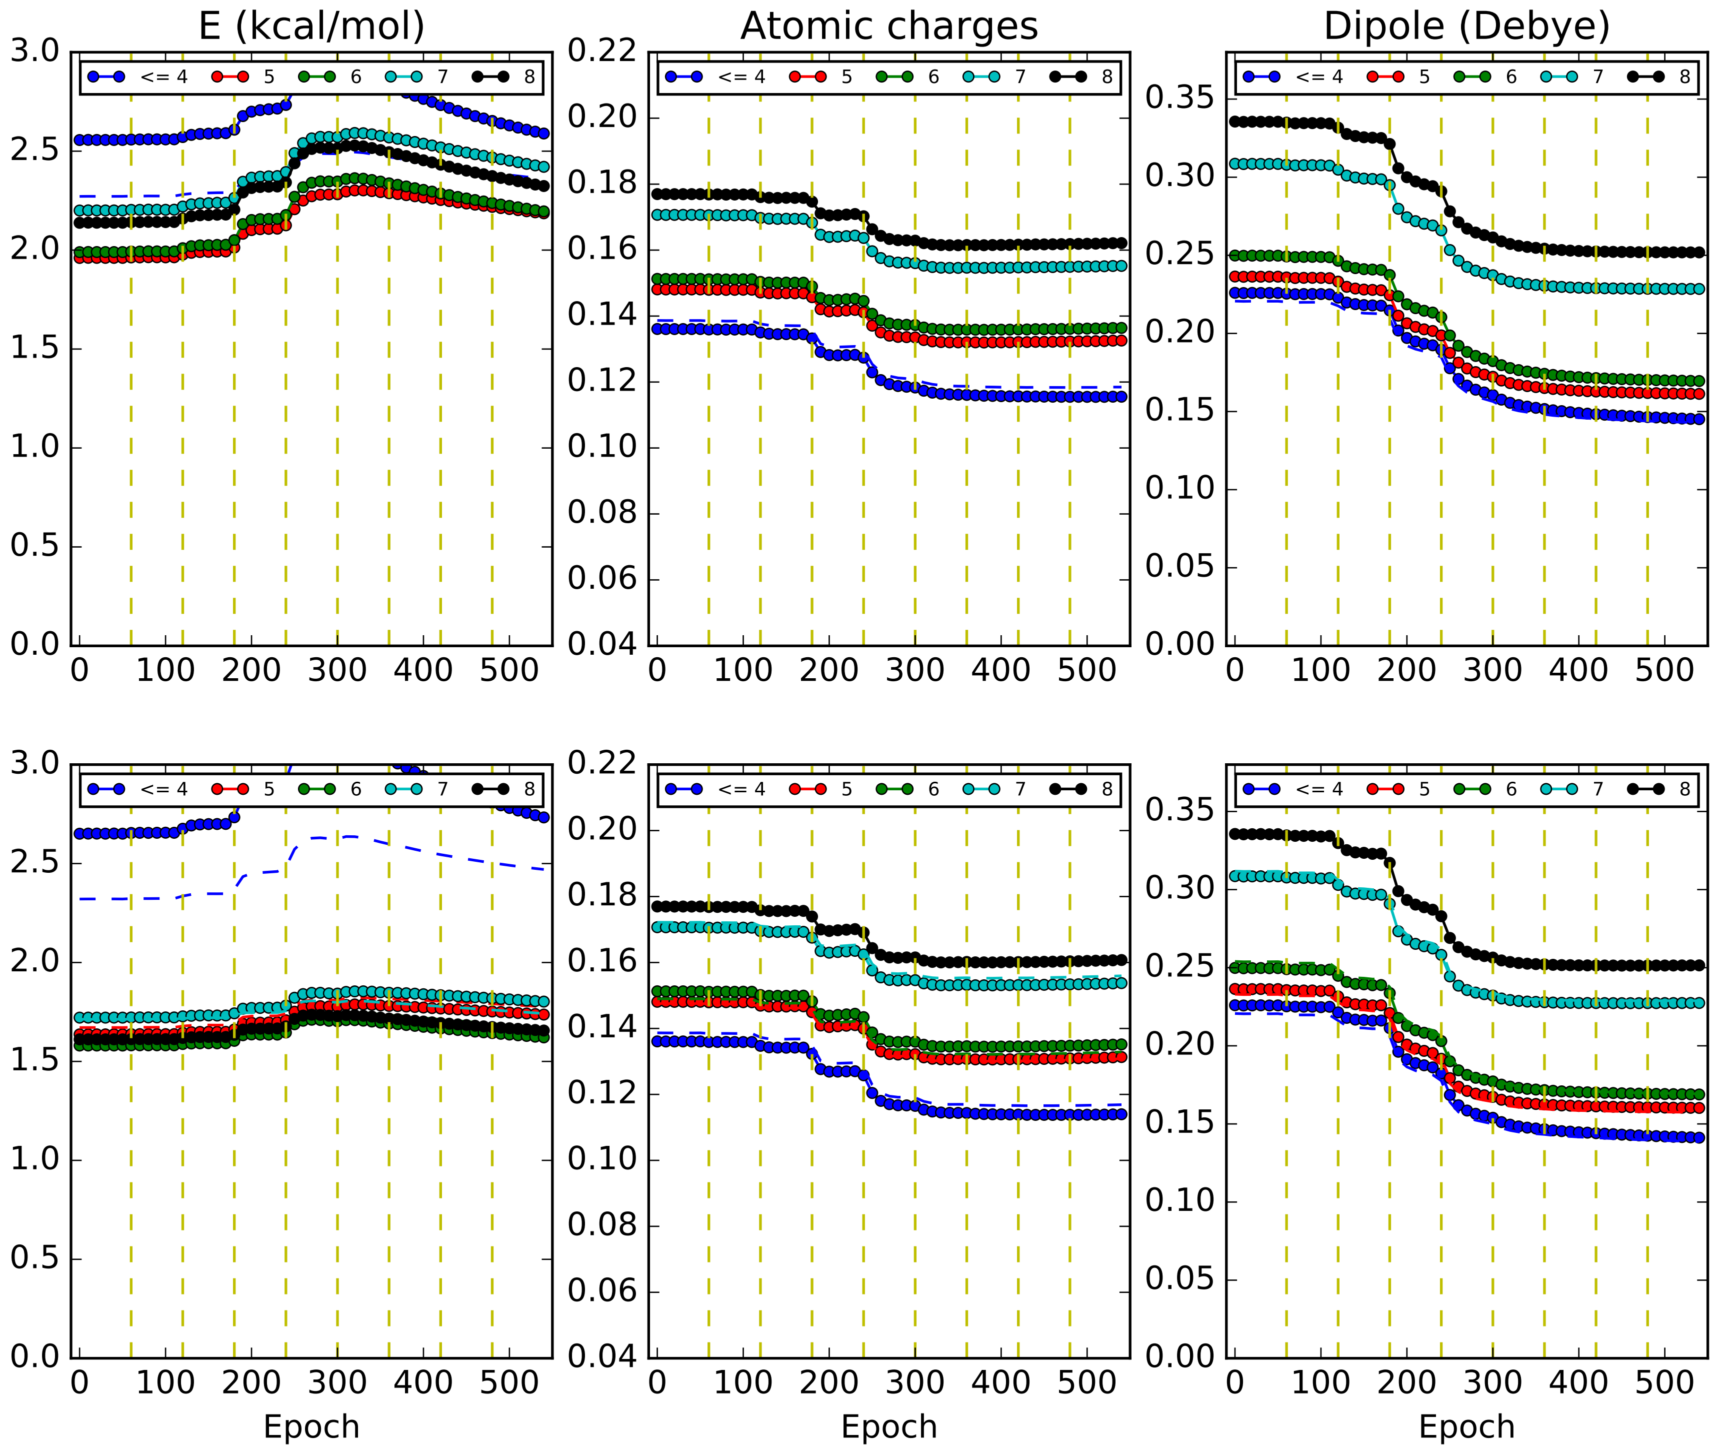

Figure S28 H Diag: DFTB MIO H Off Diag: Spline
G Diag: DFTB MIO G Off Diag: DFTB MIO Repulsive: DFTB MIO

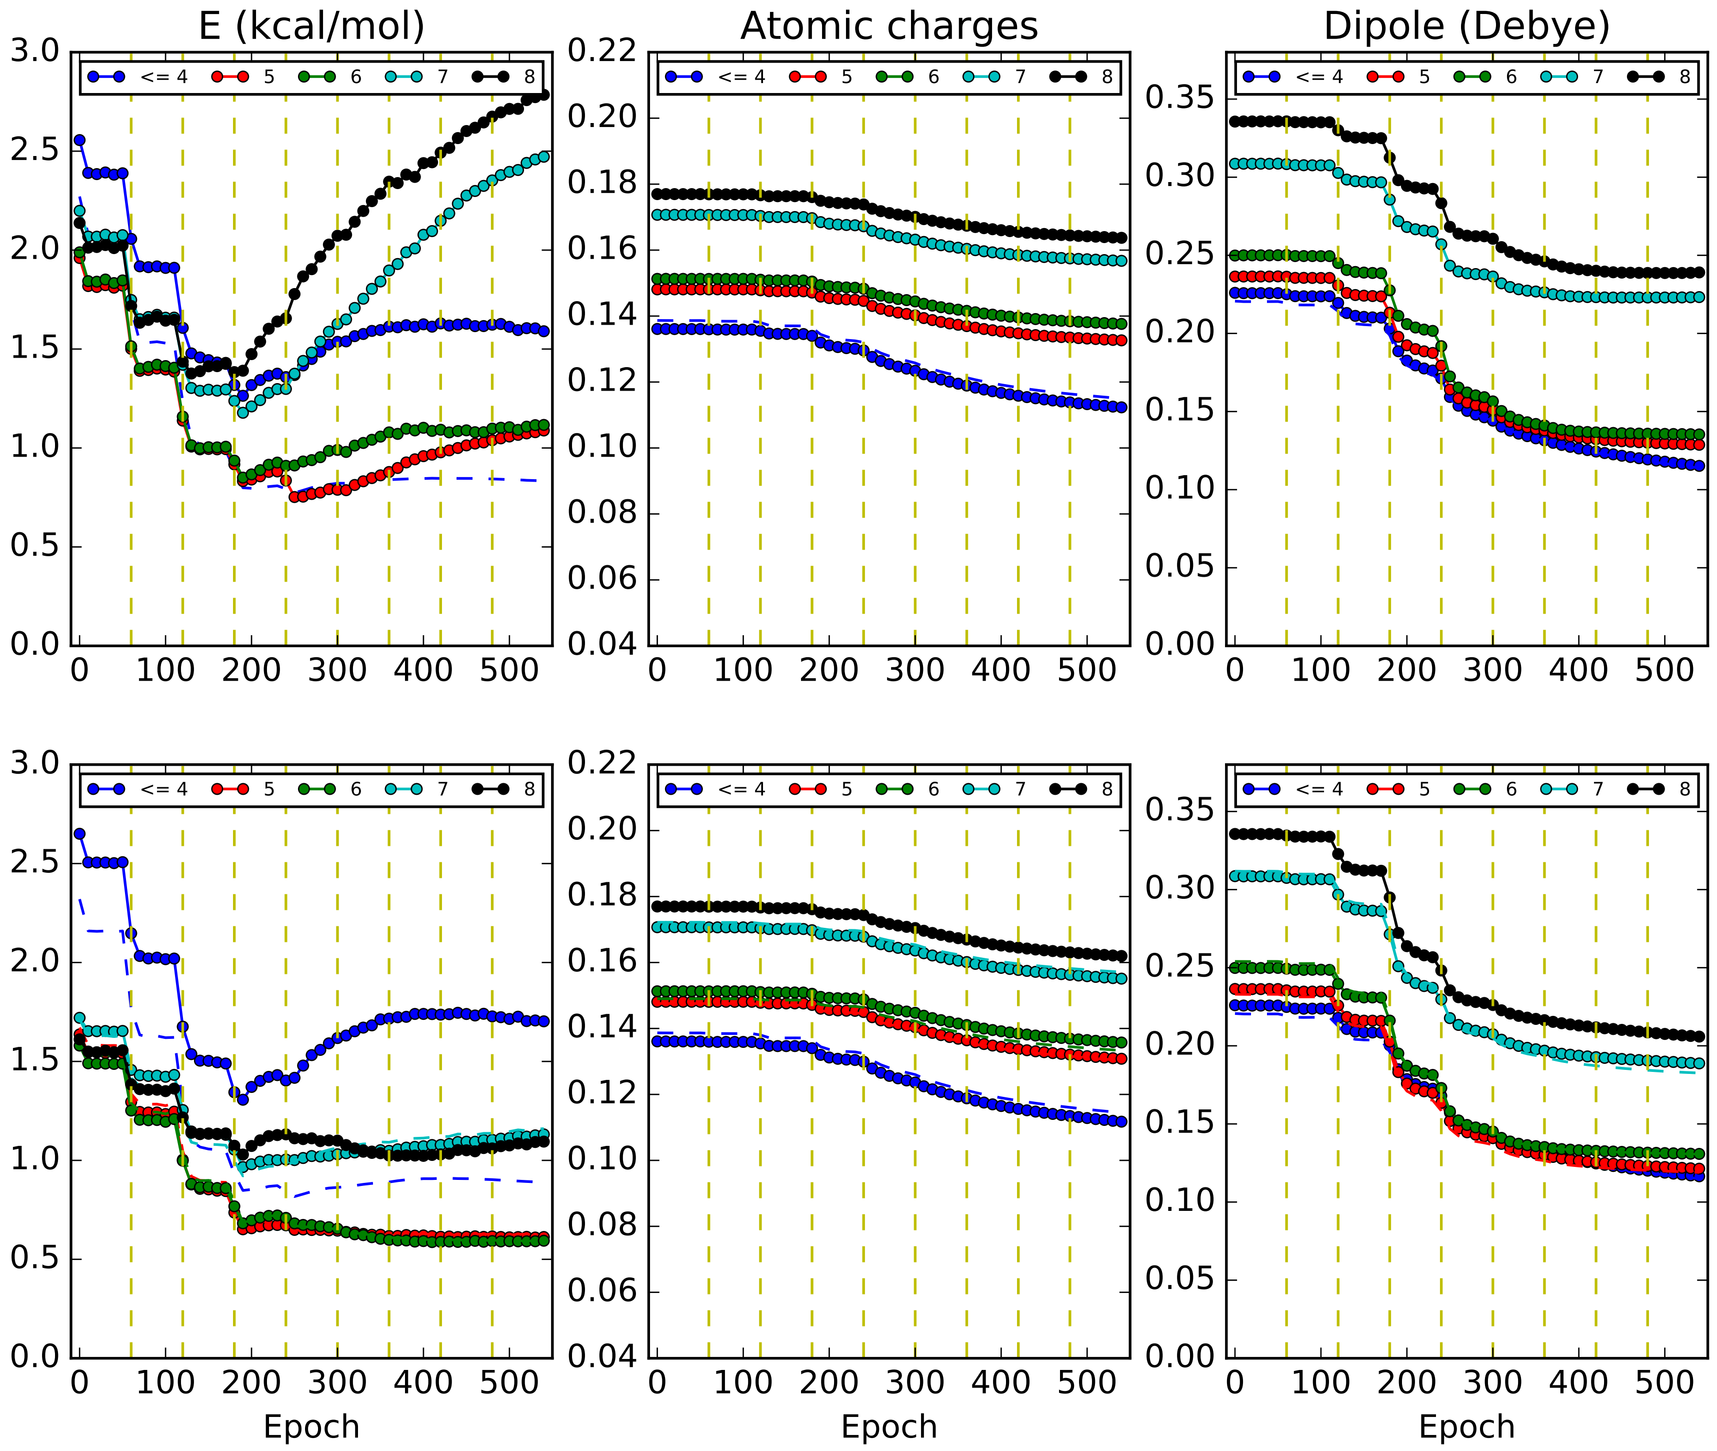

Figure S29 H Diag: DFTB MIO H Off Diag: DFTB MIO
G Diag: Single Variable G Off Diag: DFTB MIO Repulsive: DFTB MIO

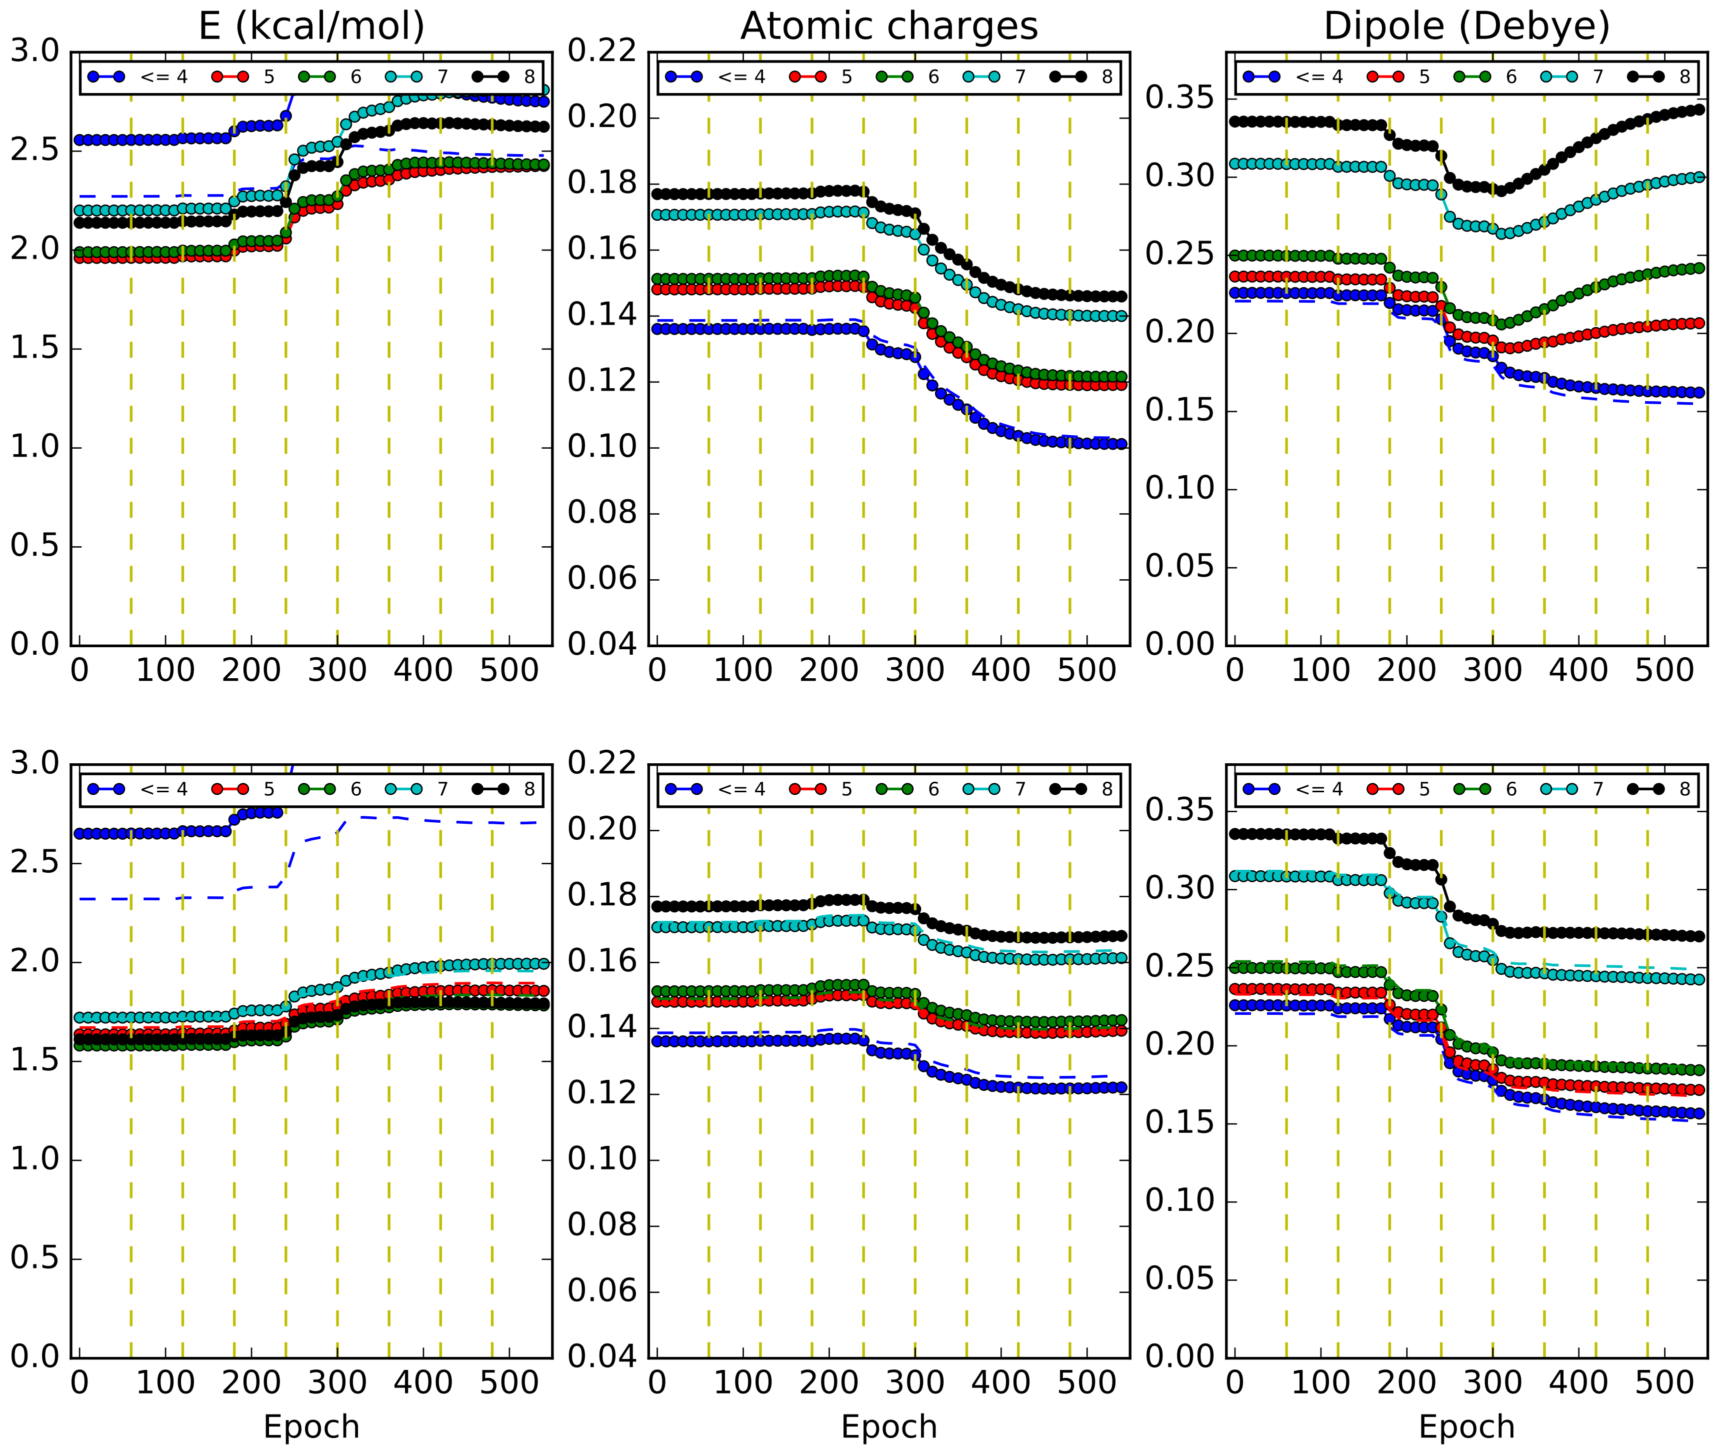

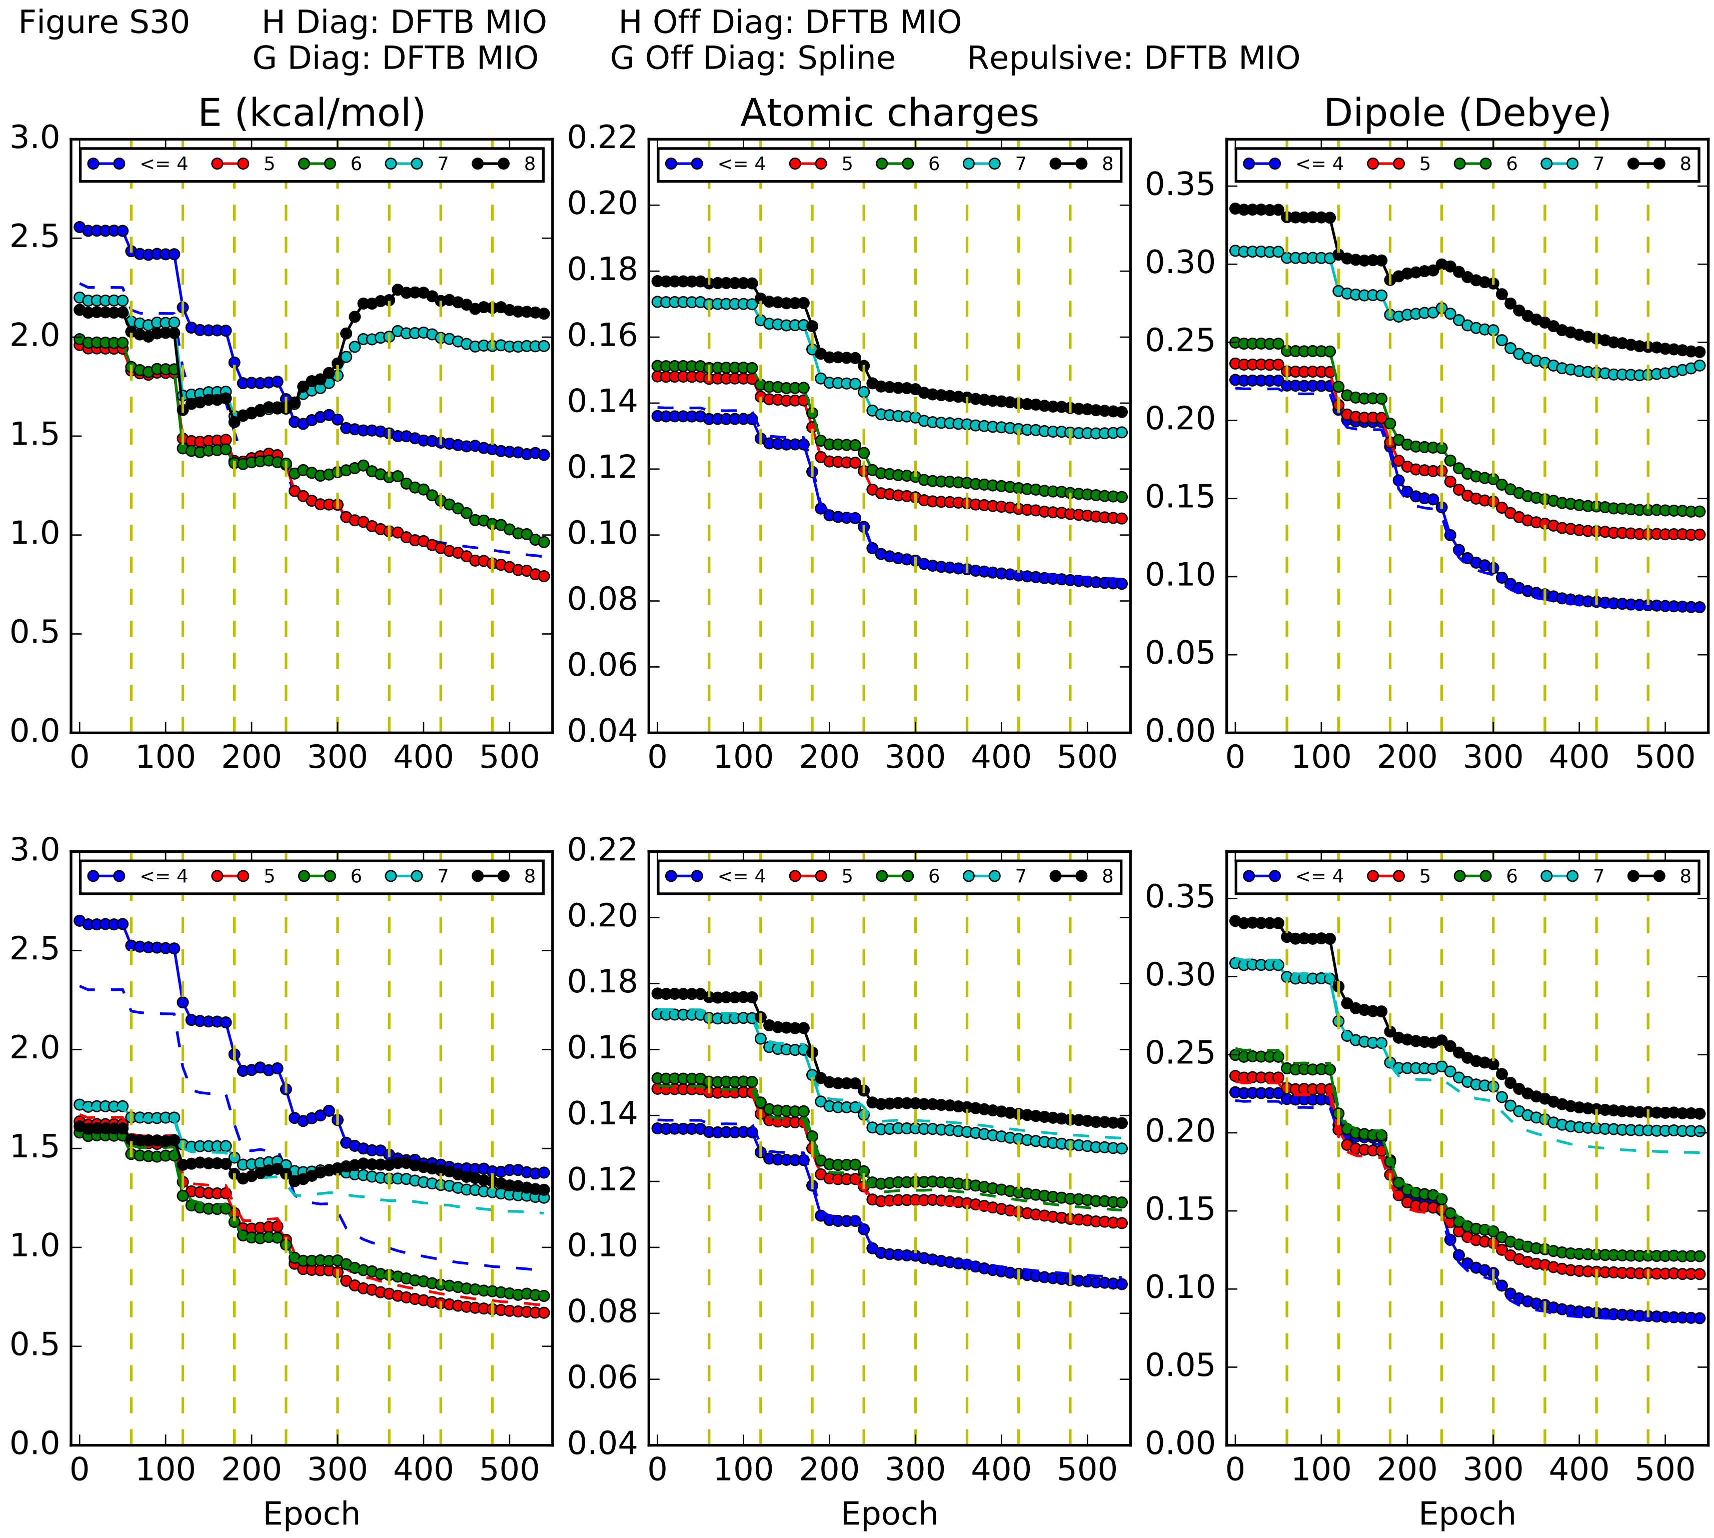

Figure S30
H Diag: DFTB MIO
H Off Diag: DFTB MIO
G Diag: DFTB MIO
G Off Diag: Spline
Repulsive: DFTB MIO
E (kcal/mol)
Atomic charges
Dipole (Debye)
<= 4
5
6
7
8
Epoch

Figure S31 H Diag: DFTB MIO H Off Diag: DFTB MIO
G Diag: DFTB MIO G Off Diag: DFTB MIO Repulsive: Spline

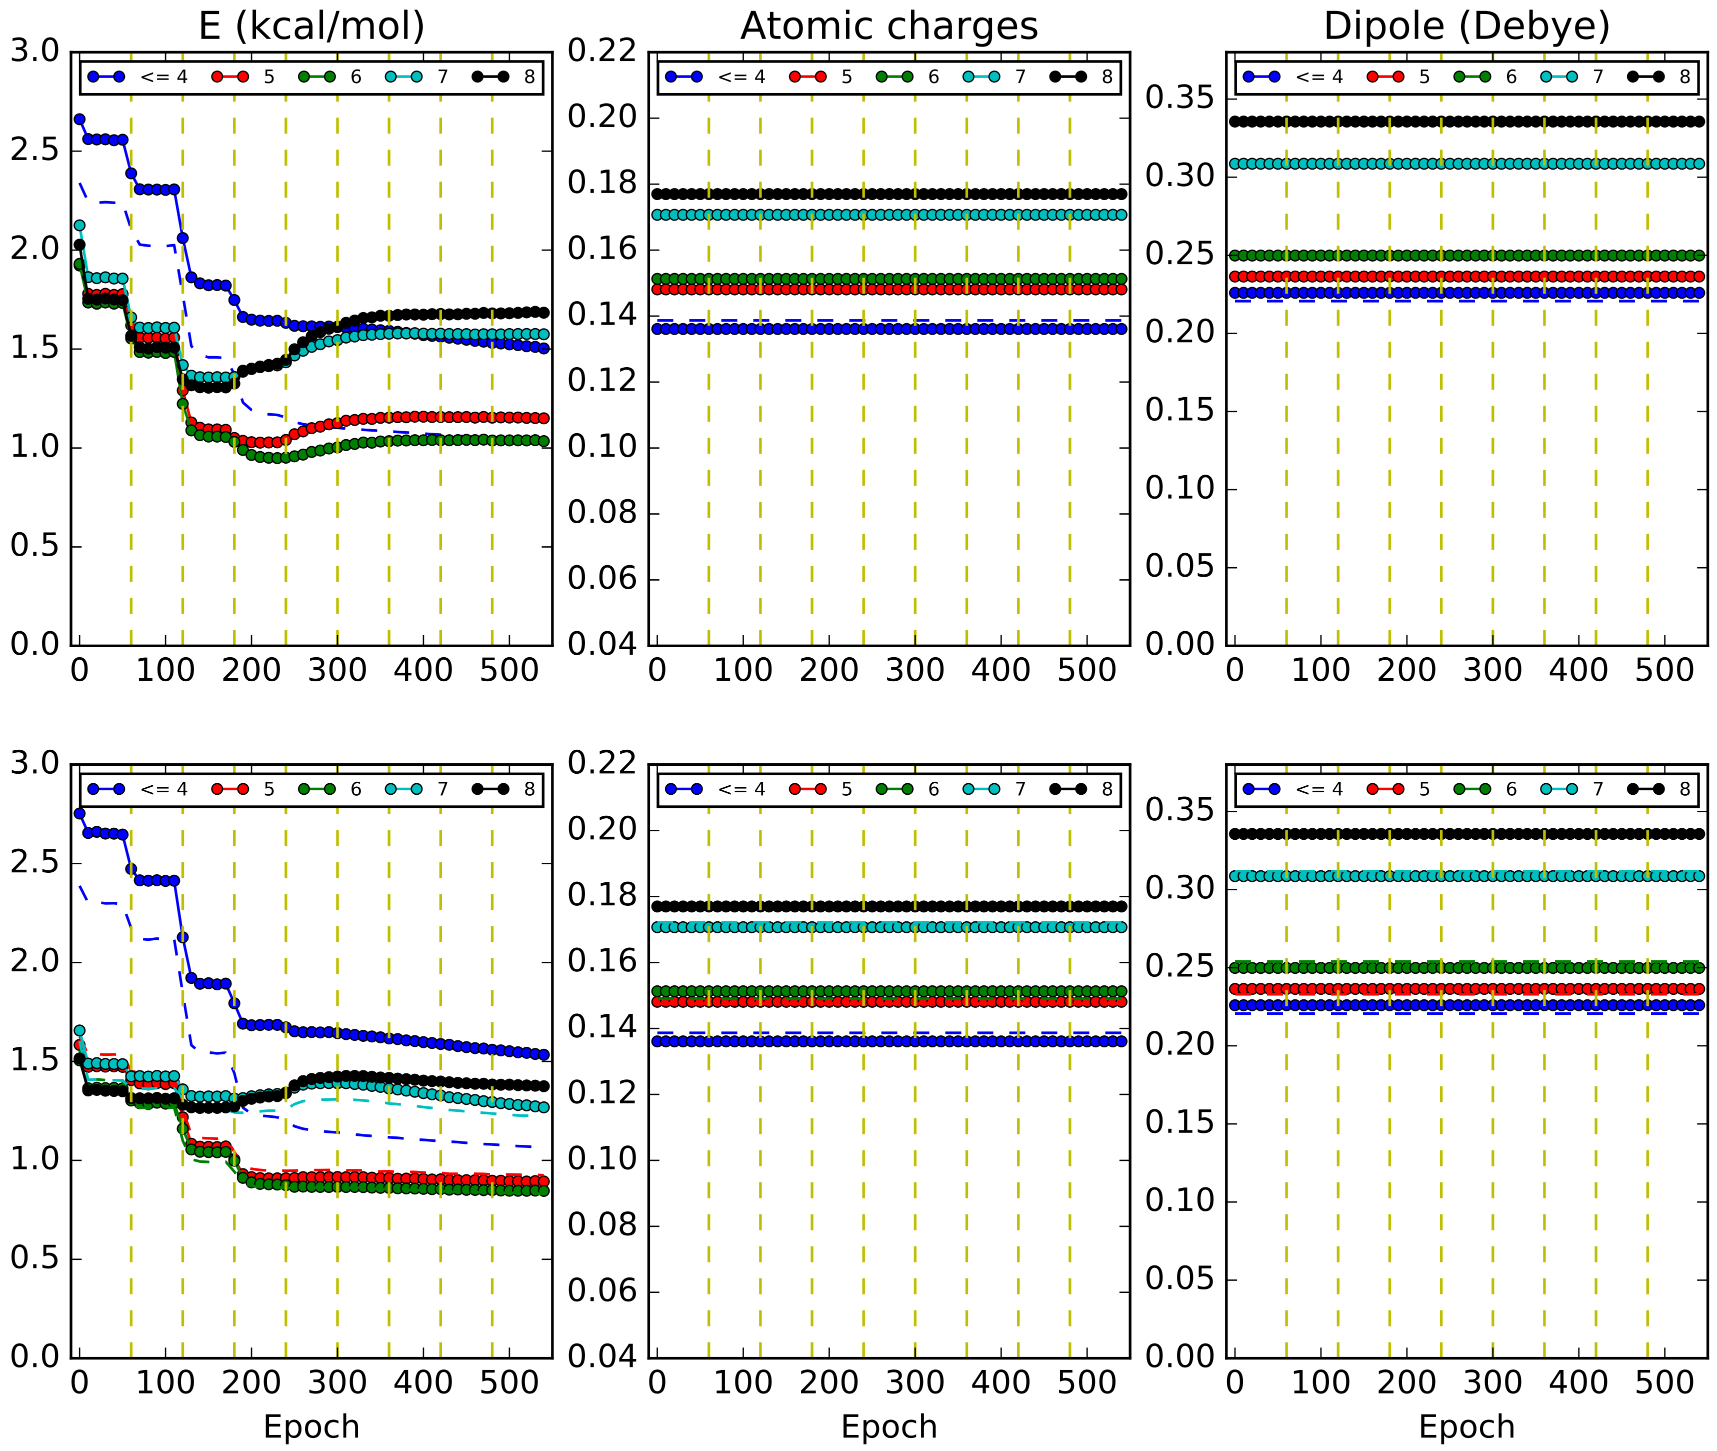

Figure S32 H Diag: FFNN 1 H Off Diag: FFNN 1
G Diag: FFNN 1 G Off Diag: FFNN 1 Repulsive: Spline

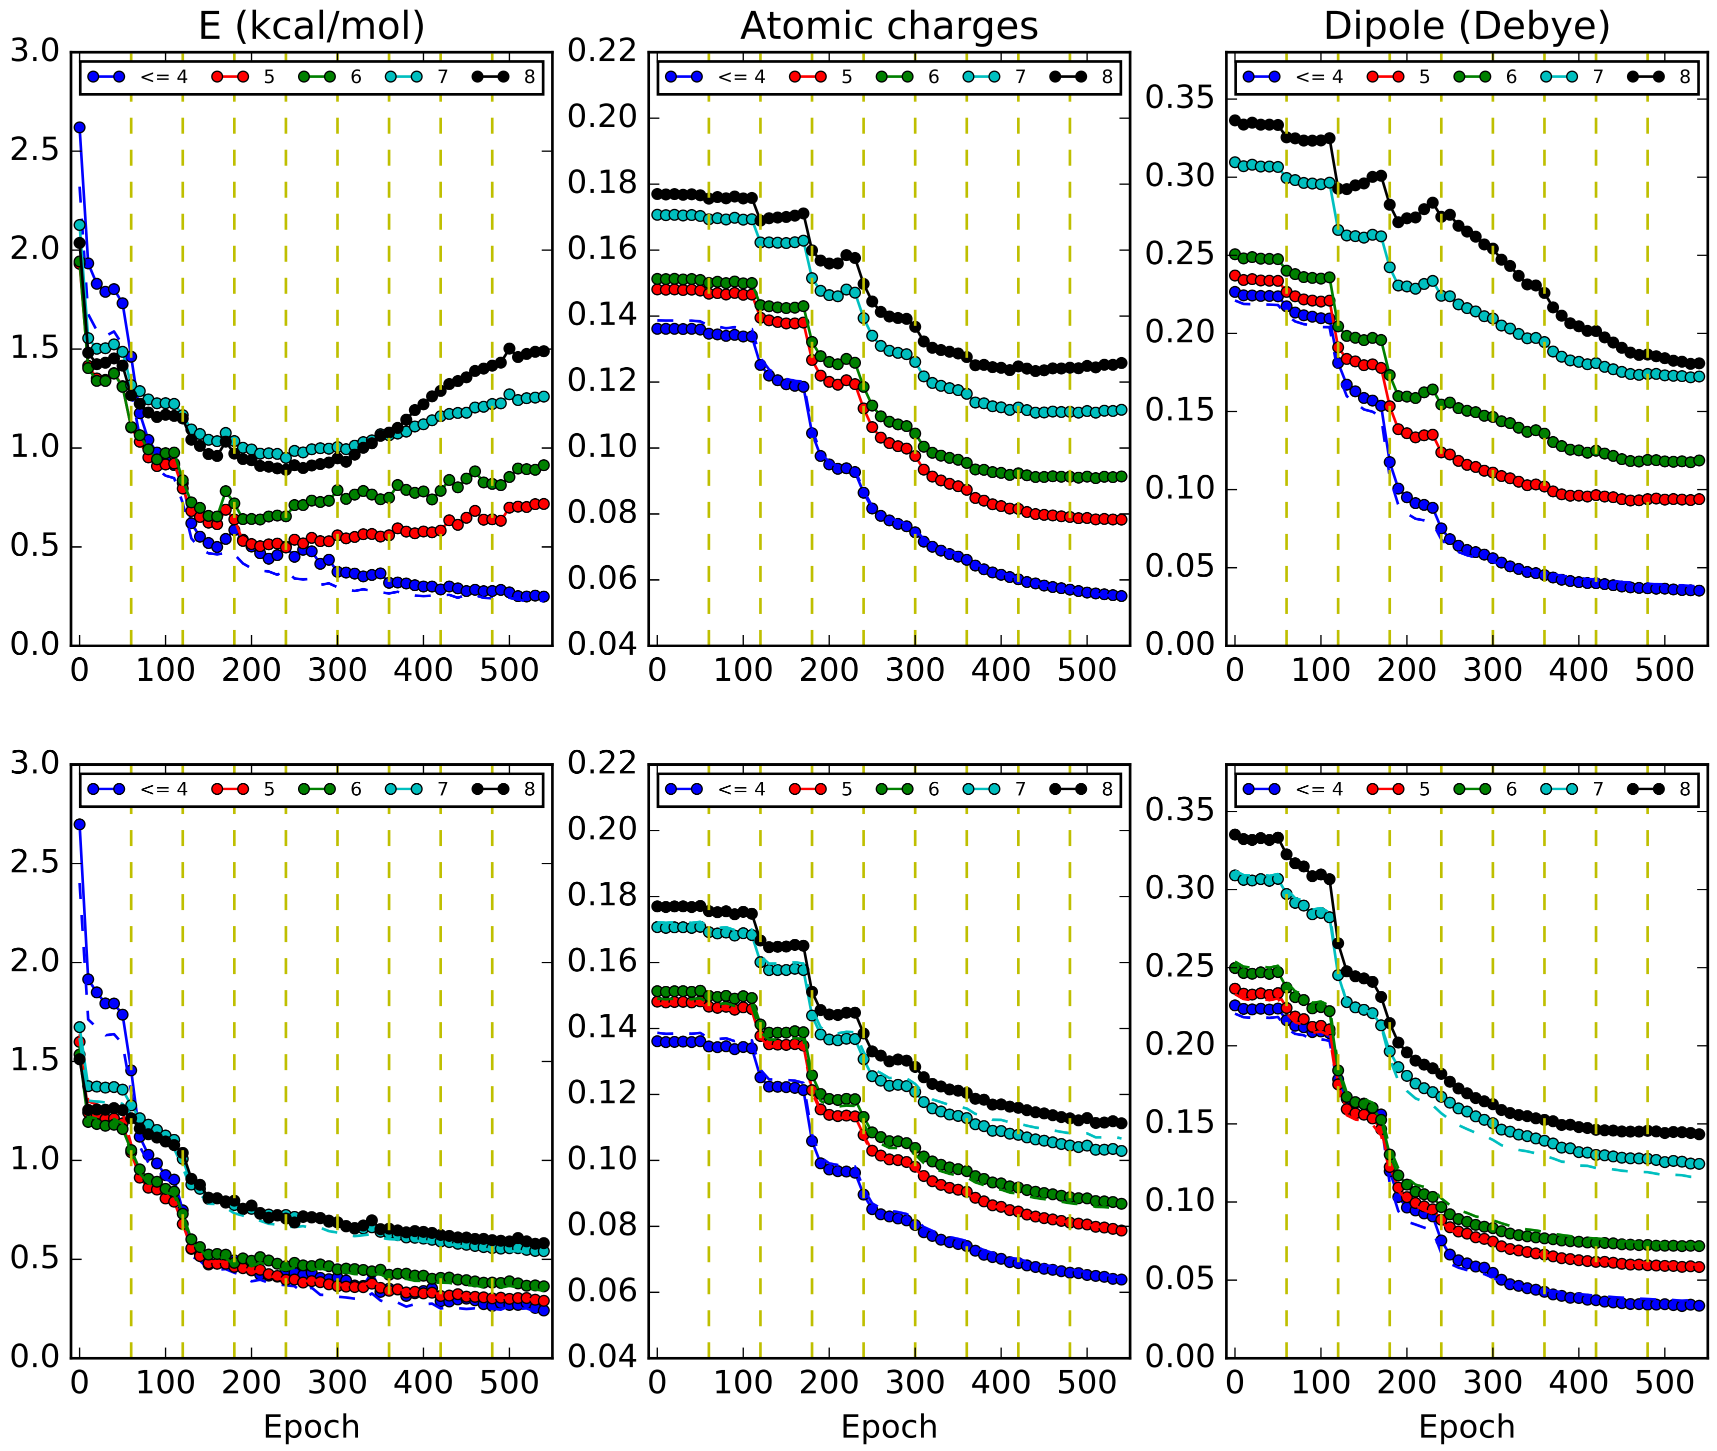

Figure S33 H Diag: DFTB MIO H Off Diag: FFNN 1
G Diag: FFNN 1 G Off Diag: FFNN 1 Repulsive: Spline

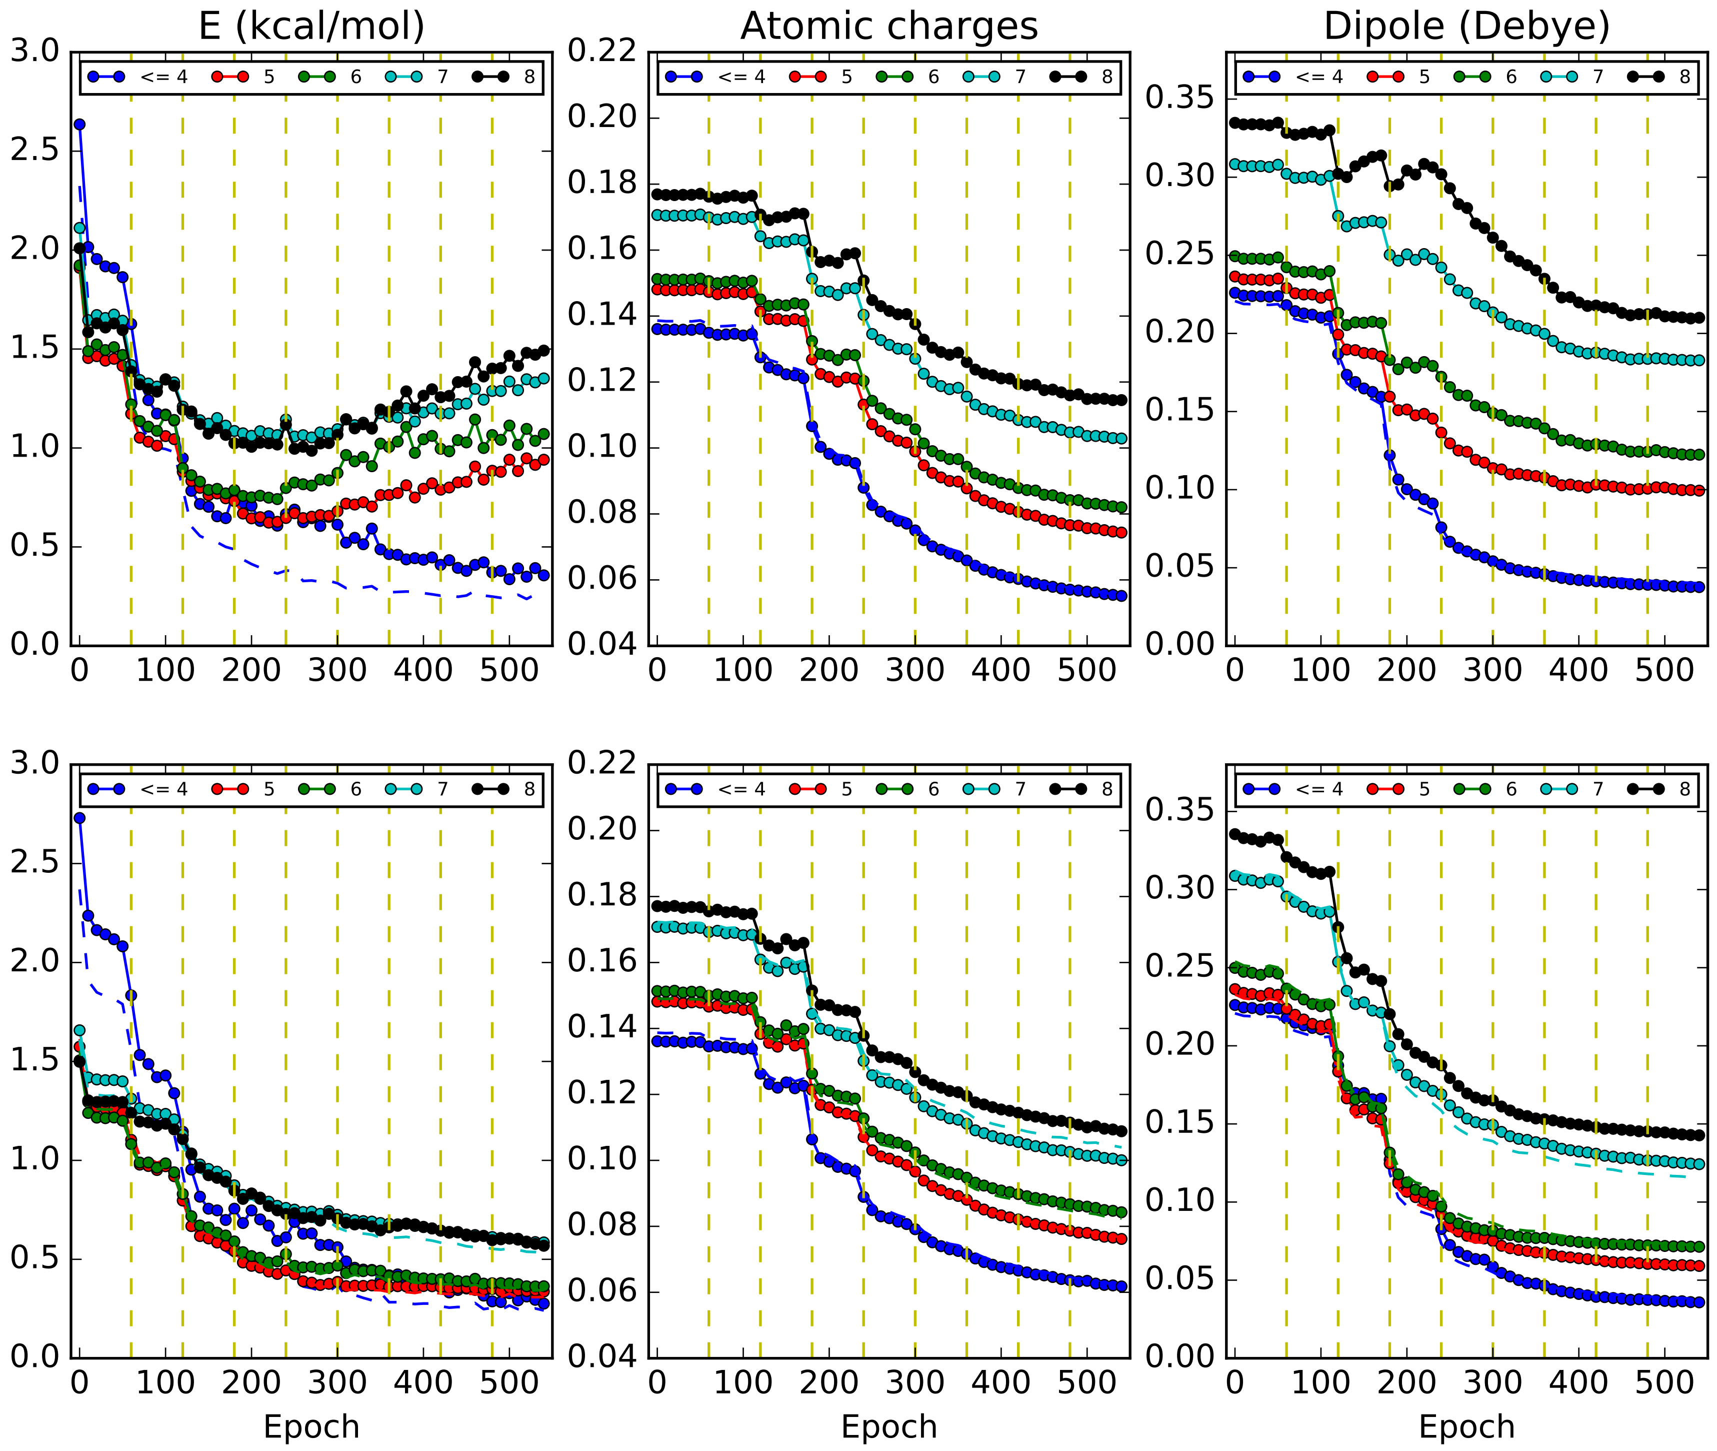

Figure S34 H Diag: FFNN 1 H Off Diag: DFTB MIO
G Diag: FFNN 1 G Off Diag: FFNN 1 Repulsive: Spline

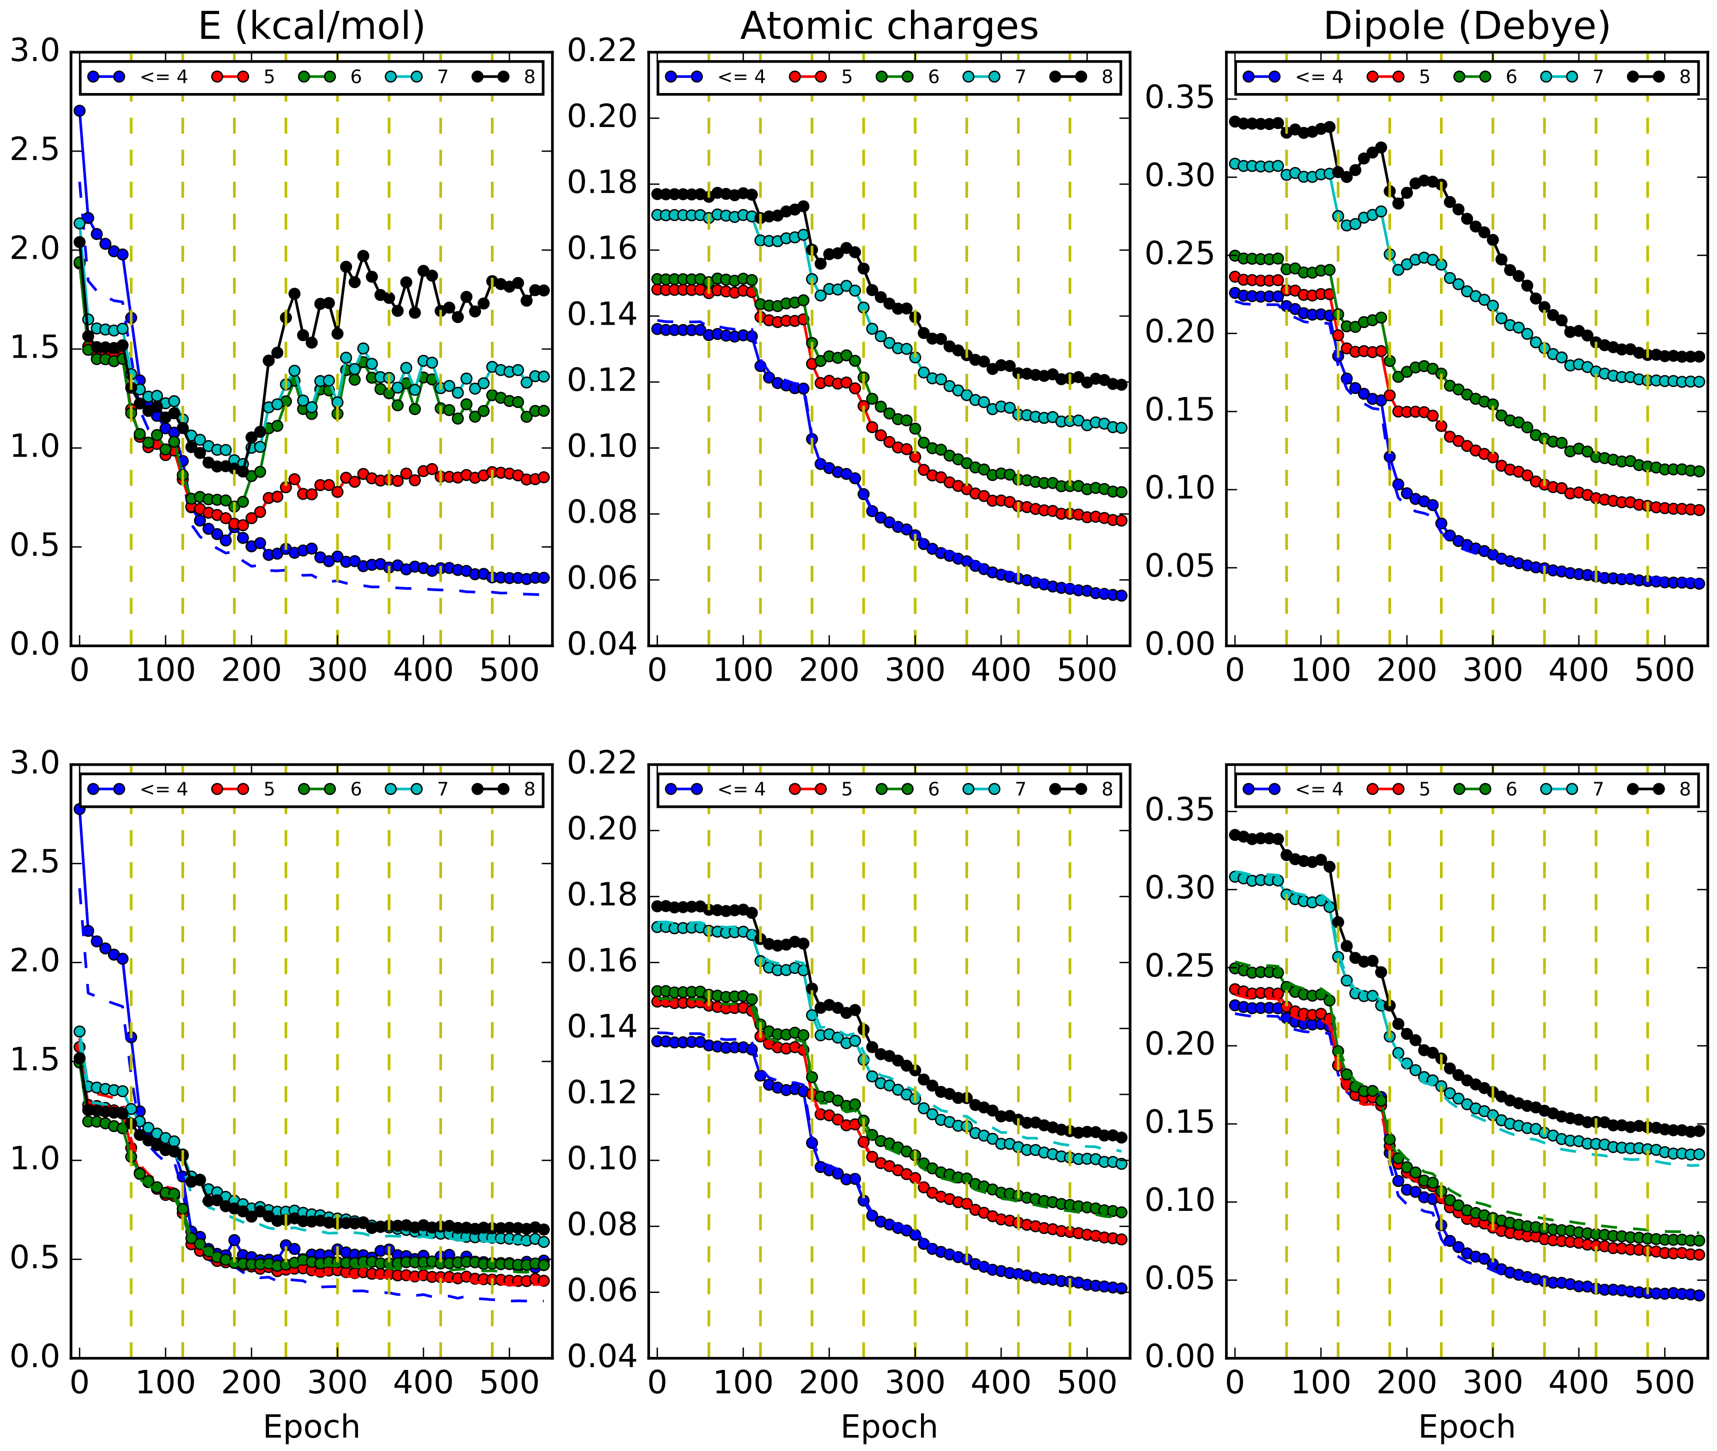

Figure S35 H Diag: FFNN 1 H Off Diag: FFNN 1
G Diag: DFTB MIO G Off Diag: FFNN 1 Repulsive: Spline

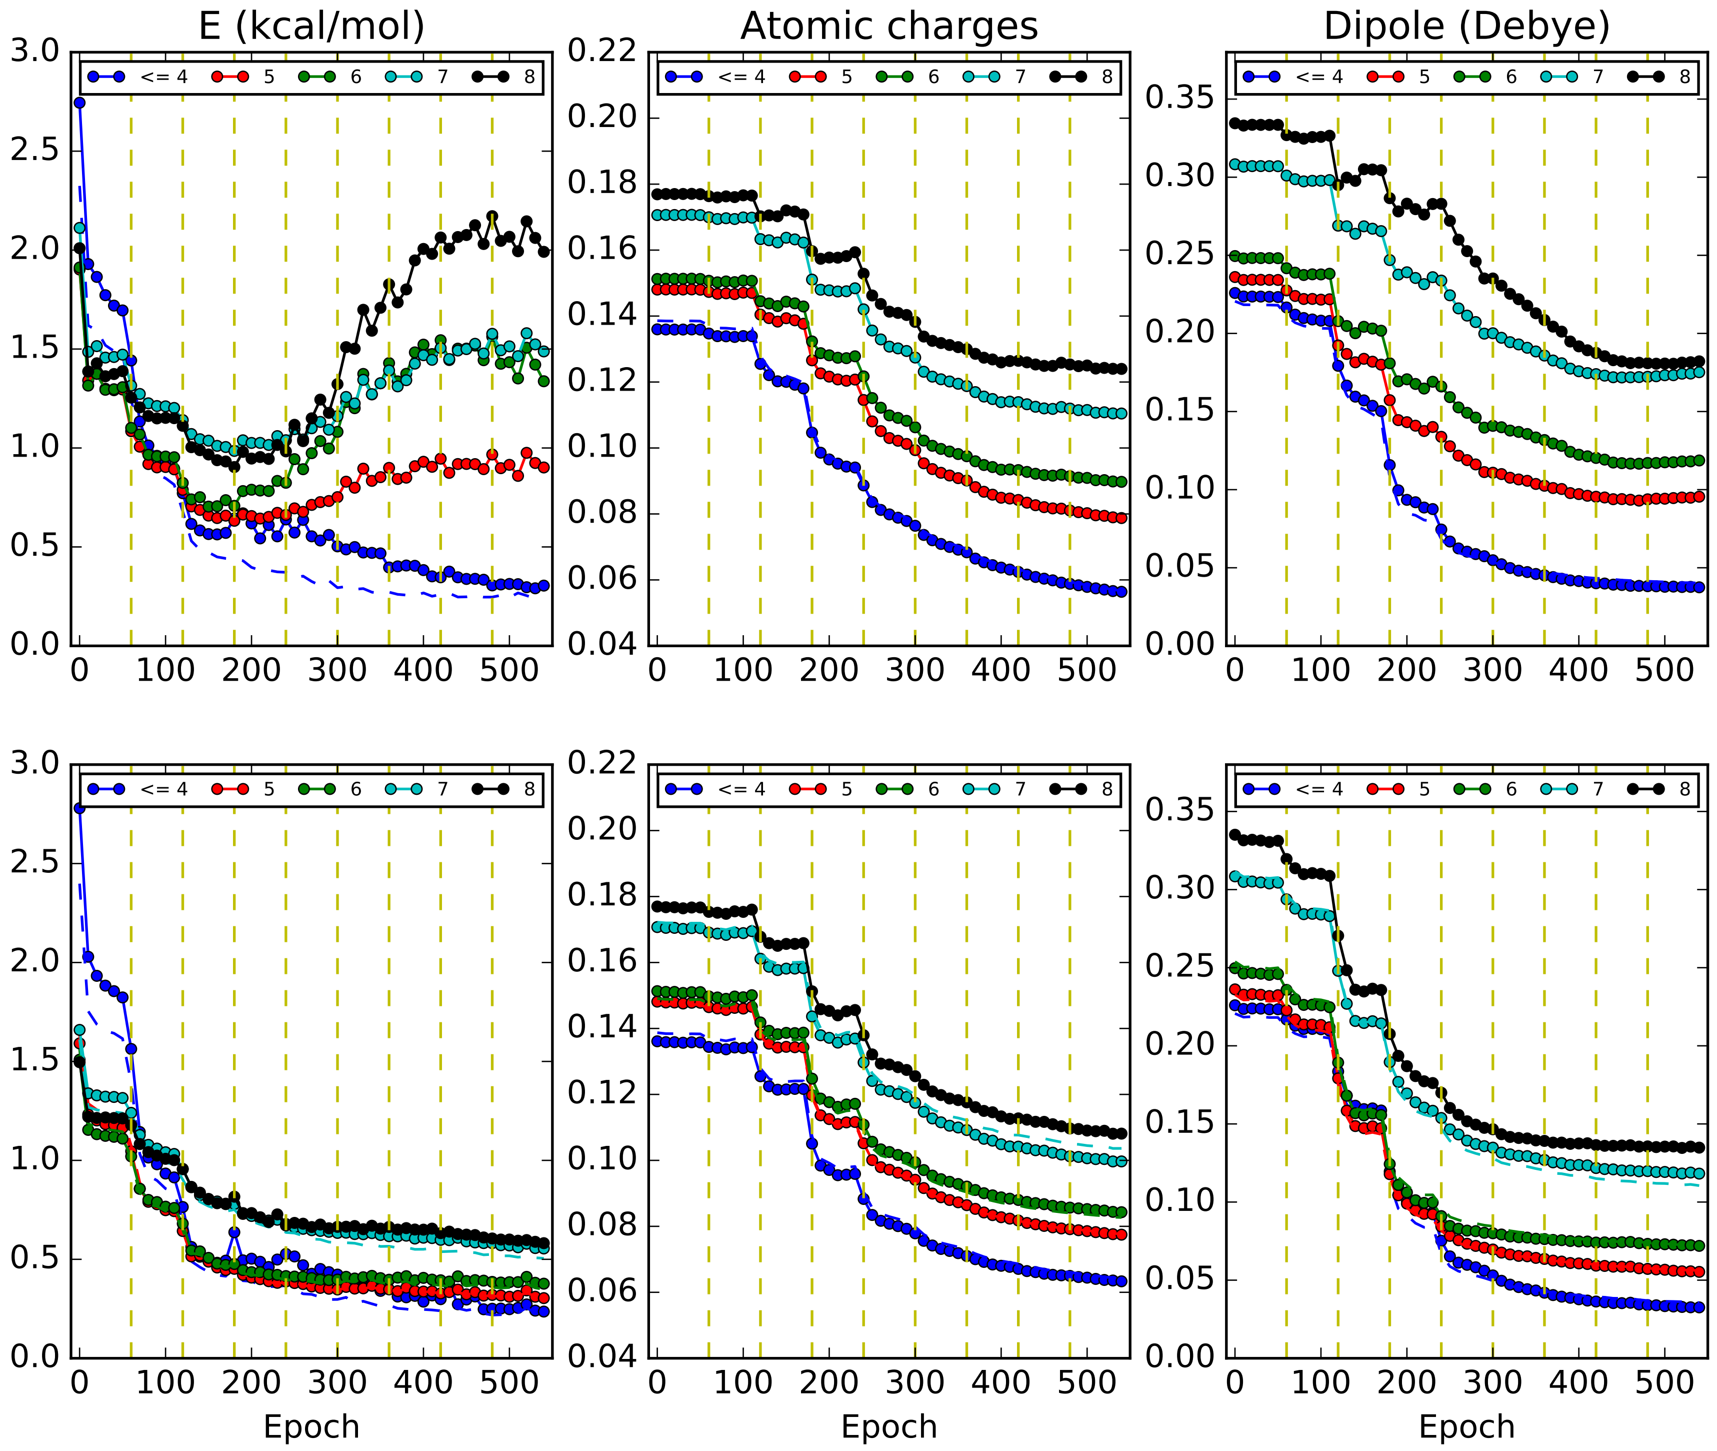

Figure S36 H Diag: FFNN 1 H Off Diag: FFNN 1
G Diag: FFNN 1 G Off Diag: DFTB MIO Repulsive: Spline

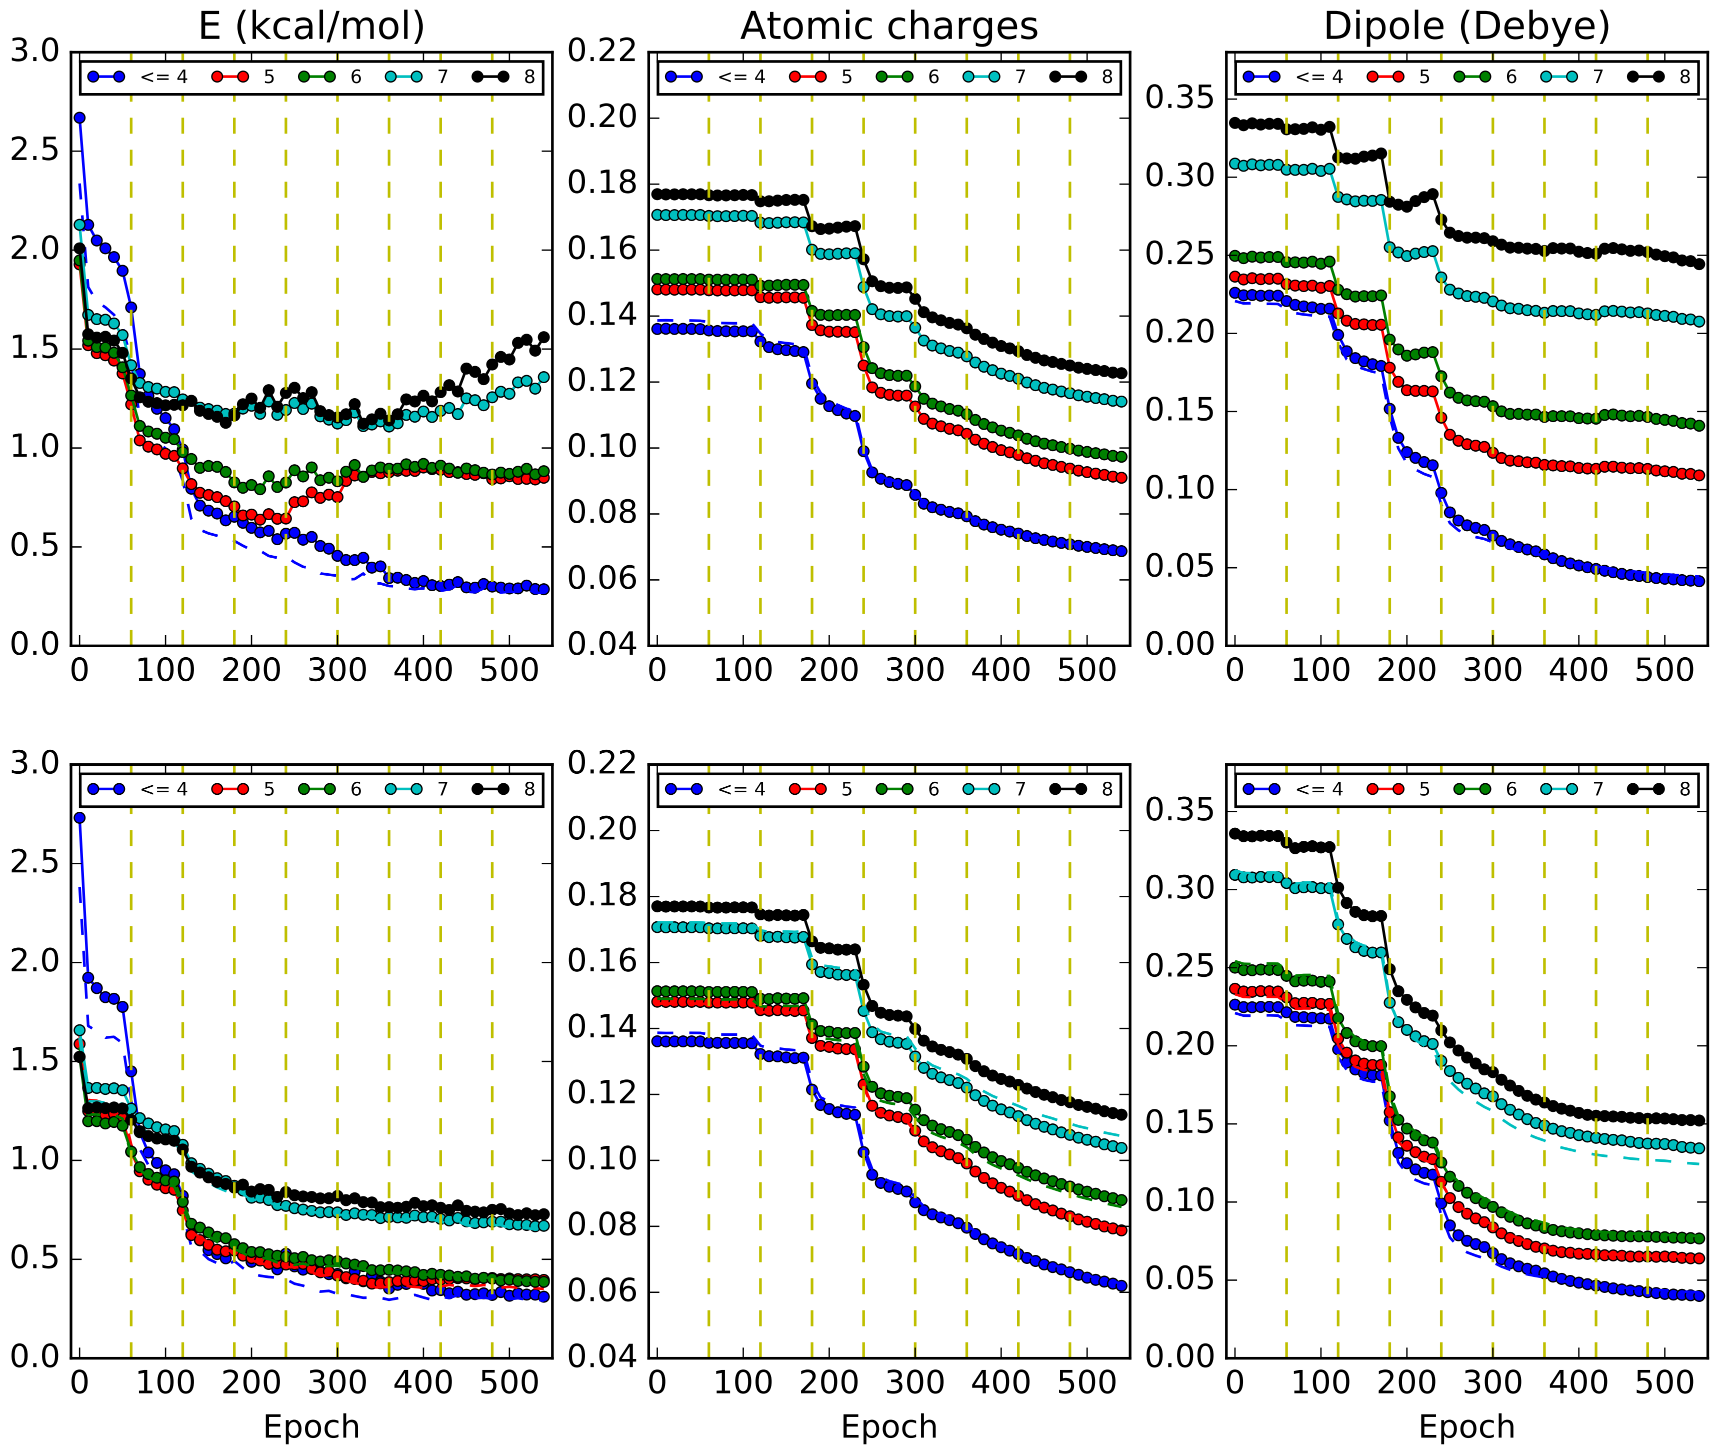

Figure S37 H Diag: FFNN 1 H Off Diag: DFTB MIO
G Diag: DFTB MIO G Off Diag: DFTB MIO Repulsive: Spline

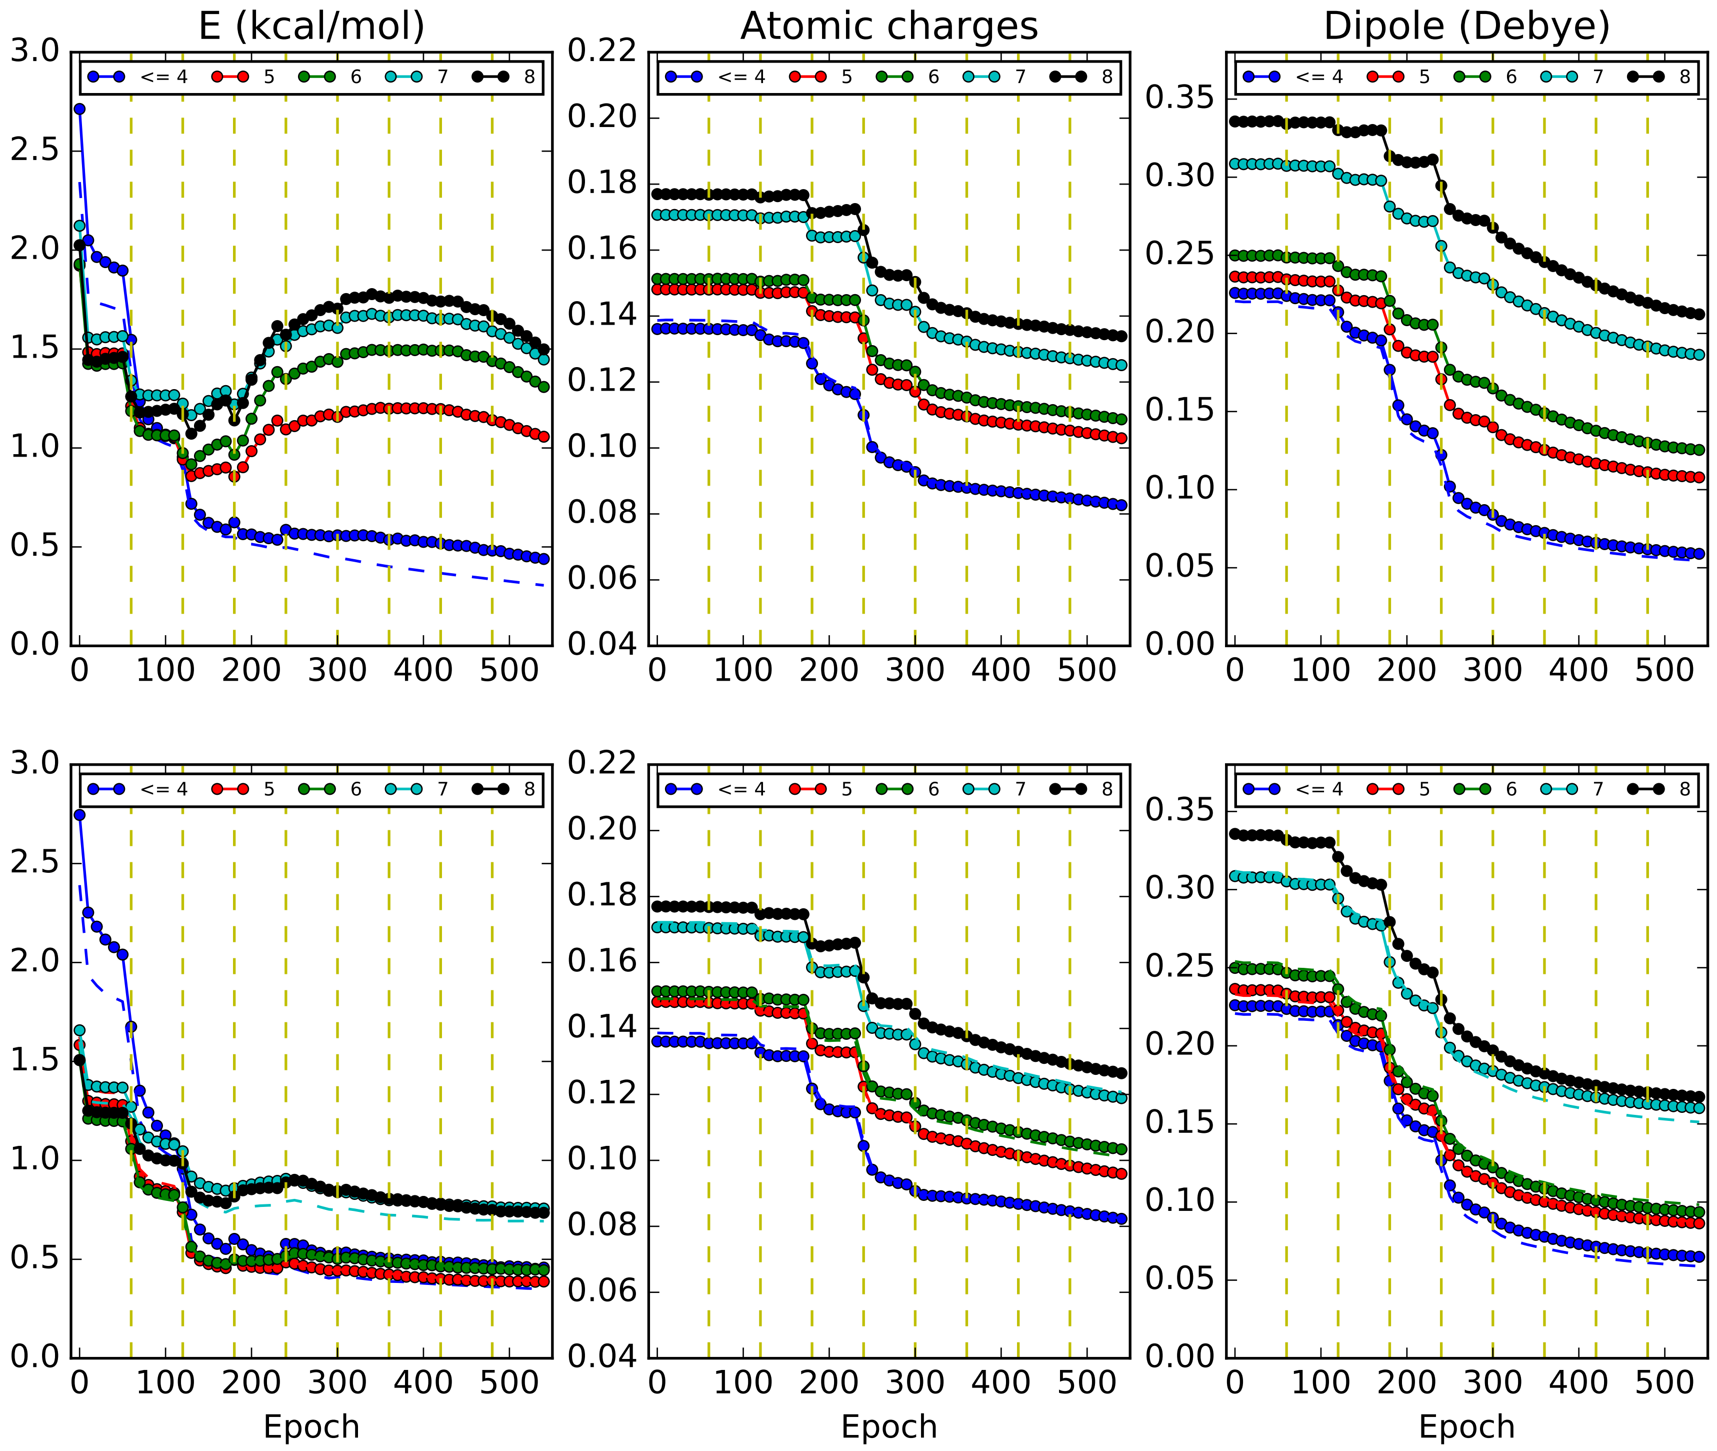

Figure S38 H Diag: DFTB MIO H Off Diag: FFNN 1
G Diag: DFTB MIO G Off Diag: DFTB MIO Repulsive: Spline

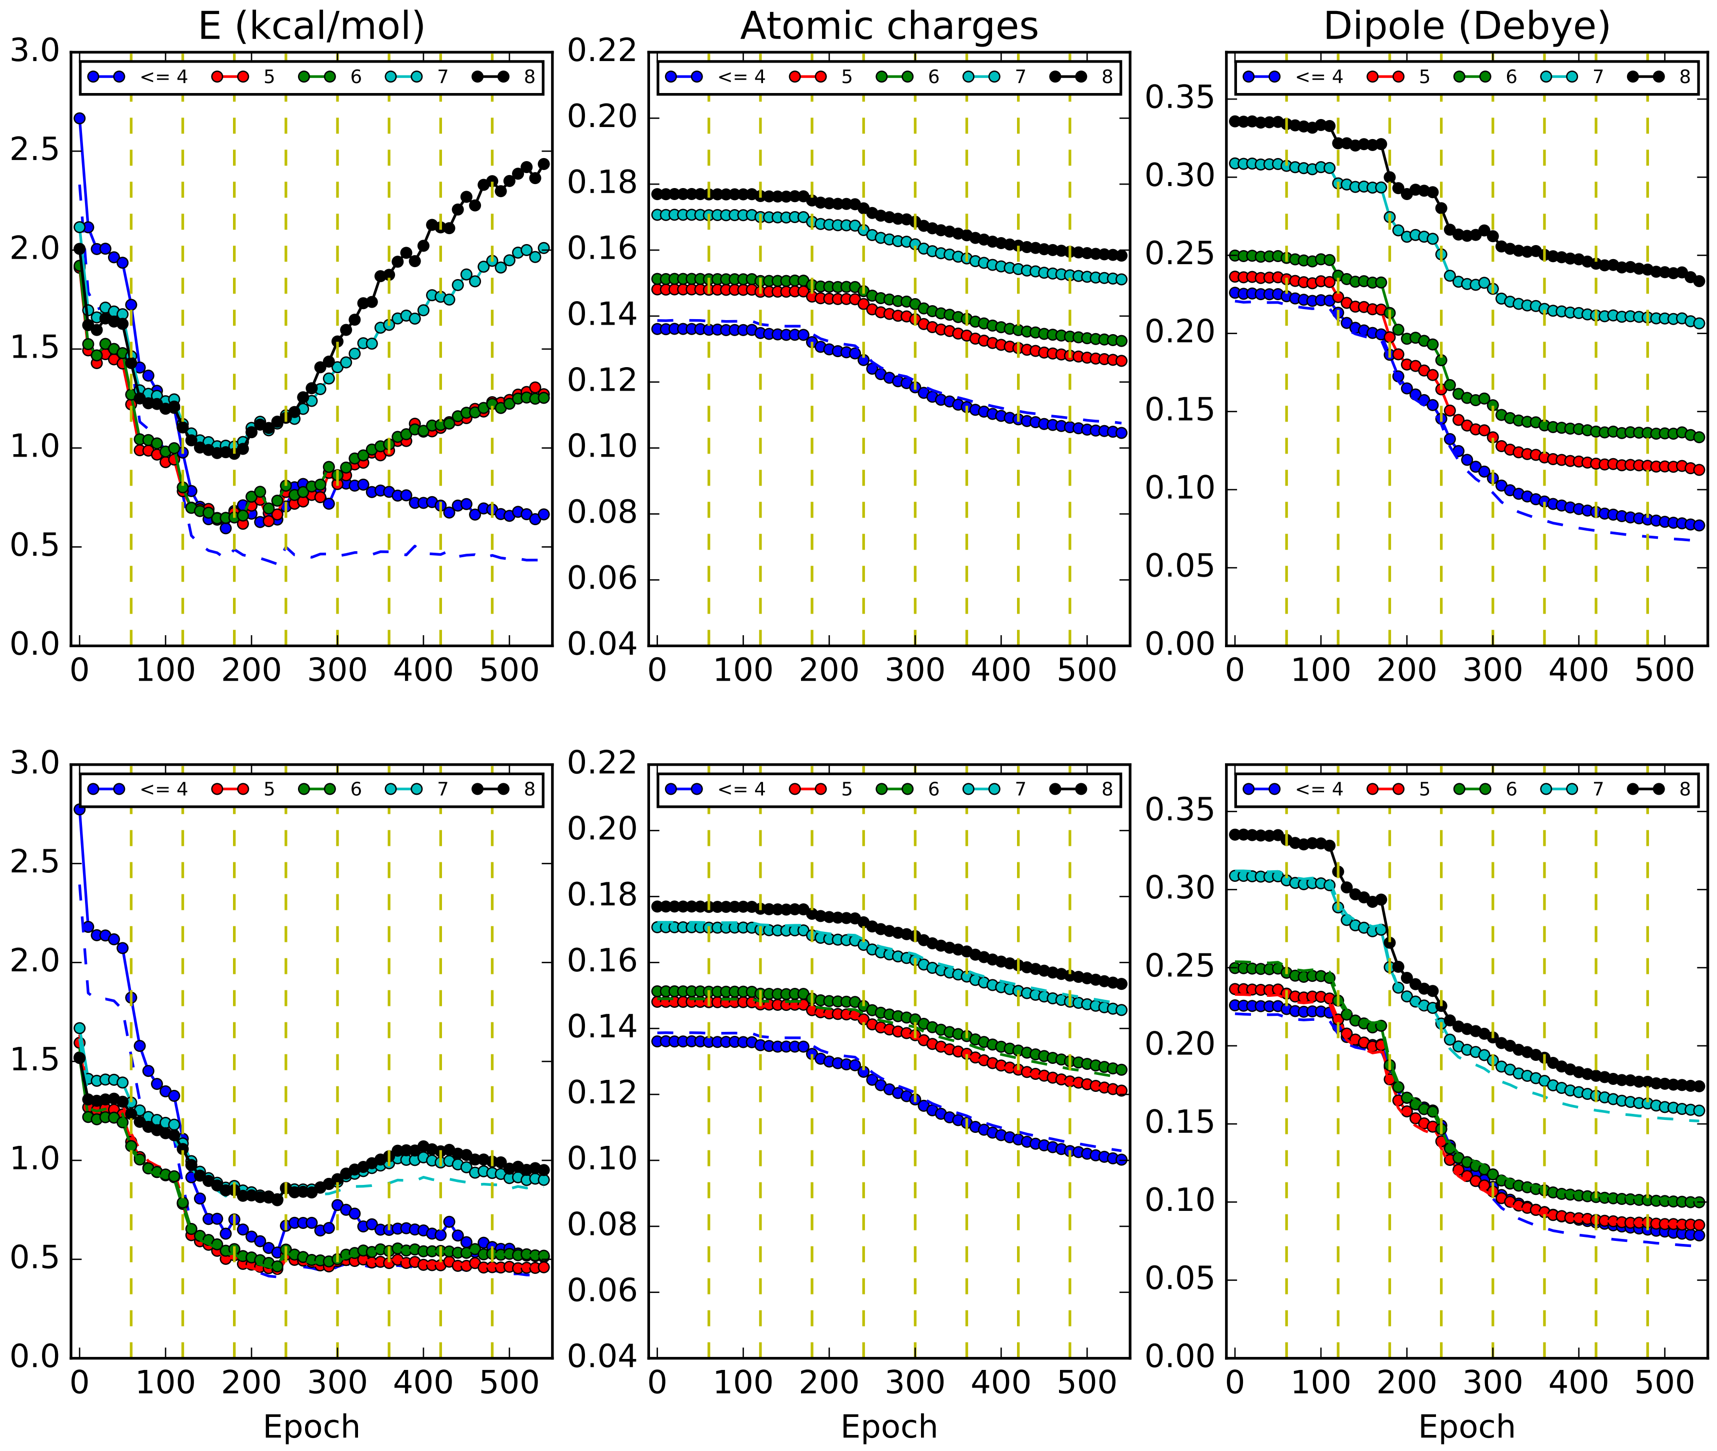

Figure S39 H Diag: DFTB MIO H Off Diag: DFTB MIO
G Diag: FFNN 1 G Off Diag: DFTB MIO Repulsive: Spline

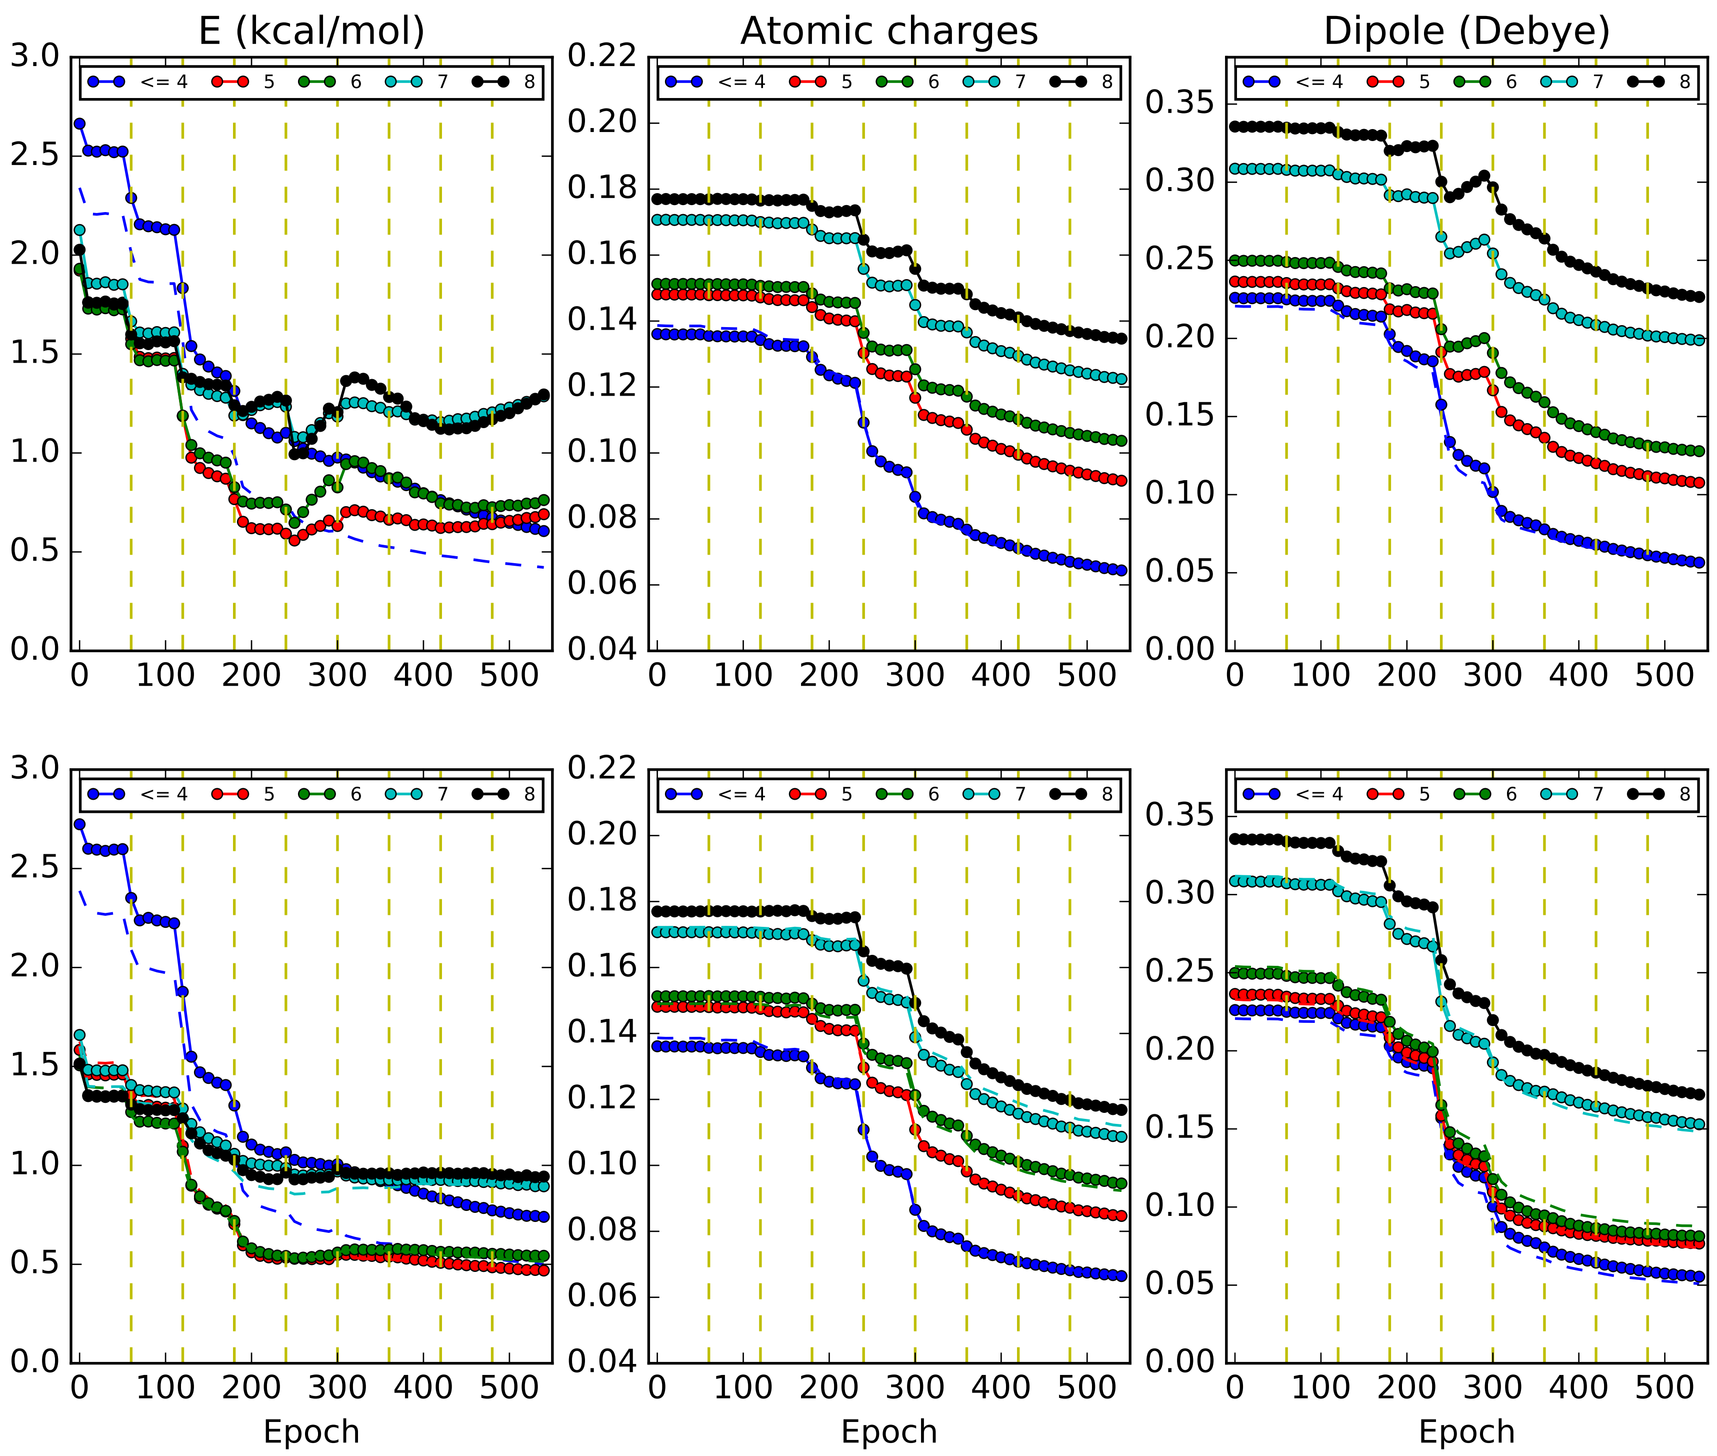

Figure S40 H Diag: DFTB MIO H Off Diag: DFTB MIO
G Diag: DFTB MIO G Off Diag: FFNN 1 Repulsive: Spline

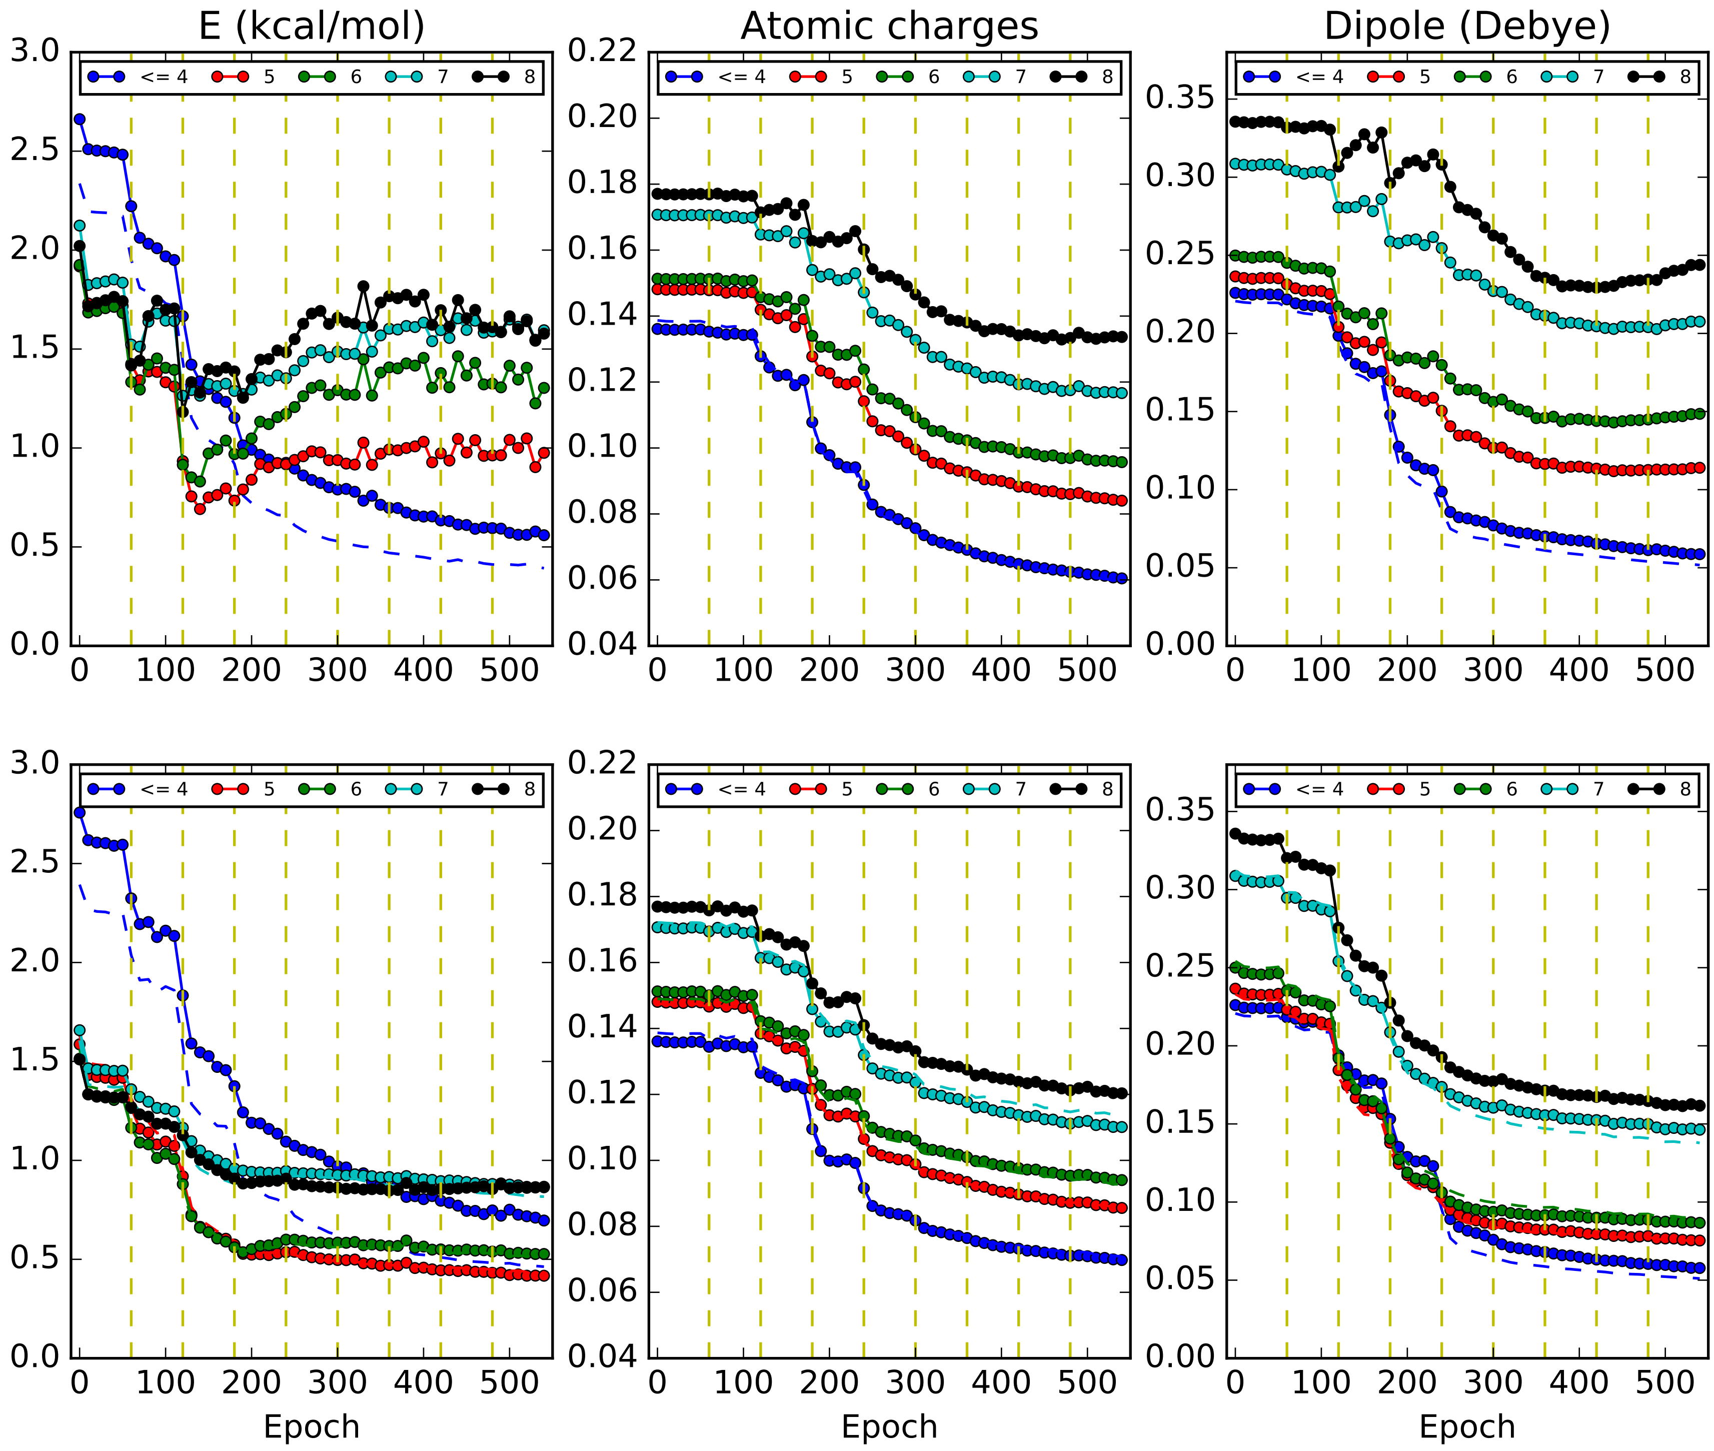

Figure S41 H Diag: FFNN 2 H Off Diag: FFNN 2
G Diag: FFNN 2 G Off Diag: FFNN 2 Repulsive: Spline

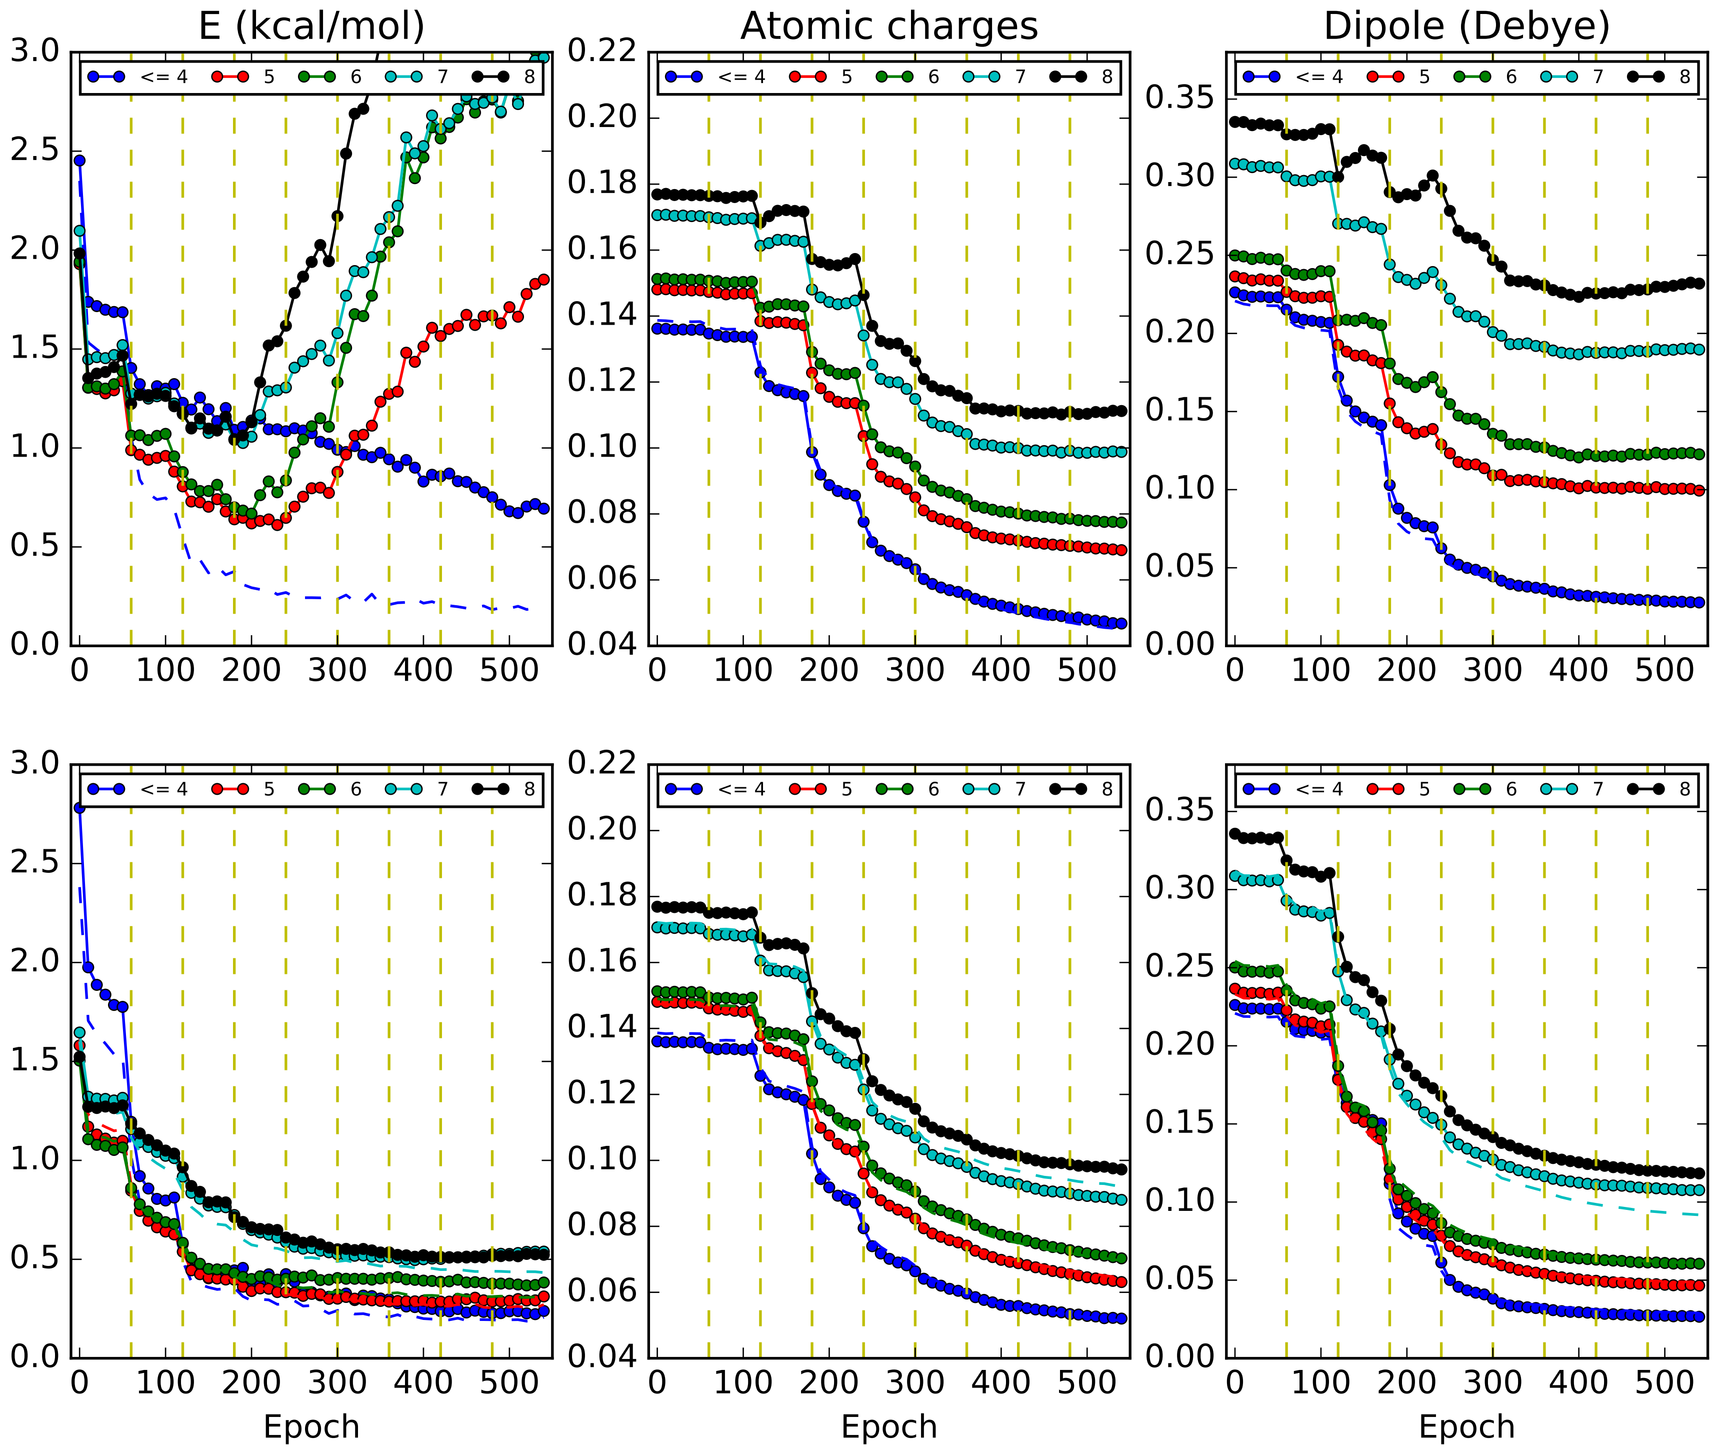

Figure S42 H Diag: FFNN 3 H Off Diag: FFNN 3
G Diag: FFNN 3 G Off Diag: FFNN 3 Repulsive: Spline

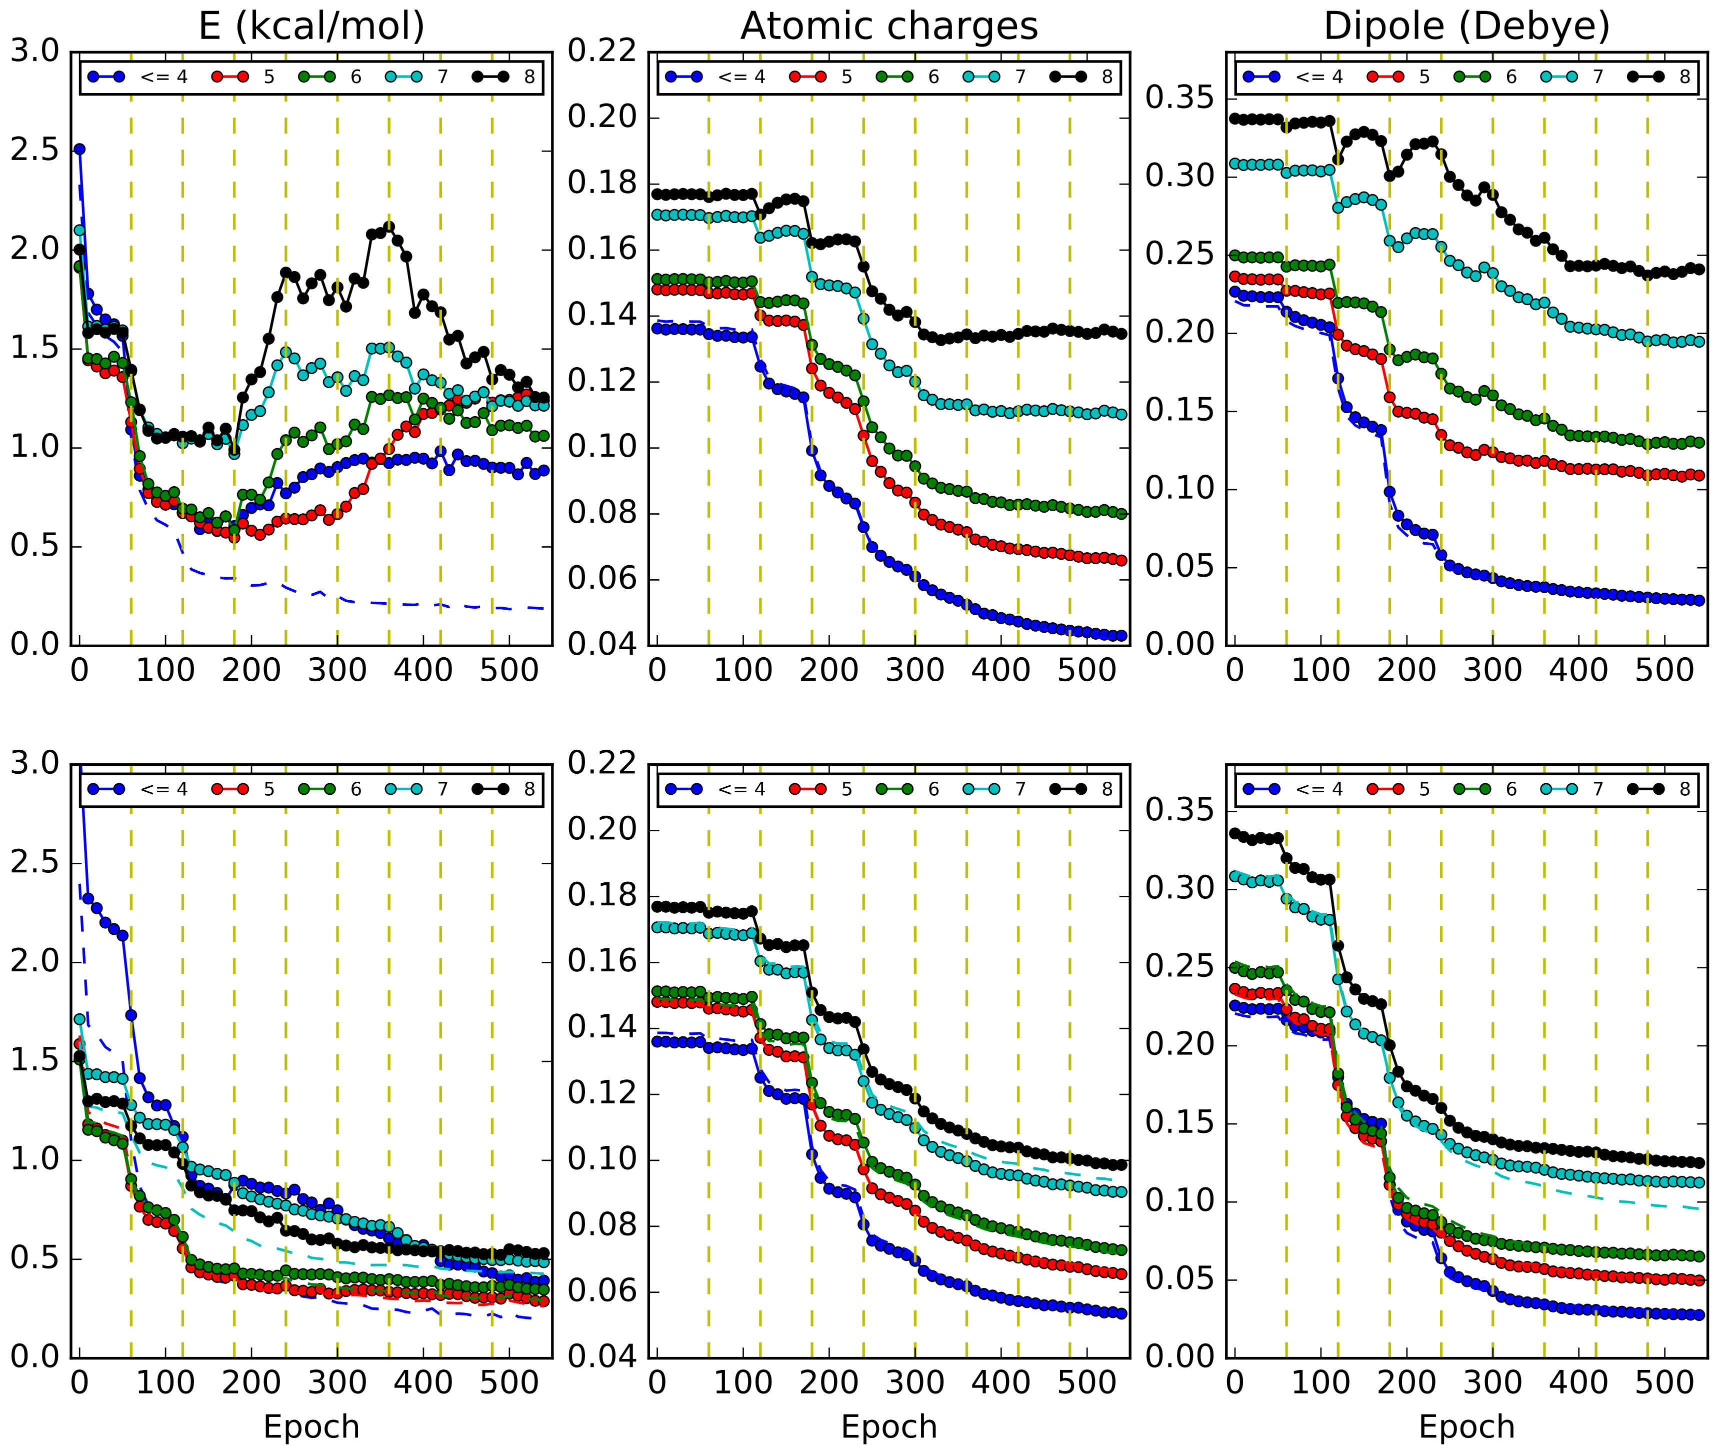

Figure S43 H Diag: FFNN 4 H Off Diag: FFNN 4
G Diag: FFNN 4 G Off Diag: FFNN 4 Repulsive: Spline

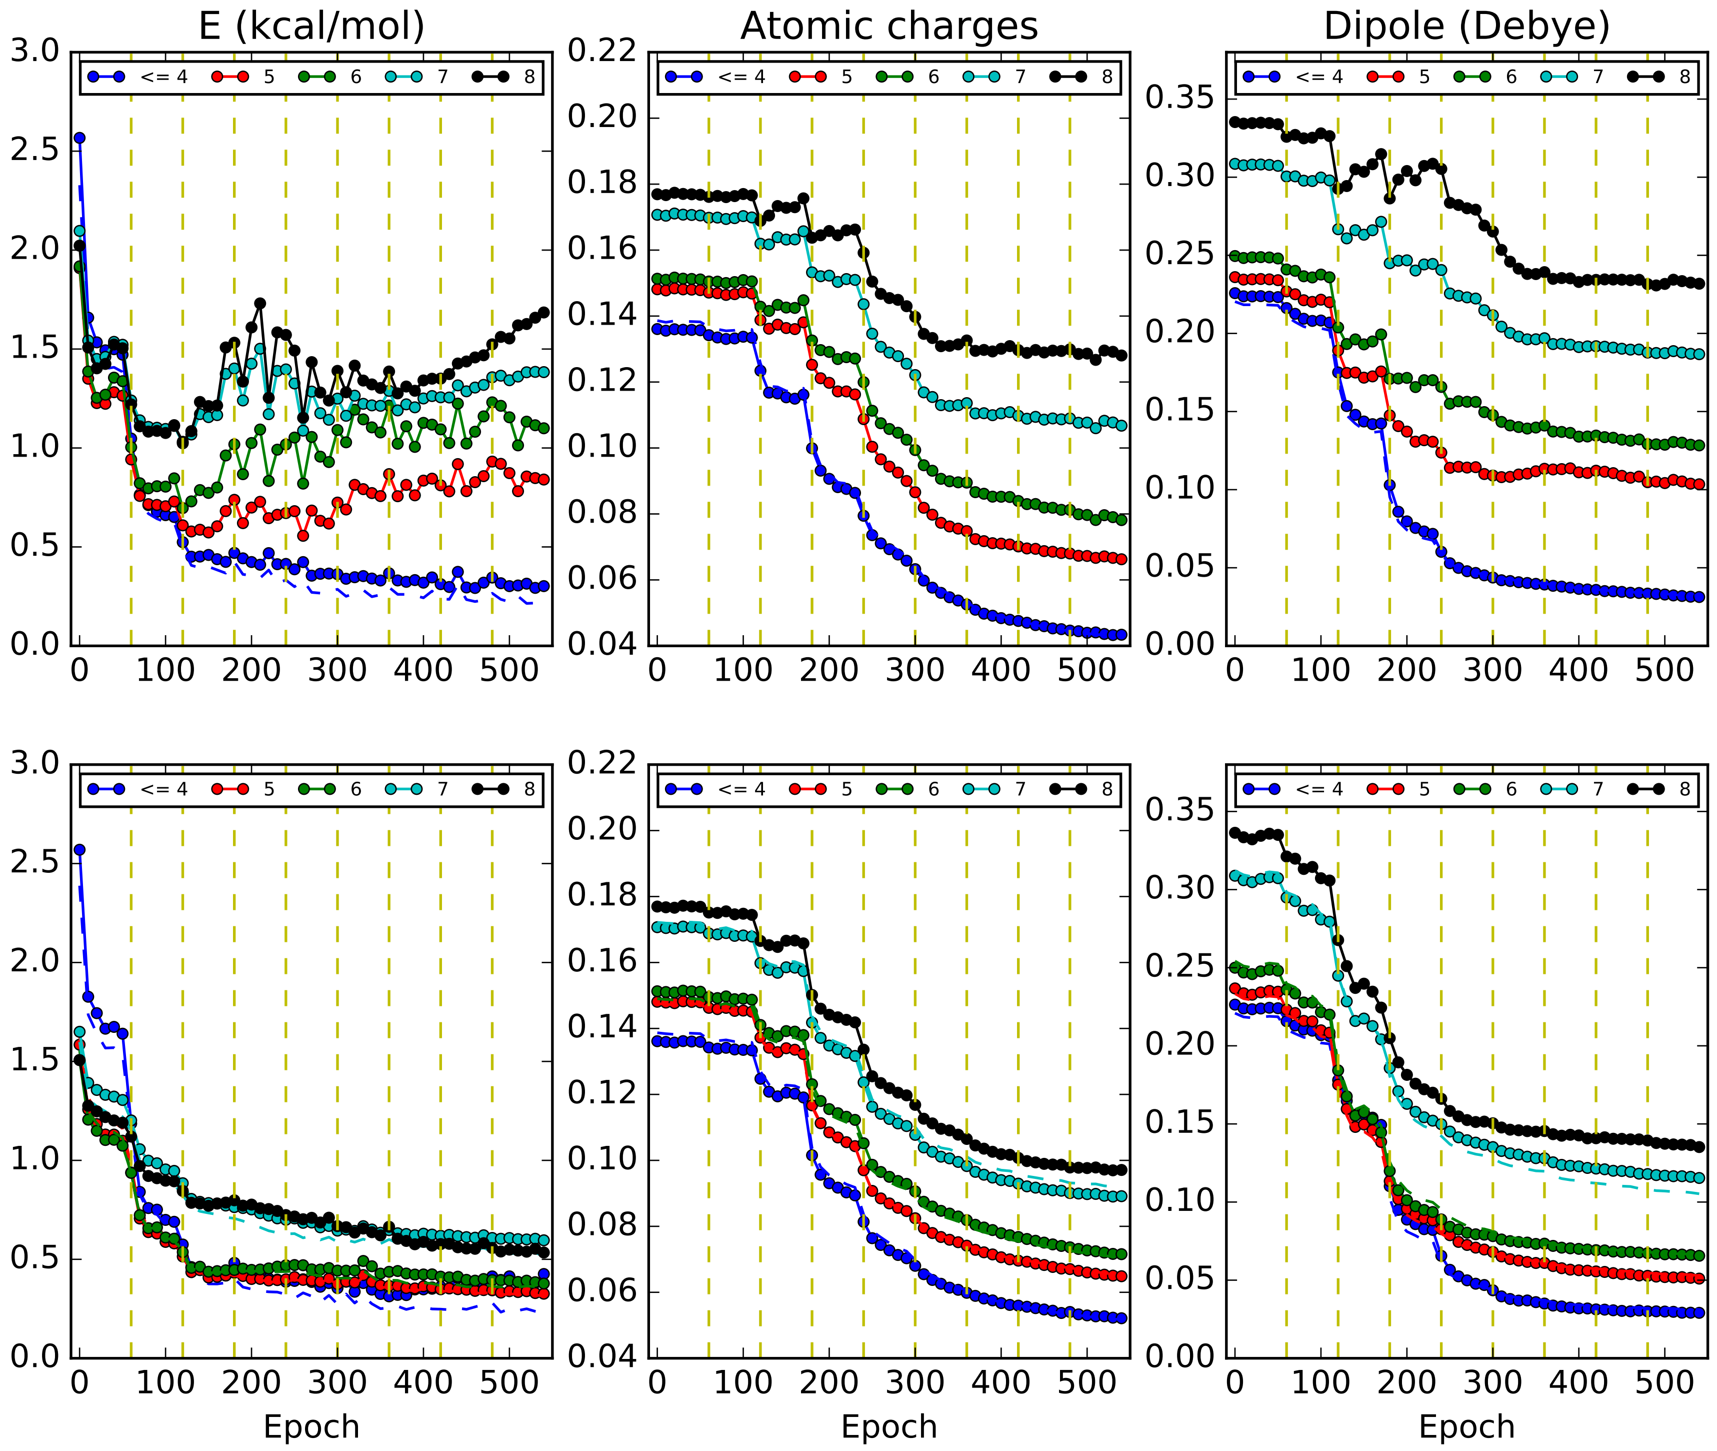

Figure S44 H Diag: FFNN 5 H Off Diag: FFNN 5
G Diag: FFNN 5 G Off Diag: FFNN 5 Repulsive: Spline

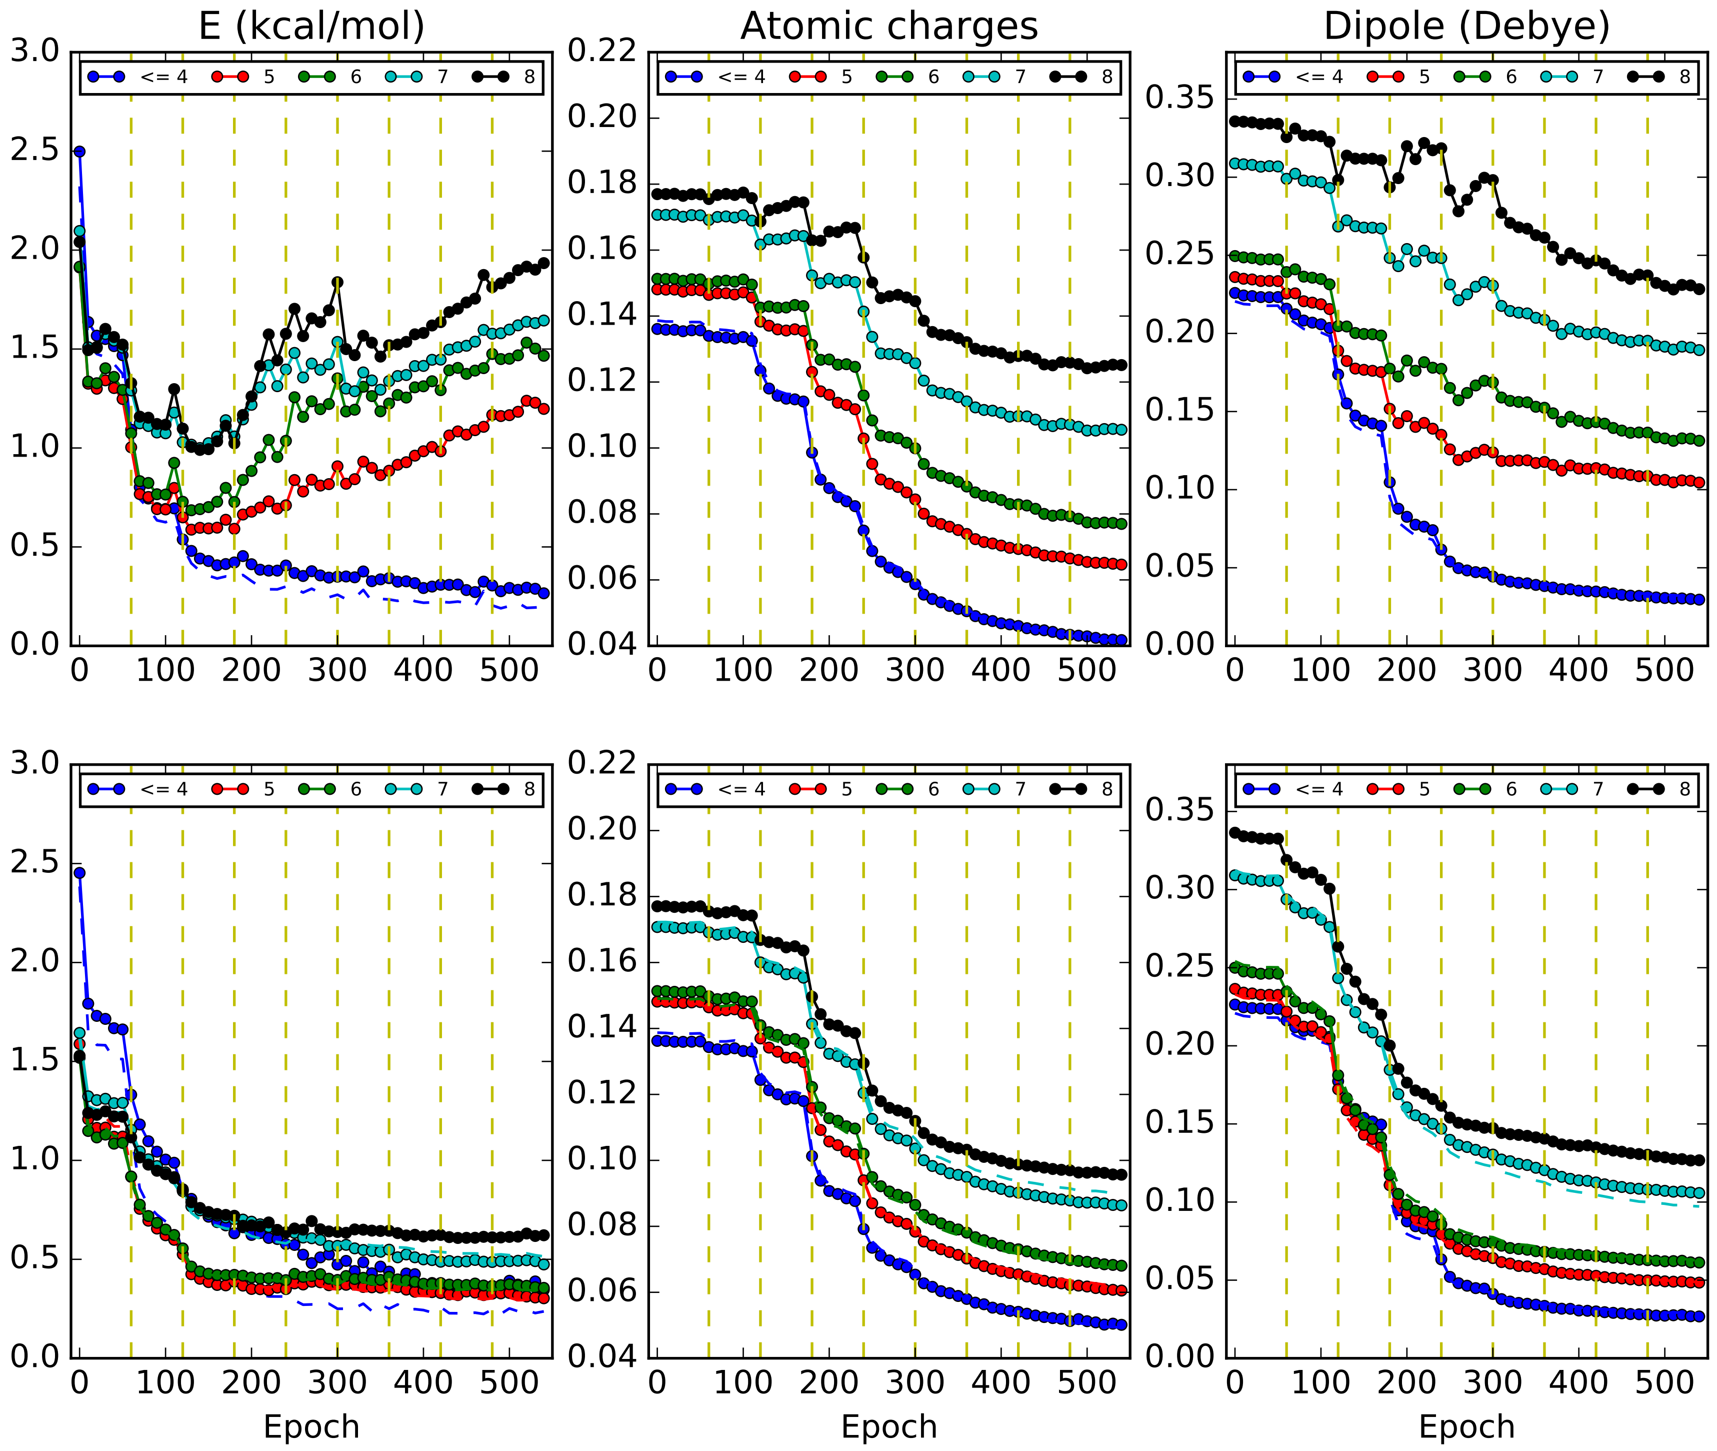

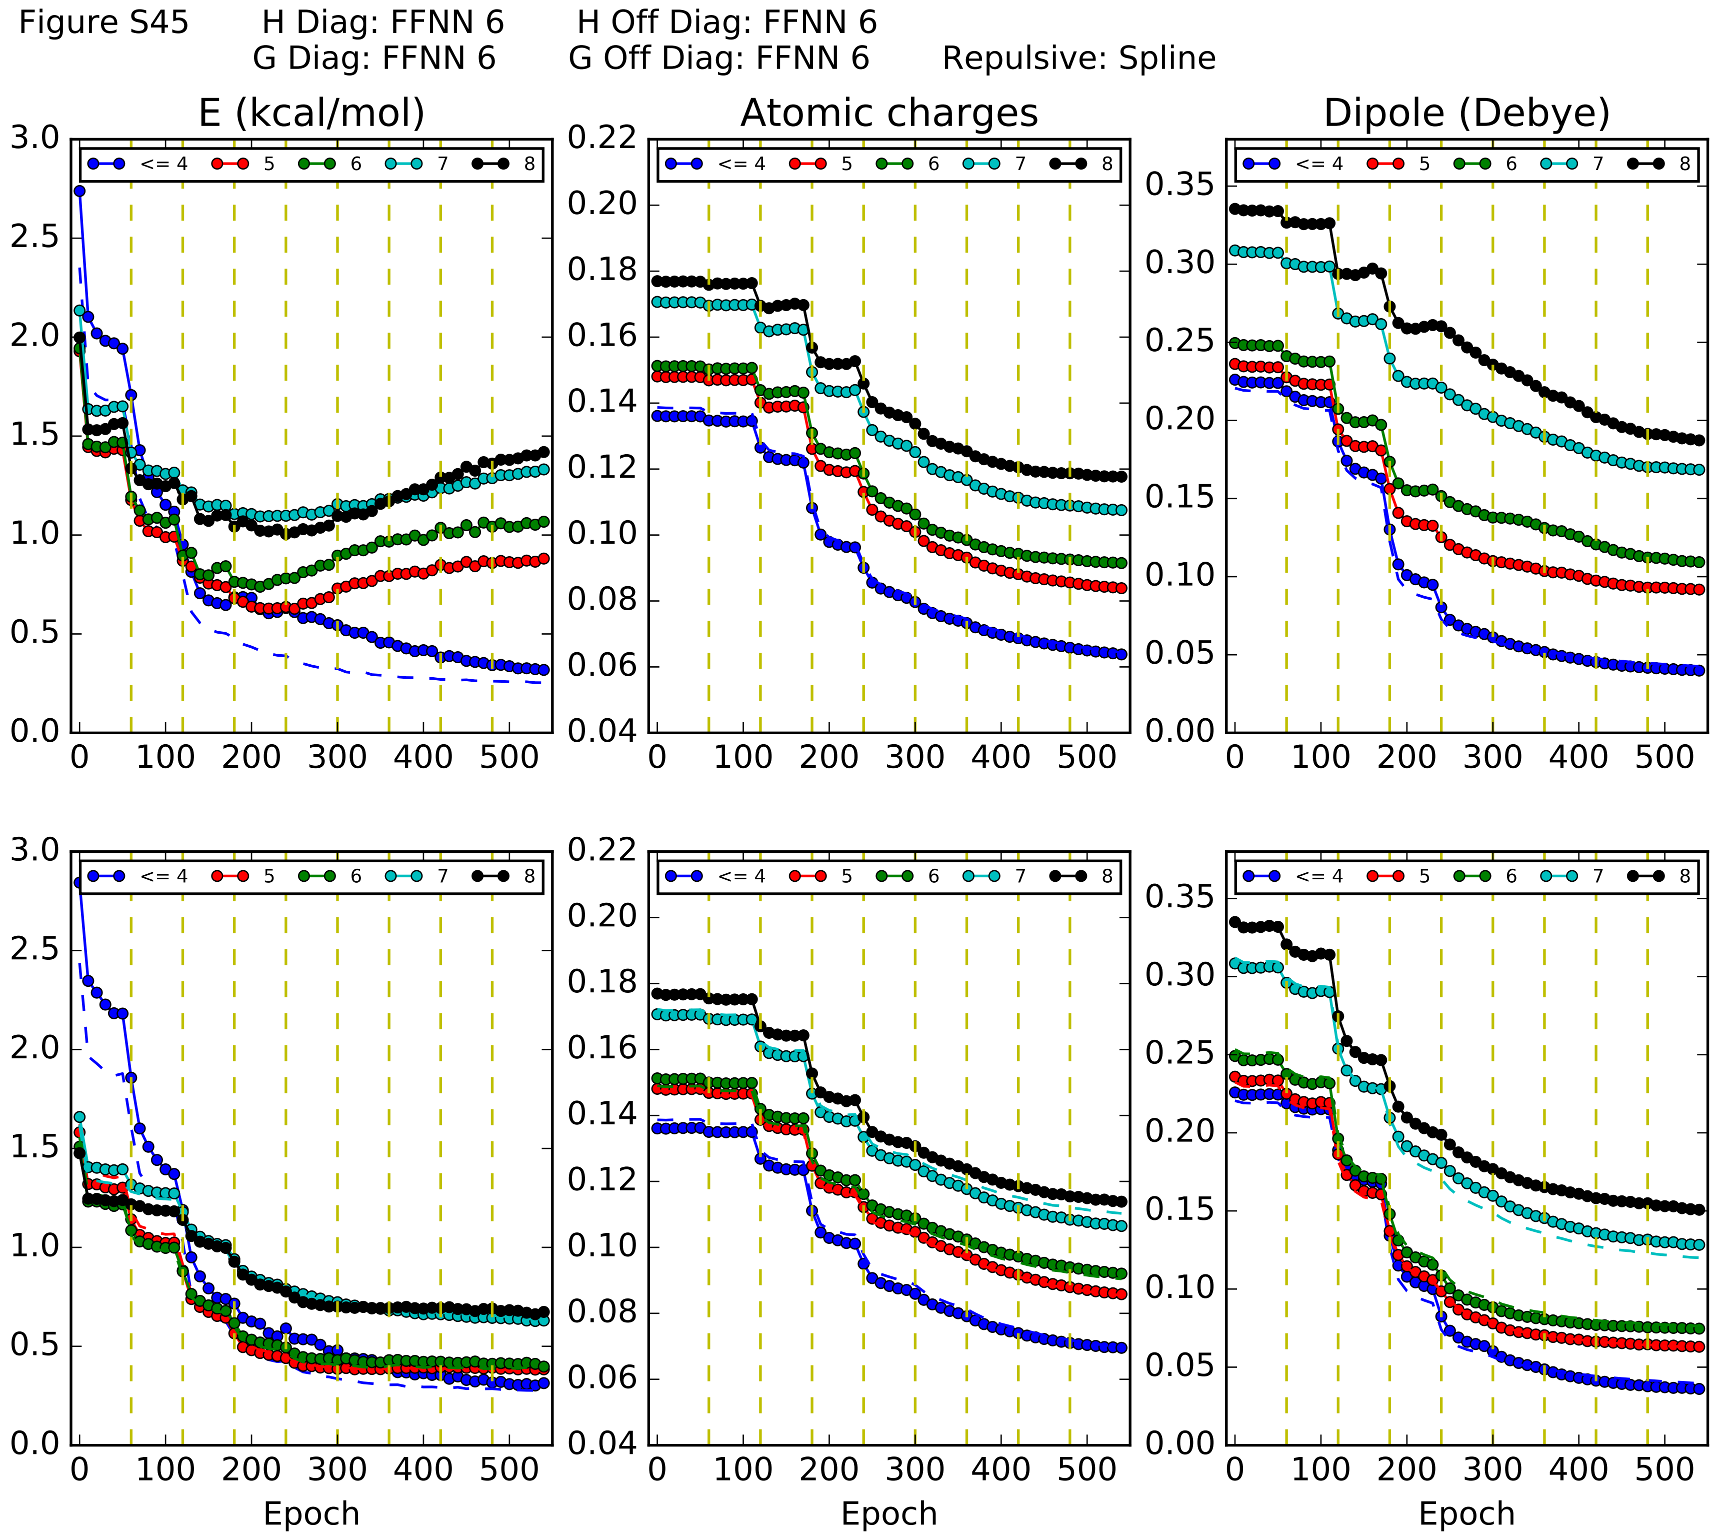

Figure S45 H Diag: FFNN 6 H Off Diag: FFNN 6
G Diag: FFNN 6 G Off Diag: FFNN 6 Repulsive: Spline
E (kcal/mol)
Atomic charges
Dipole (Debye)
<= 4
5
6
7
8
Epoch

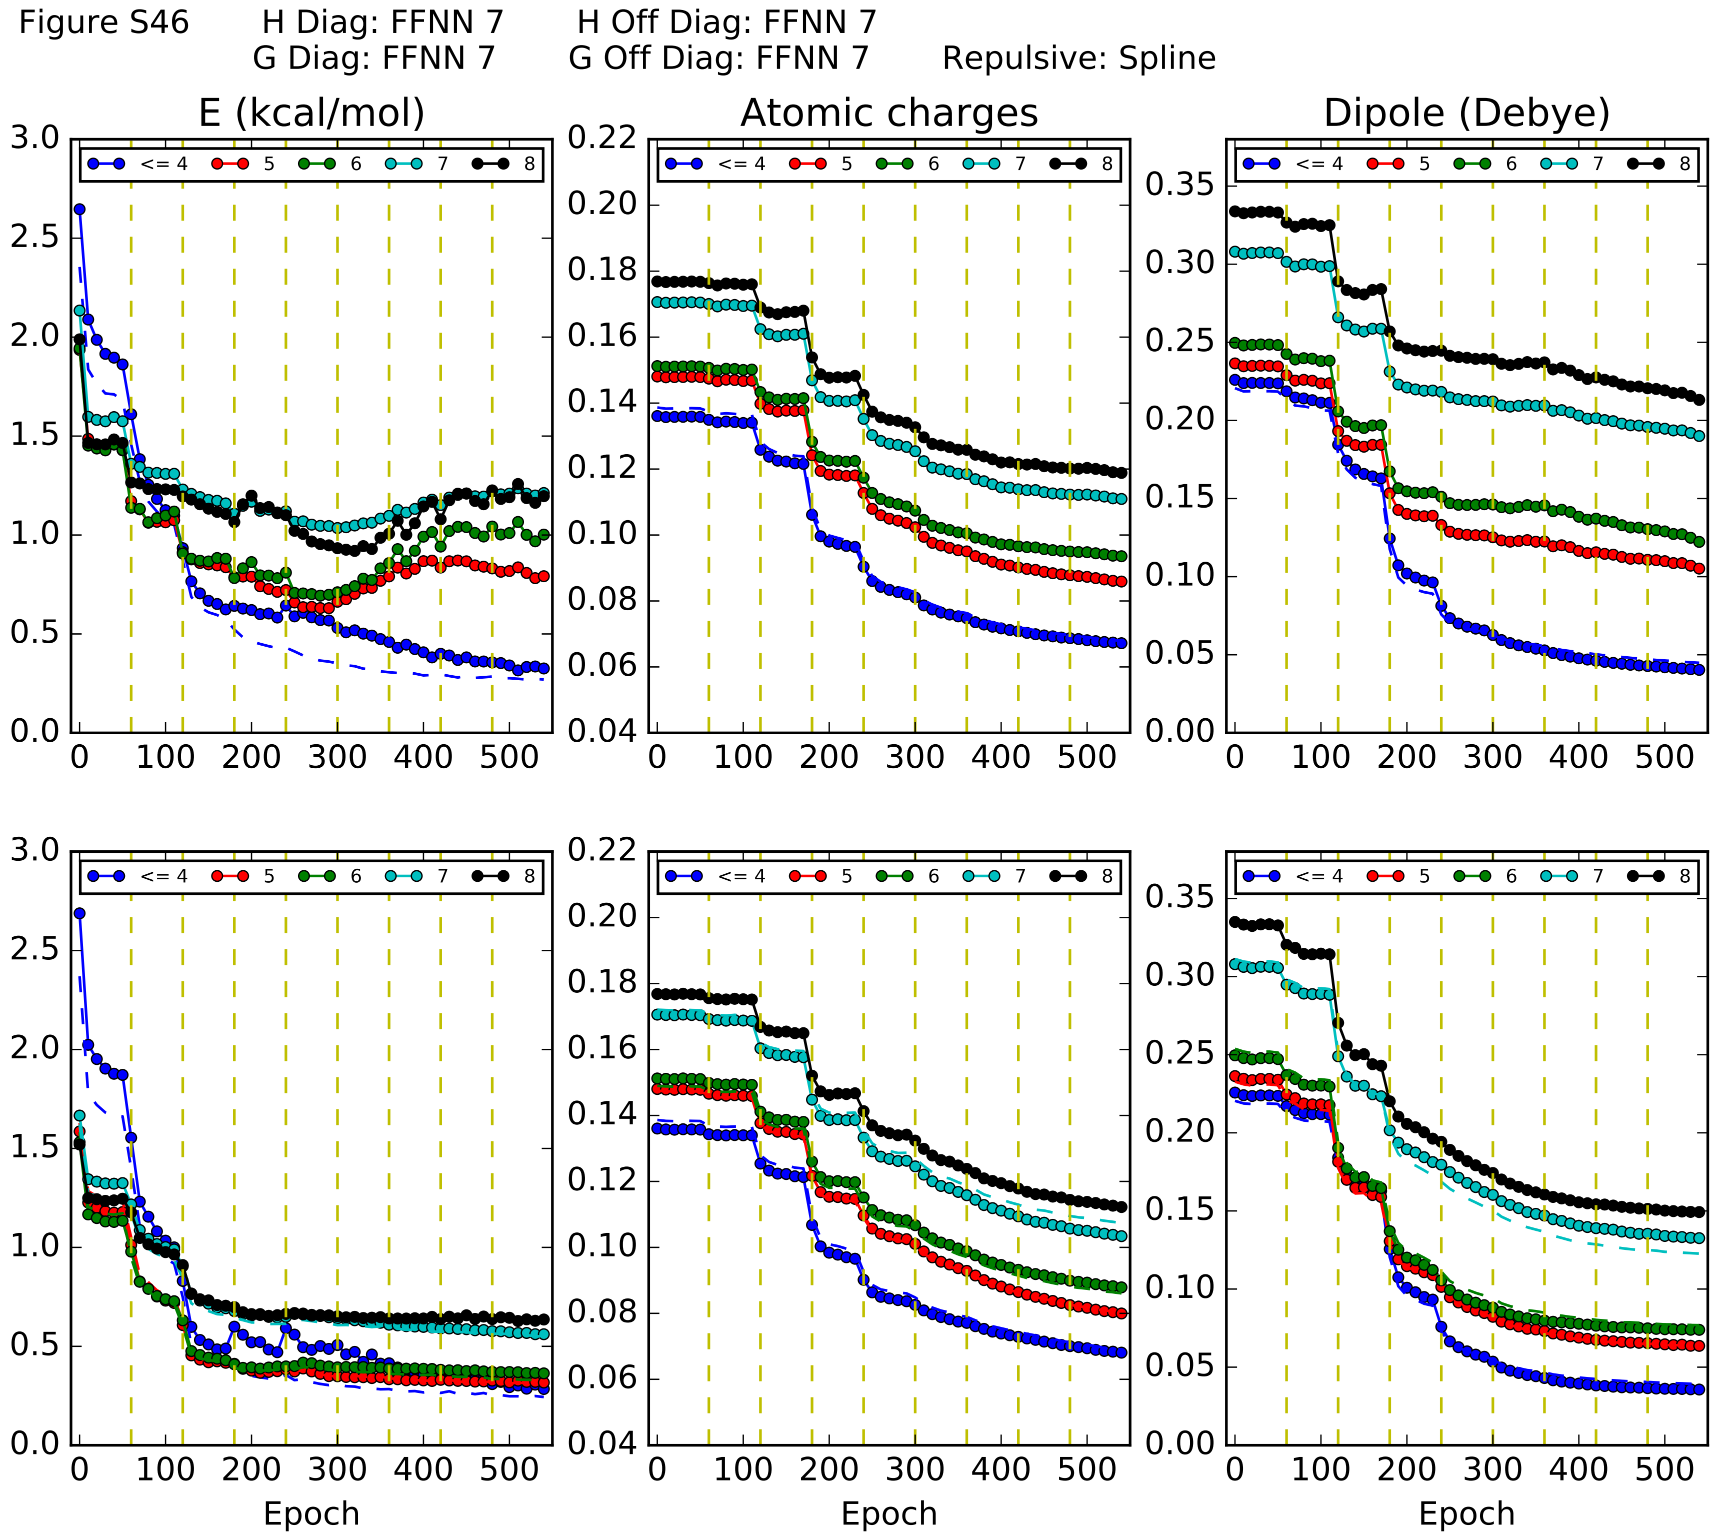
Figure S46
H Diag: FFNN 7
H Off Diag: FFNN 7
G Diag: FFNN 7
G Off Diag: FFNN 7
Repulsive: Spline
E (kcal/mol)
Atomic charges
Dipole (Debye)
<= 4
5
6
7
8
Epoch

Figure S47 H Diag: FFNN 8 H Off Diag: FFNN 8
G Diag: FFNN 8 G Off Diag: FFNN 8 Repulsive: Spline

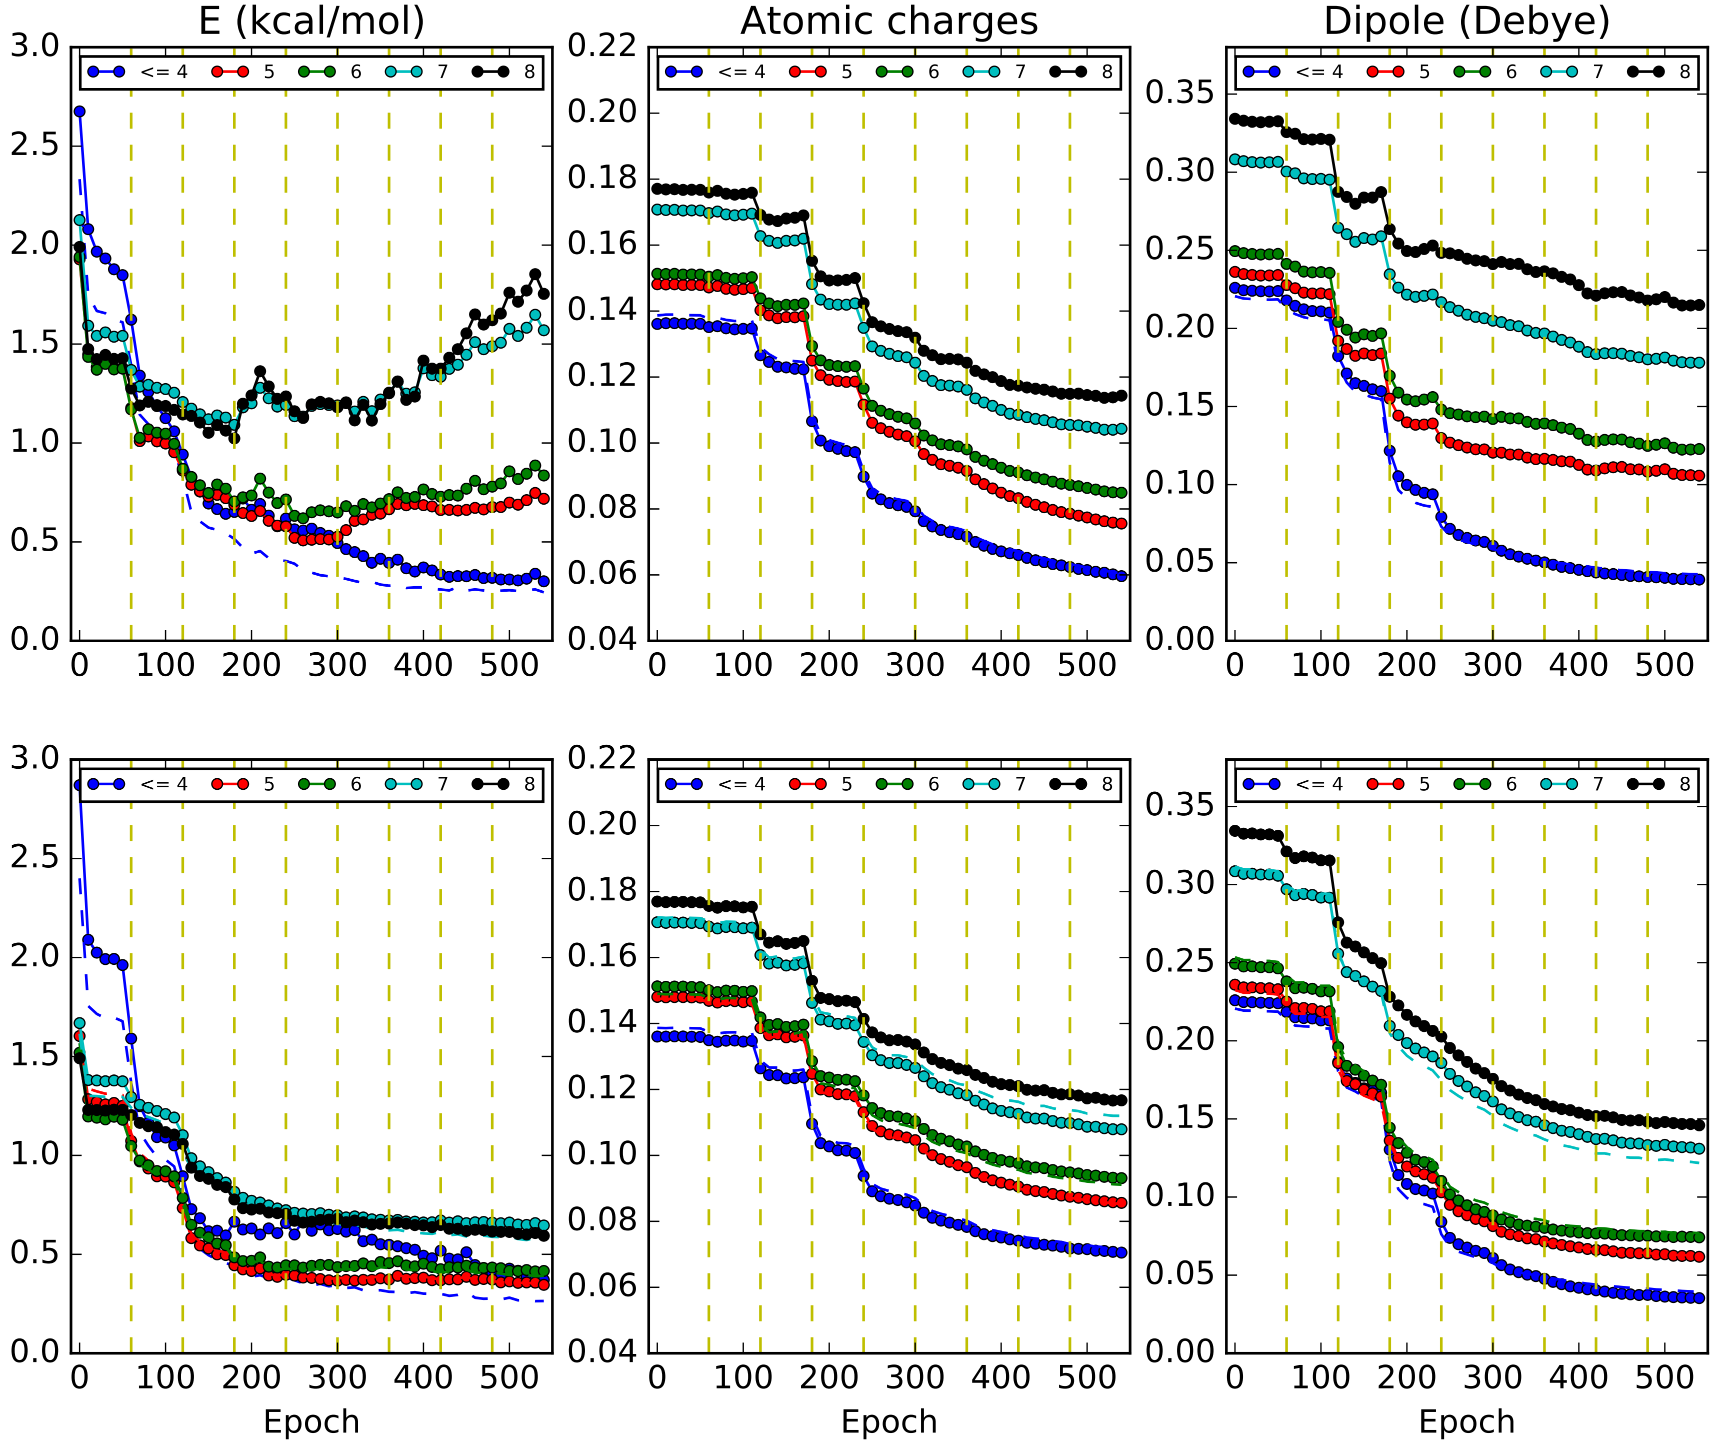

Figure S48 H Diag: FFNN 9 H Off Diag: FFNN 9
G Diag: FFNN 9 G Off Diag: FFNN 9 Repulsive: Spline

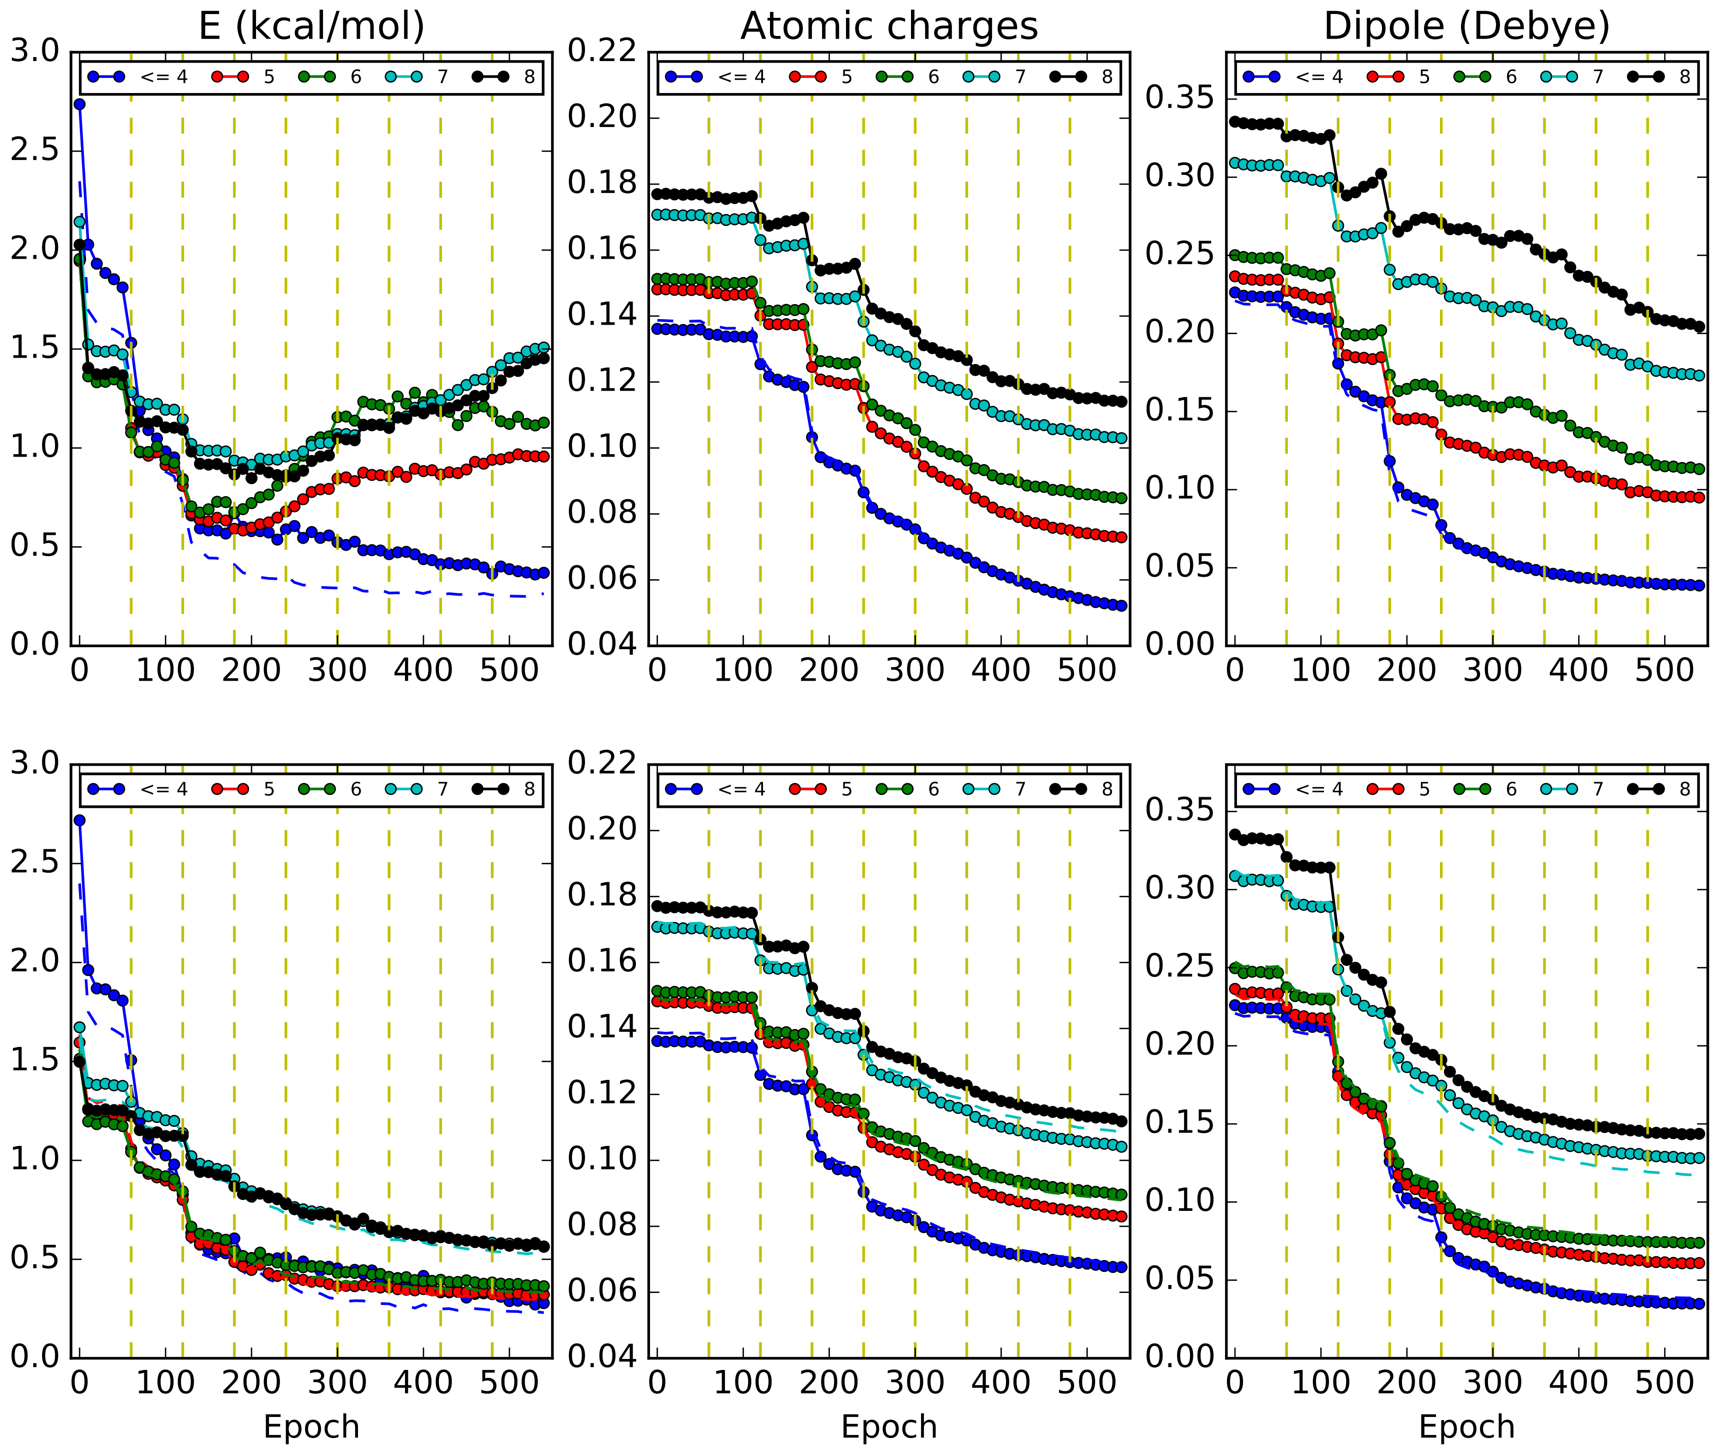

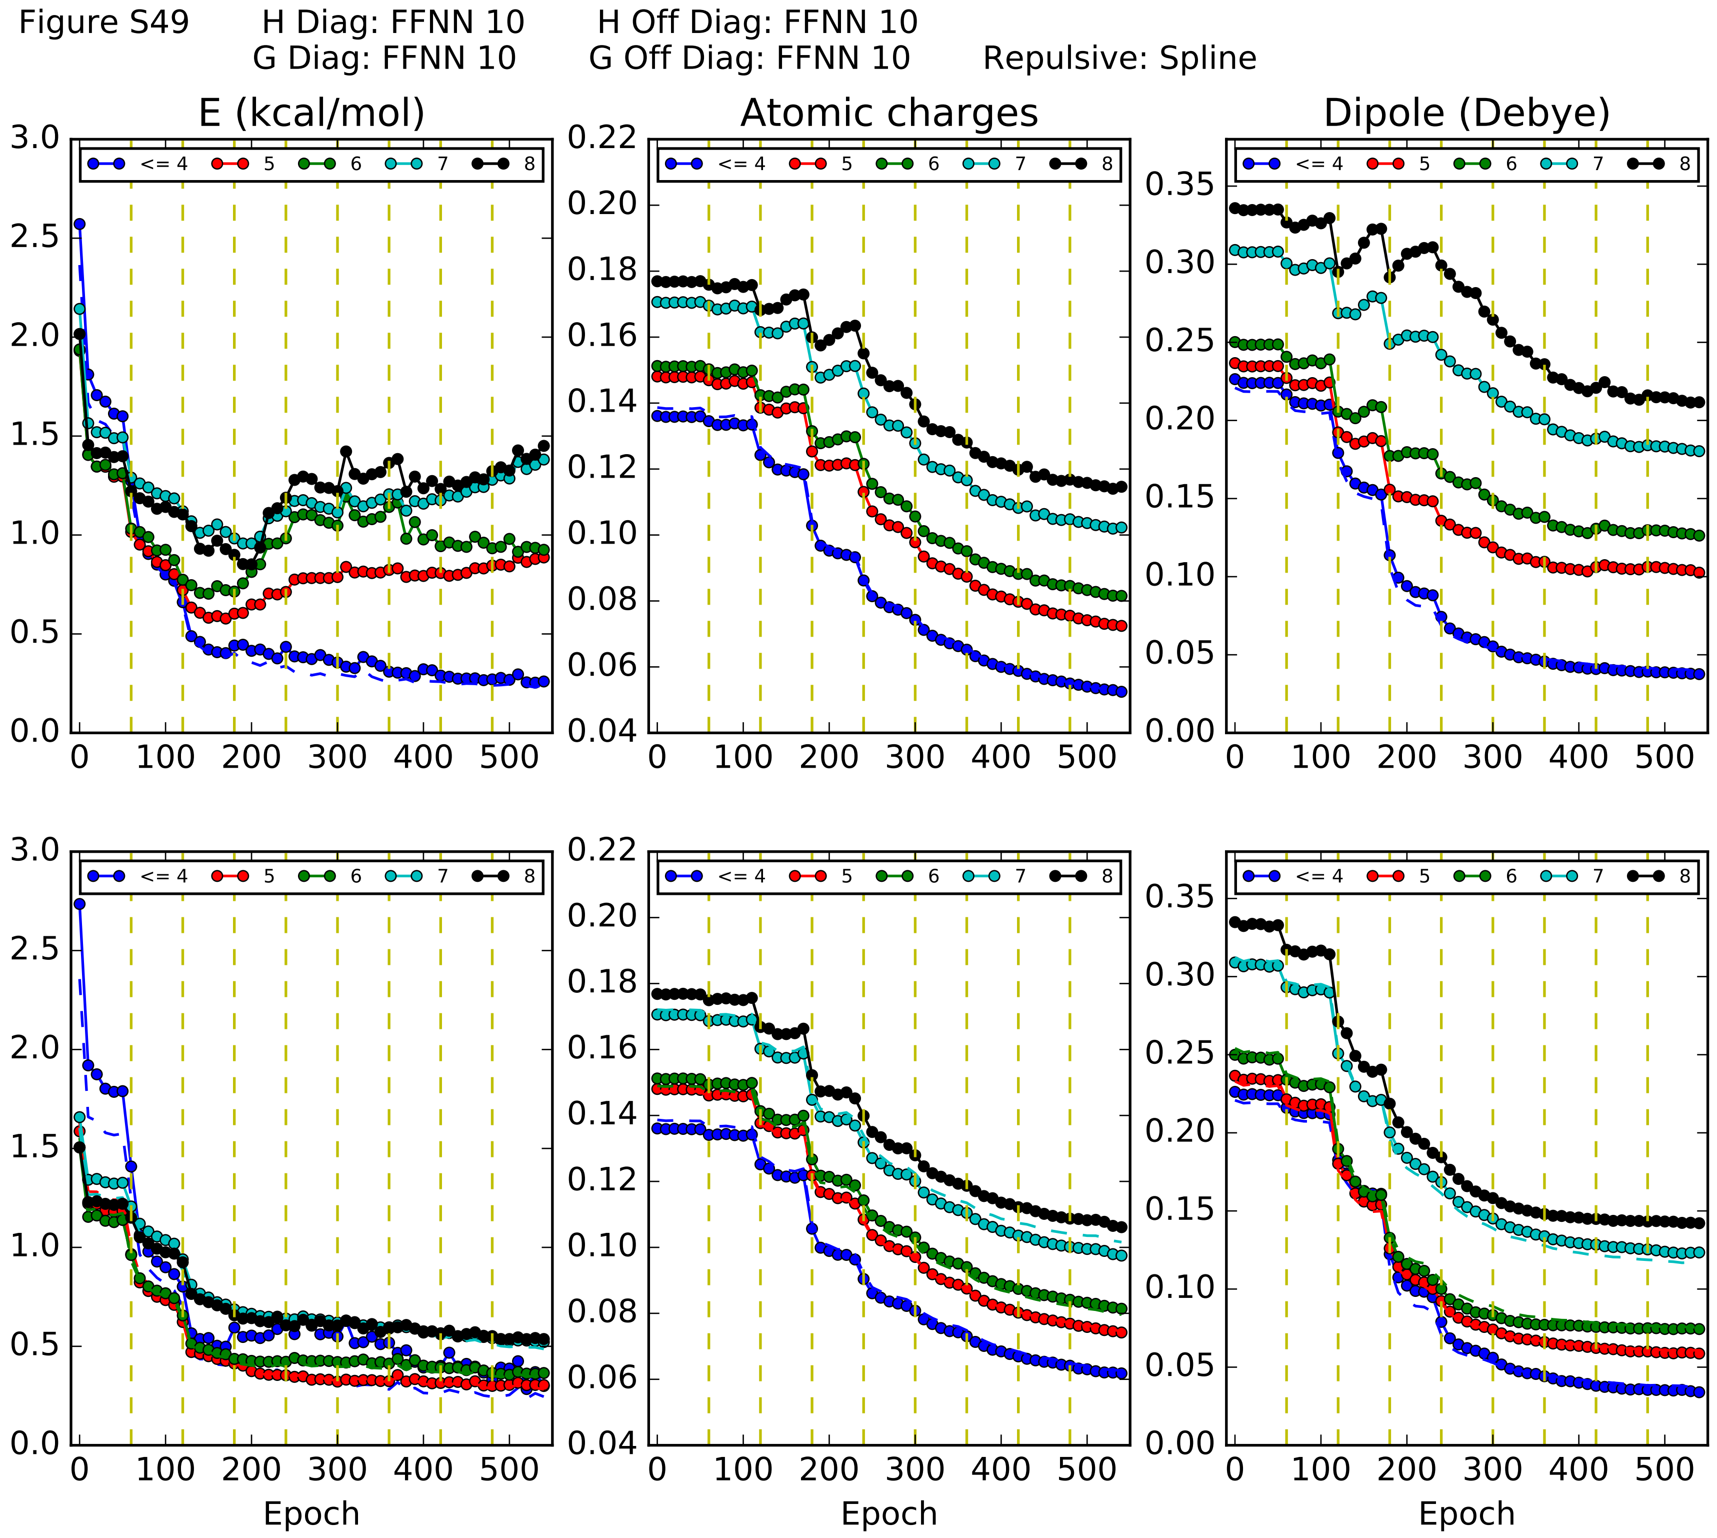
Figure S49
H Diag: FFNN 10
H Off Diag: FFNN 10
G Diag: FFNN 10
G Off Diag: FFNN 10
Repulsive: Spline
E (kcal/mol)
Atomic charges
Dipole (Debye)
<= 4
5
6
7
8
Epoch

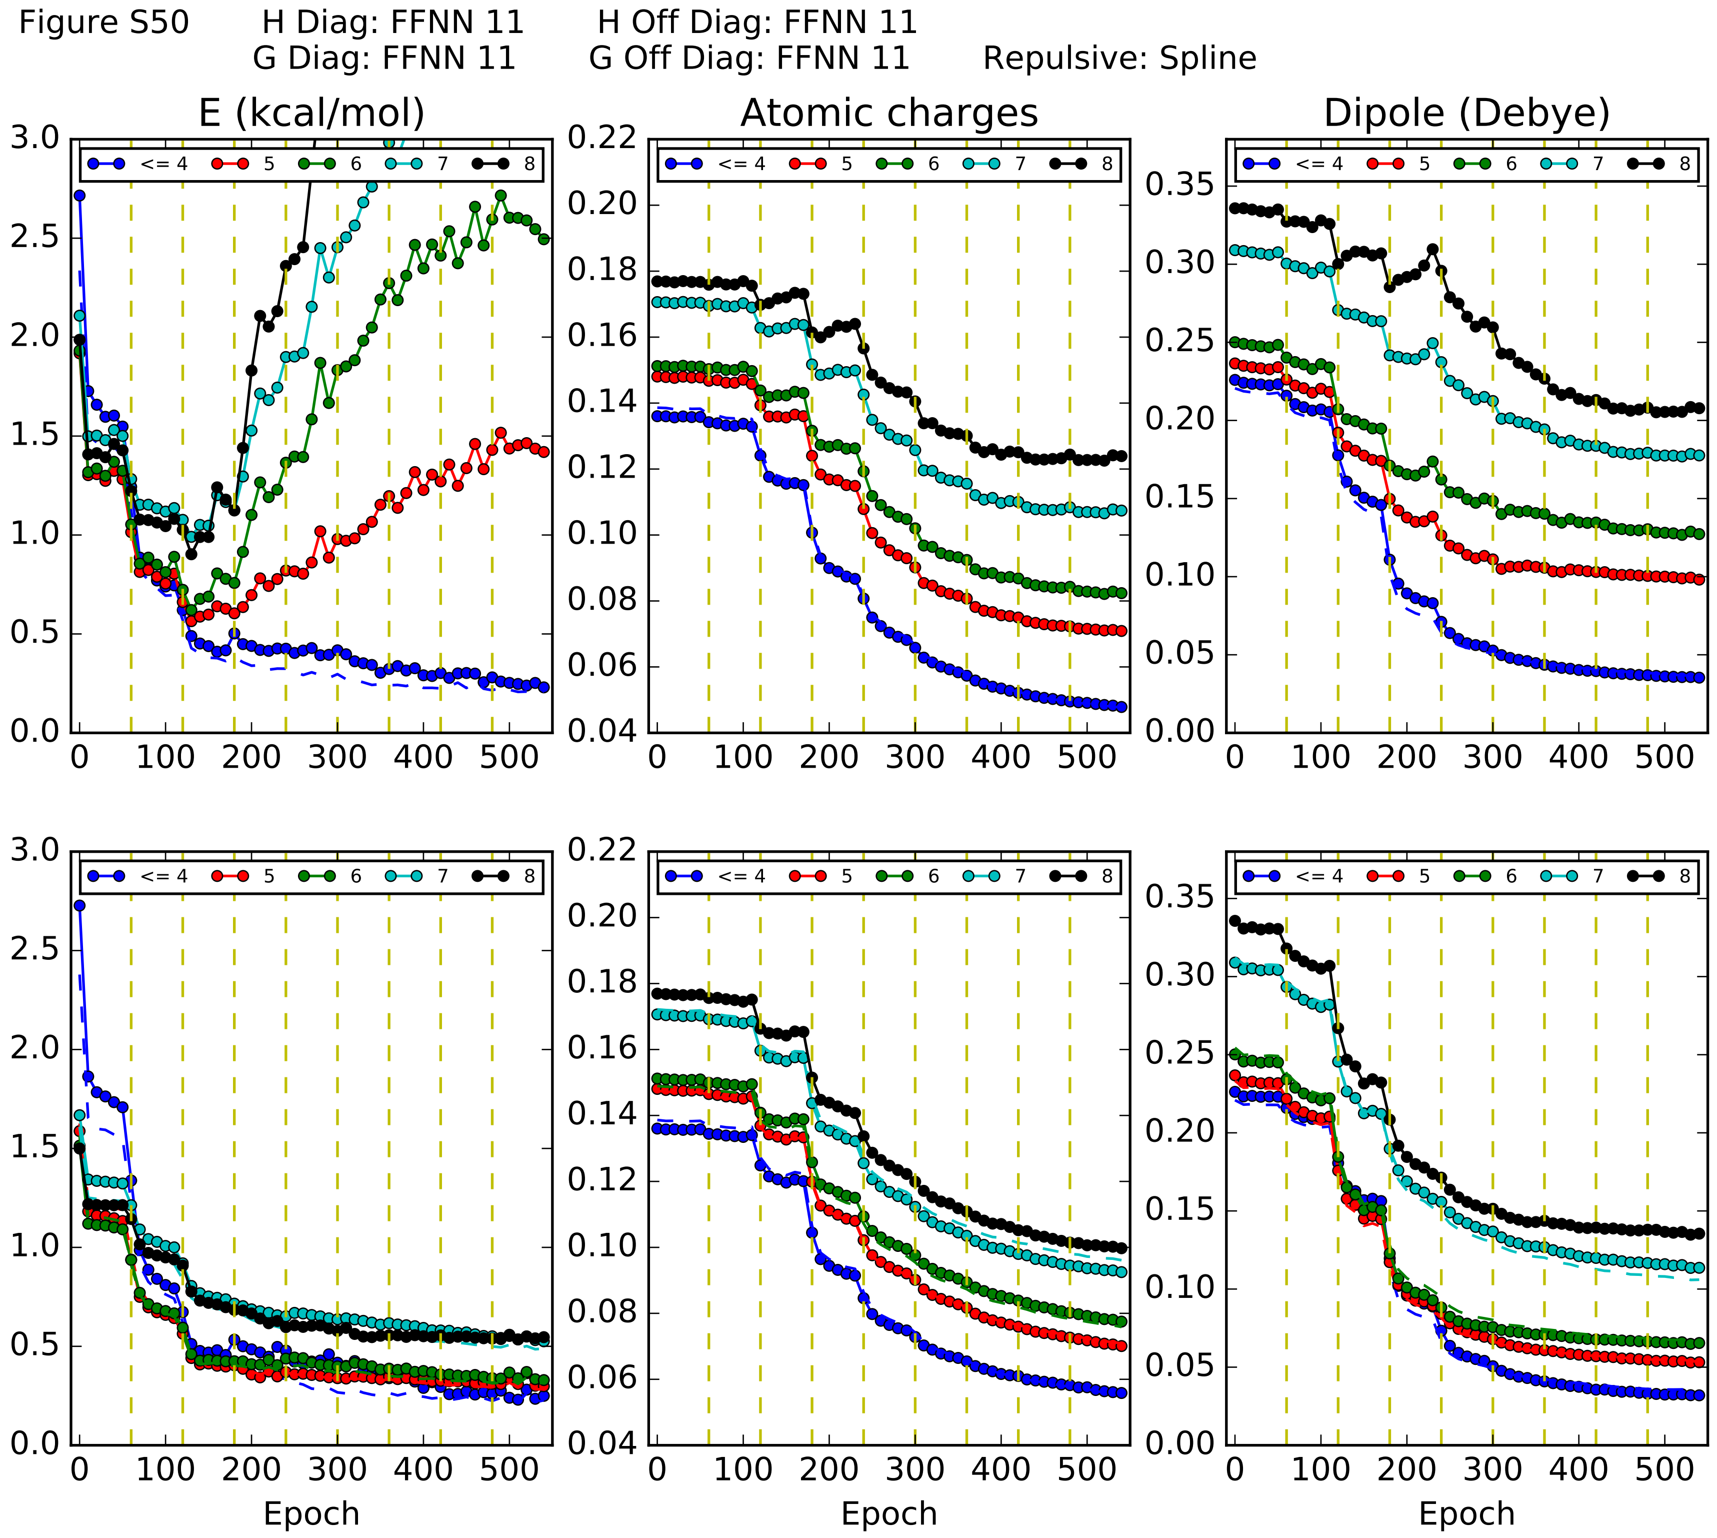

Figure S50
H Diag: FFNN 11
H Off Diag: FFNN 11
G Diag: FFNN 11
G Off Diag: FFNN 11
Repulsive: Spline
E (kcal/mol)
Atomic charges
Dipole (Debye)
<= 4
5
6
7
8
Epoch

Figure S51 H Diag: FFNN 12 H Off Diag: FFNN 12
G Diag: FFNN 12 G Off Diag: FFNN 12 Repulsive: Spline

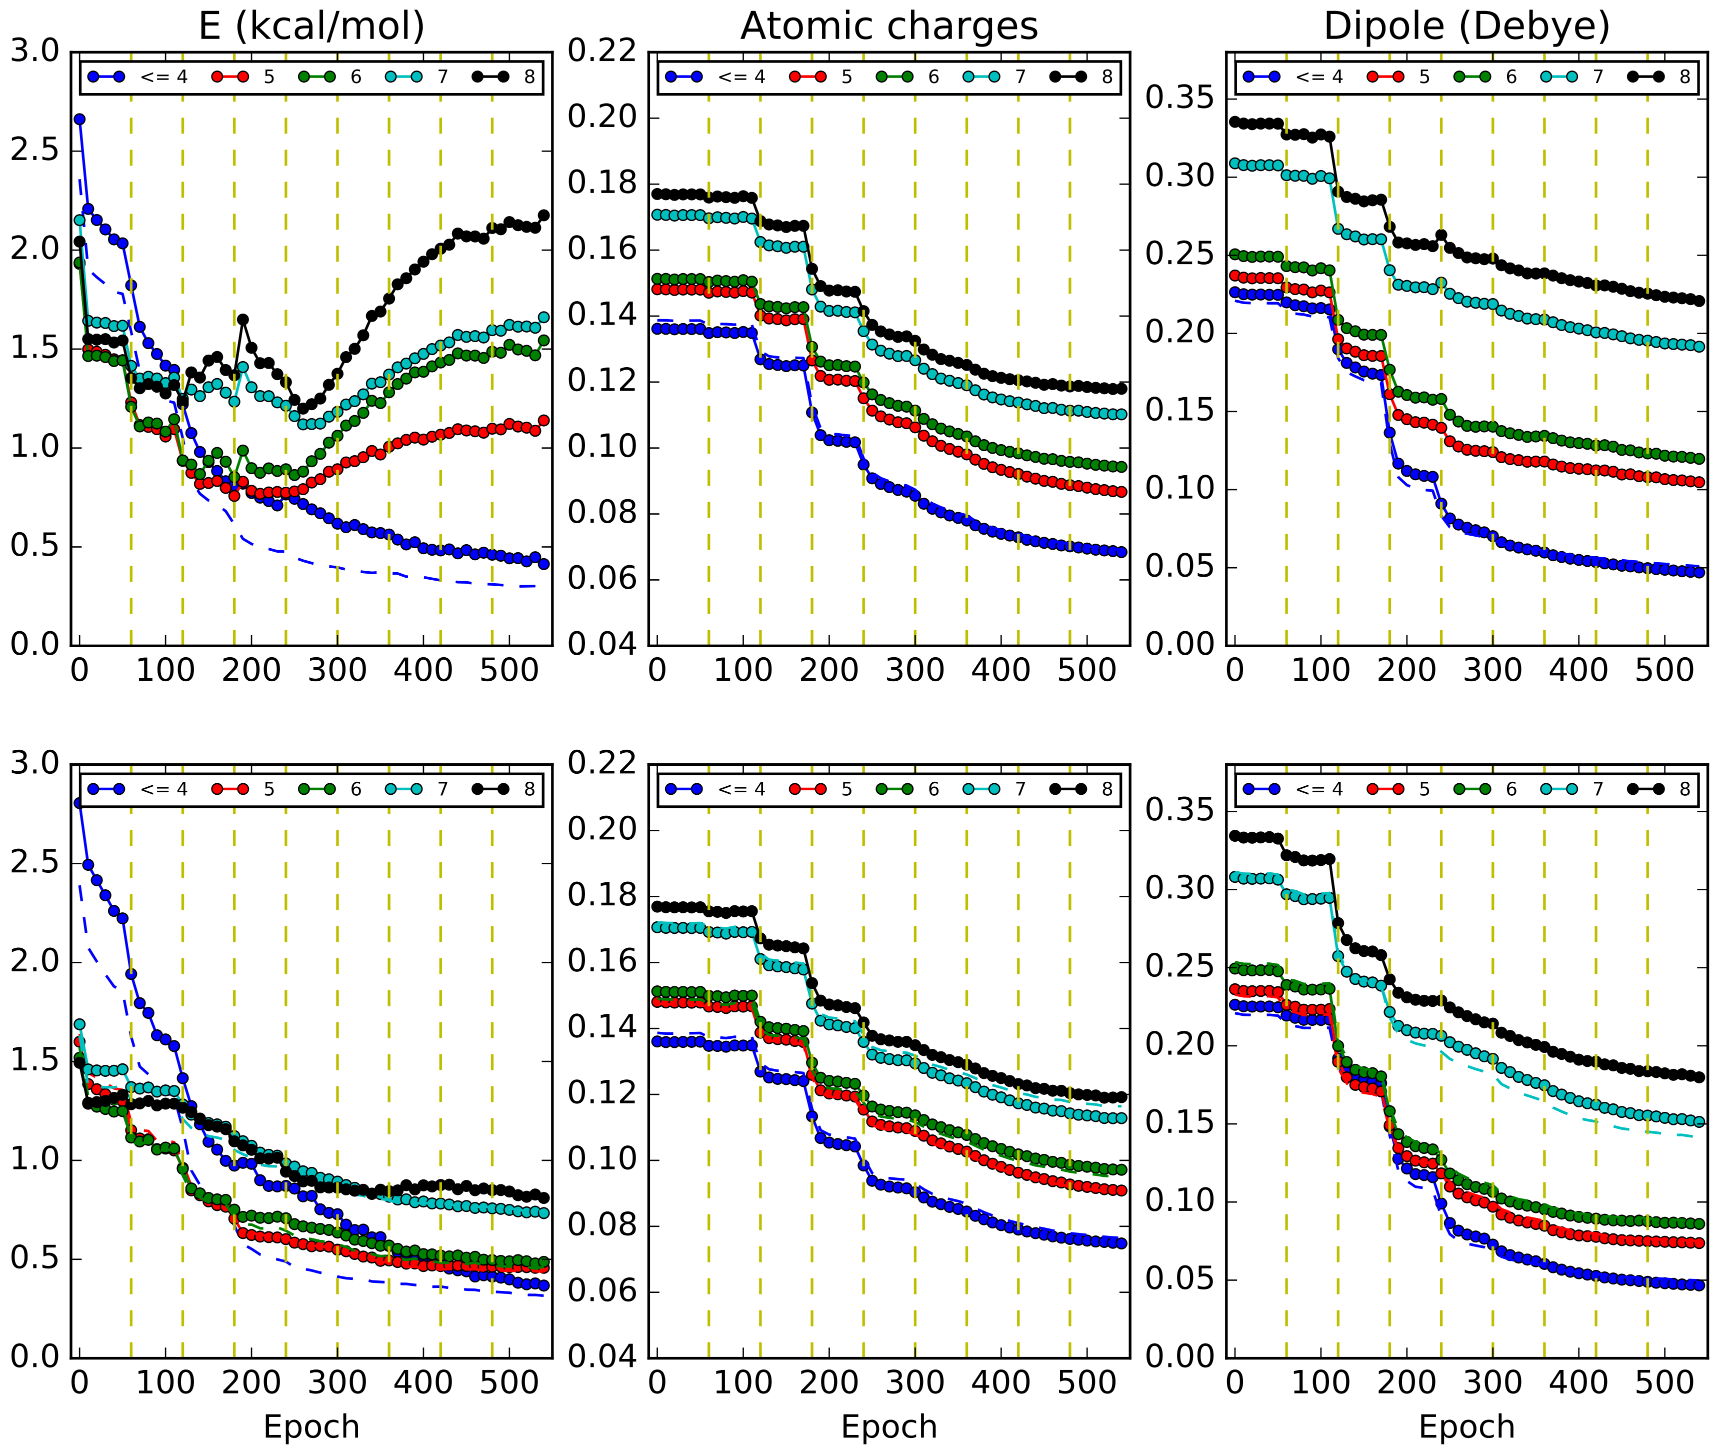

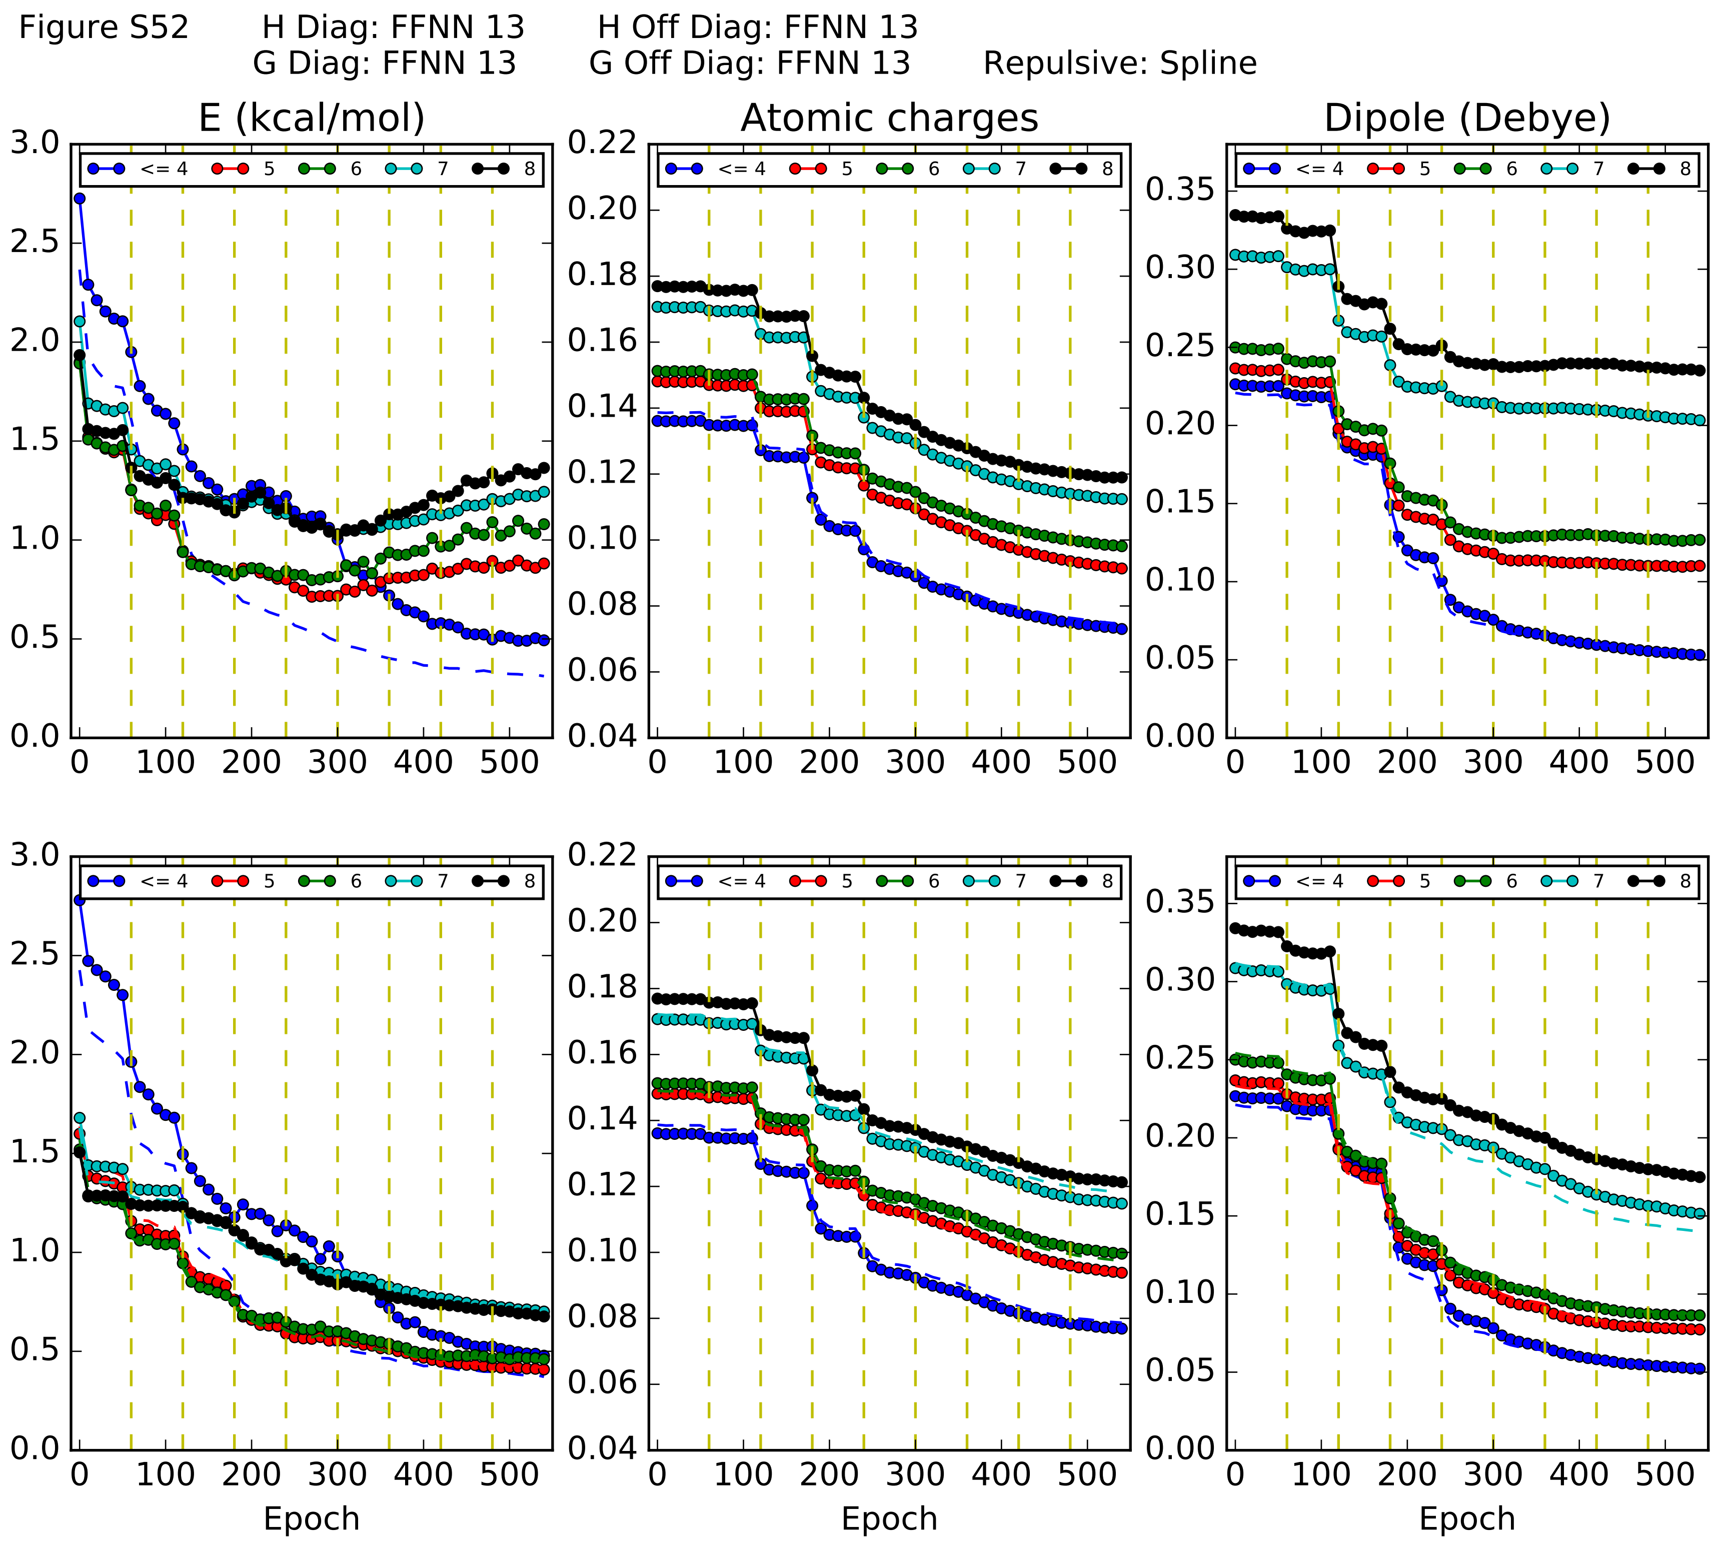
Figure S52
H Diag: FFNN 13
H Off Diag: FFNN 13
G Diag: FFNN 13
G Off Diag: FFNN 13
Repulsive: Spline
E (kcal/mol)
Atomic charges
Dipole (Debye)
<= 4
5
6
7
8
Epoch

Figure S53 H Diag: FFNN 14 H Off Diag: FFNN 14
G Diag: FFNN 14 G Off Diag: FFNN 14 Repulsive: Spline

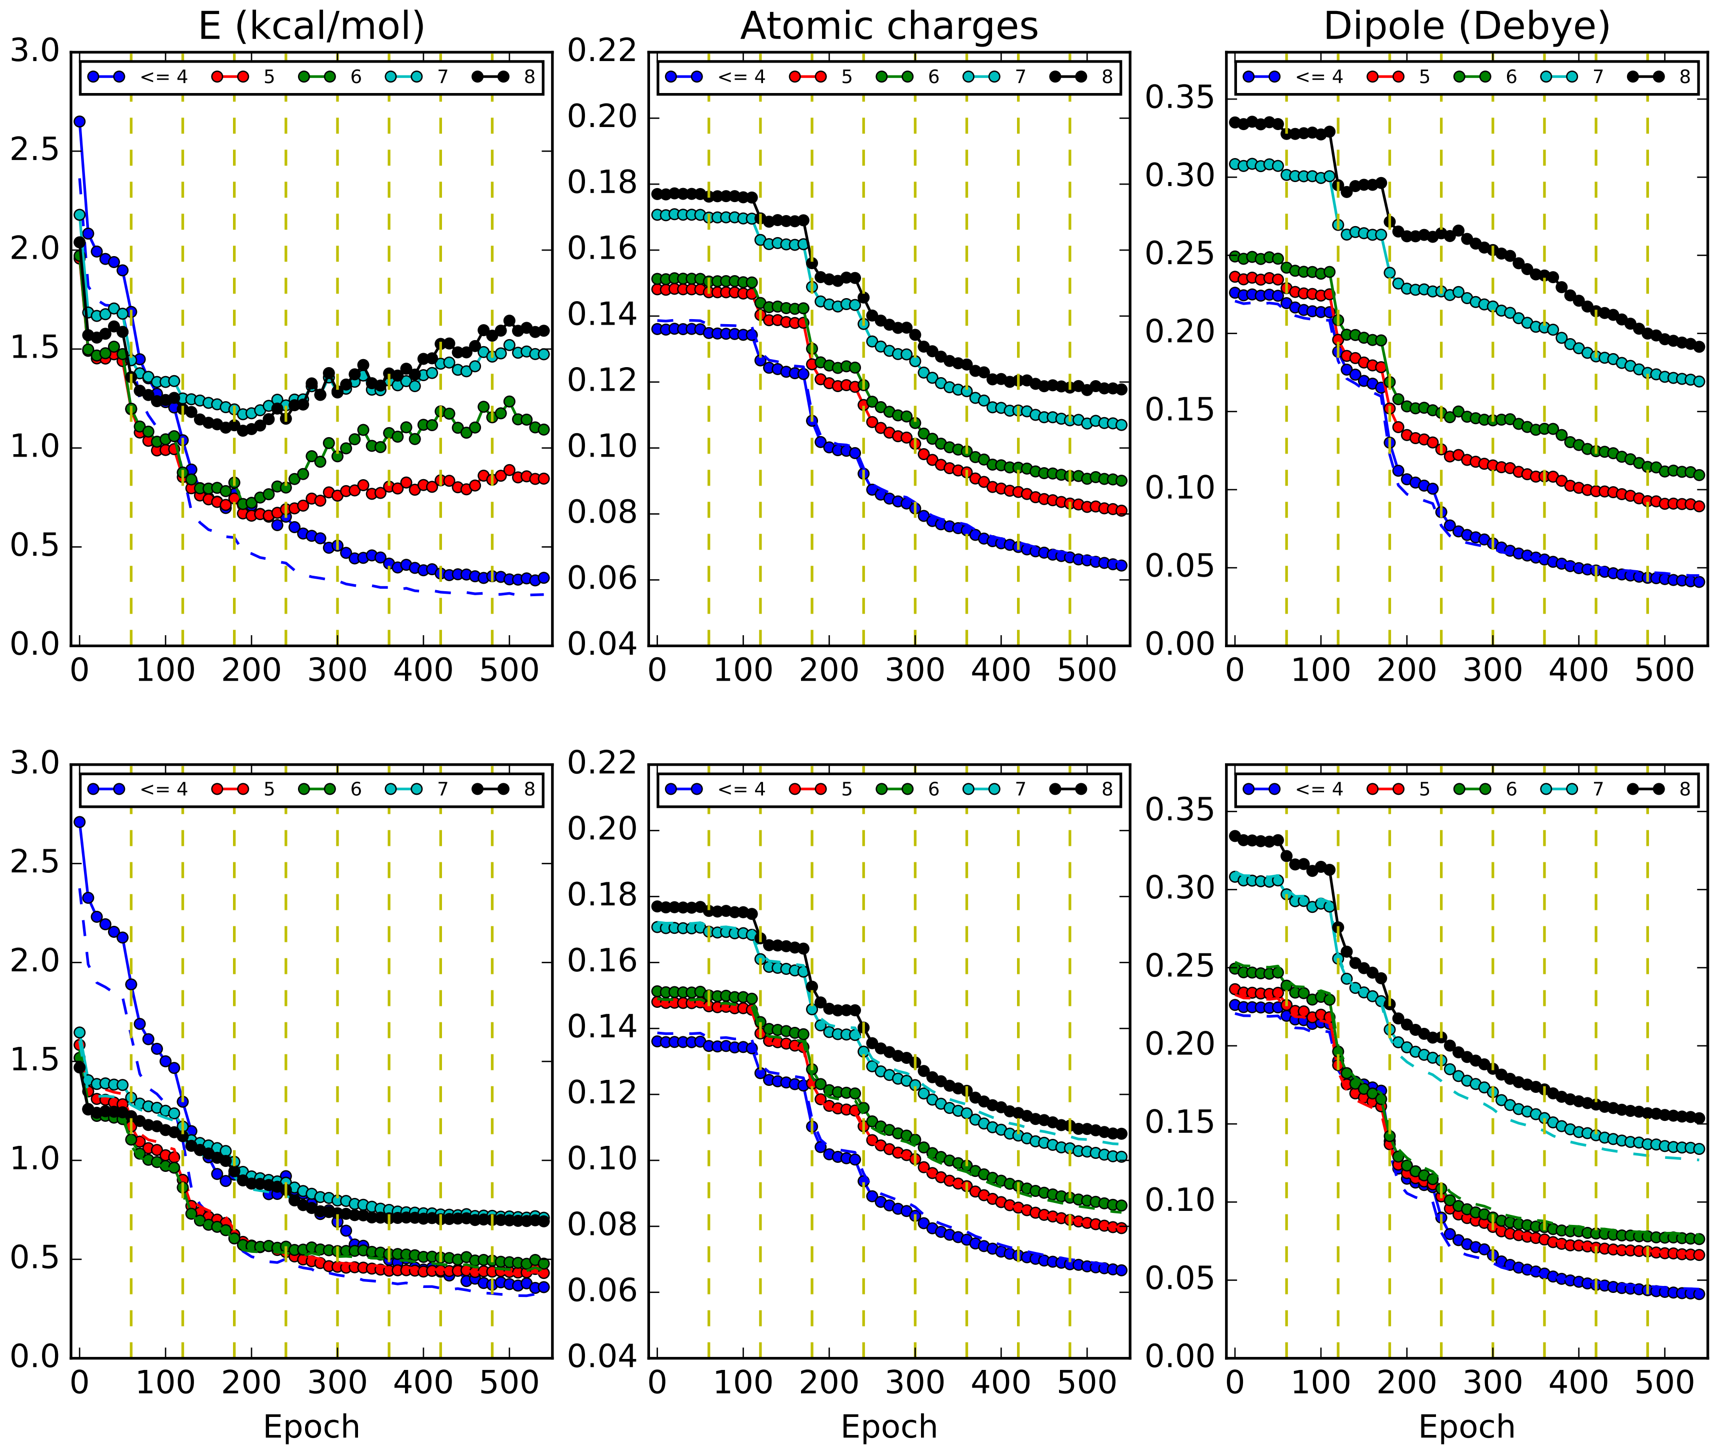

Figure S54 H Diag: FFNN 15 H Off Diag: FFNN 15
G Diag: FFNN 15 G Off Diag: FFNN 15 Repulsive: Spline

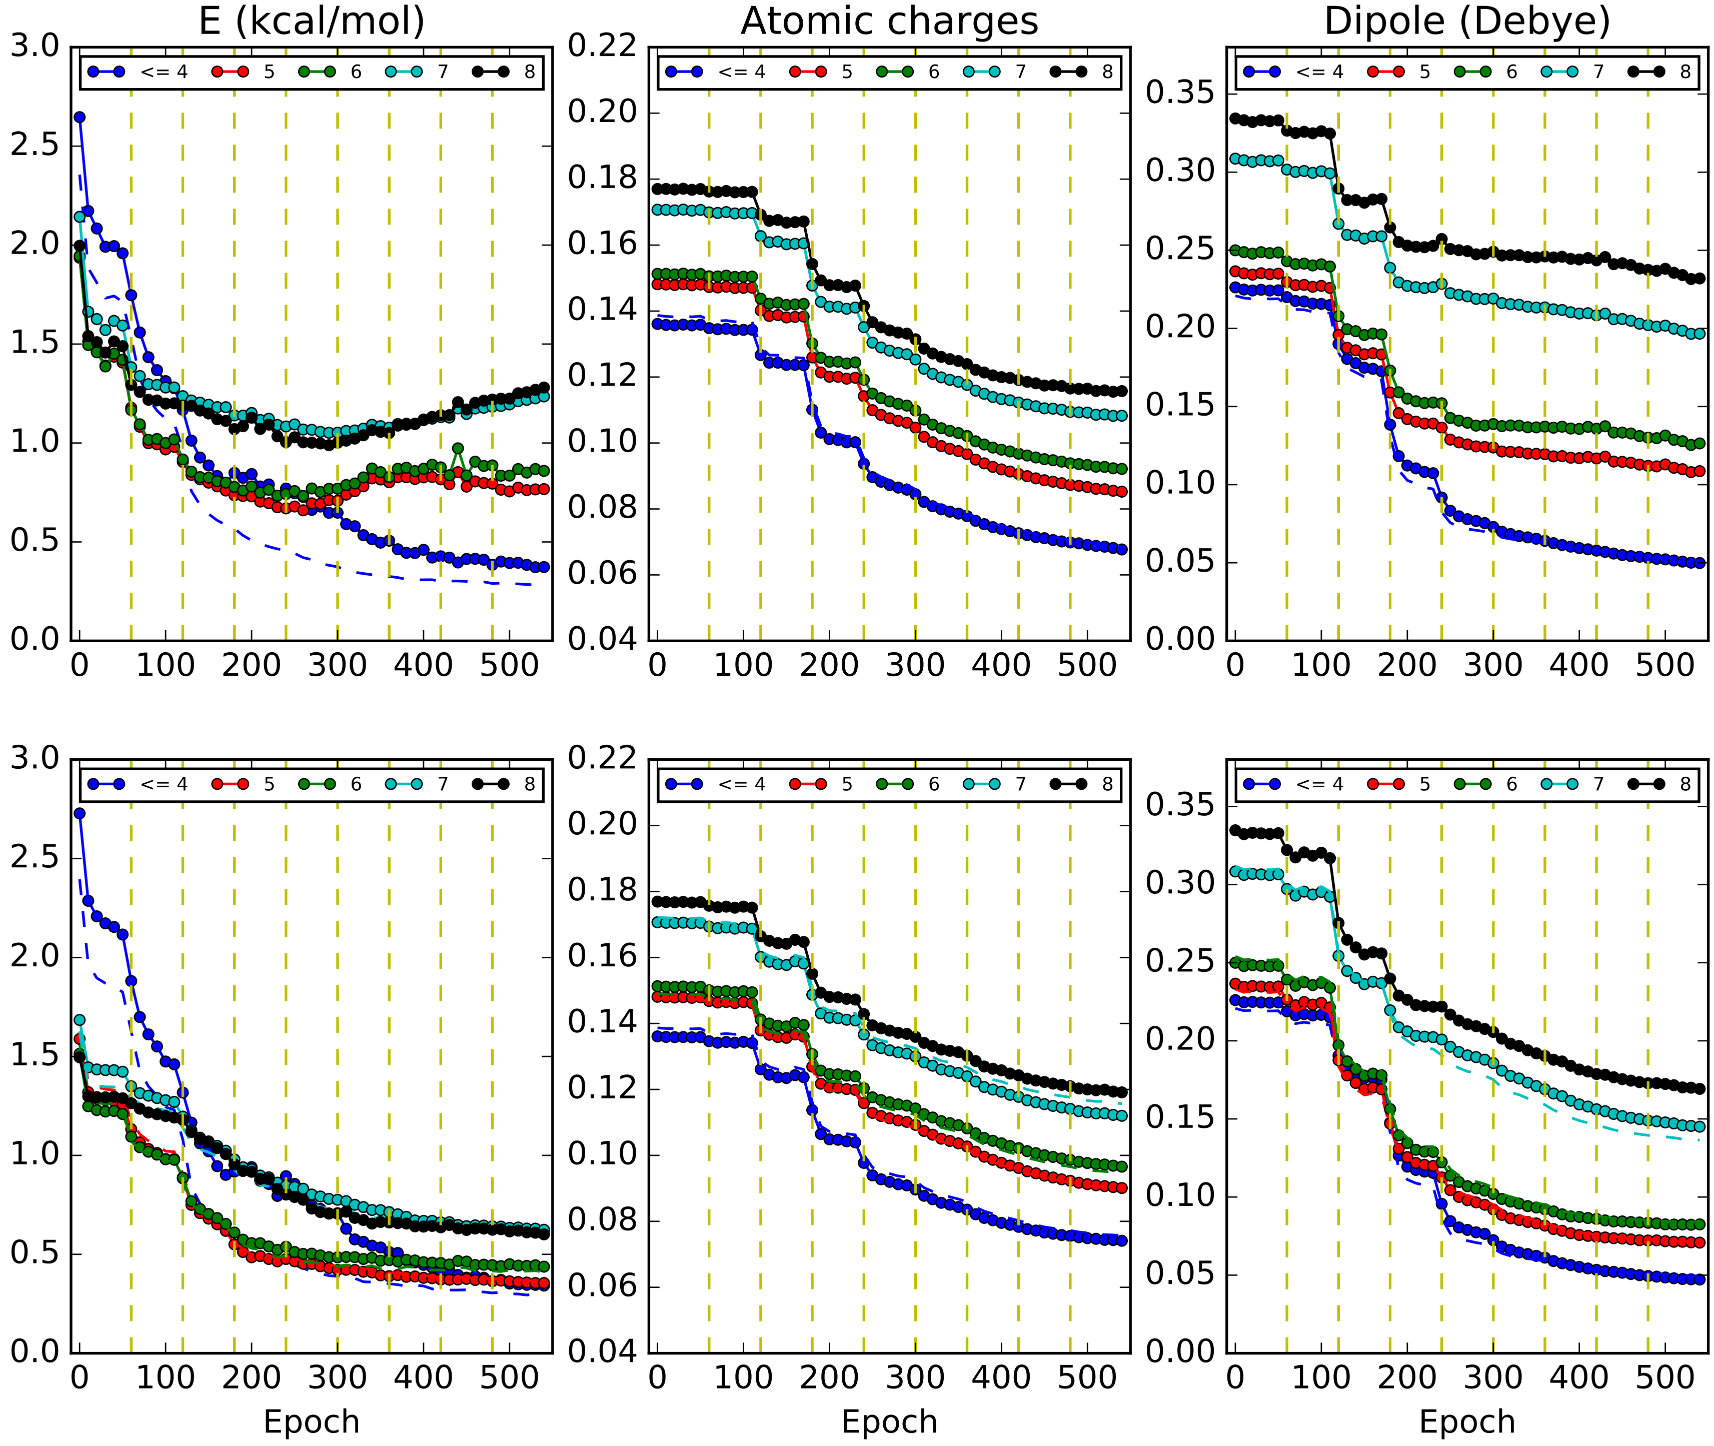

Figure S55 H Diag: FFNN 16 H Off Diag: FFNN 16
G Diag: FFNN 16 G Off Diag: FFNN 16 Repulsive: Spline

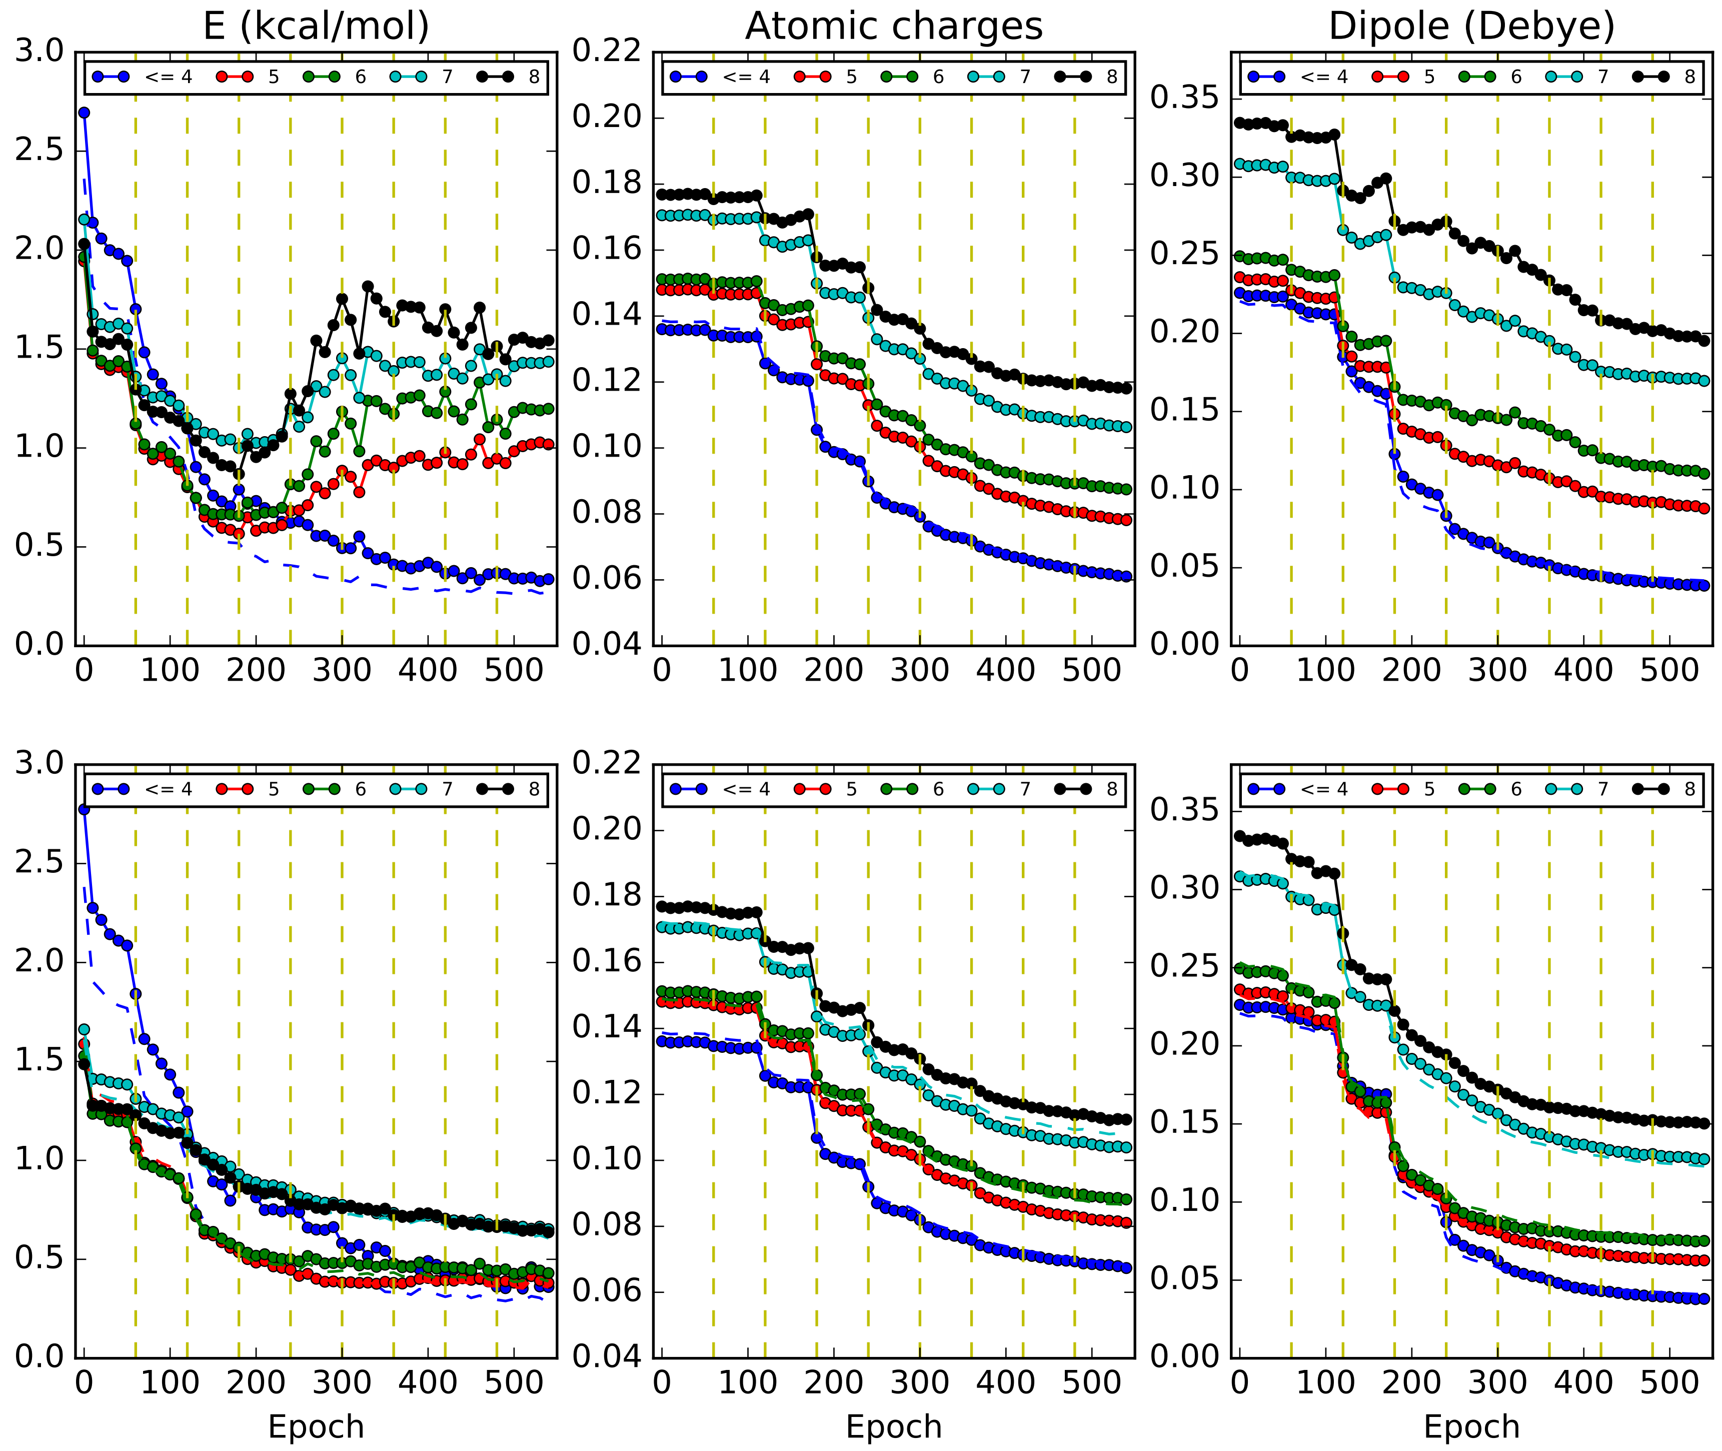

Figure S56 H Diag: FFNN 2 EB H Off Diag: FFNN 2 EB
G Diag: FFNN 2 EB G Off Diag: FFNN 2 EB Repulsive: Spline

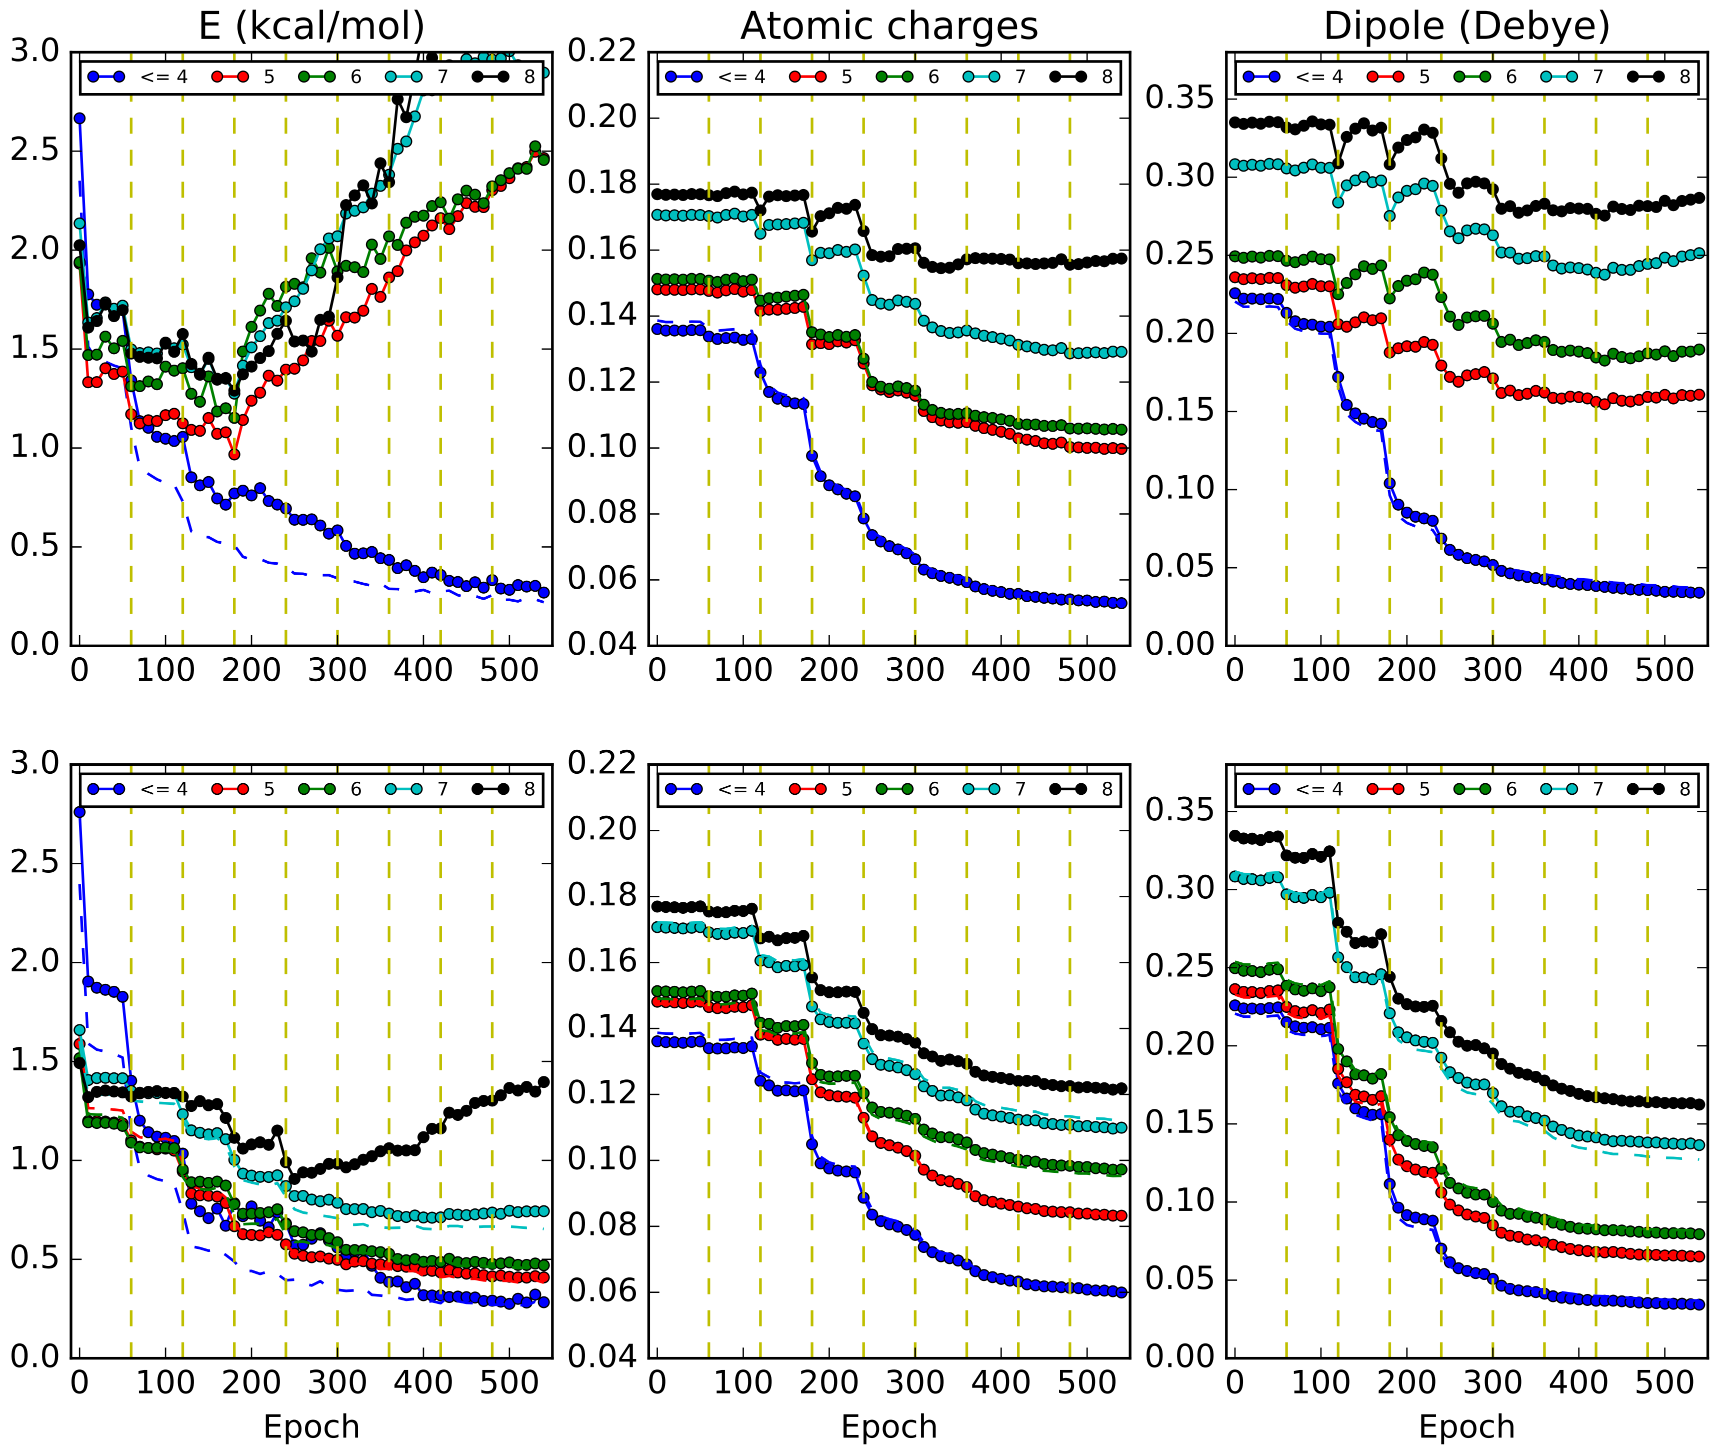

Figure S57 H Diag: FFNN 3 EB H Off Diag: FFNN 3 EB
G Diag: FFNN 3 EB G Off Diag: FFNN 3 EB Repulsive: Spline

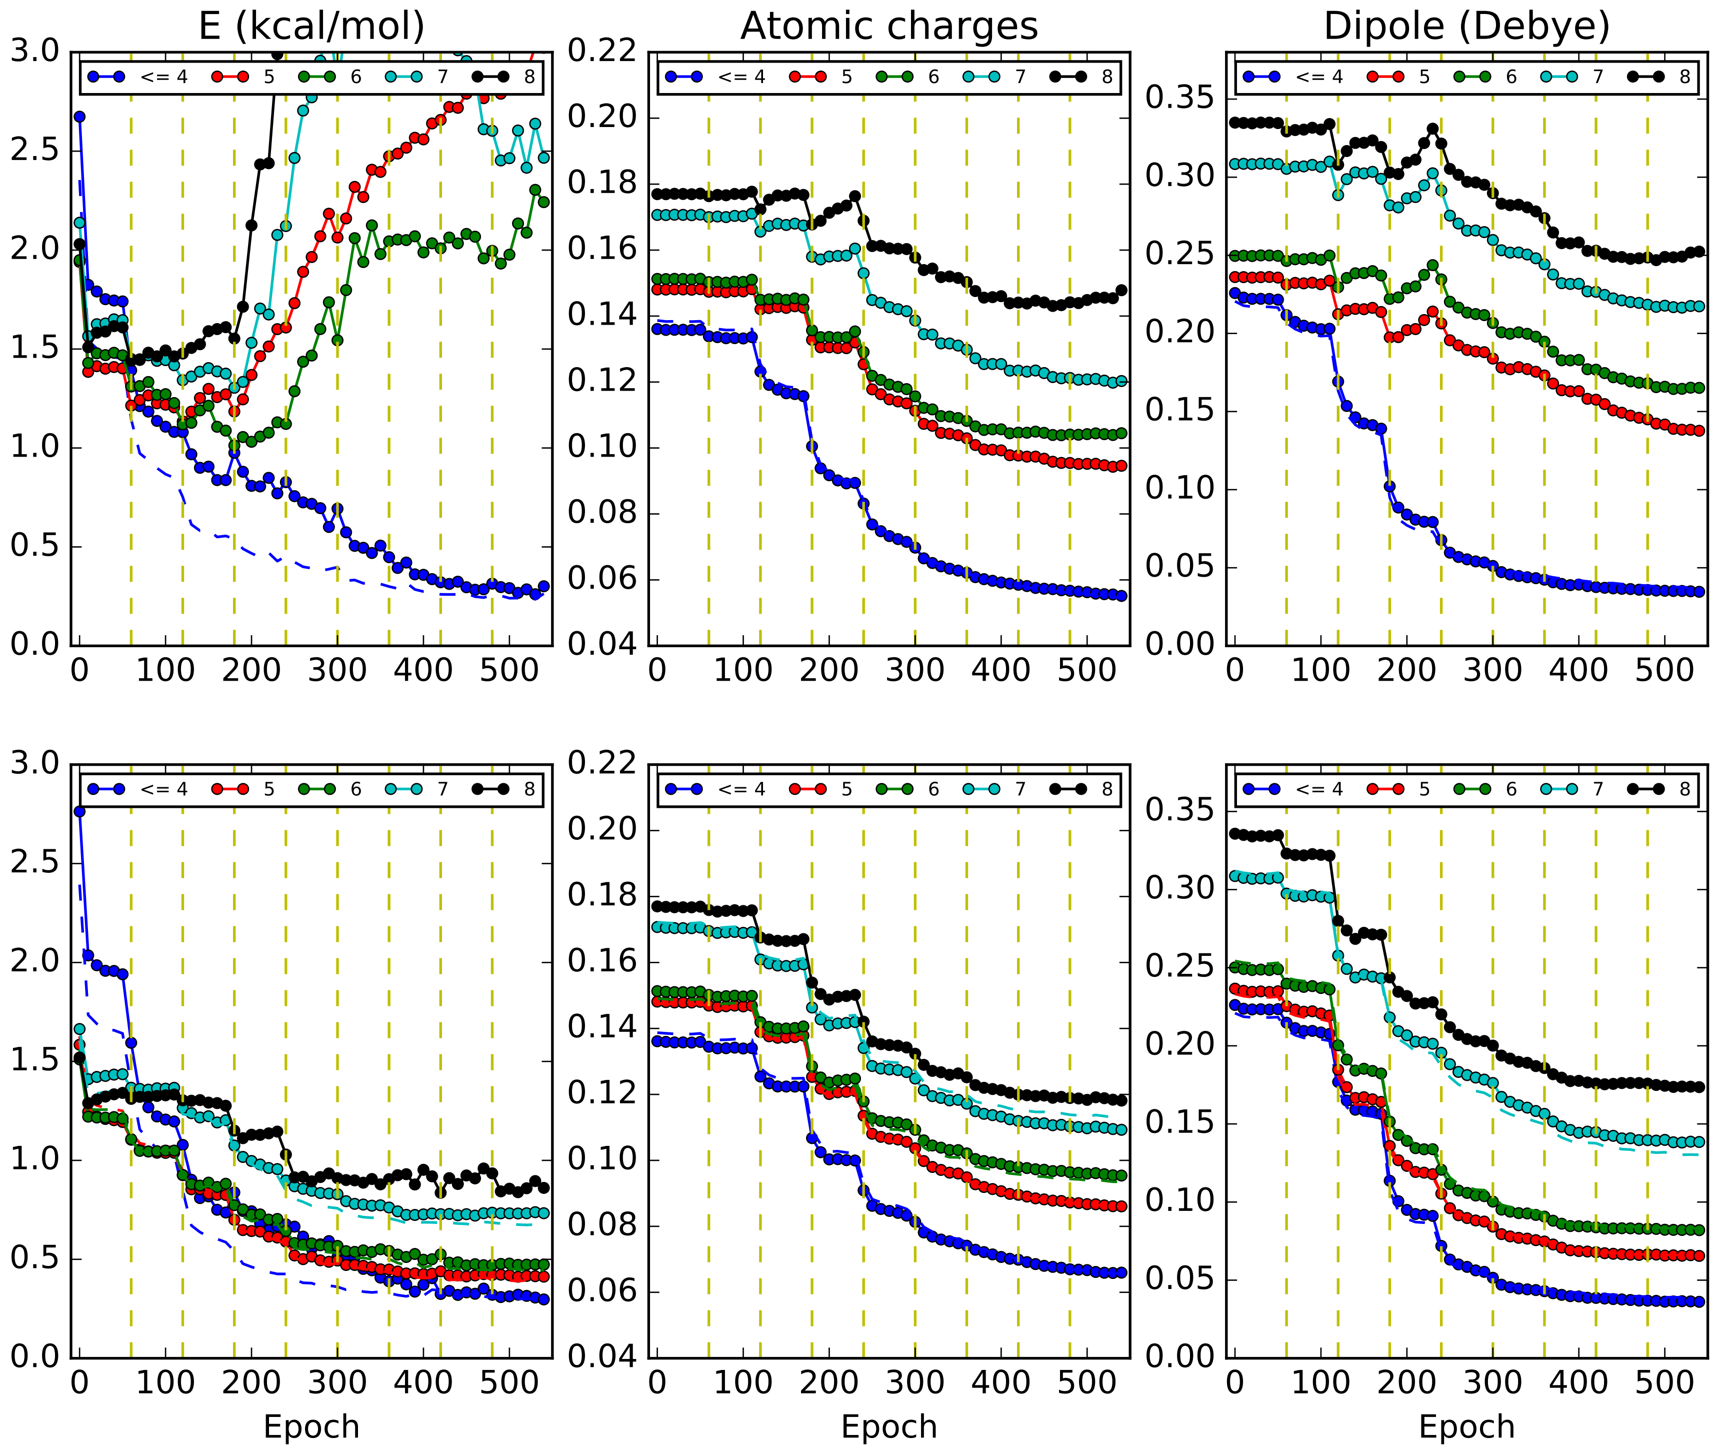

Figure S58 H Diag: FFNN 4 EB H Off Diag: FFNN 4 EB
G Diag: FFNN 4 EB G Off Diag: FFNN 4 EB Repulsive: Spline

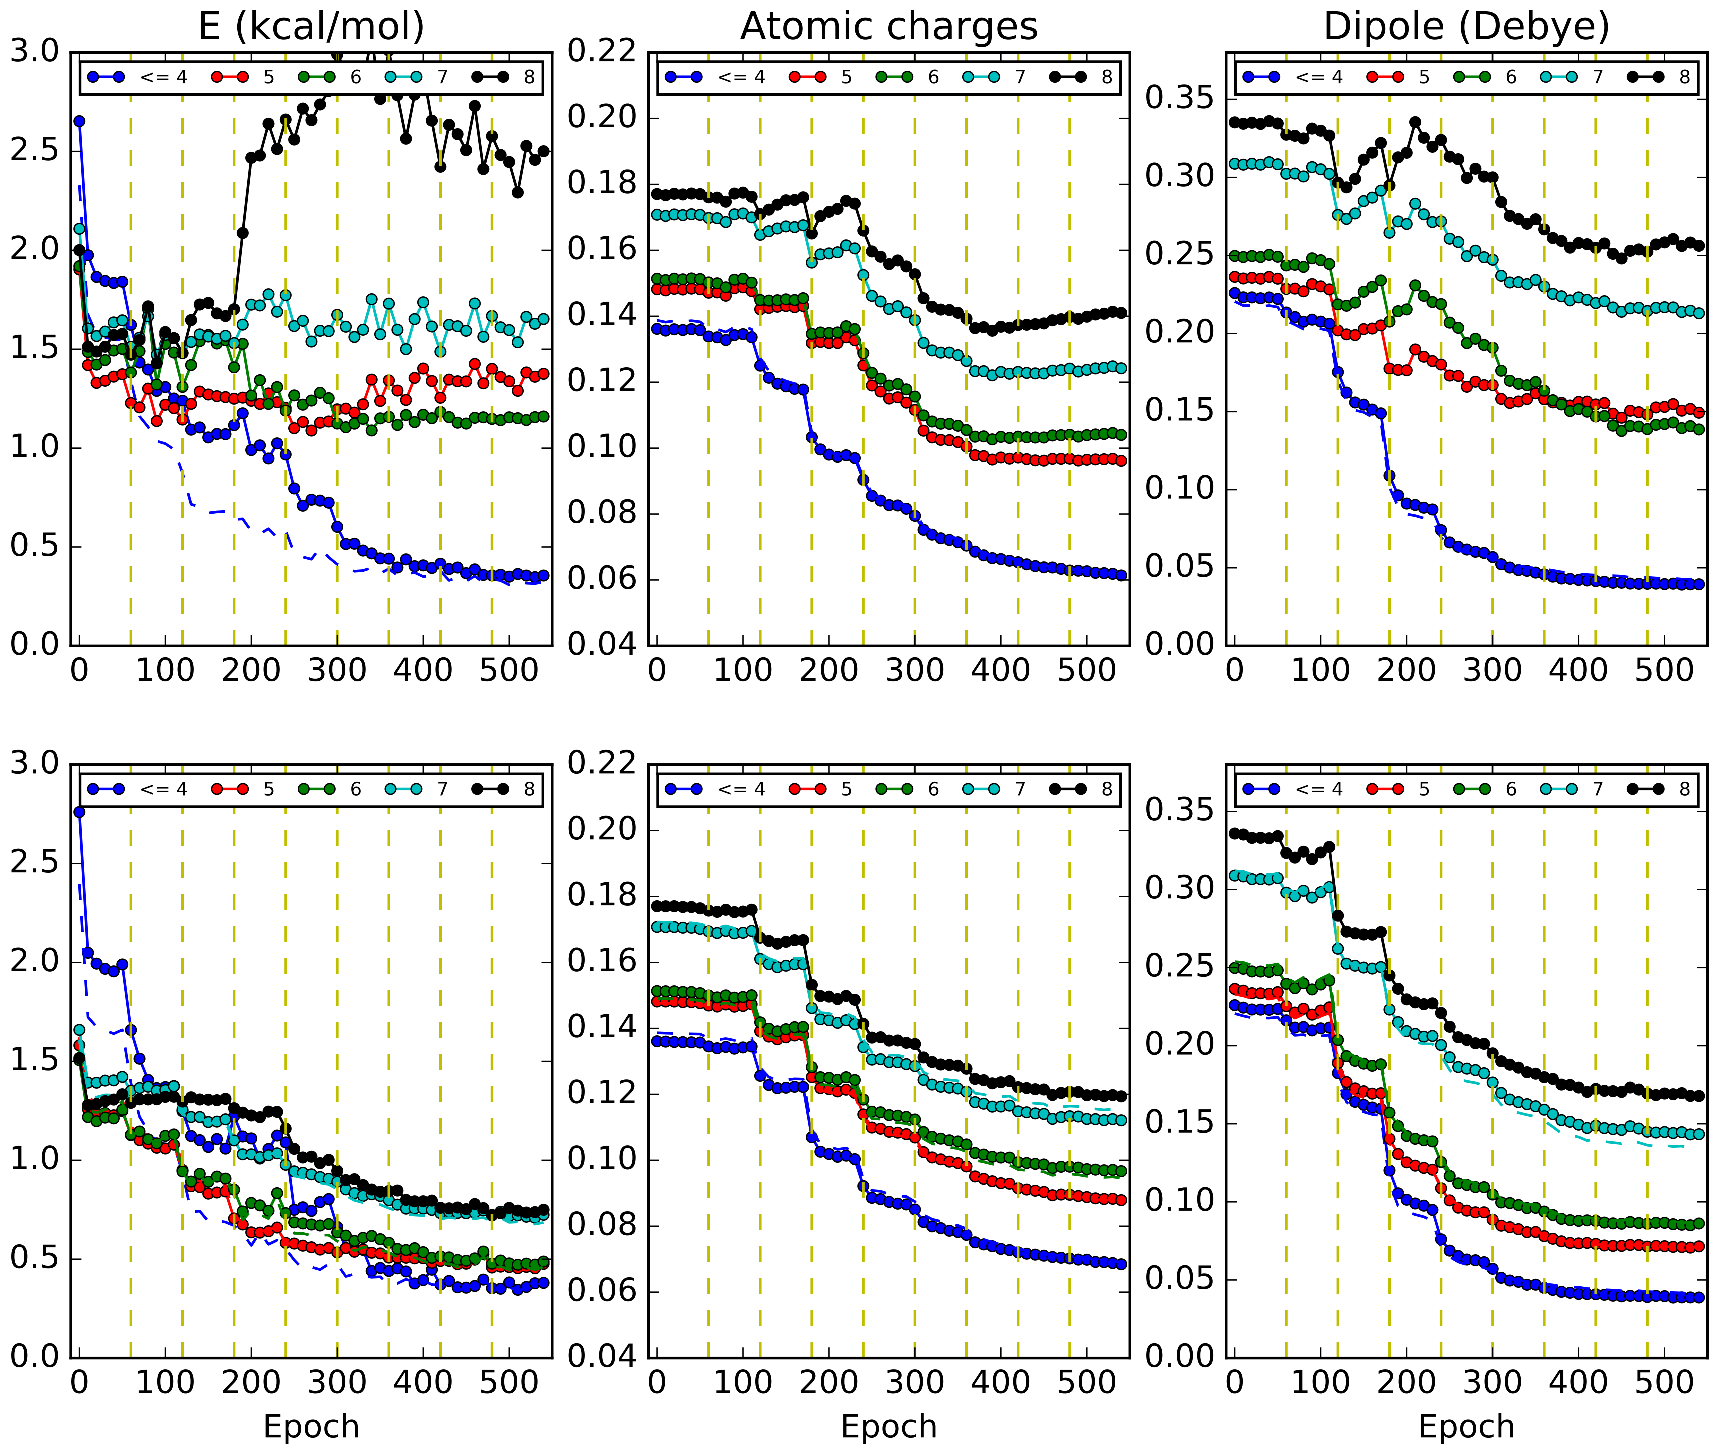

Figure S59 H Diag: FFNN 5 EB H Off Diag: FFNN 5 EB
G Diag: FFNN 5 EB G Off Diag: FFNN 5 EB Repulsive: Spline

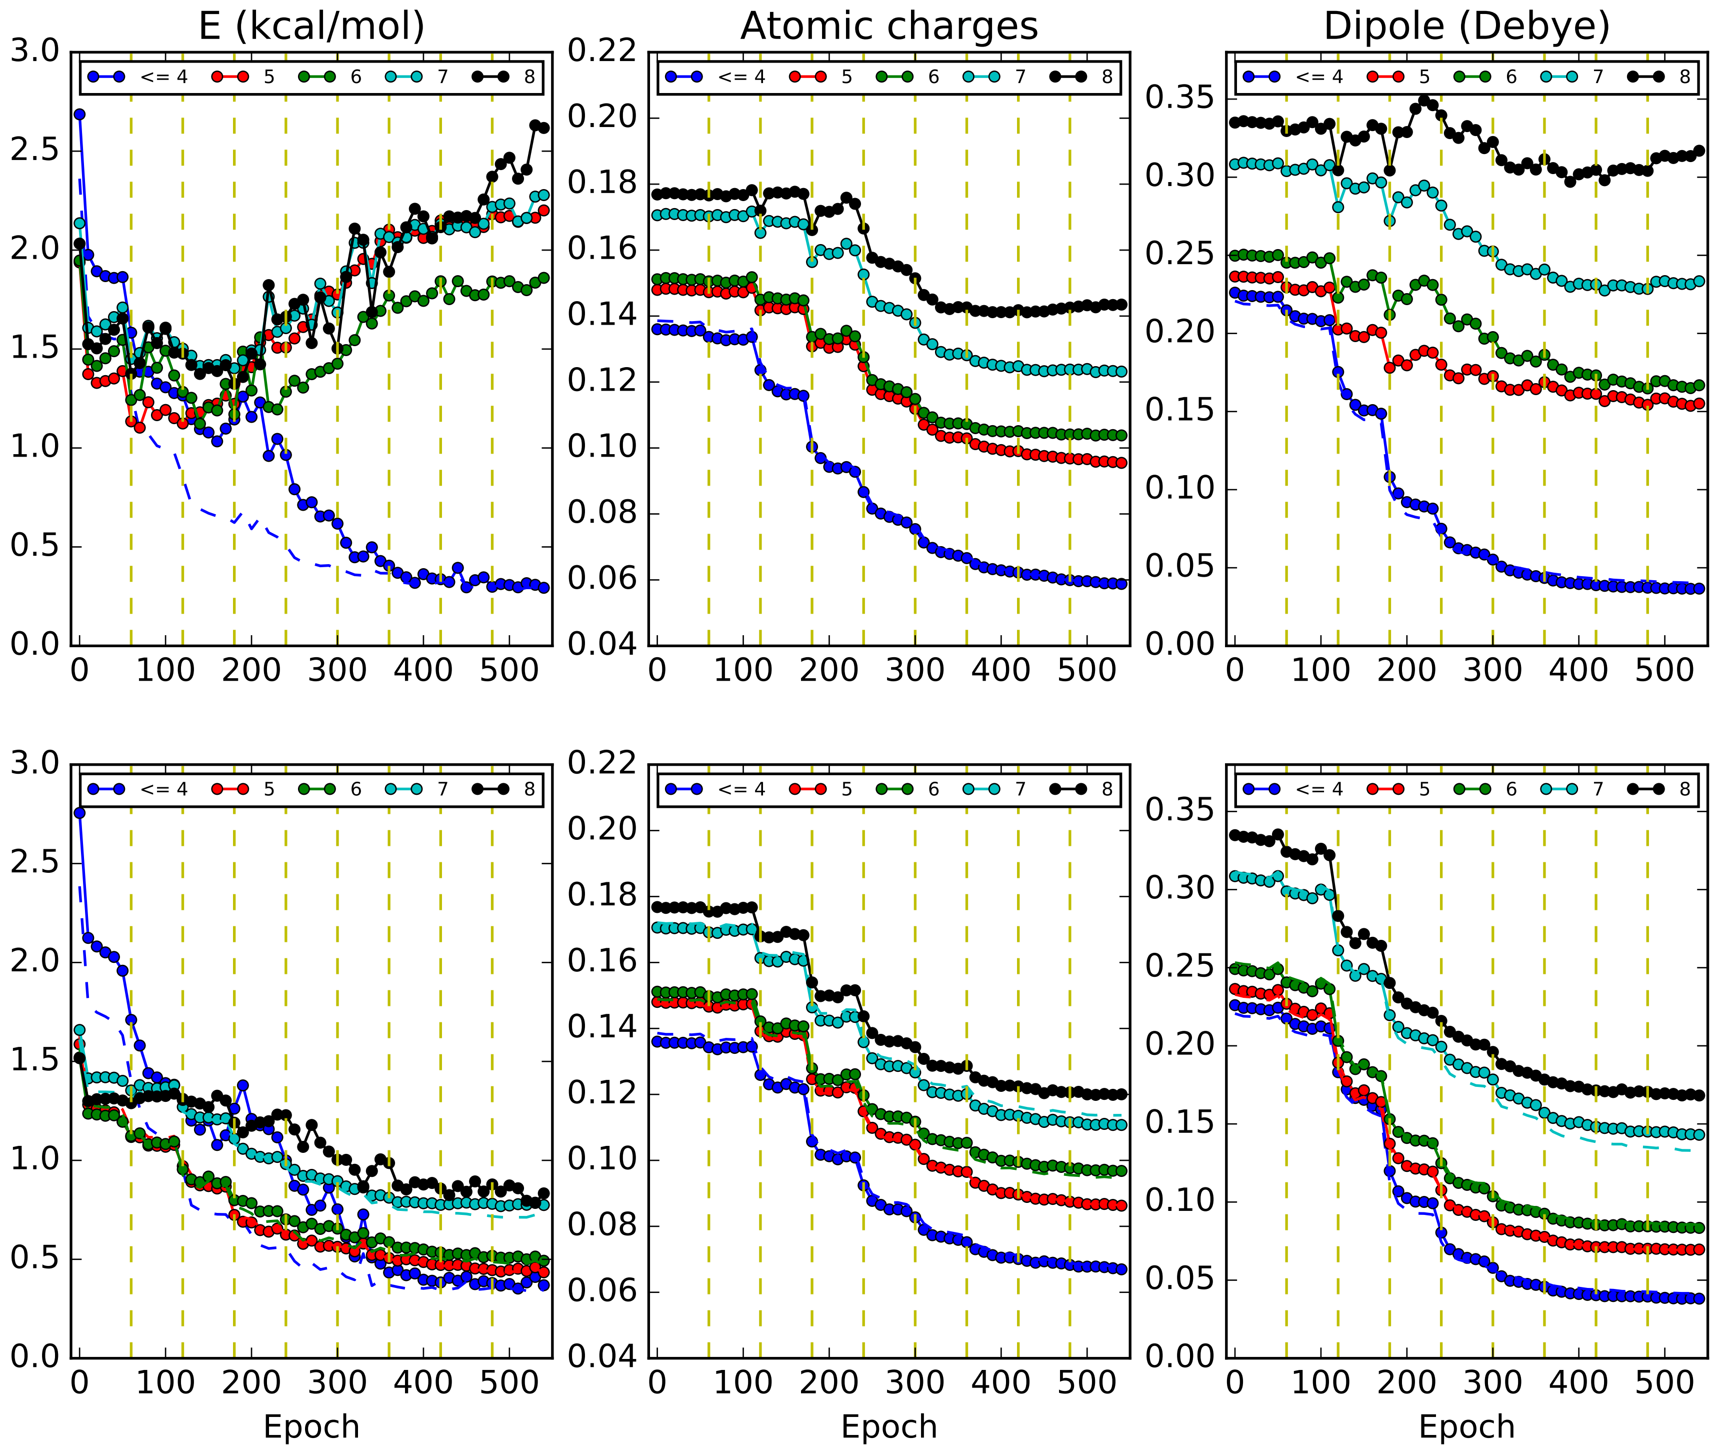

Supplement: Supplementary file 2 [file supporting_info.pdf]
